# Supplementary material for: Tightening Bounds on Probabilities of Causation By Merging Datasets
Source: arXiv:2310.08406 source file (2023-10-12)
Supplement: Supplementary file 2 [file causal_graph_structure.tex]

\newcommand{\yshift}{-4em}
\newcommand{\xshift}{5em}
\newcommand{\xzcol}{red!60!white}
\newcommand{\yzcol}{blue!60!white}

\begin{figure}[h]
\centering\subfigure[]
 {\begin{tikzpicture}\label{v-structure}
 \centering
 \node (X) [obs,thick] {$X$};
 \node (Y) [obs, xshift=2*\xshift] {$Y$};
 \node (Z) [obs, xshift=\xshift, yshift=\yshift] {$Z$};
 \edge [color=\xzcol, thick] {X}{Z};
 \edge [color=\yzcol, thick] {Y}{Z};
 \plate[yshift=-0.em,
 inner sep=0.5em,
 ultra thick,
 color=\yzcol] {M2}{(Y) (Z)}{\textcolor{\yzcol}{\textbf{RCT 2}}};
 \tikzset{plate caption/.style={caption, node distance=0, inner sep=0pt, below left=5pt and 0pt of #1.south,text height=.2em,text depth=0.3em}}
 \plate[yshift=0.3em,
 inner sep=0.5em,
 ultra thick,
 color=\xzcol] {M1}{(X) (Z)}{\textcolor{\xzcol}{\textbf{RCT 1}}}; \end{tikzpicture}\label{fig:causal-graph}}
\caption{(a) \small \textbf{Causal graph representing independent clinical trials studying identical outcomes.}}
\end{figure}
