# Supplementary material for: Tightening Bounds on Probabilities of Causation By Merging Datasets
Source: arXiv:2310.08406 source file (2023-10-12)
Supplement: Supplementary file 4 [file old_main.tex]

\documentclass{article}
\usepackage{graphicx} % Required for inserting images
\usepackage{amsmath}
\usepackage{amsthm}
\usepackage{amssymb}
\usepackage{color}
\usepackage{subfigure}
\usepackage{tikz}
\usepackage{comment}
\usepackage[toc,page]{appendix}
\usetikzlibrary{shapes.geometric,positioning,bayesnet,calc,intersections,through,backgrounds}
\usetikzlibrary{arrows,shapes,plotmarks,positioning}
\usetikzlibrary{decorations.markings}
\usepackage{tkz-euclide}
\usepackage{pgfplots}
\tikzset{>=stealth'}
\tikzstyle{graphnode} =
   [circle,draw=black,minimum size=22pt,text centered,text
     width=22pt,inner sep=0pt]
\tikzstyle{var}   =[graphnode,fill=white]
\tikzstyle{vardashed}   =[graphnode,draw=gray,fill=white]
\tikzstyle{obs}   =[graphnode,fill=black,text=white]
\tikzstyle{obsgrey}   =[graphnode,draw=white,fill=lightgray,text=black]
\tikzstyle{par}    =[graphnode,draw=white,fill=red,text=black]
 \tikzstyle{crucial} =[graphnode,draw=white,fill=yellow,text=black]
\tikzstyle{fac}   =[rectangle,draw=black,fill=black!25,minimum size=5pt]
\tikzstyle{facprior} =[rectangle,draw=black,fill=black,text=white,minimum size=5pt]
\tikzstyle{edge}  =[draw=white,double=black,very thick,-]
\tikzstyle{blueedge}  =[draw=white,double=blue,very thick,-]
\tikzstyle{rededge}  =[draw=white,double=red,very thick,-]
\tikzstyle{prior} =[rectangle, draw=black, fill=black, minimum size=
5pt, inner sep=0pt]
\tikzstyle{dirprior} = [circle, draw=black, fill=black, minimum
size=5pt, inner sep=0pt]
\tikzstyle{dot_node}=[draw=black,fill=black,shape=circle]
\usepackage{enumitem}

\newtheorem{theorem}{Theorem}
\newtheorem{remark}[theorem]{Remark}
\newcommand\atalanti[1]{\textcolor{blue}{Atalanti: #1} }% Notes for Atalanti
\newtheorem{lemma}[theorem]{Lemma}
\makeatletter
\renewcommand*\env@matrix[1][*\c@MaxMatrixCols c]{%
  \hskip -\arraycolsep
  \let\@ifnextchar\new@ifnextchar
  \array{#1}}
\makeatother

\setlist[itemize]{leftmargin=*,itemsep=0em,topsep=0em}
\setlist[enumerate]{leftmargin=*,itemsep=0em,topsep=0em}
\usepackage{csquotes}
\usepackage{natbib}
\bibliographystyle{unsrtnat}

\title{Appendix For Tightening Bounds on Probabilities of Causation By Merging Datasets}
\author{}
\makeatletter
\newcommand{\xRightarrow}[2][]{\ext@arrow 0359\Rightarrowfill@{#1}{#2}}
\newcommand{\independent}{\perp \!\!\! \perp}
\makeatother

\begin{document}

\maketitle
\appendix
\section{Proof of Theorem 1}
To prove Theorem 1, we first state lemmas we utilize as part of our proof. The lemmas are organized in subsections as follows. First, Lemma 1 and 2 are needed to constrain the set of target distributions using the external dataset (\S \ref{subsec:constraint_set_target_distr}) and to express the set of target distributions compatible with the external distribution as a system of equations and its $N$ corresponding free parameters, where $N + 1$ is the cardinality of the support of $Y$. Furthermore, they place bounds on the free parameters in this system. Lemma 3 and 4 examine the conditions that govern the bounds on the free parameters. Next, Lemma 5 and 6 re-express the bounds on $PNS$ originally derived using the joint distributions $P(Z, X, Y)$ in terms of the free parameters derived in Lemma 1 and Lemma 2. Lemmas 7 through 20 examine the behavior of the maximum  operators in the bounds provided in Lemma 5 and 6 under various constraints on the free parameters. Finally, we use these lemmas to provide the proof for the lower bound and upper bound of the PNS. The proof for the lemmas can be found in Section \ref{sec:lemma-proofs}. 

\subsection{Constraining the Set of Target Distributions Using the External Dataset}\label{subsec:constraint_set_target_distr}


\begin{lemma}\label{lemma:RREF-y}
Let $X$ and $Z$ be binary random variables, and let $Y$ be a discrete random variable taking on values in $0, \dots ,N$. Let $X$, $Y$ and $Z$ obey the causal structure in Fig. 3(b). Then, given marginals $P^T(Z, X)$ and $P^E(Z, Y)$, the conditional distributions $P(Z \mid X, Y)$ can be expressed in terms of free parameters $P(Z = 1 \mid X = 1, Y = i)$ for $i \in \{1, \dots, N\}$ as

{\small
\begin{align*}
\mathbb{P}(Z = 1 \mid X = 0, Y = 0) &=  \frac{p_x}{1 - p_x}\sum_{n = 1}^N\frac{p_{y_n}}{p_{y_0}}\mathbb{P}(Z = 1 \mid X = 1, Y = n) + \frac{p^E_{10}p_{y_0} - p^T_{11}p_x}{(1 - p_x)p_{y_0}}\\
\mathbb{P}(Z = 1 \mid X = 1, Y = 0)&= \frac{p^T_{11}}{p_{y_0}} - \sum_{n = 1}^N\frac{p_{y_n}}{p_{y_0}}\mathbb{P}(Z = 1 \mid X = 1, Y = n)\\
\mathbb{P}(Z = 1 \mid X = 0, Y = 1)&= \frac{p^E_{11}}{1 - p_x} - \frac{p_x}{1 - p_x}\mathbb{P}(Z = 1 \mid X = 1, Y = 1)\\
\mathbb{P}(Z = 1 \mid X = 0, Y = 2)&= \frac{p^E_{12}}{1 - p_x} - \frac{p_x}{1 - p_x}\mathbb{P}(Z = 1 \mid X = 1, Y = 2)\\
\vdots\\
\mathbb{P}(Z = 1 \mid X = 0, Y = N)&= \frac{p^E_{1N}}{1 - p_x} - \frac{p_x}{1 - p_x}\mathbb{P}(Z = 1 \mid X = 1, Y = N)\\
\end{align*}
}
Where $P(X = 1)$ is denoted as $p_x$, $P(Y = n)$ is denoted as $p_{y_n}$, $P^T(Z = 1 \mid X = 1)$ is denoted as $p^T_{11}$, $P^T(Z = 1 \mid X = 0)$ is denoted as $p^T_{10}$, and $P^E(Z = 1 \mid Y = n)$ is denoted as $p^E_{1n}$ for $n \in \{0, \dots, N\}$.
\end{lemma}

\begin{lemma}\label{lem:free-param-bounds}
To ensure the solution to the system of equations in Lemma \ref{lemma:RREF-y} form coherent probabilities, the following bounds on the free parameters must hold
{\small
\begin{align}\label{eq:sum-bounds}
\max\begin{bmatrix}
   \frac{p^T_{11}p_x - p^E_{10}p_{y_0}}{p_x} \\
   p_{11} - p_{y_0}
\end{bmatrix} \leq \sum_{n = 1}^N p_{y_n}\mathbb{P}(Z = 1 \mid X = 1, Y = n) 
\leq \min\begin{bmatrix}
    \frac{(1 - p_x)p_{y_0} + p^T_{11}p_x - p^E_{10}p_{y_0}}{p_x}\\
    p^T_{11}
\end{bmatrix}
\end{align}
}

And for each $i \in \{1, \dots, N\}$, we the bounds on the following free parameters $P(Z = 1\mid X = 1, Y = i)$
\begin{align}\label{eq:individual-bounds}
    \max\begin{bmatrix}
        0\\
        \frac{p^E_{1i} - (1 - p_x)}{p_x}
    \end{bmatrix}
        \leq P(Z = 1\mid X = 1, Y = i) \leq 
    \min\begin{bmatrix}
        1\\
        \frac{p^E_{1i}}{p_x}
    \end{bmatrix}
\end{align}
\end{lemma}

\subsection{Relation of Bounds on Free Parameters to the External Dataset}

Lemma \ref{lem:bounds-conditions} and Lemma \ref{lem:inidiv-bounds-conditions} establish the relationship between the external dataset and the upper and lower bounds in Lemma \ref{lem:free-param-bounds}.
\begin{lemma}\label{lem:bounds-conditions}
    The following implications hold:
    \begin{enumerate}
        \item 
        \begin{equation*}
        p^E_{10} < p_x \implies \frac{p^T_{11}p_x - p^E_{10}p_{y_0}}{p_x} > p^T_{11} - p_{y_0}   
        \end{equation*}
    
        \item 
        \begin{equation*}
        p^E_{10} \geq p_x \implies \frac{p^T_{11}p_x - p^E_{10}p_{y_0}}{p_x} \leq p^T_{11} - p_{y_0}   
        \end{equation*}
        \item 
        \begin{equation*}
        p^E_{10} < 1 - p_x \implies p^T_{11} < \frac{(1 - p_x)p_{y_0} + p^T_{11}p_x - p^E_{10}p_{y_0}}{p_x}
        \end{equation*}
        \item 
        \begin{equation*}
        p^E_{10} \geq 1 - p_x \implies p^T_{11} \geq \frac{(1 - p_x)p_{y_0} + p^T_{11}p_x - p^E_{10}p_{y_0}}{p_x}
        \end{equation*}
\end{enumerate}
\end{lemma}
\begin{lemma}\label{lem:inidiv-bounds-conditions}
For $i \in \{1, \dots, N\}$, when $p^E_{1i} \geq 1 - p_x \implies \frac{p^E_{11} - (1 - p_x)}{p_x} \geq 0$. When $p^E_{1i} < p_x \implies \frac{p^E_{11}}{p_x} \leq 1$    
\end{lemma}

\subsection{Bounds on PNS In Terms of Free Parameters}

In Lemma \ref{lem:joint-bounds}, we re-express bounds in \cite{dawid2017probability} on PC in terms of PNS under the assumption of exogenity. 
\begin{lemma}\label{lem:joint-bounds}
Let $X$, $Z$ be binary random variables, and let $Y$ be a discrete multivalued random variable, obeying the causal structure in Fig 2. We define the $PNS$ as
\begin{equation*}
    PNS \equiv P(Z_{\mathbf{x}} = 1, Z_{\mathbf{x^\prime}}  = 0)
\end{equation*}
Where $\mathbf{x}$ and $\mathbf{x^\prime}$ denote the setting of $X$ to $1$ and $0$ respectively. Bounds on the PNS under the causal graph in \ref{fig:causal-graph} given the joint distribution $P(Z, X, Y)$ are given in \cite{dawid2017probability} as 
\begin{align*}
    \Delta \leq PNS \leq \mathbb{P}(Z = 1 \mid X = 1) - \Gamma
\end{align*}

Where
\begin{equation*}
    \Delta = \sum_y \mathbb{P}(Y = y)\max \{0, \mathbb{P}(Z = 1 \mid X = 1, Y = y) - \mathbb{P}(Z = 1 \mid X = 0, Y = y)\} 
\end{equation*}

And $\Gamma$ is 
\begin{align*}
    \Gamma = \sum_y \mathbb{P}(Y = y)\max \{0, \mathbb{P}(Z = 1 \mid X = 1, Y = y) - \mathbb{P}(Z = 0 \mid X = 0, Y = y)\} 
\end{align*}
\end{lemma}

At this point we remind to the reader that the above bounds require access to the joint distribution $P(Z, X, Y)$. Given the scenario described in the paper, we do not have access to this. Therefore, in Lemma \ref{lem:max-operator-expressions} we are expressing the joint $P(Z\mid  X, Y)$ in terms of the free parameters corresponding to the system of equations derived in Lemma \ref{lemma:RREF-y}. 
\begin{lemma}\label{lem:max-operator-expressions}
    Given $P(Z, X)$ and $P(Z, Y)$, using the solution to the system of equations in Lemma \ref{lemma:RREF-y}, each of the terms in $\Delta$ and $\Gamma$ defined in Lemma \ref{lem:joint-bounds} are expressed in terms of the free parameters below. First, for $\Gamma$, each of the terms can be written as
    \[
    \mathbb{P}(Z = 1 \mid X = 1, Y = 0) - \mathbb{P}(Z = 0 \mid X = 0, Y = 0)
    \]
    \begin{equation}
    = \frac{p^E_{10} - (1 - p_x)}{1 - p_x} + \frac{\sum_{n = 1}^N p_{y_n}P(Z = 1 \mid X = 1, Y = n) - p^T_{11}}{p_{y_0}}\Bigg(\frac{p_x}{1 - p_x} - 1\Bigg)
    \end{equation}
    And for the terms in $\Gamma$ corresponding to $Y = i$, $i \in \{1, \dots , N\}$
    \[
    P(Z = 1 \mid X = 1, Y = i) - P(Z = 0 \mid X = 0, Y = i)
    \]
    \begin{equation}
        P(Z = 1 \mid X = 1, Y = i)\Bigg(1 - \frac{p_x}{1 - p_x}\Bigg) + \frac{p^\prime_{11} - (1 - p_x)}{1 - p_x}
    \end{equation}
    Similarly, the terms in $\Delta$ can be expressed in terms of the free parameter as
    \[
    \mathbb{P}(Z = 1 \mid X = 1, Y = 0) - \mathbb{P}(Z = 1 \mid X = 0, Y = 0)
    \]
    \begin{equation}
       \frac{p^T_{11} - p^E_{10}p_{y_0} - \sum_{n = 1}^N p_{y_n}\mathbb{P}(Z = 1\mid X = 1, Y = n)}{(1 - p_x)p_{y_0}} 
    \end{equation}
    And for the terms in $\Delta$ corresponding to $Y = i$, $i \in \{1, \dots , N\}$
    \[
    \mathbb{P}(Z = 1 \mid X = 1, Y = 1) - \mathbb{P}(Z = 1 \mid X = 0, Y = 1)
    \]
    \begin{equation}
        \frac{\mathbb{P}(Z = 1 \mid X = 1, Y = i) - p^E_{1i}}{1 - p_x}
    \end{equation}
\end{lemma}


\subsection{Behavior of Max Operators in $\Gamma$}
The behavior of this function must be analyzed in two cases, one where $p_x > 1 - p_x$, and vice-versa. We present results for $p_x > 1 - p_x$, and analogous results can be derived for $p_x < 1 - p_x$. 

\begin{lemma}\label{lem:max-operator-gamma-0}
    Assume $p_x > 1 - p_x$. The function $\max \{0, \mathbb{P}(Z = 1 \mid X = 1, Y = 0) - \mathbb{P}(Z = 0 \mid X = 0, Y = 0)\}$ defined in Lemma \ref{lem:max-operator-expressions} will be greater than or equal to $0$ when
    \begin{equation}
            \sum_{n = 1}^N p_{y_n}P(Z = 1 \mid X = 1, Y = n) \geq \frac{p_{y_0}((1 - p_x) - p^E_{10})}{p_x - (1 - p_x)} + p^T_{11}
    \end{equation}
\end{lemma}

\begin{lemma}\label{lem:max-operator-gamma-0-positive}
    Assume $p_x > 1 - p_x$. If $p^E_{10} \geq p_x$, then 
    \[
    p^T_{11} - p_{y_0} \geq \frac{p_{y_0}((1 - p_x) - p^E_{10})}{p_x - (1 - p_x)} + p^T_{11}
    \]
\end{lemma}

\begin{remark}
    Lemma \ref{lem:max-operator-gamma-0} and Lemma \ref{lem:max-operator-gamma-0-positive} imply that when $p_x > 1 - p_x$, $p^E_{10} \geq \max\{p_x, 1 - p_x\}$ then 
\begin{align*}
    &\max\{0, \mathbb{P}(Z = 1 \mid X = 1, Y = 0) - \mathbb{P}(Z = 0 \mid X = 0, Y = 0)\}\\
    &= \mathbb{P}(Z = 1 \mid X = 1, Y = 0) - \mathbb{P}(Z = 0 \mid X = 0, Y = 0)
\end{align*}
\end{remark}

Analogously, when $p^E_{10} \leq \min\{p_x, 1 - p_x\}$, i.e. $p^E_{10} \leq 1 - p_x$, similar results are obtained, and to show this, we state the following Lemmas.
\begin{lemma}\label{lem:gamma-0-lower-side-px}
    Assume $p_x > 1 - p_x$. If $p^E_{10} < p_x$, then 
    \[
    \frac{p^T_{11}p_x - p^E_{10}p_{y_0}}{p_x} < \frac{p_{y_0}((1 - p_x) - p^E_{10})}{p_x - (1 - p_x)} + p^T_{11}
    \]
\end{lemma}

\begin{lemma}\label{lem:gamma-0-lower-side-1-minus-px}
    Assume $p_x > 1 - p_x$. If $p^E_{10} \leq 1 - p_x$, then 
    \[
    p^T_{11} \leq \frac{p_{y_0}((1 - p_x) - p^E_{10})}{p_x - (1 - p_x)} + p^T_{11}
    \]
\end{lemma}
\begin{remark}
Lemma \ref{lem:gamma-0-lower-side-px} and Lemma \ref{lem:gamma-0-lower-side-1-minus-px} imply that when $p_x > 1 - p_x$, $p^E_{10} \leq \min\{p_x, 1 - p_x\}$ then 
\begin{align*}
    &\max\{0, \mathbb{P}(Z = 1 \mid X = 1, Y = 0) - \mathbb{P}(Z = 0 \mid X = 0, Y = 0)\} = 0
\end{align*}    
\end{remark}

Next, consider the case when $1 - p_x < p^\prime_{10} < p_x$. Then the following bounds hold
\begin{align*}
   \frac{p_{11}x - p^\prime_{10}y_0}{p_x} 
 \leq \sum_{n = 1}^N y_n\mathbb{P}(Z = 1 \mid X = 1, Y = n) 
\leq \frac{(1 - x)y_0 + p_{11}x - p^\prime_{10}y_0}{x}
\end{align*}

From Lemma 9, $\frac{p_{11}x - p^\prime_{10}y_0}{x} < \frac{p_{y_0}((1 - p_x) - p^\prime_{10})}{p_x - (1 - p_x)} + p_{11}$. And under these conditions,
\begin{align*}
    \frac{p_{y_0}((1 - p_x) - p^\prime_{10})}{p_x - (1 - p_x)} + p_{11} < \frac{(1 - x)y_0 + p_{11}x - p^\prime_{10}y_0}{x}
\end{align*}

% \begin{lemma}
%     Assume $p_x < 1 - p_x$. The function $\max \{0, \mathbb{P}(Z = 1 \mid X = 1, Y = 0) - \mathbb{P}(Z = 0 \mid X = 0, Y = 0)\} \geq 0$ when
%     \begin{align*}
%             \sum_{n = 1}^N p_{y_n}P(Z = 1 \mid X = 1, Y = n) \leq \frac{p_{y_0}( p^\prime_{10} - (1 - p_x))}{(1 - p_x) - p_x} + p_{11}   
%     \end{align*}
% \end{lemma}
Now, we provide lemmas that similarly examine the behavior of $\max \{0, \mathbb{P}(Z = 1 \mid X = 1, Y = i) - \mathbb{P}(Z = 0 \mid X = 0, Y = i)\}$. As before, the behavior of this function needs to be analyzed in two case, and we provide lemmas for $p_x > 1 - p_x$, and lemmas for $p_x < 1 - p_x$ can be analogously derived.

\begin{lemma}
    Assume $p_x > 1 - p_x$. The function $\max \{0, \mathbb{P}(Z = 1 \mid X = 1, Y = i) - \mathbb{P}(Z = 0 \mid X = 0, Y = i)\} \geq 0$ for $i \in \{1, \dots, N\}$ when
    \begin{align*}
            P(Z = 1 \mid X = 1, Y = i) \leq \frac{p^\prime_{1i} - (1 - p_x)}{p_x - (1 - p_x)}    
    \end{align*}
\end{lemma}

\begin{lemma}
    Assume $p_x > 1 - p_x$. If $p^\prime_{1i} \geq x$ for $i \in \{1, \dots , N\}$, then 
    \begin{align*}
            1 \leq \frac{p^\prime_{1i} - (1 - p_x)}{p_x - (1 - p_x)}    
    \end{align*}
\end{lemma}
This implies that when $p^\prime_{1i} \geq \max \{p_x, 1 - p_x\}$, then
\begin{align*}
    &\max \{0, \mathbb{P}(Z = 1 \mid X = 1, Y = i) - \mathbb{P}(Z = 0 \mid X = 0, Y = i)\}\\
    &= \mathbb{P}(Z = 1 \mid X = 1, Y = i) - \mathbb{P}(Z = 0 \mid X = 0, Y = i)
\end{align*}

Next, when $p^\prime_{1i} \leq \min\{p_x, 1 - p_x\}$, then consider the following Lemmas.
\begin{lemma}
    Assume $p_x > 1 - p_x$. If $p^\prime_{1i} < p_x$ for $i \in \{1, \dots , N\}$, then 
    \begin{align*}
            \frac{p^\prime_{11}}{p_x} > \frac{p^\prime_{1i} - (1 - p_x)}{p_x - (1 - p_x)}    
    \end{align*}
\end{lemma}
\begin{lemma}
    Assume $p_x > 1 - p_x$. If $p^\prime_{1i} \leq 1 - p_x$ for $i \in \{1, \dots , N\}$, then 
    \begin{align*}
            0 \geq \frac{p^\prime_{1i} - (1 - p_x)}{p_x - (1 - p_x)}    
    \end{align*}
\end{lemma}
This implies that when $p^\prime_{1i} \leq \min \{p_x, 1 - p_x\}$, then
\begin{align*}
    &\max \{0, \mathbb{P}(Z = 1 \mid X = 1, Y = i) - \mathbb{P}(Z = 0 \mid X = 0, Y = i)\} = 0
\end{align*}

And when $1 - p_x < p^\prime_{1i} < p_x$, then $\frac{p^\prime_{11}}{p_x} > \frac{p^\prime_{1i} - (1 - p_x)}{p_x - (1 - p_x)}$ and $\frac{p^\prime_{11} - (1 - p_x)}{p_x} < \frac{p^\prime_{1i} - (1 - p_x)}{p_x - (1 - p_x)}$. 

\subsection{Behavior of Max Operators in $\Delta$}

\begin{lemma}
    The function $\max \{0, \mathbb{P}(Z = 1 \mid X = 1, Y = 0) - \mathbb{P}(Z = 1 \mid X = 0, Y = 0)\} \geq 0$ when
    \begin{align*}
        p_{11} - p^\prime_{10}p_{y_0} \geq  \sum_{n = 1}^N p_{y_n}\mathbb{P}(Z = 1\mid X = 1, Y = n)
    \end{align*}
\end{lemma}

\begin{lemma}
    The following inequalities hold
    \begin{equation}
        p_{11} \geq p_{11} - p^\prime_{10}p_{y_0}
    \end{equation}
    \begin{equation}
        \frac{(1 - x)y_0 + p_{11}x - p^\prime_{10}y_0}{x} \geq p_{11} - p^\prime_{10}y_0
    \end{equation}
    \begin{equation*}
        p_{11} - p_{y_0} \leq p_{11} - p^\prime_{10}y_0
    \end{equation*}    
    \begin{equation*}
        \frac{p_{11}p_x - p^\prime_{10}p_{y_0}}{p_x} \leq p_{11} - p^\prime_{10}y_0
    \end{equation*}    
\end{lemma}
\begin{proof}
    \item The upper bound is $\frac{p_{11}}{y_1}$: Assume
        \begin{align*}
            \frac{p_{11}}{y_1} &< \frac{p_{11} - p^\prime_{10}y_0}{y_1}\\
            \implies & 0 < -\frac{p^\prime_{10}y_0}{y_1}
        \end{align*}
        This is a contradiction, hence
        \[
            \frac{p_{11}}{y_1} \geq \frac{p_{11} - p^\prime_{10}y_0}{y_1}
        \]
        \item The upper bound is $\frac{(1 - x)y_0 + p_{11}x - p^\prime_{10}y_0}{x}$: Assume
        \begin{align*}
            \frac{p_{11} - p^\prime_{10}y_0}{y_1} &> \frac{(1 - x)y_0 + p_{11}x - p^\prime_{10}y_0}{xy_1}\\
            p_{11} - p^\prime_{10}y_0 &> \frac{(1 - x)y_0 + p_{11}x - p^\prime_{10}y_0}{x}\\
            p_{11}x - p^\prime_{10}xy_0 &> (1 - x)y_0 + p_{11}x - p^\prime_{10}y_0\\
            - p^\prime_{10}xy_0 &> (1 - x)y_0 - p^\prime_{10}y_0\\
            p^\prime_{10}y_0(1 - x) &> (1 - x)y_0 \\
            \implies p^\prime_{10} &> 1 \\
        \end{align*}
\end{proof}


This Lemma implies that  $\max\{0, \mathbb{P}(Z = 1 \mid X = 1, Y = 0) - \mathbb{P}(Z = 1 \mid X = 0, Y = 0)\}$ can be either zero or non-zero over the range of the free parameters. 

Now, we similarly examine the behavior of $\max \{0, \mathbb{P}(Z = 1 \mid X = 1, Y = i) - \mathbb{P}(Z = 1 \mid X = 0, Y = i)\}$.

\begin{lemma}
    The function $\max \{0, \mathbb{P}(Z = 1 \mid X = 1, Y = i) - \mathbb{P}(Z = 1 \mid X = 0, Y = i)\} \geq 0$ for $i \in \{1, \dots, N\}$ when
    \begin{equation*}
        p^\prime_{1i} \leq P(Z = 1 \mid X = 1, Y = 1)
    \end{equation*}
\end{lemma}

\begin{lemma}
    The following inequalities hold
    \begin{align*}
            1 &\geq p^\prime_{1i}\\
            \frac{p^\prime_{1i}}{p_x} &\geq p^\prime_{1i}\\
            0 &\leq p^\prime_{1i}\\
            \frac{p^\prime_{1i} - (1 - p_x)}{p_x} &\leq p^\prime_{1i}
    \end{align*}
\end{lemma}
This Lemma implies that  $\max\{0, \mathbb{P}(Z = 1 \mid X = 1, Y = i) - \mathbb{P}(Z = 1 \mid X = 0, Y = i)\}$ can be either zero or non-zero over the range of the free parameters.   
\subsection{Behavior of Upper Bound on PNS Under Special Conditions}

Here we analyze the behavior of the upper bound on the PNS in Theorem 1 under certain conditions, since these will be used in the proof of Theorem 1.

\begin{lemma}
    Given the upper bound in Theorem 2 on PNS, when $p_x > 1 - p_x$ and all $p^\prime_{1i} \geq p_x$ for $i \in \{0, \dots, N\}$ and , then 
    \[
    p_{00} < p_{11} - \sum_{i = 0}^N \Phi_i
    \]
\end{lemma}

\begin{proof}
    Since $p^\prime_{1i} \geq p_x$ for all $i$, then all the indicators will evaluate to $1$, as a result $p_{11} - \sum_{i = 0}^N \Phi_i$ will equal
    \begin{align*}
        &p_{11} - \sum_{i = 0}^N \frac{p_{y_i}(p^\prime_{1i} - p_x)}{1 - p_x}\\
        &\implies = \frac{p_{11}(1 - p_x) - \sum_{i = 0}^N p_{y_i}(p^\prime_{1i} - p_x)}{1 - p_x}\\
        &\implies = \frac{p_{11}(1 - p_x) - p_{11}p_x - p_{10}(1 - p_x) + p_x}{1 - p_x}\\
        &\implies = \frac{p_{11}(1 - p_x) - p_{11}p_x + p_{00}(1 - p_x) - (1 - p_x) + p_x}{1 - p_x}\\
        &\implies = p_{01}(\frac{p_x}{1 - p_x} - 1) + p_{00}\\
    \end{align*}
    And since $p_x > 1 - p_x$, this quantity will be greater than $p_{00}$.
\end{proof}

\begin{lemma}
    Given the upper bound in Theorem 2 on PNS, when $p_x > 1 - p_x$ and $p^\prime_{1i} \leq 1 - p_x$ for $i \in \{0, \dots, N\}$ and , then 
    \[
    p_{00} - \sum_{i = 0}^N \Theta_i> p_{11}
    \]
\end{lemma}

\begin{proof}
Since $p^\prime_{1i} \leq 1 - p_x$ for all $i$, then all the indicators will evaluate to $1$, as a result $p_{00} - \sum_{i = 0}^N \Theta_i$ will equal
\begin{align*}
    &p_{00} - \sum_{i = 0}^N \frac{p_{y_i}((1 - p_x) - p^\prime_{1i})}{1 - p_x}\\
    &\implies = \frac{p_{00}(1 - p_x) - (1 - p_x) + \sum_{i = 0}^N p_{y_i}p^\prime_{1i}}{1 - p_x}
    &\implies = \frac{-p_{10}(1 - p_x) + \sum_{i = 0}^N p_{y_i}p^\prime_{1i}}{1 - p_x}\\
    &\implies = \frac{p_{11}p_x}{1 - p_x}
\end{align*}
And since $p_x > 1 - p_x$, this concludes the proof.
\end{proof}
%%%%%%%%%%%%%%%%%%%%%%%%%%%%%%%%%%%%%%%%%%%%%%%%%%%%%%%%%%%%%%%%%%%%%%%%%%%%%%

\begin{lemma}
    Given the upper bound in Theorem 2 on PNS, when $p_x < 1 - p_x$ and all $p^\prime_{1i} \geq 1 - p_x$ for $i \in \{0, \dots, N\}$ and , then 
    \[
    p_{00} < p_{11} - \sum_{i = 0}^N \Phi_i
    \]
\end{lemma}

\begin{proof}
    Since $p^\prime_{1i} \geq 1 - p_x$ for all $i$, then all the indicators will evaluate to $1$, as a result $p_{11} - \sum_{i = 0}^N \Phi_i$ will equal
    \begin{align*}
        &p_{11} - \sum_{i = 0}^N \frac{p_{y_i}(p^\prime_{1i} - (1 - p_x))}{p_x}\\
        &\implies = \frac{p_{11}p_x - \sum_{i = 0}^N p_{y_i}(p^\prime_{1i} - (1 - p_x))}{p_x}\\
        &\implies = \frac{p_{11}p_x - p_{11}p_x - p_{10}(1 - p_x) + (1 - p_x)}{p_x}\\
        &\implies = \frac{p_{00}(1 - p_x)}{p_x}
    \end{align*}
    And since $p_x < 1 - p_x$, this quantity will be greater than $p_{00}$.
\end{proof}

\begin{lemma}
    Given the upper bound in Theorem 2 on PNS, when $p_x < 1 - p_x$ and $p^\prime_{1i} \leq p_x$ for $i \in \{0, \dots, N\}$ and , then 
    \[
    p_{00} - \sum_{i = 0}^N \Theta_i> p_{11}
    \]
\end{lemma}

\begin{proof}
Since $p^\prime_{1i} \leq p_x$ for all $i$, then all the indicators will evaluate to $1$, as a result $p_{00} - \sum_{i = 0}^N \Theta_i$ will equal
\begin{align*}
    &p_{00} - \sum_{i = 0}^N \frac{p_{y_i}(p_x - p^\prime_{1i})}{p_x}\\
    &\implies = \frac{p_{00}p_x - p_x + \sum_{i = 0}^N p_{y_i}p^\prime_{1i}}{p_x}\\
    &\implies = \frac{-p_{10}p_x + p_{10}(1 - p_x)}{p_x} + p_{11}\\
    &\implies = p_{10}(\frac{1 - p_x}{p_x} - 1) + p_{11}
\end{align*}
And since $1 - p_x > p_x$, the ineqality holds.
\end{proof}

\begin{lemma}
    Assume $p_x > 1 - p_x$. Assume all $1 - p_x < p^\prime_{1i} < p_x$. Then all max operators to can open simultaneously if and only if $\Phi_X \geq 0$. 
\end{lemma}

\begin{proof}
    To prove an if and only if, we first show that all max operators opening implies $p_{11} + p_{10} - 1 \geq 0$, and then the other way round. 

    Starting with the first, note that for all max operators to open simultaneously, the following conditions must hold
\begin{align*}
    \sum_{n = 1}^N p_{y_n}P(Z = 1 \mid X = 1, Y = n) \geq \frac{p_{y_0}((1 - p_x) - p^\prime_{10})}{p_x - (1 - p_x)} + p_{11}
\end{align*}
And for all $i \in \{1, \dots N\}$
\begin{align*}
    P(Z = 1 \mid X = 1, Y = i) \leq \frac{p^\prime_{1i} - (1 - p_x)}{p_x - (1 - p_x)}    
\end{align*}

This is equivalent to
\begin{align*}
    &\frac{p_{y_0}((1 - p_x) - p^\prime_{10})}{p_x - (1 - p_x)} + p_{11} \leq \sum_{i = 1}^N p_{y_i}\frac{p^\prime_{1i} - (1 - p_x)}{p_x - (1 - p_x)}\\
    &\implies p_{y_0}((1 - p_x) - p^\prime_{10}) + p_{11}(p_x - (1 - p_x)) +  \leq \sum_{i = 1}^N p_{y_i}(p^\prime_{1i} - (1 - p_x))\\
    &\implies (1 - p_x) + p_{11}(p_x - (1 - p_x)) +  \leq \sum_{i = 1}^N p_{y_i}p^\prime_{1i} + p^\prime_{10}p_{y_0}\\
    &\implies (1 - p_x) - p_{11}(1 - p_x) +  \leq p_{10}(1 - p_x)\\
    &\implies 0 \leq p_{11} + p_{10} - 1
\end{align*}

Next, to prove the backward implication, we utilize a proof by contrapositive, i.e. we must prove that .  
\[
\frac{p_{y_0}((1 - p_x) - p^\prime_{10})}{p_x - (1 - p_x)} + p_{11} > \sum_{i = 1}^N p_{y_i}\frac{p^\prime_{1i} - (1 - p_x)}{p_x - (1 - p_x)} \implies p_{11} + p_{10} - 1 < 0
\]

To see this, note that
\begin{align*}
    &\frac{p_{y_0}((1 - p_x) - p^\prime_{10})}{p_x - (1 - p_x)} + p_{11} > \sum_{i = 1}^N p_{y_i}\frac{p^\prime_{1i} - (1 - p_x)}{p_x - (1 - p_x)}\\
    &\implies p_{y_0}((1 - p_x) - p^\prime_{10}) + p_{11}(p_x - (1 - p_x)) > \sum_{i = 1}^N p_{y_i}(p^\prime_{1i} - (1 - p_x))\\
    &\implies (1 - p_x)  - p_{11}(1 - p_x) > p_{10}p_x\\
    &\implies 0  > p_{11} + p_{10} - 1
\end{align*}

\end{proof}

\begin{lemma}
    All max operators in $\Delta$ can open simultaneously if and only if $p_{11} - p_{10} \geq 0$. 
\end{lemma}

\begin{proof}
To prove an if and only if, we first show that all max operators opening implies $p_{11} - p_{10} \geq 0$, and then the other way round. 

Starting with the first, note that for all max operators to open simultaneously, the following conditions must hold
\begin{align*}
    p_{11} - p^\prime_{10}p_{y_0} \geq  \sum_{n = 1}^N p_{y_n}\mathbb{P}(Z = 1\mid X = 1, Y = n)
\end{align*}
And for all $i \in \{1, \dots N\}$
\begin{align*}
    P(Z = 1 \mid X = 1, Y = i) \geq p^\prime_{1i}
\end{align*}

This is equivalent to
\begin{align*}
    &\sum_{i = 1}^N p_{y_i}p^\prime_{1i} \leq p_{11} - p^\prime_{10}p_{y_0}\\
    &\implies \sum_{i = 0}^N p_{y_i}p^\prime_{1i} \leq p_{11} \\
    &\implies p_{11}p_x + p_{10}(1 - p_x) \leq p_{11} \\
    &\implies 0 \leq (1 - p_x)(p_{11} - p_{10})\\
\end{align*}

This proves the forward implication. A similar proof for the backward implication can be provided using a proof by contra positive as well, concluding the proof for this lemma. 
\end{proof}
% \begin{lemma}
%     Assume $p_x < 1 - p_x$. The functions $\max \{0, \mathbb{P}(Z = 1 \mid X = 1, Y = i) - \mathbb{P}(Z = 0 \mid X = 0, Y = i)\} \geq 0$ for $i \in \{1, \dots, N\}$ when
%     \begin{align*}
%             P(Z = 1 \mid X = 1, Y = i) \geq \frac{(1 - p_x) - p^\prime_{1i}}{(1 - p_x) - p_x}    
%     \end{align*}
% \end{lemma}


% % \begin{lemma}
% %     Assume $p_x > 1 - p_x$. If $p^\prime_{10} < x$, then 
% %     \[
% %     \frac{p_{11}x - p^\prime_{10}y_0}{x} < \frac{p_{y_0}((1 - p_x) - p^\prime_{10})}{p_x - (1 - p_x)} + p_{11}
% %     \]
% % \end{lemma}


% \begin{lemma}
%     Assume $p_x < 1 - p_x$. If $p^\prime_{10} \geq 1 - p_x$, then 
%     \[
%      \frac{(1 - p_x)p_{y_0} + p_{11}p_x - p^\prime_{10}p_{y_0}}{p_x} \leq \frac{p_{y_0}( p^\prime_{10} - (1 - p_x))}{(1 - p_x) - p_x} + p_{11}   
%     \]
% \end{lemma}

% \begin{lemma}
%     Assume $p_x < 1 - p_x$. If $p^\prime_{10} < 1 - p_x$, then 
%     \[
%     p_{11} > \frac{p_{y_0}( p^\prime_{10} - (1 - p_x))}{(1 - p_x) - p_x} + p_{11}
%     \]
% \end{lemma}

% \begin{lemma}
%     Assume $p_x < 1 - p_x$. If $p^\prime_{1i} \geq 1 - p_x$ for $i \in \{1, \dots , N\}$, then 
%     \begin{align*}
%             \frac{p^\prime_{1i} - (1 - p_x)}{p_x} \geq \frac{(1 - p_x) - p^\prime_{1i}}{(1 - p_x) - p_x}    
%     \end{align*}
% \end{lemma}

% \begin{lemma}
%     Assume $p_x < 1 - p_x$. If $p^\prime_{1i} < 1 - p_x$ for $i \in \{1, \dots , N\}$, then 
%     \begin{align*}
%             0 < \frac{(1 - p_x) - p^\prime_{1i}}{(1 - p_x) - p_x}       
%     \end{align*}
% \end{lemma}

% \begin{lemma}
%     Let $X$, $Z$ and $Y$ be binary random variables obeying the causal structure in \ref{fig:causal-graph}. Then, if the following conditions hold,
%     \begin{align*}
%         x &> 1 - x\\
%         p^\prime_{11} &\geq x\\
%         p^\prime_{10} &\geq x\\
%     \end{align*}
%     Then $\implies \Phi_X > 0$.
% \end{lemma}

% \begin{proof}
%     Since $P(Z, X)$ and $P(Z, Y)$ are marginals of $P(Z , X, Y)$, the following holds
%     \[
%     p_{11}x + p_{10}(1 - x) = p^\prime_{11}y_1 + p^\prime_{10}y_0
%     \]
%     Since $x > 1 - x$
%     \begin{align*}
%         \implies p_{11}x + p_{10}x > p^\prime_{11}y_1 + p^\prime_{10}y_0\\
%         \intertext{Since $p^\prime_{11} \geq x$ and $p^\prime_{11} \geq x$}
%         \implies p_{11}x + p_{10}x > xy_1 + xy_0\\
%         \implies p_{11}x + p_{10}x > x \implies p_{11} + p_{10} > 1\\
%         \implies \Phi_X > 0
%     \end{align*}
% \end{proof}

% \begin{lemma}
%     Let $X$, $Z$ and $Y$ be binary random variables obeying the causal structure in \ref{fig:causal-graph}. Then, if the following conditions hold,
%     \begin{align*}
%         1 - x &> x\\
%         p^\prime_{11} &\geq 1 - x\\
%         p^\prime_{10} &\geq 1 - x\\
%     \end{align*}
%     Then $\implies \Phi_X > 0$.
% \end{lemma}

% \begin{lemma}
%     Let $X$, $Z$ and $Y$ be binary random variables obeying the causal structure in \ref{fig:causal-graph}. Then, if the following conditions hold,
%     \begin{align*}
%         x &> 1 - x\\
%         p^\prime_{11} &\leq 1 - x\\
%         p^\prime_{10} &\leq 1 - x\\
%     \end{align*}
%     Then $\implies \Phi_X < 0$.
% \end{lemma}

% \begin{lemma}
%     Let $X$, $Z$ and $Y$ be binary random variables obeying the causal structure in \ref{fig:causal-graph}. Then, if the following conditions hold,
%     \begin{align*}
%         1 - x &> x\\
%         p^\prime_{11} &\leq x\\
%         p^\prime_{10} &\leq x\\
%         \implies& \Phi_X < 0
%     \end{align*}
% \end{lemma}

% \begin{lemma}\label{lem:a-leq-b}
%     Assume $x > 1 - x$. Denote $\Phi_X = p_{11} + p_{10} - 1$, and denote $a$ and $b$ as 
%     \begin{align*}
%             a &= \frac{y_0((1 - x) - p^\prime_{10})}{y_1(x - (1 - x))} + \frac{p_{11}}{y_1}\\
%             b &= \frac{p^\prime_{11} - (1 - x)}{x - (1 - x)}    
%     \end{align*}
%     Then, $\Phi_X \geq 0 \implies a \leq b$
% \end{lemma}

% \begin{lemma}\label{lem:a-geq-b}
%     Assume $x > 1 - x$. Denote $\Phi_X = p_{11} + p_{10} - 1$, and denote $a$ and $b$ as 
%     \begin{align*}
%             a &= \frac{y_0((1 - x) - p^\prime_{10})}{y_1(x - (1 - x))} + \frac{p_{11}}{y_1}\\
%             b &= \frac{p^\prime_{11} - (1 - x)}{x - (1 - x)}    
%     \end{align*}
%     Then, $\Phi_X < 0 \implies a > b$
% \end{lemma}

\subsection{Proof Of Upper Bound In Theorem 1}

According to Theorem 1, the upper bound is given as
\begin{align*}
    & PNS \leq \min\begin{bmatrix}
        p_{11} - \sum_{i = 0}^1\mathbb{I}(p^\prime_{1i} \geq \max\{1 - p_x, p_x\})\frac{p_{y_i}(p^\prime_{1i} - \max\{1 - p_x, p_x\})}{\min\{1 - p_x, p_x\}}\\
        p_{00} - \sum_{i = 0}^1\mathbb{I}(p^\prime_{1i} \leq \min\{1 - p_x, p_x\})\frac{p_{y_i}(\min\{1 - p_x, p_x\} - p^\prime_{1i})}{\min\{1 - p_x, p_x\}}\\
    \end{bmatrix}
\end{align*}
The upper bound is obtained by solving
\begin{align*}
    PNS \leq  \mathbb{P}(Z = 1 \mid X = 1) - \min_{P_i} \Gamma(P_i)
\end{align*}
We follow a proof by cases approach, and demonstrate on a case-by-case basis that $\mathbb{P}(Z = 1 \mid X = 1) - \min_{P_i} \Gamma(P_i)$ equals the bounds proposed in Theorem 1. 

Given binary $Y$, we can use Lemma \ref{lemma:RREF-y} and Lemma \ref{lem:free-param-bounds} to obtain the solutions for the joint distribution given the marginals, by constraining the following conditionals $P(Z = 1| X, Y)$ with respect to the free parameter $P(Z = 1 \mid X = 1, Y = 1)$.

{\small
\begin{align*}
\mathbb{P}(Z = 1 \mid X = 0, Y = 0) &=  \frac{p_x}{1 - p_x}\frac{p_{y_1}}{p_{y_0}}\mathbb{P}(Z = 1 \mid X = 1, Y = 1) + \frac{p^\prime_{10}p_{y_0} - p_{11}p_x}{(1 - p_x)p_{y_0}}\\
\mathbb{P}(Z = 1 \mid X = 1, Y = 0)&= \frac{p_{11}}{p_{y_0}} - \frac{p_{y_1}}{p_{y_0}}\mathbb{P}(Z = 1 \mid X = 1, Y = 1)\\
\mathbb{P}(Z = 1 \mid X = 0, Y = 1)&= \frac{p^\prime_{11}}{1 - p_x} - \frac{p_x}{1 - p_x}\mathbb{P}(Z = 1 \mid X = 1, Y = 1)
\end{align*}
}

And the following bounds on the free parameter $P(Z = 1 \mid X = 1, Y = 1)$ must hold

{\small
\begin{align}\label{equation:sum-bounds}
\max\begin{bmatrix}
   \frac{p_{11}p_x - p^\prime_{10}p_{y_0}}{p_x} \\
   p_{11} - p_{y_0}
\end{bmatrix} \leq y_1\mathbb{P}(Z = 1 \mid X = 1, Y = 1) 
\leq \min\begin{bmatrix}
    \frac{(1 - p_x)p_{y_0} + p_{11}p_x - p^\prime_{10}p_{y_0}}{p_x}\\
    p_{11}
\end{bmatrix}
\end{align}
}

Along with
\begin{align}
    \max\begin{bmatrix}\label{equation:individual-bounds}
        0\\
        \frac{p^\prime_{11} - (1 - p_x)}{p_x}
    \end{bmatrix}
        \leq P(Z = 1\mid X = 1, Y = 1) \leq 
    \min\begin{bmatrix}
        1\\
        \frac{p^\prime_{11}}{p_x}
    \end{bmatrix}
\end{align}
In the binary case, $\Gamma$ is expressed as
\begin{align*}
    \Gamma &= P(Y = 0)\max \{0, P(Z = 1 \mid X = 1, Y = 0) - P(Z = 0 \mid X = 0, Y = 0)\}\\
    &+ P(Y = 1)\max \{0, P(Z = 1 \mid X = 1, Y = 1) - P(Z = 0 \mid X = 0, Y = 1)\} 
\end{align*}

And based on Lemma \ref{lem:max-operator-expressions}, each of these terms in $\Gamma$ can be written as
\begin{enumerate}
    \item 
    \[P(Z = 1 \mid X = 1, Y = 0) - P(Z = 0 \mid X = 0, Y = 0)\]
    \begin{equation}\label{equation:binary-gamma-y0}
        \frac{p^\prime_{10} - (1 - p_x)}{1 - p_x} + \frac{p_{y_1}P(Z = 1 \mid X = 1, Y = 1) - p_{11}}{p_{y_0}}\Bigg(\frac{p_x}{1 - p_x} - 1\Bigg) 
    \end{equation}
    \item 
    \[
    P(Z = 1 \mid X = 1, Y = 1) - P(Z = 0 \mid X = 0, Y = 1)
    \]
    \begin{equation}\label{equation:binary-gamma-y1}
        P(Z = 1 \mid X = 1, Y = 1)(1 - \frac{p_x}{1 - p_x}) + \frac{p^\prime_{11} - (1 - p_x)}{1 - p_x}\\
    \end{equation}
\end{enumerate}
\subsubsection{$p_x = 1 - p_x$}

In this setting, we will prove the following equations hold 
\begin{equation}\label{equation:upper-bound-1}
p_{11} - \min_{P_i} \Gamma(P_i) = p_{11} - \sum_{i = 0}^1\mathbb{I}(p^\prime_{1i} \geq \max\{1 - p_x, p_x\})\frac{p_{y_i}(p^\prime_{1i} - \max\{1 - p_x, p_x\})}{\min\{1 - p_x, p_x\}}    
\end{equation}
And
\begin{equation}\label{equation:upper-bound-2}
p_{11} - \min_{P_i} \Gamma(P_i) = p_{00} - \sum_{i = 0}^N\mathbb{I}(p^\prime_{1i} \leq \min\{1 - p_x, p_x\})\frac{p_{y_i}(\min\{1 - p_x, p_x\} - p^\prime_{1i})}{\min\{1 - p_x, p_x\}}    
\end{equation}
Note that when $p_x = 1 - p_x$, $\Gamma$ is no longer a function of $P(Z = 1 \mid X = 1, Y = 1)$ since \ref{equation:binary-gamma-y0} and \ref{equation:binary-gamma-y1} are no longer a function of $P(Z = 1 \mid X = 1, Y = 1)$. $\Gamma$ will equal
\begin{align*}
    \Gamma = p_{y_0}\max \{0, \frac{p^\prime_{10} - (1 - p_x)}{1 - p_x} \}
    + p_{y_1}\max \{0,  \frac{p^\prime_{11} - (1 - p_x)}{1 - p_x}\} 
\end{align*}
And the upper bound on PNS will equal
\begin{align*}
    p_{11} - \Gamma
\end{align*}
Next, we show on a case by case basis that $p_{11} - \Gamma$ will always equal both \ref{equation:upper-bound-1} and \ref{equation:upper-bound-2}. We provide the proof for one case, and the rest of the cases can be proved in a similar fashion.\\
\textbf{Case I}: $p^\prime_{10} \geq 1 - p_x$ and $p^\prime_{11} \geq 1 - p_x$: $\Gamma$ will equal
    \begin{align*}
        \Gamma &= \frac{p_{y_0}p^\prime_{10} - p_{y_0}(1 - p_x)}{1 - p_x} + \frac{p_{y_1}p^\prime_{11} - p_{y_1}(1 - p_x)}{1 - p_x}\\
        \implies p_{11} - \Gamma &= p_{11} - \frac{p_{y_0}p^\prime_{10} - p_{y_0}(1 - p_x)}{1 - p_x} - \frac{p_{y_1}p^\prime_{11} - p_{y_1}(1 - p_x)}{1 - p_x}
    \end{align*}
    By direct comparison, this is equal to \ref{equation:upper-bound-1}. Next, to prove the equality to \ref{equation:upper-bound-2}, note that
    \begin{align*}
        &p_{11} - \frac{p_{y_0}p^\prime_{10} - p_{y_0}(1 - p_x)}{1 - p_x} - \frac{p_{y_1}p^\prime_{11} - p_{y_1}(1 - p_x)}{1 - p_x}\\
        \intertext{Since $p_x = 1 - p_x$}
        &\implies = \frac{p_{11}p_x - p_{y_0}p^\prime_{10} + p_{y_0}(1 - p_x) - p_{y_1}p^\prime_{11} + p_{y_1}(1 - p_x)}{1 - p_x}\\
        &= \frac{-p_{10}(1 - p_x) + (1 - p_x)}{1 - p_x}\\
        &= p_{00}
    \end{align*}
    And by comparison to \ref{equation:upper-bound-2}, we can see these are equal as well.
This proves that in the case $x = 1 - x$, $p_{11} - \Gamma$ will equal \ref{equation:upper-bound-1} and \ref{equation:upper-bound-2}. Now, we move on to the scenario where $p_x > 1 - p_x$.
\subsubsection{$p_x > 1 - p_x$} 

Here we follow a similar proof by cases as well, with each case being defined by relation of $p^\prime_{10}$ and $p^\prime_{11}$ to $p_x$ and $1 - p_x$. \\
Note that since $p_x > 1 - p_x$, $\max \{0, \mathbb{P}(Z = 1 \mid X = 1, Y = 0) - \mathbb{P}(Z = 0 \mid X = 0, Y = 0)\}$ is an increasing function of the free parameter, while $\max \{0, \mathbb{P}(Z = 1 \mid X = 1, Y = i) - \mathbb{P}(Z = 0 \mid X = 0, Y = i)\}$ is a decreasing function of the free parameter.\\
\newline
\textbf{Case I}
Consider the following case
\begin{align*}
    p_x &\leq p^\prime_{10}\\
    p_x &\leq p^\prime_{11}\\
\end{align*}
Since $p^\prime_{10} \geq \max\{p_x, 1 - p_x\}$, and the same for $p^\prime_{11}$, the following hold

\begin{align*}
    &\max \{0, \mathbb{P}(Z = 1 \mid X = 1, Y = 0) - \mathbb{P}(Z = 0 \mid X = 0, Y = 0)\}\\
    &= \mathbb{P}(Z = 1 \mid X = 1, Y = 0) - \mathbb{P}(Z = 0 \mid X = 0, Y = 0)
\end{align*}

As well as 
\begin{align*}
    &\max \{0, \mathbb{P}(Z = 1 \mid X = 1, Y = 1) - \mathbb{P}(Z = 0 \mid X = 0, Y = 1)\}\\
    &= \mathbb{P}(Z = 1 \mid X = 1, Y = 1) - \mathbb{P}(Z = 0 \mid X = 0, Y = 1)
\end{align*}

And since $\Gamma$ is equal to their weighted sum, $\Gamma = \Phi_X$. Hence
\[
p_{11} - \Gamma = p_{00}
\]

And based on Lemma XXX (prove this later), this will equal the result in Theorem 1.\\
\newline
\textbf{Case II}
Consider the following case
\begin{align*}
    p^\prime_{10} \leq 1 - p_x \\
    p^\prime_{11} \leq 1 - p_x \\
\end{align*}
Based on Lemma XXX and Lemma XXXX, both max operators will equal $0$ over the entire range of the free parameter. Hence $\Gamma = 0$, and the bound is $p_{11}$.\\
\newline
\textbf{Case III}
Consider the following case
\begin{align*}
    p_x &\leq p^\prime_{10}\\
    p^\prime_{11} &\leq 1 - p_x\\
\end{align*}

Based on Lemma XXX, since $p^\prime_{1i} \leq \min\{p_x, 1 - p_x\}$, $\max \{0, \mathbb{P}(Z = 1 \mid X = 1, Y = i) - \mathbb{P}(Z = 0 \mid X = 0, Y = i)\} = 0$ over the entire range of the free parameter. However, since $p^\prime_{10} \geq \max\{p_x, 1 - p_x\}$, $\max \{0, \mathbb{P}(Z = 1 \mid X = 1, Y = 0) - \mathbb{P}(Z = 0 \mid X = 0, Y = 0)\} \geq 0$. 

Consequently, finding the $\min \Gamma$ comes down to solving
\[
\min \max \{0, \mathbb{P}(Z = 1 \mid X = 1, Y = 0) - \mathbb{P}(Z = 0 \mid X = 0, Y = 0)\}
\]
Since we have proved that both lower bounds are large enough to ensure $ \max \{0, \mathbb{P}(Z = 1 \mid X = 1, Y = 0) - \mathbb{P}(Z = 0 \mid X = 0, Y = 0)\} \geq 0$, this is written as $\min \mathbb{P}(Z = 1 \mid X = 1, Y = 0) - \mathbb{P}(Z = 0 \mid X = 0, Y = 0)$. This is an increasing function of the free parameter, and the minimum will be attained at the lower bound of the free parameter, which will be $\max\{0, p_{11} - p_{y_0}\}$.

Substituting both values of the free parameter into $\mathbb{P}(Z = 1 \mid X = 1, Y = 0) - \mathbb{P}(Z = 0 \mid X = 0, Y = 0)$, 
\begin{align*}
    \Gamma = \min \mathbb{P}(Z = 1 \mid X = 1, Y = 0) - \mathbb{P}(Z = 0 \mid X = 0, Y = 0) \\ 
    = \max\{\frac{p_{y_0}(p^\prime_{10} - p_x)}{1 - p_x}, \Phi_x + \frac{p_{y_1}((1 - p_x) - p^\prime_{11})}{1 - p_x} \}
\end{align*}

And since the upper bound is $p_{11} - \Gamma$, then 
\begin{align*}
    &p_{11} - \max\{\frac{p_{y_0}(p^\prime_{10} - p_x)}{1 - p_x}, \Phi_x + \frac{p_{y_1}((1 - p_x) - p^\prime_{11})}{1 - p_x} \}\\
    &= \min\{p_{11} - \frac{p_{y_0}(p^\prime_{10} - p_x)}{1 - p_x}, p_{00} - \frac{p_{y_1}((1 - p_x) - p^\prime_{11})}{1 - p_x}\} 
\end{align*}

This aligns with the bounds in Theorem 1.\\
\newline
\textbf{Case IV}
Consider the following case
\begin{align*}
    1 - p_x &< p_x \leq p^\prime_{10}\\
    1 - p_x &< p^\prime_{11} < p_x\\
\end{align*}
Based on Lemma XXX and Lemma XXX, $\max \{0, \mathbb{P}(Z = 1 \mid X = 1, Y = 0) - \mathbb{P}(Z = 0 \mid X = 0, Y = 0) \}= \mathbb{P}(Z = 1 \mid X = 1, Y = 0) - \mathbb{P}(Z = 0 \mid X = 0, Y = 0)$ over the entire range of free parameters. However, $\max \{0, \mathbb{P}(Z = 1 \mid X = 1, Y = 0) - \mathbb{P}(Z = 0 \mid X = 0, Y = 0) \}$ may be zero or non-zero, and depending on the bounds on the free parameter. If the bounds on the free parameter allow $\max \{0, \mathbb{P}(Z = 1 \mid X = 1, Y = 1) - \mathbb{P}(Z = 0 \mid X = 0, Y = 1) \}$ to be $0$ or non-zero, then $\min \Gamma$ would be attained at the lower bound of the free parameter, since increasing the value of the free parameter increases the value of $\max \{0, \mathbb{P}(Z = 1 \mid X = 1, Y = 0) - \mathbb{P}(Z = 0 \mid X = 0, Y = 0) \}$, and once as long as $\max \{0, \mathbb{P}(Z = 1 \mid X = 1, Y = 1) - \mathbb{P}(Z = 0 \mid X = 0, Y = 1) \}$ is also non-zero their weighted sum will evaluate to the constant $p_{11} + p_{10} - 1$. However, as the value of the free parameter increases, $\max \{0, \mathbb{P}(Z = 1 \mid X = 1, Y = 1) - \mathbb{P}(Z = 0 \mid X = 0, Y = 1) \} = 0$ while increasing the value of the other max operator. Since the lower bound is maximum of the two lower bounds implied by the bounds, it becomes equivalent to choosing between $\min \Gamma = \max\{p_{11} + p_{10} - 1, p_{11} - \frac{p_{y_0}(p^\prime_{10} - p_x)}{1 - p_x}\}$, and hence $p_{11} - \max\{p_{11} + p_{10} - 1, \frac{p_{y_0}(p^\prime_{10} - p_x)}{1 - p_x}\}$ will equal
\[
\min\{p_{00}, p_{11} - \frac{p_{y_0}(p^\prime_{10} - p_x)}{1 - p_x}
\]
And this matches the bounds proposed in Theorem 1.\\
\newline
\textbf{Case V}
Consider the following case
\begin{align*}
    1 - p_x &< p^\prime_{10} < p_x\\
    1 - p_x &< p^\prime_{11} < p_x\\
\end{align*}

Based on Lemma XX and XX, both max operators in $\Gamma$ can be non-zero or zero over the range of the free parameters. 

Based on Lemma XXX, when the range of the free parameters allow both max operators to simultaneously equal open with non-zero terms, then $\Gamma = p_{11} + p_{10} - 1$. And deviation away from this state would be greater than $p_{11} + p_{10} - 1$ since this would allow either max operator to increase while the other max operator that counterbalanced this increase before will evaluate to $0$, making their sum greater than $p_{11} + p_{10} - 1$.  

Next, consider the case XX, when both max operators cannot simultaneously open as non-zero terms. Based on Lemma XX, the bounds on $P(Z = 1 \mid X = 1, Y = 1)$ are
\[max
\begin{bmatrix}
    \frac{p^\prime_{11} - (1 - p_x)}{p_x}\\
    \frac{p^\prime_{11}p_{y_1} - p_{10}(1 - p_x)}{p_xp_{y_1}}
\end{bmatrix} \leq P(Z = 1 \mid X = 1, Y = 1) \leq 
min\begin{bmatrix}
   \frac{p^\prime_{11}}{x}\\
   \frac{(1 - x)(1 - y) - p_{10}(1 - x) + p^\prime_{11}y}{xy}
\end{bmatrix}
\]

Now, we check whether the lower bounds are greater than (b) and if the upper bounds are less than (a).
\begin{enumerate}
    \item First, $\frac{p^\prime_{11} - (1 - x)}{x} < \frac{p^\prime_{11} - (1 - x)}{2x - 1}$ since the denominator is smaller on the right hand side. This lower bound is less than (a), and will consequently be less than (b). 
    \item Checking the lower bound of $\frac{p^\prime_{11}y - p_{10}(1 - x)}{xy}$ against (b), using a proof by contradiction. Assume,
    \[ \frac{p^\prime_{11}y - p_{10}(1 - x)}{xy} > 
        \frac{p^\prime_{11}y - (1 - x)(p_{11} + p_{10} - 1) - y(1 - x)}{y(x - (1 - x))}
    \]

Checking the right hand side of the implication
\begin{align*}
    &\implies p^\prime_{11}y(x - (1 - x)) - p_{10}(1 - x)(x - (1 - x)) > p^\prime_{11}xy - x(1 - x)(p_{11} + p_{10} - 1) -xy(1 - x)\\
    &\implies -p^\prime_{11}y - p_{10}(x - (1 - x)) >  - x(p_{11} + p_{10} - 1) -xy\\
    &\implies -p^\prime_{11}y + p_{10}(1 - x) - p_{10}x  >  - xp_{11} - xp_{10} + x -xy\\
    &\implies -p^\prime_{11}y + p_{10}(1 - x) + xp_{11}  >  x(1 - y)\\
    &\implies p^\prime_{10}(1 - y) > x(1 - y) \implies p^\prime_{10} > x
\end{align*}

This is a contradiction based on the case we are in. So,
    \[
        \frac{p^\prime_{11}y - p_{10}(1 - x)}{xy} \leq 
        \frac{p^\prime_{11}y - (1 - x)(p_{11} + p_{10} - 1) - y(1 - x)}{y(x - (1 - x))}
    \]
\end{enumerate}

Checking the upper bounds now. 

\begin{enumerate}
    \item When the upper bound is $\frac{p^\prime_{11}}{x}$: Checking this against the (a).
    \begin{align*}
    \frac{p^\prime_{11}}{x} < \frac{p^\prime_{11} - (1 - x)}{x - (1 - x)}
    \implies p^\prime_{11}x - p^\prime_{11}(1 - x) < p^\prime_{11}x - x(1 - x)\\
    \implies p^\prime_{11} > x
    \end{align*}
    This is a contradiction because of the case we are in. So
    \[
    \frac{p^\prime_{11}}{x} \geq \frac{p^\prime_{11} - (1 - x)}{x - (1 - x)}
    \]
    \item When the upper bound is $\frac{(1 - x)(1 - y) - p_{10}(1 - x) + p^\prime_{11}y}{xy}$: Assume
    \[
    \frac{(1 - x)(1 - y) - p_{10}(1 - x) + p^\prime_{11}y}{xy} < \frac{p^\prime_{11} - (1 - x)}{x - (1 - x)}
    \]
    \begin{align*}
      &\implies (1 - x)(1 - y)(x - (1 - x)) - p_{10}(1 - x)(x - (1 - x)) + p^\prime_{11}y(x - (1 - x)) < p^\prime_{11}xy - xy(1 - x)\\
      &\implies (1 - x)(1 - y)(x - (1 - x)) - p_{10}(1 - x)(x - (1 - x)) -p^\prime_{11}y(1 - x) < - xy(1 - x)\\
      &\implies (1 - y)(x - (1 - x)) - p_{10}(x - (1 - x)) -p^\prime_{11}y < - xy\\
      &\implies x - xy - (1 - y)(1 - x) - p_{10}(x - (1 - x)) -p^\prime_{11}y < - xy\\
      &\implies x - (1 - y)(1 - x) - p_{10}(x - (1 - x)) -p^\prime_{11}y < 0\\
      &\implies x - p_{10}x - (1 - y)(1 - x) + p_{10}(1 - x) -p^\prime_{11}y < 0\\
      &\implies x - p_{10}x - (1 - y)(1 - x) + p^\prime_{10}(1 - y) - p_{11}x < 0\\
      &\implies x(1 - p_{10} - p_{11}) - (1 - y)(1 - x) + p^\prime_{10}(1 - y)  < 0\\
      &\implies  (1 - y)(p^\prime_{10} - (1 - x))  < x(p_{11} + p_{10} - 1)\\
    \end{align*}
This creates a contradiction since the LHS is positive but the RHS is negative.

So, no falsification in this case. So,

    \[
    \frac{(1 - x)(1 - y) - p_{10}(1 - x) + p^\prime_{11}y}{xy} \geq \frac{p^\prime_{11} - (1 - x)}{x - (1 - x)}
    \]
\end{enumerate}


This shows that there will always be a region of the space of the free parameter where both max operators will evaluate to $0$, making this the minimum. 


% In Lemma XXXX, we showed that $p_{11} - p_{y_0}$ will make $\max\{0, P(Z = 1 \mid X = 1, Y = 0) - P(Z = 1 \mid X = 0, Y = 0)\} = 0$. If $\frac{p_{11} - p_{y_0}}{p_{y_1}}$ is the lower bound on the free parameter, 

% In the case where both max operators cannot simultaneously be $0$, there exists a region of the free parameter where both max operators open as non-zero terms, and will make $\Gamma$ evaluate to $p_{11} + p_{10} - 1$. 

Hence, $\Gamma$ will equal $0$ or  depending on whether the free parameter allows both max operators to be zero simultaneously or not. Based on Lemma XXX, this is determined by $p_{11} + p_{10} - 1 \geq 0$. Hence the bounds will be
\[
p_{11} - \max\{0, p_{11} + p_{10} - 1\} = \min\{p_{11}, p_{00}\}
\]
Similar approaches can be used for the rest of the cases, as well as for the case when $p_x < 1 - p_x$. 

\subsection{Proof Of Lower Bound In Theorem 1}

Based on Lemma XX, every term in $\Delta$ can be expressed in terms of the free parameter as

\begin{enumerate}
    \item $\mathbb{P}(Z = 1 \mid X = 1, Y = 0) - \mathbb{P}(Z = 1 \mid X = 0, Y = 0)$
    \begin{equation}\label{eq:delta-max-operator-y0}
    \frac{p_{11} - p^\prime_{10}p_{y_0} - p_{y_1}\mathbb{P}(Z = 1\mid X = 1, Y = 1)}{(1 - p_x)p_{y_0}}
\end{equation} 

\item $\mathbb{P}(Z = 1 \mid X = 1, Y = 1) - \mathbb{P}(Z = 1 \mid X = 0, Y = 1)$
    \begin{equation}\label{eq:delta-max-operator-y1}
        \frac{\mathbb{P}(Z = 1 \mid X = 1, Y = 1) - p^\prime_{11}}{1 - p_x}
    \end{equation}
\end{enumerate}

First, consider the case when both max operators can open with non-zero terms at the same time, i.e. $p^\prime_{11} < P(Z = 1 \mid X = 1, Y = 1) < \frac{p_{11} - p^\prime_{10}y_0}{y_1}$, which based on Lemma XXXX, happens when $p_{11} - p_{10} > 0$. In this case, $\Delta$ is minimized for values of the free parameter when all the max operators are non-zero. 

This can be seen on a case by case basis, where we first examine how to decrease Eq. \ref{eq:delta-max-operator-y0}. This would be accomplished by increasing the value of $P(Z = 1 \mid X = 1, Y = 1)$, however, this also increases the value of Eq. \ref{eq:delta-max-operator-y1}. Since their weighted sum is a constant, it means that the increase of one counterbalances the decrease in another, however, after a certain point since the max operator corresponding to Eq. \ref{eq:delta-max-operator-y0} starts evaluating to $0$, this increase is no longer counterbalanced, leading to Eq. \ref{eq:delta-max-operator-y1} taking on a value greater than $p_{11} - p_{10}$ (the value of the sum of both max operators). 

Next, consider the case when $p_{11} - p_{10} \leq 0$, based on Lemma XXX, both max operators cannot open with non-zero terms at the same time. First we check whether any lower bounds are large enough to make $P(Z = 1 \mid X = 1, Y = 1) - p^\prime_{11} > 0$. 

We utilize a proof by contradiction to show each of the lower bounds cannot be greater than $p^\prime_{11}$. When the lower bound is $0$ or $\frac{p^\prime_{11} - (1 - p_x)}{p_x}$, from Lemma XX we have seen there are not large enough to make $\max\{0, P(Z = 1 \mid X = 1, Y = 1)\}$ equal to a non-zero value. We now check the remaining possibilities for lower bounds. 
    \begin{enumerate}
        \item If the lower bound is $\frac{p_{11} - y_0}{y_1}$: Assume
        \begin{align*}
            \frac{p_{11} - y_0}{y_1} &> p^\prime_{11}\\
            \implies (1 - x)(p_{11} - p_{10}) > y_0p^\prime_{00}
        \end{align*}
        This is a contradiction since $p_{11} - p_{10} \leq 0$, hence 
        \[
            \frac{p_{11} - y_0}{y_1} \leq p^\prime_{11}
        \]
        \item The lower bound is $\frac{p_{11}x - p^\prime_{10}y_0}{xy_1}$: Assume 
        \begin{align*}
            \frac{p_{11}x - p^\prime_{10}y_0}{xy_1} &> p^\prime_{11}\\
            \implies p_{11} - p_{10} > p^\prime_{10}y_0
        \end{align*}
        And this is a contradiction as well for the same reasons as before, hence
        \[
            \frac{p_{11}x - p^\prime_{10}y_0}{xy_1} \leq p^\prime_{11}\\
        \]
    \end{enumerate}
Hence, we have shown the lower bounds are always going to allow $\max\{0, P(Z = 1 \mid X = 1, Y = 1)\}$ to take on the value of $0$. Next, checking whether the upper bound restrict the range of $\max\{0, \frac{p_{11} - p^\prime_{10}y_0 - y_1\mathbb{P}(Z = 1\mid X = 1, Y = 1)}{(1 - x)y_0}\}$. 
    
From Lemma XXX, this requires $P(Z = 1 \mid X = 1, Y = 1) < \frac{p_{11} - p^\prime_{10}y_0}{y_1}$. Following a similar argument as before, we need the upper bound on $P(Z = 1 \mid X = 1, Y = 1)$ to be less than $\frac{p_{11} - p^\prime_{10}y_0}{y_1}$. From Lemma XXX, $\frac{p_{11}}{y_1}$ and $\frac{(1 - x)y_0 + p_{11}x - p^\prime_{10}y_0}{x}$ are greater, so we prove the remaining bounds.
    \begin{enumerate}
        \item The upper bound is $1$: Assume
        \begin{align*}
            1 &< \frac{p_{11} - p^\prime_{10}y_0}{y_1}\\
            y_1 &< p_{11} - p_{11}x - p_{10}(1 - x) + p^\prime_{11}y_1\\
            \implies& y_1p^\prime_{01} < (1 - x)(p_{11} - p_{10})
        \end{align*}
        This is a contradiction as well, hence
        \[
        1 \geq \frac{p_{11} - p^\prime_{10}y_0}{y_1}
        \]
        \item The upper bound is $\frac{p^\prime_{11}}{x}$: Assume
        \begin{align*}
            \frac{p^\prime_{11}}{x} &< \frac{p_{11} - p^\prime_{10}y_0}{y_1}\\
            \implies& (1 - x)p^\prime_{11}y_1 < (1 - x)(p_{11} - p_{10})
        \end{align*}
        This is a contradiction, hence 
        \[
            \frac{p^\prime_{11}}{x} \geq \frac{p_{11} - p^\prime_{10}y_0}{y_1}
        \]
\end{enumerate}

Since we have shown that the lower bound of $P(Z = 1\mid X = 1, Y = 1)$ is always less than $p^\prime_{11}$ and the upper bound is always greater than $\frac{p_{11} - p^\prime_{10}y_0}{y_1}$, there will always be a value of $P(Z = 1\mid X = 1, Y = 1)$ allowed such that both max operators open as $0$. 

So we have shown that when $p_{11} - p_{10} > 0$, $\Delta$ will evaluate to $p_{11} - p_{10}$, and $0$ otherwise. This concludes the proof of the lower bound. 

\section{Proof of Theorem 2}

The proof for this Theorem follows a similar proof for the proof of Theorem 1, and we prove the lower bounds and upper bounds separately. 

Based on Lemma \ref{lem:free-param-bounds}, the following bounds hold for the free parameters. 
{\small
\begin{align}
\max\begin{bmatrix}
   \frac{p_{11}p_x - p^\prime_{10}p_{y_0}}{p_x} \\
   p_{11} - p_{y_0}
\end{bmatrix} \leq \sum_{n = 1}^N y_n\mathbb{P}(Z = 1 \mid X = 1, Y = n) 
\leq \min\begin{bmatrix}
    \frac{(1 - p_x)p_{y_0} + p_{11}p_x - p^\prime_{10}y_0}{p_x}\\
    p_{11}
\end{bmatrix}
\end{align}
}

And for each $i \in \{1, \dots, N\}$, we the bounds on the following free parameters $P(Z = 1\mid X = 1, Y = i)$
\begin{align}\label{eq:individual-bounds}
    \max\begin{bmatrix}
        0\\
        \frac{p^\prime_{1i} - (1 - x)}{x}
    \end{bmatrix}
        \leq P(Z = 1\mid X = 1, Y = i) \leq 
    \min\begin{bmatrix}
        1\\
        \frac{p^\prime_{1i}}{x}
    \end{bmatrix}
\end{align}

\subsection{Proof for Upper Bound in Theorem 2}
In the binary case, $\Gamma$ is expressed as
\begin{equation}\label{eq:arbitrary-y-gamma}
    \Gamma &= \sum_{y}P(Y = y)\max \{0, P(Z = 1 \mid X = 1, Y = y) - P(Z = 0 \mid X = 0, Y = y)\}
\end{equation}

And based on Lemma \ref{lem:max-operator-expressions}, each of these terms in $\Gamma$ can be written as
\begin{enumerate}
    \item 
    \[P(Z = 1 \mid X = 1, Y = 0) - P(Z = 0 \mid X = 0, Y = 0)\]
    \begin{equation}\label{equation:arbitrary-gamma-y0}
        \frac{p^\prime_{10} - (1 - p_x)}{1 - p_x} + \frac{p_{y_1}P(Z = 1 \mid X = 1, Y = 1) - p_{11}}{p_{y_0}}\Bigg(\frac{p_x}{1 - p_x} - 1\Bigg) 
    \end{equation}
    \item 
    \[
    P(Z = 1 \mid X = 1, Y = 1) - P(Z = 0 \mid X = 0, Y = 1)
    \]
    \begin{equation}\label{equation:arbitrary-gamma-yi}
        P(Z = 1 \mid X = 1, Y = 1)(1 - \frac{p_x}{1 - p_x}) + \frac{p^\prime_{11} - (1 - p_x)}{1 - p_x}\\
    \end{equation}
\end{enumerate}

\subsubsection{$p_x = 1 - p_x$}

In this setting, we will prove the following equations hold 
\begin{equation}\label{eq:arbitrary-y-upper-bound-1}
p_{11} - \min_{P_i} \Gamma(P_i) = p_{11} - \sum_{i = 0}^N\mathbb{I}(p^\prime_{1i} \geq \max\{1 - p_x, p_x\})\frac{p_{y_i}(p^\prime_{1i} - \max\{1 - p_x, p_x\})}{\min\{1 - p_x, p_x\}}    
\end{equation}
And
\begin{equation}\label{equation:arbitrary-y-upper-bound-2}
p_{11} - \min_{P_i} \Gamma(P_i) = p_{00} - \sum_{i = 0}^N\mathbb{I}(p^\prime_{1i} \leq \min\{1 - p_x, p_x\})\frac{p_{y_i}(\min\{1 - p_x, p_x\} - p^\prime_{1i})}{\min\{1 - p_x, p_x\}}    
\end{equation}
Note that when $p_x = 1 - p_x$, $\Gamma$ is no longer a function of $P(Z = 1 \mid X = 1, Y = 1)$ since \ref{equation:arbitrary-gamma-y0} and \ref{equation:arbitrary-gamma-yi} are no longer a function of $P(Z = 1 \mid X = 1, Y = 1)$. $\Gamma$ will equal
\begin{align*}
    \Gamma = \sum_{i = 0}^N p_{y_i}\max \{0, \frac{p^\prime_{1i} - (1 - p_x)}{1 - p_x} \}
\end{align*}
Next, we show on a case by case basis that $p_{11} - \Gamma$ will always equal both \ref{eq:arbitrary-y-upper-bound-1} and \ref{equation:arbitrary-y-upper-bound-2}. Partition the set $\{0, \dots, N\}$ into two disjoint subsets $R$ and $L$ such that $\forall i \in R$, $p^\prime_{1i} \geq p_x$, $\forall j \in L$, $p^\prime_{1j} \leq p_x$. Then, $p_{11} - \Gamma$ will evaluate to
\begin{equation}\label{eq:equal-x-part-a}
    p_{11} - \Gamma = p_{11} - \sum_{r \in R} p_{y_r}\frac{p^\prime_{1r} - (1 - p_x)}{1 - p_x}
\end{equation}
By direct comparison, this is equal to Eq. \ref{eq:arbitrary-y-upper-bound-1}. Next, since $p_x = 1 - p_x$ Eq. \ref{eq:equal-x-part-a} can be written as
\begin{align*}
    &\frac{p_{11}p_x - \sum_{r \in R} p_{y_r}(p^\prime_{1r} - (1 - p_x))}{1 - p_x}
\intertext{Using the identity $p_{11}p_x + p_{10}(1 - p_x) = \sum_{i = 0}^N p^\prime_{1i}p_{y_i}$}
&\implies = \frac{- p_{10}(1 - p_x) + \sum_{l \in L} p_{y_l}p^\prime_{1l} + (1 - \sum_{l \in L}p_{y_l})(1 - p_x)}{1 - p_x}\\
&\implies = p_{00} - \sum_{l \in L} \frac{p_{y_l}((1 - p_x) - p^\prime_{1l})}{1 - p_x}
\end{align*}
% We provide the proof for one case, and the rest of the cases can be proved in a similar fashion.\\
% \textbf{Case I}: $p^\prime_{10} \geq 1 - p_x$ and $p^\prime_{11} \geq 1 - p_x$: $\Gamma$ will equal
%     \begin{align*}
%         \Gamma &= \frac{p_{y_0}p^\prime_{10} - p_{y_0}(1 - p_x)}{1 - p_x} + \frac{p_{y_1}p^\prime_{11} - p_{y_1}(1 - p_x)}{1 - p_x}\\
%         \implies p_{11} - \Gamma &= p_{11} - \frac{p_{y_0}p^\prime_{10} - p_{y_0}(1 - p_x)}{1 - p_x} - \frac{p_{y_1}p^\prime_{11} - p_{y_1}(1 - p_x)}{1 - p_x}
%     \end{align*}
%     By direct comparison, this is equal to \ref{equation:upper-bound-1}. Next, to prove the equality to \ref{equation:upper-bound-2}, note that
%     \begin{align*}
%         &p_{11} - \frac{p_{y_0}p^\prime_{10} - p_{y_0}(1 - p_x)}{1 - p_x} - \frac{p_{y_1}p^\prime_{11} - p_{y_1}(1 - p_x)}{1 - p_x}\\
%         \intertext{Since $p_x = 1 - p_x$}
%         &\implies = \frac{p_{11}p_x - p_{y_0}p^\prime_{10} + p_{y_0}(1 - p_x) - p_{y_1}p^\prime_{11} + p_{y_1}(1 - p_x)}{1 - p_x}\\
%         &= \frac{-p_{10}(1 - p_x) + (1 - p_x)}{1 - p_x}\\
%         &= p_{00}
%     \end{align*}
And by comparison to \ref{equation:upper-bound-2}, we can see these are equal as well.
This proves that in the case $x = 1 - x$, $p_{11} - \Gamma$ will equal \ref{equation:upper-bound-1} and \ref{equation:upper-bound-2}. Now, we move on to the scenario where $p_x > 1 - p_x$.

\subsection{$p_x > 1 - p_x$}

We prove the bounds when $p_x > 1 - p_x$ in the following cases.\\
\textbf{Case I}: 
Consider the following case. $p^\prime_{10} \leq \min{p_x, 1 - p_x}$. Partition $\{1, \dots N\}$ into three disjoint subsets $L$, $R$ and $S$ such that $\forall l \in L \; p^\prime_{1l} \leq \min\{p_x, 1 - p_x\}$,  $\forall r \in R \; p^\prime_{1r} \geq \max\{p_x, 1 - p_x\}$,  and $\forall s \in S \; 1 - p_x < p^\prime_{1s} < p_x$. 

Then, from Lemma XXX and XXXX, $\max\{P(Z = 1\mid X = 1, Y = 0) - P(Z = 0\mid X = 0, Y = 0)\} = 0$ over the entire range of the free parameters. Similarly, $\forall l \max\{P(Z = 1\mid X = 1, Y = l) - P(Z = 0\mid X = 0, Y = l)\} = 0$ over the entire range of free parameters.  

For the remaining max operators in $\Gamma$ corresponding to $S$ and $R$, they will all vary independently and be decreasing functions of their corresponding free parameter. Hence, to minimize $\Gamma$ over the range of free parameters, we want to minimize each of the max operators in $\Gamma$ corresponding to $S$ and $R$ while obeying the bounds on the free parameters. 

From Lemma XXX, all $\forall r \in R \max\{P(Z = 1\mid X = 1, Y = r) - P(Z = 0\mid X = 0, Y = r)\} = P(Z = 1\mid X = 1, Y = r) - P(Z = 0\mid X = 0, Y = r)$. Similarly, all the max operators corresponding to $S$ can be zero or non-zero.\\

We consider the following values of free parameters will minimize $Gamma$.
\begin{enumerate}
    \item $\forall l \in L \; P(Z = 1 \mid X = 1, Y = l) = 0$
    \item $\forall r \in R \; P(Z = 1 \mid X = 1, Y = l) = 1$
    \item $\forall s \in S \; P(Z = 1 \mid X = 1, Y = l) = \frac{p^\prime_{1s} - (1 - p_x)}{p_x - (1 - p_x)}$
\end{enumerate}

This setting of free parameters minimizes $Gamma$ because it sets all the max operators capable of attaining $0$ equal to $0$, while minimizing the remaining max operators. This would result in $Gamma$ evaluating as
\[
\Gamma = \sum_{r \in R} p_{y_r}\frac{p^\prime_{1r} - p_x}{1 - p_x}
\]

However, we must check whether this setting of the free parameters obeys the restrictions on the weighted sum of free parameters. To this end, we must check
\begin{align}
\frac{p_{11}p_x - p^\prime_{10}p_{y_0}}{p_x} 
 \leq \sum_{s \in S} y_s \frac{p^\prime_{1s} - (1 - p_x)}{p_x - (1 - p_x)} + \sum_{r \in R} p_{y_r}
\leq p_{11}
\end{align}

With respect to the lower bound, even if $\sum_{s \in S} y_s \frac{p^\prime_{1s} - (1 - p_x)}{p_x - (1 - p_x)} + \sum_{r \in R} p_{y_r}$ not sufficiently large enough, the only parameters that are allowed to increase are $P(Z = 1 \mid X = 1, Y = 0)$, $P(Z = 1 \mid X = 1, Y = l)$ and $P(Z = 1 \mid X = 1, Y = s)$, since the remaining parameters are already set at their individual upper bounds. This will not change the value of $\Gamma$ since the corresponding max operators will still remain $0$ even with the increase in the value of free parameters. 

However, when this upper bound does not hold, then, we must minimize $\Gamma$ while obeying $\sum_{i = 1}^N p_{y_i}P(Z = 1 \mid X = 1, Y = i) \leq p_{11}$. To evaluate this, note that any solution to $\min \Gamma$ will set all the max operators $\forall s \in S\; P(Z = 1 \mid X = 1, Y = s) - P(Z = 0\mid X = 0, Y = s)$ to exactly $0$ or greater, since further reduction still gives a zero, while restricting the range of the other free parameters, thereby increasing the value of $\Gamma$. Therefore, $\forall s \in S\; \max\{0, P(Z = 1 \mid X = 1, Y = s) - P(Z = 0\mid X = 0, Y = s)\} = P(Z = 1 \mid X = 1, Y = s) - P(Z = 0\mid X = 0, Y = s)$. Now, $\Gamma$ will be evaluated as

\begin{align}
\Gamma &= \min_{P} \sum_{s \in S} P(Y = s)(P(Z = 1\mid X = 1, Y = s) - P(Z = 0\mid X = 1, Y = s))\notag\\ 
&+ \sum_{r \in R} P(Y = r)(P(Z = 1\mid X = 1, Y = r) - P(Z = 0\mid X = 1, Y = r))    
\end{align}

And expressing this in terms of free parameters as 
\begin{align*}
\Gamma &= \min_P \sum_{i \in R, S}p_{y_i}(P(Z = 1 \mid X = 1, Y = i)\Bigg(1 - \frac{p_x}{1 - p_x}\Bigg) + \sum_{i \in R, S}p_{y_i} \frac{p^\prime_{11} - (1 - p_x)}{1 - p_x})\\
&= \Bigg(1 - \frac{p_x}{1 - p_x}\Bigg)\sum_{i \in R, S}p_{y_i}P(Z = 1 \mid X = 1, Y = i) + \sum_{i \in R, S} \frac{p^\prime_{11} - (1 - p_x)}{1 - p_x}
\end{align*}

Since $\Gamma$ is a decreasing function of the weighted sum of free parameters, it will be minimized at the upper bound of $\sum_{i = 1}^N P(Z = 1 \mid X = 1, Y = i)$, which in this case equals $p_{11}$. And since the solution for $\min \Gamma$ will set $\forall l \in L\; P(Z = 1 \mid X = 1, L = l) = 0$, $\sum_{i \in R, S}p_{y_i}(P(Z = 1 \mid X = 1, Y = i) = p_{11}$. Plugging this into the expression of $\Gamma$ evaluates to 
\begin{align*}
    &\Bigg(1 - \frac{p_x}{1 - p_x}\Bigg)p_{11} + \sum_{i \in R, S} p_{y_i}\frac{p^\prime_{11} - (1 - p_x)}{1 - p_x}\\
    &\implies = p_{11} +  \frac{-p_{11}p_x + \sum_{i \in R, S} p_{y_i}(p^\prime_{11} - (1 - p_x))}{1 - p_x}\\
    &\implies = p_{11} +  \frac{p_{10}(1 - p_x) - \sum_{l \in l} p_{y_l}p^\prime_{1l} - \sum_{i \in R, S} p_{y_i}(1 - p_x)}{1 - p_x}\\
    &\implies = p_{11} +  \frac{p_{10}(1 - p_x) - (1 - p_x) - \sum_{l \in l} p_{y_l}p^\prime_{1l} - \sum_{i \in R, S} p_{y_i}(1 - p_x) + (1 - p_x)}{1 - p_x}\\
    &\implies = p_{11} +  p_{10} - 1 + \frac{ - \sum_{l \in l} p_{y_l}p^\prime_{1l} + \sum_{l \in L} p_{y_l}(1 - p_x)}{1 - p_x}\\
    &\implies = p_{11} +  p_{10} - 1 + \sum_{l \in L}p_{y_l}\frac{(1 - p_x) - p^\prime_{1l}}{1 - p_x}
\end{align*}

Hence, $\min \Gamma$ will be decided by whether $p_{11} < \sum_{s \in S} y_s \frac{p^\prime_{1s} - (1 - p_x)}{p_x - (1 - p_x)} + \sum_{r \in R} p_{y_r}$ or not. And since $\Gamma$ is a decreasing one-to-one function of the free parameter, this is equivalent to choosing $\max\{ \sum_{r \in R} p_{y_r}\frac{p^\prime_{1r} - p_x}{1 - p_x}, p_{11} +  p_{10} - 1 + \sum_{l \in L}p_{y_l}\frac{(1 - p_x) - p^\prime_{1l}}{1 - p_x}\}$. Since this this is subtracted from $p_{11}$, this max can be converted to a min again, giving us the desired upper bound.\\
\newline
\textbf{Case II}: Consider the following case. $p^\prime_{10} \geq \max{p_x, 1 - p_x}$. Partition $\{1, \dots N\}$ into three disjoint subsets $L$, $R$ and $S$ such that $\forall l \in L \; p^\prime_{1l} \leq \min\{p_x, 1 - p_x\}$,  $\forall r \in R \; p^\prime_{1r} \geq \max\{p_x, 1 - p_x\}$,  and $\forall s \in S \; 1 - p_x < p^\prime_{1s} < p_x$. 

Then, from Lemma XXX and XXXX, $\max\{0, P(Z = 1\mid X = 1, Y = 0) - P(Z = 0\mid X = 0, Y = 0)\} = P(Z = 1\mid X = 1, Y = 0) - P(Z = 0\mid X = 0, Y = 0)$ over the entire range of the free parameters. Similarly, $\forall l \max\{P(Z = 1\mid X = 1, Y = l) - P(Z = 0\mid X = 0, Y = l)\} = 0$, and $\forall r \max\{P(Z = 1\mid X = 1, Y = r) - P(Z = 0\mid X = 0, Y = r)\} = P(Z = 1\mid X = 1, Y = r) - P(Z = 0\mid X = 0, Y = r)$ over the entire range of free parameters.  

In this case, $\Gamma$ will evaluate to
\begin{align}
    \Gamma =& \sum_{i \in \{0, R\}} P(Y = i)(P(Z = 1 \mid X = 1, Y = i) - P(Z = 0 \mid X = 0, Y = i))\notag\\ 
    &+ \sum_{s \in S}P(Y = s) \max\{0, P(Z = 1 \mid X = 1, Y = s) - P(Z = 0\mid X = 0, Y = s)
\end{align}

Expressing this in terms of free parameters, we get
\begin{align}
    \Gamma =& p_{y_0}\frac{p^\prime_{10} - (1 - p_x)}{1 - p_x} + (\sum_{n = 1}^N p_{y_n}P(Z = 1 \mid X = 1, Y = n) - p_{11})\Bigg(\frac{p_x}{1 - p_x} - 1\Bigg)\notag\\
    &+  \sum_{i \in R}p_{y_i} \{P(Z = 1 \mid X = 1, Y = i)\Bigg(1 - \frac{p_x}{1 - p_x}\Bigg) + \frac{p^\prime_{11} - (1 - p_x)}{1 - p_x}\}\notag\\ 
    &+ \sum_{s \in S} P(Y = s)\max\{0, P(Z = 1 \mid X = 1, Y = s)\Bigg(1 - \frac{p_x}{1 - p_x}\Bigg) + \frac{p^\prime_{1s} - (1 - p_x)}{1 - p_x}\}
\end{align}

The above can be simplified to
\begin{align*}
    & p_{y_0}\frac{p^\prime_{10} - (1 - p_x)}{1 - p_x} - p_{11}\Bigg(\frac{p_x}{1 - p_x} - 1\Bigg) + \Bigg(\frac{p_x}{1 - p_x} - 1\Bigg)\sum_{n = 1}^N p_{y_n}P(Z = 1 \mid X = 1, Y = n)\notag\\
    &+  \sum_{i \in R}\Bigg(1 - \frac{p_x}{1 - p_x}\Bigg)p_{y_i}P(Z = 1 \mid X = 1, Y = i) + \sum_{i \in R} p_{y_r}\frac{p^\prime_{11} - (1 - p_x)}{1 - p_x}\notag\\ 
    &+ \sum_{s \in S} p_{y_s}\max\{0, P(Z = 1 \mid X = 1, Y = s)\Bigg(1 - \frac{p_x}{1 - p_x}\Bigg) + \frac{p^\prime_{1s} - (1 - p_x)}{1 - p_x}\}\\
    &\implies = p_{y_0}\frac{p^\prime_{10} - (1 - p_x)}{1 - p_x} - p_{11}\Bigg(\frac{p_x}{1 - p_x} - 1\Bigg)\\
    &+ \sum_{i \in R} p_{y_r}\frac{p^\prime_{11} - (1 - p_x)}{1 - p_x} + \Bigg(\frac{p_x}{1 - p_x} - 1\Bigg)\sum_{n \in N \setminus R} p_{y_n}P(Z = 1 \mid X = 1, Y = n)\\ 
    &+ \sum_{s \in S} p_{y_s}\max\{0, P(Z = 1 \mid X = 1, Y = s)\Bigg(1 - \frac{p_x}{1 - p_x}\Bigg) + \frac{p^\prime_{1s} - (1 - p_x)}{1 - p_x}\}\notag\\
\end{align*}

So, minimizing the above is equivalent to minimizing the following since $p_x > 1 - p_x$ and probabilities are non-negative.
\begin{align*}
&\Bigg(\frac{p_x}{1 - p_x} - 1\Bigg)\sum_{l \in L} p_{y_l}P(Z = 1 \mid X = 1, Y = n) + \Bigg(\frac{p_x}{1 - p_x} - 1\Bigg)\sum_{s \in S} p_{y_s}P(Z = 1 \mid X = 1, Y = n)\\ 
&+ \sum_{s \in S} p_{y_s}\max\{0, P(Z = 1 \mid X = 1, Y = s)\Bigg(1 - \frac{p_x}{1 - p_x}\Bigg) + \frac{p^\prime_{1s} - (1 - p_x)}{1 - p_x}\}\notag\\
\end{align*}

First, all the free parameters corresponding to $l$ will be minimized when set to $0$, which is allowed based on our assumption. 

Note that when the max operator is equal to $P(Z = 1 \mid X = 1, Y = s)\Bigg(1 - \frac{p_x}{1 - p_x}\Bigg) + \frac{p^\prime_{1s} - (1 - p_x)}{1 - p_x}$, the weighted sums of the free parameter cancel each other and equal a constant, i.e. both of them have a counterbalancing effect. 

Hence the minimum is attained when each max operator is exactly $P(Z = 1 \mid X = 1, Y = s)\Bigg(1 - \frac{p_x}{1 - p_x}\Bigg) + \frac{p^\prime_{1s} - (1 - p_x)}{1 - p_x}$, since any deviation away from this will only increase the value of the free parameters without counterbalancing their increase with the max operator since it would be $0$. Then this evaluates to
\begin{align*}
    &\implies = p_{y_0}\frac{p^\prime_{10} - (1 - p_x)}{1 - p_x} - p_{11}\Bigg(\frac{p_x}{1 - p_x} - 1\Bigg) + \sum_{i \in R} p_{y_r}\frac{p^\prime_{11} - (1 - p_x)}{1 - p_x}\\ 
    &+ \sum_{s \in S} p_{y_s}\frac{p^\prime_{1s} - (1 - p_x)}{1 - p_x}\}\notag\\
\end{align*}

And following a similar calculation as the previous case, this can be simplified to
\begin{align*}
    \Gamma = p_{11} + p_{10} - 1 + \sum_{l \in L}p_{y_l}\frac{(1 - p_x) - p^\prime_{1l}}{1 - p_x} 
\end{align*}
However, the above calculations assume that the constraints on the free parameters allow it to take on values such that the max operators behave as we describe. Specifically, this involves $P(Z = 1\mid X = 1, Y = r) = \frac{p^\prime_{1r}}{p_x}$, letting all the variables corresponding to $S$ equal $\frac{p^\prime_{1s} - (1 - p_x)}{p_x - (1 - p_x)}$, and all the variables in $L$ equal to $0$. In the case where $\sum_{i = 1}^N p_{y_N}P(Z = 1 \mid X = 1, Y = i) \geq p_{11} - p_{y_0}$. In this case, $\Gamma$, following a similar argument for $S$ as before, $\Gamma$ will evaluate to 
\begin{align}
    \Gamma =& \sum_{i \in \{0, R\}} P(Y = i)(P(Z = 1 \mid X = 1, Y = i) - P(Z = 0 \mid X = 0, Y = i))\notag\\ 
    &+ \sum_{s \in S}P(Y = s) (P(Z = 1 \mid X = 1, Y = s) - P(Z = 0\mid X = 0, Y = s))
\end{align}
\begin{align*}
&= p_{y_0}\frac{p^\prime_{10} - (1 - p_x)}{1 - p_x} - p_{11}\Bigg(\frac{p_x}{1 - p_x} - 1\Bigg) + \Bigg(\frac{p_x}{1 - p_x} - 1\Bigg)\sum_{n = 1}^N p_{y_n}P(Z = 1 \mid X = 1, Y = n)\notag\\
    &+  \sum_{i \in R}\Bigg(1 - \frac{p_x}{1 - p_x}\Bigg)p_{y_i}P(Z = 1 \mid X = 1, Y = i) + \sum_{r \in R} p_{y_r}\frac{p^\prime_{1r} - (1 - p_x)}{1 - p_x}\notag\\ 
    &+ \sum_{s \in S} p_{y_s}(P(Z = 1 \mid X = 1, Y = s)\Bigg(1 - \frac{p_x}{1 - p_x}\Bigg) + \frac{p^\prime_{1s} - (1 - p_x)}{1 - p_x}\})
\end{align*}

And canceling out relevant terms yields
\begin{align*}
&= p_{y_0}\frac{p^\prime_{10} - (1 - p_x)}{1 - p_x} - p_{11}\Bigg(\frac{p_x}{1 - p_x} - 1\Bigg) + \Bigg(\frac{p_x}{1 - p_x} - 1\Bigg)\sum_{l \in L} p_{y_l}P(Z = 1 \mid X = 1, Y = l)\notag\\
    &+ \sum_{r \in R} p_{y_r}\frac{p^\prime_{1r} - (1 - p_x)}{1 - p_x} + \sum_{s \in S} p_{y_s}\frac{p^\prime_{1s} - (1 - p_x)}{1 - p_x}\}
\end{align*}

To minimize this quantity, we must find the minimum allowed value of $\sum_{l \in L} p_{y_l}P(Z = 1 \mid X = 1, Y = l)$ while still respecting $\sum_{i = 1}^N p_{y_N}P(Z = 1 \mid X = 1, Y = i) \geq p_{11} - p_{y_0}$ and having the max operators behave the same way. This means $\forall r \in R$, set $P(Z = 1 \mid X = 1, Y =r) = 1$ to the highest possible value since these cancel out. Next, set $\forall s \in S$, set $P(Z = 1 \mid X = 1, S = s) = \frac{p^\prime_{1s} - (1 - p_x)}{p_x - (1 - p_x)}$. This entails the following bounds
\begin{align*}
    p_{11} - p_{y_0} \leq \sum_{l \in L}p_{y_l} P(Z = 1 \mid X = 1, Y = l) + \sum_{s \in S} p_{y_s} \frac{p^\prime_{1s} - (1 - p_x)}{p_x - (1 - p_x)} + \sum_{r \in R}p_{y_r}
\end{align*}

Substituting the lowest possible value for $\sum_{l \in L}p_{y_l}P(Z = 1 \mid X = 1, Y = l)$ into the equation above
\begin{align*}
&= p_{y_0}\frac{p^\prime_{10} - (1 - p_x)}{1 - p_x} - p_{11}\Bigg(\frac{p_x}{1 - p_x} - 1\Bigg)\\
&+ \Bigg(\frac{p_x}{1 - p_x} - 1\Bigg)\Bigg(p_{11} - p_{y_0} - \sum_{s \in S} p_{y_s} \frac{p^\prime_{1s} - (1 - p_x)}{p_x - (1 - p_x)} - \sum_{r \in R}p_{y_r} \Bigg)\notag\\
&+ \sum_{r \in R} p_{y_r}\frac{p^\prime_{1r} - (1 - p_x)}{1 - p_x} + \sum_{s \in S} p_{y_s}\frac{p^\prime_{1s} - (1 - p_x)}{1 - p_x}\}
\end{align*}

And this can be simplified as
\begin{align*}
&= p_{y_0}\frac{p^\prime_{10} - p_x}{1 - p_x} 
+ \Bigg(\frac{p_x}{1 - p_x} - 1\Bigg)\Bigg( - \sum_{s \in S} p_{y_s} \frac{p^\prime_{1s} - (1 - p_x)}{p_x - (1 - p_x)} - \sum_{r \in R}p_{y_r} \Bigg)\notag\\
&+ \sum_{r \in R} p_{y_r}\frac{p^\prime_{1r} - (1 - p_x)}{1 - p_x} + \sum_{s \in S} p_{y_s}\frac{p^\prime_{1s} - (1 - p_x)}{1 - p_x}\}\\
&\implies = p_{y_0}\frac{p^\prime_{10} - p_x}{1 - p_x} 
+ \sum_{r \in R} p_{y_r}\frac{p^\prime_{1r} - p_x}{1 - p_x} 
\end{align*}

And subtracting this from $p_{11}$, and applying a similar argument as before using the one to one correspondence of the free parameter with the bounds can be used to prove these match the bounds in Theorem 2.\\

\textbf{Case III}: Consider the following case. $1 - p_x < p^\prime_{10} < \max{p_x, 1 - p_x}$. Partition $\{1, \dots N\}$ into three disjoint subsets $L$, $R$ and $S$ such that $\forall l \in L \; p^\prime_{1l} \leq \min\{p_x, 1 - p_x\}$,  $\forall r \in R \; p^\prime_{1r} \geq \max\{p_x, 1 - p_x\}$,  and $\forall s \in S \; 1 - p_x < p^\prime_{1s} < p_x$. 

We first consider the special case where for all $i$, $1 - p_x < p^\prime_{1i} < p_x$. Then, from Lemma XXX, for all max operators to simultaneously equal $P(Z = 1 \mid X = 1, Y = i) - P(Z = 0 \mid X = 0, Y = i)$, then $p_{11} + p_{10} - 1 \geq 0$. Here, by a similar argument as Theorem 1, if $p_{11} + p_{10} - 1 \geq 0$, then all max operators will cancel out the values for the free parameter, and any shift from this will be greater because the counterbalancing action of the max operators will not be there. 

Next, we consider the case where $p_{11} + p_{10} - 1 < 0$. Here all bounds cannot simultaneously open, and so we check whether the bounds on the free parameters all allow the max operators to evaluate to $0$. 

From Lemma XXX, when $P(Z = 1 \mid X = 1, Y = i) = \frac{p^\prime_{1i} - (1 - p_x)}{p_x - (1 - p_x)}$, then the $\max\{0, P(Z = 1 \mid X = 1, Y = i) - P(Z = 0 \mid X = 0, Y = i\} = 0$. However, we still need to examine the behavior of $\max\{0, P(Z = 1 \mid X = 1, Y = 0) - P(Z = 0\mid X = 0, Y = 0\}$ at the value. So we check whether $\sum_{i = 1}^N p_{y_i}\frac{p^\prime_{1i} - (1 - p_x)}{p_x - (1 - p_x)} \leq \frac{p_{y_0}((1 - p_x) - p^\prime_{10})}{p_x - (1 - p_x)} + p_{11}$. 

Following a similar calculation as Lemma XXX, we can show that $p_{11} + p_{10} - 1 < 0 \implies \sum_{i = 1}^N p_{y_i}\frac{p^\prime_{1i} - (1 - p_x)}{p_x - (1 - p_x)} < \frac{p_{y_0}((1 - p_x) - p^\prime_{10})}{p_x - (1 - p_x)} + p_{11}$, which means that there at this value of free parameters $\frac{p^\prime_{1i} - (1 - p_x)}{p_x - (1 - p_x)}$, all the max operators can open as $0$. When the lower bound from individual bounds group overrides the sum bounds group, this will be a valid solution and make all max operators equal $0$. However, when the sum of bounds lower bound overrides this, we know this bound still alolows for $P(Y = 0)$ max operator to equal $0$, and since it has only increase the lower bound, it will only decrease already $0$ individual max operators, always allowing $0$ as a solution.  

So when $p_{11} + p_{10} - 1 \geq 0$, all max operators open and give the bound of $p_{11} - p_{10} - 1$, and otherwise $0$. This proves the bounds we care about. 

\subsection{Proof for Lower Bound in Theorem 2}

As seen in Lemma XXX, when $p_{11} - p_{10} \geq 0$, all max operators can open. In this case, this will be the minimum since any deviation from this setting results in one of the max operators becoming $0$ and no longer being able to counterbalance the increase in the other, leading to an increase in the overall value of $\Delta$. 

Next, consider the case where $p_{11} - p_{10} < 0$, then all max operators cannot open simultaneously. Here we show that all max operators equaling $0$ will be a valid point in the space of the free parameters. For $i \in \{1, \dots , N\}$, each of their corresponding max operators will equal $0$ when $P(Z = 1\mid X = 1, Y = i) = p^\prime_{1i}$. As seen in Lemma XX, the individual bounds on $P(Z = 1 \mid X = 1, Y = 1)$ allow this point to exist.  Next, we check whether this setting of $P(Z = 1 \mid X = 1, Y = i)$ makes the $P(Y = 0)$ max operator evaluate to $0$, i.e. $\sum_{i = 1}^N p_{y_i}p^\prime_{1i} \geq p_{11} - p^\prime_{10}p_{y_0}$. And since $p_{11} - p_{10} < 0$, $\sum_{i = 1}^N p_{y_i}p^\prime_{1i} > p_{11} - p^\prime_{10}p_{y_0}$. 

However, this still requires us to ensure $\sum_{i = 1}^N p_{y_i}p^\prime_{1i}$ is a valid setting for the free parameter, and therefore we must check whether this is less than both the upper bounds on the weighted sum of the free parameter, i.e.

\begin{align*}
    \sum_{i = 1}^N p_{y_i}p^\prime_{1i} \leq p_{11}\\
    \sum_{i = 1}^N p_{y_i}p^\prime_{1i} \leq \frac{p_{11}p_x - p^\prime_{10}p_{y_0}}{p_x}\\
\end{align*}

To check the first, see that
\begin{align*}
        &\sum_{i = 1}^N p_{y_i}p^\prime_{1i} \leq p_{11}\\
        &\implies p_{11}p_x + p_{10}(1 - p_x) - p^\prime_{10}p_{y_0} \leq p_{11}\\
        &\implies  - p^\prime_{10}p_{y_0} \leq (1 - p_x)(p_{11} - p_{10})\\
\end{align*}
And this show the point evaluating to $0$ will be contained when $p_{11}$ is the upper bound.

Next, when $\frac{p_{11}p_x - p^\prime_{10}p_{y_0}}{p_x}$ is the lower bound, this mean this is smaller than $p_{11}$. Since the $P(Y = 0)$ max operator can still equal $0$, we set $\sum_{i = 1}^N p_{y_i}P(Z = 1 \mid X = 1, Y = i)$ equal to $ p_{11} - p^\prime_{10}p_{y_0}$. Since $p_{11} - p_{10} < 0$, then $p_{11} - p^\prime_{10}p_{y_0} < \sum_{i = 1}^N p^\prime_{1i}$, this means the values of the individual free parameter can be lowered even more than $p^\prime_{1i}$, allowing the remaining max operators to equal $0$ as well. This shows that in all cases, the solution of $0$ will be contained. 

And by a similar reasoning as before, this means $\Delta = \max\{0, p_{11} - p_{10}\}$. 

% \begin{align*}
%      &\sum_{i = 1}^N p_{y_i}p^\prime_{1i} \leq \frac{p_{11}p_x - p^\prime_{10}p_{y_0}}{p_x}\\
%     &- p^\prime_{10}p_{y_0} \leq (1 - p_x)(p_{11} - p_{10}) - \frac{p^\prime_{10}p_{y_0}}{p_x}\\
% \end{align*}
\section{Proof of Theorem 3}
To prove Theorem 3, we first state lemmas we utilize in the proof. Proofs can be found in Section XX. 

\begin{lemma}\label{lemma:RREF-y-delta}
Let $X$ and $Z$ be binary random variables, and let $Y$ be a discrete random variable taking on values in $0, \dots ,N$. Assume access to two distributions $P^T(Z, X)$ and $P^E(Z, Y)$, where $P^T(Y) = P^E(Y)$, $P^E(X) = P^T(X) + \delta_X$, $X \independent Y$ in both $P^E$ and $P^T$ and $P^T(Z = 1 \mid X, Y) = P^E(Z = 1\mid X, Y)$. The conditional distributions $P^T(Z \mid X, Y)$ can be expressed as a system of equations with free parameters $P^T(Z = 1 \mid X = 1, Y = i)$ for $i \in \{1, \dots, N\}$ as

{\small
\begin{align*}
P^T(Z = 1 \mid X = 0, Y = 0) &=  \frac{p_x + \delta_X}{1 - p_x - \delta_X}\sum_{n = 1}^N\frac{p_{y_n}}{p_{y_0}}P^T(Z = 1 \mid X = 1, Y = n) + \frac{p^E_{10}p_{y_0} - p^T_{11}(p_x + \delta_X)}{(1 - p_x - \delta_X)p_{y_0}}\\
P^T(Z = 1 \mid X = 1, Y = 0)&= \frac{p^T_{11}}{p_{y_0}} - \sum_{n = 1}^N\frac{p_{y_n}}{p_{y_0}}P^T(Z = 1 \mid X = 1, Y = n)\\
P^T(Z = 1 \mid X = 0, Y = 1)&= \frac{p^E_{11}}{1 - p_x - \delta_X} - \frac{p_x + \deltaXX}{1 - p_x - \delta_X}P^T(Z = 1 \mid X = 1, Y = 1)\\
P^T(Z = 1 \mid X = 0, Y = 2)&= \frac{p^E_{12}}{1 - p_x - \delta_X} - \frac{p_x + \delta_X}{1 - p_x - \delta_X}P^T(Z = 1 \mid X = 1, Y = 2)\\
\vdots\\
P^T(Z = 1 \mid X = 0, Y = N)&= \frac{p^E_{1N}}{1 - p_x - \delta_X} - \frac{p_x + \delta_X}{1 - p_x - \delta_X}P^T(Z = 1 \mid X = 1, Y = N)\\
\end{align*}
}
Where $P^T(X = 1)$ is denoted as $p_x$ , $P^T(Y = n)= P^E(Y = n)$ is denoted as $p_{y_n}$, $P^T(Z = 1 \mid X = 1)$ is denoted as $p^T_{11}$, $P^T(Z = 1 \mid X = 0)$ is denoted as $p^T_{10}$, and $P^T(Z = 1 \mid Y = n)$ is denoted as $p^E_{1n}$ for $n \in \{0, \dots, N\}$.
\end{lemma}

\begin{lemma}\label{lem:free-param-bounds-delta}
To ensure the solution to the system of equations in Lemma \ref{lemma:RREF-y-delta} form coherent probabilities, the following bounds on the free parameters must hold
{\small
\begin{align}\label{eq:sum-bounds}
\max\begin{bmatrix}
   \frac{p^T_{11}(p_x + \delta_X) - p^E_{10}p_{y_0}}{p_x + \delta_X} \\
   p^T_{11} - p_{y_0}
\end{bmatrix} \leq \sum_{n = 1}^N y_nP^T(Z = 1 \mid X = 1, Y = n) 
\leq \min\begin{bmatrix}
    \frac{(1 - p_x - \delta_X)p_{y_0} + p^T_{11}(p_x + \delta_X) - p^E_{10}y_0}{p_x + \delta_X}\\
    p^T_{11}
\end{bmatrix}
\end{align}
}

And for each $i \in \{1, \dots, N\}$, we the bounds on the following free parameters $P(Z = 1\mid X = 1, Y = i)$
\begin{align}\label{eq:individual-bounds}
    \max\begin{bmatrix}
        0\\
        \frac{p^E_{1i} - (1 - p_x - \delta_X)}{p_x + \delta_X}
    \end{bmatrix}
        \leq P^T(Z = 1\mid X = 1, Y = i) \leq 
    \min\begin{bmatrix}
        1\\
        \frac{p^E_{1i}}{p_x + \delta_X}
    \end{bmatrix}
\end{align}
\end{lemma}

\begin{lemma}
    The following implications hold:
    \begin{equation*}
     p^E_{10} < p_x + \delta_X \implies \frac{p^T_{11}(p_x + \delta_X) - p^E_{10}p_{y_0}}{p_x + \delta_X} > p^T_{11} - p_{y_0}   
    \end{equation*}
    \begin{equation*}
     p^T_{10} \geq p_x + \delta_X \implies \frac{p^T_{11}(p_x + \delta_X) - p^E_{10}p_{y_0}}{p_x + \delta_X} \leq p^T_{11} - p_{y_0}   
    \end{equation*}
    \begin{equation*}
        p^E_{10} < 1 - p_x - \delta_X \implies p^T_{11} < \frac{(1 - p_x - \delta_X)p_{y_0} + p^T_{11}(p_x + \delta_X) - p^E_{10}p_{y_0}}{p_x + \delta_X}
    \end{equation*}
    \begin{equation*}
        p^E_{10} \geq 1 - p_x - \delta_X \implies p^T_{11} \geq \frac{(1 - p_x - \delta_X)p_{y_0} + p^T_{11}(p_x + \delta_X) - p^E_{10}p_{y_0}}{p_x + \delta_X}
    \end{equation*}
\end{lemma}

\begin{proof}
Each of these is proved using a proof by contra-positive. Starting with $p^E_{10} < p_x + \delta_X \implies \frac{p_{11}(p_x + \delta_X) - p^E_{10}p_{y_0}}{p_x + \delta_X} > p^T_{11} - p_{y_0}$, the contra-positive of this statement is
    \[
    \frac{p^T_{11}(p_x + \delta_X) - p^E_{10}p_{y_0}}{p_x + \delta_X} \leq p^T_{11} - p_{y_0} \implies p^E_{10} \geq p_x + \delta_X
    \]
    To see this holds, note that
    \begin{align*}
        \frac{p^T_{11}(p_x + \delta_X) - p^E_{10}p_{y_0}}{p_x + \delta_X} \leq p^T_{11} - p_{y_0}\\
        \implies -\frac{p^E_{10}p_{y_0}}{p_x + \delta_X} \leq  - p_{y_0}\\
        \implies p^\prime_{10} \geq p_x + \delta_X
    \end{align*}
This proves $p^E_{10} < p_x + \delta_X \implies \frac{p^T_{11}(p_x + \delta_X) - p^E_{10}p_{y_0}}{p_x + \delta_X} > p^T_{11} - p_{y_0}$.\\
Next, for $p^E_{10} \geq p_x + \delta_X \implies \frac{p^T_{11}(p_x + \delta_X) - p^E_{10}p_{y_0}}{p_x + \delta_X} \leq p^T_{11} - p_{y_0}$, following a similar proof strategy, the contra-positive can be written as
\[
\frac{p_{11}(p_x + \delta_X) - p^E_{10}p_{y_0}}{p_x + \delta_X} > p^T_{11} - p_{y_0} \implies p^E_{10} < p_x + \delta_X
\]
To see this holds, note that
\begin{align*}
    \frac{p_{11}p_x - p^\prime_{10}p_{y_0}}{p_x} > p_{11} - p_{y_0}\\
    \implies -\frac{p^\prime_{10}p_{y_0}}{p_x} > - p_{y_0}\\
    \implies p^\prime_{10} < p_x
\end{align*}
This proves $p^\prime_{10} \geq p_x \implies \frac{p_{11}p_x - p^\prime_{10}p_{y_0}}{p_x} \leq p_{11} - p_{y_0}$.\\
Next, for $p^\prime_{10} < 1 - p_x \implies p_{11} < \frac{(1 - p_x)p_{y_0} + p_{11}p_x - p^\prime_{10}p_{y_0}}{p_x}$, the contra-positive is written as
\[
p_{11} \geq \frac{(1 - p_x)p_{y_0} + p_{11}p_x - p^\prime_{10}p_{y_0}}{p_x}  \implies p^\prime_{10} \geq 1 - p_x
\]
To see this holds, note that
\begin{align*}
    &p_{11} \geq \frac{(1 - p_x)p_{y_0} + p_{11}p_x - p^\prime_{10}p_{y_0}}{p_x}\\
    &\implies 0 \geq (1 - p_x)p_{y_0} - p^\prime_{10}p_{y_0}\\
    &\implies  p^\prime_{10} \geq 1 - p_x
\end{align*}
This proves $p^\prime_{10} < 1 - p_x \implies p_{11} < \frac{(1 - p_x)p_{y_0} + p_{11}p_x - p^\prime_{10}p_{y_0}}{p_x}$.\\
Next, for $p^\prime_{10} \geq 1 - p_x \implies p_{11} \geq \frac{(1 - p_x)p_{y_0} + p_{11}p_x - p^\prime_{10}p_{y_0}}{p_x}$ the contra-positive is written as
\[
p_{11} < \frac{(1 - p_x)p_{y_0} + p_{11}p_x - p^\prime_{10}p_{y_0}}{p_x}  \implies p^\prime_{10} < 1 - p_x
\]
To see this holds, note that
\begin{align*}
    &p_{11} < \frac{(1 - p_x)p_{y_0} + p_{11}p_x - p^\prime_{10}p_{y_0}}{p_x}\\
    &\implies 0 < (1 - p_x)p_{y_0} - p^\prime_{10}p_{y_0}
    &\implies p^\prime_{10} < 1 - p_x
\end{align*}

This concludes the proof.
\end{proof}

\begin{lemma}
For $i \in \{1, \dots, N\}$, when $p^\prime_{1i} > 1 - p_x \implies \frac{p^\prime_{11} - (1 - p_x)}{p_x} > 0$. When $p^\prime_{1i} < p_x \implies \frac{p^\prime_{11}}{p_x} < 1$    
\end{lemma}

\begin{lemma}
Using the solution to the system of equations in Lemma \ref{lemma:RREF-y-delta}, each of the terms in $\Delta$ and $\Gamma$ defined in Lemma \ref{lem:joint-bounds} are expressed in terms of the free parameters below. 
\begin{enumerate}
    \item For the term in $\Gamma$ corresponding to $Y = 0$
    \begin{align*}
        &\mathbb{P}(Z = 1 \mid X = 1, Y = 0) - \mathbb{P}(Z = 0 \mid X = 0, Y = 0)\\
        &= \frac{p^\prime_{10} - (1 - p_x)}{1 - p_x} + \frac{\sum_{n = 1}^N p_{y_n}P(Z = 1 \mid X = 1, Y = n) - p_{11}}{p_{y_0}}\Bigg(\frac{p_x}{1 - p_x} - 1\Bigg)
    \end{align*}
    
\item For the terms in $\Gamma$ corresponding to $Y = i$, $i \in \{1, \dots , N\}$
    \begin{align*}
        &P(Z = 1 \mid X = 1, Y = i) - P(Z = 0 \mid X = 0, Y = i)\\
        &= P(Z = 1 \mid X = 1, Y = i)\Bigg(1 - \frac{p_x}{1 - p_x}\Bigg) + \frac{p^\prime_{11} - (1 - p_x)}{1 - p_x}\\
    \end{align*}
\item For the term in $\Delta$ corresponding to $Y = 0$:
    \begin{align*}
        &\mathbb{P}(Z = 1 \mid X = 1, Y = 0) - \mathbb{P}(Z = 1 \mid X = 0, Y = 0)\\
        &= \frac{p_{11} - p^\prime_{10}p_{y_0} - \sum_{n = 1}^N p_{y_n}\mathbb{P}(Z = 1\mid X = 1, Y = n)}{(1 - p_x)p_{y_0}}
    \end{align*}
\item For the term in $\Delta$ corresponding to $Y = i$, $i \in \{1, \dots , N\}$
    \begin{align*}
        &\mathbb{P}(Z = 1 \mid X = 1, Y = 1) - \mathbb{P}(Z = 1 \mid X = 0, Y = 1)\\
        &=\frac{\mathbb{P}(Z = 1 \mid X = 1, Y = i) - p^\prime_{1i}}{1 - p_x}
    \end{align*}
\end{enumerate}
\end{lemma}

\begin{proof}
    Using the system of equations obtained in Lemma \ref{lemma:RREF-y-delta}, each term in $\Gamma$ can be expressed using these free parameters. 
\begin{enumerate}
    \item $\max \{0, \mathbb{P}(Z = 1 \mid X = 1, Y = 0) - \mathbb{P}(Z = 0 \mid X = 0, Y = 0)\}$
    \begin{equation}\label{eq:Gamma-y0-1}
        P^T(Z = 1 \mid X = 1, Y = 0) &= \frac{p^T_{11}}{p_{y_0}} - \sum_{n = 1}^N\frac{p_{y_n}}{p_{y_0}}P^T(Z = 1 \mid X = 1, Y = n)
    \end{equation}
    \begin{align}\label{eq:Gamma-y0-2}
        &P^T(Z = 0 \mid X = 0, Y = 0) = 1 -\\
        &\Bigg(\frac{p_x + \delta_X}{1 - p_x - \delta_X}\sum_{n = 1}^N\frac{p_{y_n}}{p_{y_0}}P^T(Z = 1 \mid X = 1, Y = n) + \frac{p^E_{10}p_{y_0} - p^T_{11}(p_x + \delta_X)}{(1 - p_x - \delta_X)p_{y_0}}\Bigg)
    \end{align}
    Subtracting these two and following a similar calculation as Lemma XXXX, this simplifies to
    \begin{equation*}
    \frac{p^E_{10} - (1 - p_x - \delta_X)}{1 - p_x - \delta_X} + \frac{\sum_{n = 1}^N p_{y_n}P^T(Z = 1 \mid X = 1, Y = n) - p^T_{11}}{p_{y_0}}\Bigg(\frac{p_x + \delta_X}{1 - p_x - \delta_X} - 1\Bigg) 
    \end{equation*}


    \item $\max\{0, P(Z = 1 \mid X = 1, Y = i) - P(Z = 0 \mid X = 0, Y = i)\}$: The probability $P(Z = 0 \mid X = 0, Y = i)$ for $i \in \{1, \dots ,N\}$ can be expressed in terms of the free parameters as
    \begin{align*}
        &P(Z = 0 \mid X = 0, Y = i) = 1 -\Bigg( \frac{p^E_{1i}}{1 - p_x - \delta_X} - \frac{p_x + \delta_X}{1 - p_x - \delta_X}P^T(Z = 1 \mid X = 1, Y = i)\Bigg)\\
        &\implies P(Z = 1 \mid X = 1, Y = i) - P(Z = 0 \mid X = 0, Y = i) \\
        &= P^T(Z = 1 \mid X = 1, Y = i) - 1 + \frac{p^E_{1i}}{1 - p_x - \delta_X} - \frac{p_x + \delta_X}{1 - p_x - \delta_X}P(Z = 1 \mid X = 1, Y = i)\\
        &= P(Z = 1 \mid X = 1, Y = i)\Bigg(1 - \frac{p_x + \delta_X}{1 - p_x - \delta_X}\Bigg) + \frac{p^E_{11} - (1 - p_x - \delta_X)}{1 - p_x - \delta_X}
    \end{align*}
\end{enumerate}
    This concludes the proof for the terms in $\Gamma$. Next, enumerating the calculations for the terms in $\Delta$.
    \begin{enumerate}
        \item $\mathbb{P}(Z = 1 \mid X = 1, Y = 0) - \mathbb{P}(Z = 1 \mid X = 0, Y = 0)$
        \begin{align*}
        &= \frac{p^T_{11}}{p_{y_0}} - \sum_{n = 1}^N\frac{p_{y_n}}{p_{y_0}}P^T(Z = 1 \mid X = 1, Y = n)\\
        & - \Bigg(\frac{p_x + \delta_X}{1 - p_x - \delta_X}\sum_{n = 1}^N\frac{p_{y_n}}{p_{y_0}}\mathbb{P}(Z = 1 \mid X = 1, Y = n)
        + \frac{p^E_{10}p_{y_0} - p^T_{11}(p_x + \delta_X)}{(1 - p_x - \delta_X))p_{y_0}}\Bigg)\\
        &= \frac{p^T_{11} - p^E_{10}p_{y_0} - \sum_{n = 1}^N p_{y_n}P^T(Z = 1\mid X = 1, Y = n)}{(1 - p_x - \delta_X)p_{y_0}}
    \end{align*}
    \item $\max\{0, \mathbb{P}(Z = 1 \mid X = 1, Y = i) - \mathbb{P}(Z = 1 \mid X = 0, Y = i)\}$ for $i \in \{1, \dots, N\}$
    \begin{align*}
        &P^T(Z = 1 \mid X = 0, Y = i) = \frac{p^E_{1i}}{1 - p_x - \delta_X} - \frac{p_x + \delta_X}{1 - p_x - \delta_X}P^T(Z = 1 \mid X = 1, Y = i)\\
        &\implies P^T(Z = 1 \mid X = 1, Y = i) - P^T(Z = 1 \mid X = 0, Y = i)\\
        &= P^T(Z = 1 \mid X = 1, Y = i) - \frac{p^E_{1i}}{1 - p_x - \delta_X} + \frac{p_x + \delta_X}{1 - p_x - \delta_X}P^T(Z = 1 \mid X = 1, Y = i)\\
        &= \frac{P^T(Z = 1 \mid X = 1, Y = i) - p^E_{1i}}{1 - p_x - \delta_X}
    \end{align*}
    \end{enumerate}
    This concludes the proof of the Lemma.
\end{proof}
\subsection{Behavior of Max Operators in $\Gamma$}
The behavior of this function must be analyzed in two cases, one where $p_x > 1 - p_x$, and vice-versa. We present results for $p_x > 1 - p_x$, and analogous results can be derived for $p_x < 1 - p_x$. 

\begin{lemma}
    Assume $p_x + \delta_X > 1 - p_x - \delta_X$. The function $\max \{0, P^T(Z = 1 \mid X = 1, Y = 0) - P^T(Z = 0 \mid X = 0, Y = 0)\} \geq 0$ when
    \begin{align*}
            \sum_{n = 1}^N p_{y_n}P(Z = 1 \mid X = 1, Y = n) \geq \frac{p_{y_0}((1 - p_x - \delta_X) - p^\prime_{10})}{(p_x + \delta_X) - (1 - p_x - \delta_X)} + p^T_{11}
    \end{align*}
\end{lemma}

\begin{proof}
    From the result of Lemma \ref{}, $\mathbb{P}(Z = 1 \mid X = 1, Y = 0) - \mathbb{P}(Z = 0 \mid X = 0, Y = 0)$ can be expressed in terms of the free parameter as
    \begin{align*}
        \frac{p^\prime_{10} - (1 - p_x)}{1 - p_x} + \frac{\sum_{n = 1}^N p_{y_n}P(Z = 1 \mid X = 1, Y = n) - p_{11}}{p_{y_0}}\Bigg(\frac{p_x}{1 - p_x} - 1\Bigg)
    \end{align*}
    Now, we use a proof by contra-positive to first show that
    \begin{align*}
        &\frac{p^\prime_{10} - (1 - p_x)}{1 - p_x} + \frac{\sum_{n = 1}^N p_{y_n}P(Z = 1 \mid X = 1, Y = n) - p_{11}}{p_{y_0}}\Bigg(\frac{p_x}{1 - p_x} - 1\Bigg) < 0\\
        &\implies \sum_{n = 1}^N p_{y_n}P(Z = 1 \mid X = 1, Y = n) < \frac{p_{y_0}((1 - p_x) - p^\prime_{10})}{p_x - (1 - p_x)} + p_{11}
    \end{align*}
    To see this, note that
    \begin{align*}
        &\frac{p^\prime_{10} - (1 - p_x)}{1 - p_x} + \frac{\sum_{n = 1}^N p_{y_n}P(Z = 1 \mid X = 1, Y = n) - p_{11}}{p_{y_0}}\Bigg(\frac{p_x}{1 - p_x} - 1\Bigg) < 0\\
        &\implies p_{y_0}\frac{p^\prime_{10} - (1 - p_x)}{p_{y_0}(1 - p_x)} + \frac{\sum_{n = 1}^N p_{y_n}P(Z = 1 \mid X = 1, Y = n) - p_{11}}{p_{y_0}}\Bigg(\frac{p_x - (1 - p_x)}{1 - p_x} \Bigg) < 0\\
        &\implies p_{y_0}(p^\prime_{10} - (1 - p_x)) + (\sum_{n = 1}^N p_{y_n}P(Z = 1 \mid X = 1, Y = n) - p_{11})\Bigg(p_x - (1 - p_x)\Bigg) < 0\\
        &\implies \sum_{n = 1}^N p_{y_n}P(Z = 1 \mid X = 1, Y = n) < \frac{p_{y_0}((1 - p_x) - p^\prime_{10})}{p_x - (1 - p_x)} + p_{11}\\
    \end{align*}
    This concludes the proof.
\end{proof}

\begin{lemma}
    Assume $p_x + \delta_X> 1 - p_x - \delta_X$. If $p^E_{10} \geq p_x + \delta_X$, then 
    \[
    p^T_{11} - y_0 \geq \frac{p_{y_0}((1 - p_x - \delta_X) - p^E_{10})}{(p_x + \delta_X) - (1 - p_x - \delta_X)} + p^T_{11}
    \]
\end{lemma}
\begin{proof}
    Following a proof by contra-positive, the contra-positive is given as
    \begin{align*}
        p_{11} - y_0 < \frac{p_{y_0}((1 - p_x) - p^\prime_{10})}{p_x - (1 - p_x)} + p_{11} \implies p^\prime_{10} < p_x
    \end{align*}
    To see this, note that
    \begin{align*}
        &p_{11} - p_{y_0} < \frac{p_{y_0}((1 - p_x) - p^\prime_{10})}{p_x - (1 - p_x)} + p_{11}\\
        &\implies - 1 < \frac{((1 - p_x) - p^\prime_{10})}{p_x - (1 - p_x)}\\
        &\implies  p_x  >  p^\prime_{10}
    \end{align*}
    This concludes the proof.
\end{proof}

These two Lemmas imply that when $p_x > 1 - p_x$, $p^\prime_{10} \geq \max\{p_x, 1 - p_x\}$ then 
\begin{align*}
    &\max\{0, \mathbb{P}(Z = 1 \mid X = 1, Y = 0) - \mathbb{P}(Z = 0 \mid X = 0, Y = 0)\}\\
    &= \mathbb{P}(Z = 1 \mid X = 1, Y = 0) - \mathbb{P}(Z = 0 \mid X = 0, Y = 0)
\end{align*}

Analogously, when $p^\prime_{10} \leq \min\{p_x, 1 - p_x\}$, i.e. $p^\prime_{10} \leq 1 - p_x$, we first consider the following Lemma.
\begin{lemma}
    Assume $p_x > 1 - p_x - \delta_X$. If $p^E < p_x$, then 
    \[
    \frac{p^T_{11}(p_x +\delta_X) - p^E_{10}p_{y_0}}{p_x} < \frac{p_{y_0}((1 - p_x - \delta_X) - p^E_{10})}{(p_x + \delta_X) - (1 - p_x - \delta_X)} + p^T_{11}
    \]
\end{lemma}
\begin{proof}
    Following a proof by contra-positive, the contra-positive is given as
    \[
    \frac{p_{11}p_x - p^\prime_{10}p_{y_0}}{p_x} \geq \frac{p_{y_0}((1 - p_x) - p^\prime_{10})}{p_x - (1 - p_x)} + p_{11} \implies p^\prime_{10} \geq p_x
    \]
    To see this, note that
    \begin{align*}
        &\frac{p_{11}p_x - p^\prime_{10}p_{y_0}}{p_x} \geq \frac{p_{y_0}((1 - p_x) - p^\prime_{10})}{p_x - (1 - p_x)} + p_{11}\\
        &\implies \frac{- p^\prime_{10}}{p_x} \geq \frac{((1 - p_x) - p^\prime_{10})}{p_x - (1 - p_x)}\\
        &\implies - p^\prime_{10}p_x + p^\prime_{10}(1 - p_x) \geq (1 - p_x)p_x - p^\prime_{10}p_x\\
        &\implies p^\prime_{10} \geq p_x
    \end{align*}
    This concludes the proof.
\end{proof}

\begin{lemma}
    Assume $p_x > 1 - p_x$. If $p^\prime_{10} \leq 1 - p_x$, then 
    \[
    p_{11} \leq \frac{p_{y_0}((1 - p_x) - p^\prime_{10})}{p_x - (1 - p_x)} + p_{11}
    \]
\end{lemma}
These two Lemmas imply that when $p_x > 1 - p_x$, $p^\prime_{10} \leq \min\{p_x, 1 - p_x\}$ then 
\begin{align*}
    &\max\{0, \mathbb{P}(Z = 1 \mid X = 1, Y = 0) - \mathbb{P}(Z = 0 \mid X = 0, Y = 0)\} = 0
\end{align*}
Next, consider the case when $1 - p_x < p^\prime_{10} < p_x$. Then the following bounds hold
\begin{align*}
   \frac{p_{11}x - p^\prime_{10}y_0}{p_x} 
 \leq \sum_{n = 1}^N y_n\mathbb{P}(Z = 1 \mid X = 1, Y = n) 
\leq \frac{(1 - x)y_0 + p_{11}x - p^\prime_{10}y_0}{x}
\end{align*}

From Lemma 9, $\frac{p_{11}x - p^\prime_{10}y_0}{x} < \frac{p_{y_0}((1 - p_x) - p^\prime_{10})}{p_x - (1 - p_x)} + p_{11}$. And under these conditions,
\begin{align*}
    \frac{p_{y_0}((1 - p_x) - p^\prime_{10})}{p_x - (1 - p_x)} + p_{11} < \frac{(1 - x)y_0 + p_{11}x - p^\prime_{10}y_0}{x}
\end{align*}

% \begin{lemma}
%     Assume $p_x < 1 - p_x$. The function $\max \{0, \mathbb{P}(Z = 1 \mid X = 1, Y = 0) - \mathbb{P}(Z = 0 \mid X = 0, Y = 0)\} \geq 0$ when
%     \begin{align*}
%             \sum_{n = 1}^N p_{y_n}P(Z = 1 \mid X = 1, Y = n) \leq \frac{p_{y_0}( p^\prime_{10} - (1 - p_x))}{(1 - p_x) - p_x} + p_{11}   
%     \end{align*}
% \end{lemma}
Now, we provide lemmas that similarly examine the behavior of $\max \{0, \mathbb{P}(Z = 1 \mid X = 1, Y = i) - \mathbb{P}(Z = 0 \mid X = 0, Y = i)\}$. As before, the behavior of this function needs to be analyzed in two case, and we provide lemmas for $p_x > 1 - p_x$, and lemmas for $p_x < 1 - p_x$ can be analogously derived.

\begin{lemma}
    Assume $p_x > 1 - p_x$. The function $\max \{0, \mathbb{P}(Z = 1 \mid X = 1, Y = i) - \mathbb{P}(Z = 0 \mid X = 0, Y = i)\} \geq 0$ for $i \in \{1, \dots, N\}$ when
    \begin{align*}
            P(Z = 1 \mid X = 1, Y = i) \leq \frac{p^\prime_{1i} - (1 - p_x - \delta_X)}{(p_x + \delta_X) - (1 - p_x - \delta_X)}    
    \end{align*}
\end{lemma}
\begin{proof}
From the result of Lemma \ref{}, $\mathbb{P}(Z = 1 \mid X = 1, Y = i) - \mathbb{P}(Z = 0 \mid X = 0, Y = i)\}$ can be expressed in terms of the free parameter as 
\[
P(Z = 1 \mid X = 1, Y = i)\Bigg(1 - \frac{p_x}{1 - p_x}\Bigg) + \frac{p^\prime_{11} - (1 - p_x)}{1 - p_x}
\]
Following a proof by contra-positive, we write the contra-positive as
\begin{align*}
&P(Z = 1 \mid X = 1, Y = i)\Bigg(1 - \frac{p_x}{1 - p_x}\Bigg) + \frac{p^\prime_{11} - (1 - p_x)}{1 - p_x} < 0\\
&\implies P(Z = 1 \mid X = 1, Y = i) > \frac{p^\prime_{1i} - (1 - p_x)}{p_x - (1 - p_x)}     
\end{align*}
To see this, note that
\begin{align*}
    &P(Z = 1 \mid X = 1, Y = i)\Bigg(1 - \frac{p_x}{1 - p_x}\Bigg) + \frac{p^\prime_{11} - (1 - p_x)}{1 - p_x} < 0\\
    &\implies P(Z = 1 \mid X = 1, Y = i)\Bigg(\frac{(1 - p_x) - p_x}{1 - p_x}\Bigg)  < \frac{(1 - p_x) - p^\prime_{11}}{1 - p_x}\\
    &\implies P(Z = 1 \mid X = 1, Y = i)\Bigg((1 - p_x) - p_x\Bigg)  < (1 - p_x) - p^\prime_{11}\\
    &\implies P(Z = 1 \mid X = 1, Y = i)  >  \frac{p^\prime_{11} - (1 - p_x)}{p_x - (1 - p_x)}
\end{align*}

This concludes the proof.
\end{proof}

\begin{lemma}
    Assume $p_x > 1 - p_x$. If $p^\prime_{1i} \geq x$ for $i \in \{1, \dots , N\}$, then 
    \begin{align*}
            1 \leq \frac{p^\prime_{1i} - (1 - p_x)}{p_x - (1 - p_x)}    
    \end{align*}
\end{lemma}
This implies that when $p^\prime_{1i} \geq \max \{p_x, 1 - p_x\}$, then
\begin{align*}
    &\max \{0, \mathbb{P}(Z = 1 \mid X = 1, Y = i) - \mathbb{P}(Z = 0 \mid X = 0, Y = i)\}\\
    &= \mathbb{P}(Z = 1 \mid X = 1, Y = i) - \mathbb{P}(Z = 0 \mid X = 0, Y = i)
\end{align*}

Next, when $p^\prime_{1i} \leq \min\{p_x, 1 - p_x\}$, then consider the following Lemmas.
\begin{lemma}
    Assume $p_x > 1 - p_x$. If $p^\prime_{1i} < p_x$ for $i \in \{1, \dots , N\}$, then 
    \begin{align*}
            \frac{p^\prime_{11}}{p_x} > \frac{p^\prime_{1i} - (1 - p_x)}{p_x - (1 - p_x)}    
    \end{align*}
\end{lemma}
\begin{lemma}
    Assume $p_x > 1 - p_x$. If $p^\prime_{1i} \leq 1 - p_x$ for $i \in \{1, \dots , N\}$, then 
    \begin{align*}
            0 \geq \frac{p^\prime_{1i} - (1 - p_x)}{p_x - (1 - p_x)}    
    \end{align*}
\end{lemma}
This implies that when $p^\prime_{1i} \leq \min \{p_x, 1 - p_x\}$, then
\begin{align*}
    &\max \{0, \mathbb{P}(Z = 1 \mid X = 1, Y = i) - \mathbb{P}(Z = 0 \mid X = 0, Y = i)\} = 0
\end{align*}

And when $1 - p_x < p^\prime_{1i} < p_x$, then $\frac{p^\prime_{11}}{p_x} > \frac{p^\prime_{1i} - (1 - p_x)}{p_x - (1 - p_x)}$ and $\frac{p^\prime_{11} - (1 - p_x)}{p_x} < \frac{p^\prime_{1i} - (1 - p_x)}{p_x - (1 - p_x)}$. 

\subsection{Behavior of Max Operators in $\Delta$}

\begin{lemma}
    The function $\max \{0, \mathbb{P}(Z = 1 \mid X = 1, Y = 0) - \mathbb{P}(Z = 1 \mid X = 0, Y = 0)\} \geq 0$ when
    \begin{align*}
        p_{11} - p^\prime_{10}p_{y_0} \geq  \sum_{n = 1}^N p_{y_n}\mathbb{P}(Z = 1\mid X = 1, Y = n)
    \end{align*}
\end{lemma}

\begin{lemma}
    The following inequalities hold
    \begin{equation}
        p_{11} \geq p_{11} - p^\prime_{10}p_{y_0}
    \end{equation}
    \begin{equation}
        \frac{(1 - x)y_0 + p_{11}x - p^\prime_{10}y_0}{x} \geq p_{11} - p^\prime_{10}y_0
    \end{equation}
    \begin{equation*}
        p_{11} - p_{y_0} \leq p_{11} - p^\prime_{10}y_0
    \end{equation*}    
    \begin{equation*}
        \frac{p_{11}p_x - p^\prime_{10}p_{y_0}}{p_x} \leq p_{11} - p^\prime_{10}y_0
    \end{equation*}    
\end{lemma}
\begin{proof}
    \item The upper bound is $\frac{p_{11}}{y_1}$: Assume
        \begin{align*}
            \frac{p_{11}}{y_1} &< \frac{p_{11} - p^\prime_{10}y_0}{y_1}\\
            \implies & 0 < -\frac{p^\prime_{10}y_0}{y_1}
        \end{align*}
        This is a contradiction, hence
        \[
            \frac{p_{11}}{y_1} \geq \frac{p_{11} - p^\prime_{10}y_0}{y_1}
        \]
        \item The upper bound is $\frac{(1 - x)y_0 + p_{11}x - p^\prime_{10}y_0}{x}$: Assume
        \begin{align*}
            \frac{p_{11} - p^\prime_{10}y_0}{y_1} &> \frac{(1 - x)y_0 + p_{11}x - p^\prime_{10}y_0}{xy_1}\\
            p_{11} - p^\prime_{10}y_0 &> \frac{(1 - x)y_0 + p_{11}x - p^\prime_{10}y_0}{x}\\
            p_{11}x - p^\prime_{10}xy_0 &> (1 - x)y_0 + p_{11}x - p^\prime_{10}y_0\\
            - p^\prime_{10}xy_0 &> (1 - x)y_0 - p^\prime_{10}y_0\\
            p^\prime_{10}y_0(1 - x) &> (1 - x)y_0 \\
            \implies p^\prime_{10} &> 1 \\
        \end{align*}
\end{proof}


This Lemma implies that  $\max\{0, \mathbb{P}(Z = 1 \mid X = 1, Y = 0) - \mathbb{P}(Z = 1 \mid X = 0, Y = 0)\}$ can be either zero or non-zero over the range of the free parameters. 

Now, we similarly examine the behavior of $\max \{0, \mathbb{P}(Z = 1 \mid X = 1, Y = i) - \mathbb{P}(Z = 1 \mid X = 0, Y = i)\}$.

\begin{lemma}
    The function $\max \{0, \mathbb{P}(Z = 1 \mid X = 1, Y = i) - \mathbb{P}(Z = 1 \mid X = 0, Y = i)\} \geq 0$ for $i \in \{1, \dots, N\}$ when
    \begin{equation*}
        p^\prime_{1i} \leq P(Z = 1 \mid X = 1, Y = 1)
    \end{equation*}
\end{lemma}

\begin{lemma}
    The following inequalities hold
    \begin{align*}
            1 &\geq p^\prime_{1i}\\
            \frac{p^\prime_{1i}}{p_x} &\geq p^\prime_{1i}\\
            0 &\leq p^\prime_{1i}\\
            \frac{p^\prime_{1i} - (1 - p_x)}{p_x} &\leq p^\prime_{1i}
    \end{align*}
\end{lemma}
This Lemma implies that  $\max\{0, \mathbb{P}(Z = 1 \mid X = 1, Y = i) - \mathbb{P}(Z = 1 \mid X = 0, Y = i)\}$ can be either zero or non-zero over the range of the free parameters.   
\subsection{Behavior of Upper Bound on PNS Under Special Conditions}

Here we analyze the behavior of the upper bound on the PNS in Theorem 1 under certain conditions, since these will be used in the proof of Theorem 1.

\begin{lemma}
    Given the upper bound in Theorem 2 on PNS, when $p_x > 1 - p_x$ and all $p^\prime_{1i} \geq p_x$ for $i \in \{0, \dots, N\}$ and , then 
    \[
    p_{00} < p_{11} - \sum_{i = 0}^N \Phi_i
    \]
\end{lemma}

\begin{proof}
    Since $p^\prime_{1i} \geq p_x$ for all $i$, then all the indicators will evaluate to $1$, as a result $p_{11} - \sum_{i = 0}^N \Phi_i$ will equal
    \begin{align*}
        &p_{11} - \sum_{i = 0}^N \frac{p_{y_i}(p^\prime_{1i} - p_x)}{1 - p_x}\\
        &\implies = \frac{p_{11}(1 - p_x) - \sum_{i = 0}^N p_{y_i}(p^\prime_{1i} - p_x)}{1 - p_x}\\
        &\implies = \frac{p_{11}(1 - p_x) - p_{11}p_x - p_{10}(1 - p_x) + p_x}{1 - p_x}\\
        &\implies = \frac{p_{11}(1 - p_x) - p_{11}p_x + p_{00}(1 - p_x) - (1 - p_x) + p_x}{1 - p_x}\\
        &\implies = p_{01}(\frac{p_x}{1 - p_x} - 1) + p_{00}\\
    \end{align*}
    And since $p_x > 1 - p_x$, this quantity will be greater than $p_{00}$.
\end{proof}

\begin{lemma}
    Given the upper bound in Theorem 2 on PNS, when $p_x > 1 - p_x$ and $p^\prime_{1i} \leq 1 - p_x$ for $i \in \{0, \dots, N\}$ and , then 
    \[
    p_{00} - \sum_{i = 0}^N \Theta_i> p_{11}
    \]
\end{lemma}

\begin{proof}
Since $p^\prime_{1i} \leq 1 - p_x$ for all $i$, then all the indicators will evaluate to $1$, as a result $p_{00} - \sum_{i = 0}^N \Theta_i$ will equal
\begin{align*}
    &p_{00} - \sum_{i = 0}^N \frac{p_{y_i}((1 - p_x) - p^\prime_{1i})}{1 - p_x}\\
    &\implies = \frac{p_{00}(1 - p_x) - (1 - p_x) + \sum_{i = 0}^N p_{y_i}p^\prime_{1i}}{1 - p_x}
    &\implies = \frac{-p_{10}(1 - p_x) + \sum_{i = 0}^N p_{y_i}p^\prime_{1i}}{1 - p_x}\\
    &\implies = \frac{p_{11}p_x}{1 - p_x}
\end{align*}
And since $p_x > 1 - p_x$, this concludes the proof.
\end{proof}
%%%%%%%%%%%%%%%%%%%%%%%%%%%%%%%%%%%%%%%%%%%%%%%%%%%%%%%%%%%%%%%%%%%%%%%%%%%%%%

\begin{lemma}
    Given the upper bound in Theorem 2 on PNS, when $p_x < 1 - p_x$ and all $p^\prime_{1i} \geq 1 - p_x$ for $i \in \{0, \dots, N\}$ and , then 
    \[
    p_{00} < p_{11} - \sum_{i = 0}^N \Phi_i
    \]
\end{lemma}

\begin{proof}
    Since $p^\prime_{1i} \geq 1 - p_x$ for all $i$, then all the indicators will evaluate to $1$, as a result $p_{11} - \sum_{i = 0}^N \Phi_i$ will equal
    \begin{align*}
        &p_{11} - \sum_{i = 0}^N \frac{p_{y_i}(p^\prime_{1i} - (1 - p_x))}{p_x}\\
        &\implies = \frac{p_{11}p_x - \sum_{i = 0}^N p_{y_i}(p^\prime_{1i} - (1 - p_x))}{p_x}\\
        &\implies = \frac{p_{11}p_x - p_{11}p_x - p_{10}(1 - p_x) + (1 - p_x)}{p_x}\\
        &\implies = \frac{p_{00}(1 - p_x)}{p_x}
    \end{align*}
    And since $p_x < 1 - p_x$, this quantity will be greater than $p_{00}$.
\end{proof}

\begin{lemma}
    Given the upper bound in Theorem 2 on PNS, when $p_x < 1 - p_x$ and $p^\prime_{1i} \leq p_x$ for $i \in \{0, \dots, N\}$ and , then 
    \[
    p_{00} - \sum_{i = 0}^N \Theta_i> p_{11}
    \]
\end{lemma}

\begin{proof}
Since $p^\prime_{1i} \leq p_x$ for all $i$, then all the indicators will evaluate to $1$, as a result $p_{00} - \sum_{i = 0}^N \Theta_i$ will equal
\begin{align*}
    &p_{00} - \sum_{i = 0}^N \frac{p_{y_i}(p_x - p^\prime_{1i})}{p_x}\\
    &\implies = \frac{p_{00}p_x - p_x + \sum_{i = 0}^N p_{y_i}p^\prime_{1i}}{p_x}\\
    &\implies = \frac{-p_{10}p_x + p_{10}(1 - p_x)}{p_x} + p_{11}\\
    &\implies = p_{10}(\frac{1 - p_x}{p_x} - 1) + p_{11}
\end{align*}
And since $1 - p_x > p_x$, the ineqality holds.
\end{proof}

\begin{lemma}
    Assume $p_x > 1 - p_x$. Assume all $1 - p_x < p^\prime_{1i} < p_x$. Then all max operators to can open simultaneously if and only if $\Phi_X \geq 0$. 
\end{lemma}

\begin{proof}
    To prove an if and only if, we first show that all max operators opening implies $p_{11} + p_{10} - 1 \geq 0$, and then the other way round. 

    Starting with the first, note that for all max operators to open simultaneously, the following conditions must hold
\begin{align*}
    \sum_{n = 1}^N p_{y_n}P(Z = 1 \mid X = 1, Y = n) \geq \frac{p_{y_0}((1 - p_x) - p^\prime_{10})}{p_x - (1 - p_x)} + p_{11}
\end{align*}
And for all $i \in \{1, \dots N\}$
\begin{align*}
    P(Z = 1 \mid X = 1, Y = i) \leq \frac{p^\prime_{1i} - (1 - p_x)}{p_x - (1 - p_x)}    
\end{align*}

This is equivalent to
\begin{align*}
    &\frac{p_{y_0}((1 - p_x) - p^\prime_{10})}{p_x - (1 - p_x)} + p_{11} \leq \sum_{i = 1}^N p_{y_i}\frac{p^\prime_{1i} - (1 - p_x)}{p_x - (1 - p_x)}\\
    &\implies p_{y_0}((1 - p_x) - p^\prime_{10}) + p_{11}(p_x - (1 - p_x)) +  \leq \sum_{i = 1}^N p_{y_i}(p^\prime_{1i} - (1 - p_x))\\
    &\implies (1 - p_x) + p_{11}(p_x - (1 - p_x)) +  \leq \sum_{i = 1}^N p_{y_i}p^\prime_{1i} + p^\prime_{10}p_{y_0}\\
    &\implies (1 - p_x) - p_{11}(1 - p_x) +  \leq p_{10}(1 - p_x)\\
    &\implies 0 \leq p_{11} + p_{10} - 1
\end{align*}

Next, to prove the backward implication, we utilize a proof by contrapositive, i.e. we must prove that .  
\[
\frac{p_{y_0}((1 - p_x) - p^\prime_{10})}{p_x - (1 - p_x)} + p_{11} > \sum_{i = 1}^N p_{y_i}\frac{p^\prime_{1i} - (1 - p_x)}{p_x - (1 - p_x)} \implies p_{11} + p_{10} - 1 < 0
\]

To see this, note that
\begin{align*}
    &\frac{p_{y_0}((1 - p_x) - p^\prime_{10})}{p_x - (1 - p_x)} + p_{11} > \sum_{i = 1}^N p_{y_i}\frac{p^\prime_{1i} - (1 - p_x)}{p_x - (1 - p_x)}\\
    &\implies p_{y_0}((1 - p_x) - p^\prime_{10}) + p_{11}(p_x - (1 - p_x)) > \sum_{i = 1}^N p_{y_i}(p^\prime_{1i} - (1 - p_x))\\
    &\implies (1 - p_x)  - p_{11}(1 - p_x) > p_{10}p_x\\
    &\implies 0  > p_{11} + p_{10} - 1
\end{align*}

\end{proof}

\begin{lemma}
    All max operators in $\Delta$ can open simultaneously if and only if $p_{11} - p_{10} \geq 0$. 
\end{lemma}

\begin{proof}
To prove an if and only if, we first show that all max operators opening implies $p_{11} - p_{10} \geq 0$, and then the other way round. 

Starting with the first, note that for all max operators to open simultaneously, the following conditions must hold
\begin{align*}
    p_{11} - p^\prime_{10}p_{y_0} \geq  \sum_{n = 1}^N p_{y_n}\mathbb{P}(Z = 1\mid X = 1, Y = n)
\end{align*}
And for all $i \in \{1, \dots N\}$
\begin{align*}
    P(Z = 1 \mid X = 1, Y = i) \geq p^\prime_{1i}
\end{align*}

This is equivalent to
\begin{align*}
    &\sum_{i = 1}^N p_{y_i}p^\prime_{1i} \leq p_{11} - p^\prime_{10}p_{y_0}\\
    &\implies \sum_{i = 0}^N p_{y_i}p^\prime_{1i} \leq p_{11} \\
    &\implies p_{11}p_x + p_{10}(1 - p_x) \leq p_{11} \\
    &\implies 0 \leq (1 - p_x)(p_{11} - p_{10})\\
\end{align*}

This proves the forward implication. A similar proof for the backward implication can be provided using a proof by contra positive as well, concluding the proof for this lemma. 
\end{proof}

\section{Proof of Theorem 4}
We start by expressing bounds on the joint probability $P(Z_{\mathbf{x}} = 1, Z_{\mathbf{x^\prime}} = 0, C, Y)$ as
{\small
\begin{equation*}
    \max\begin{bmatrix}
        0\\
        P(Z_{\mathbf{x}} = 1, C, Y) - P(Z_{\mathbf{x^\prime}} = 1, C, Y)
        \end{bmatrix} \leq P(Z_{\mathbf{x}} = 1, Z_{\mathbf{x^\prime}} = 0, C, Y)
        \leq \min \begin{bmatrix}
            P(Z_{\mathbf{x}} = 1, C, Y)\\
            P(Z_{\mathbf{x^\prime}} = 0, C, Y)
        \end{bmatrix}
    
\end{equation*}
}
Where the upper bound follows from $P(A, B) \leq \min\{P(A), P(B)\}$ for random variables $A$ and $B$. The lower bound is proved below. 
\begin{align*}
    P(Z_{\mathbf{x}} = 1, C, Y) - P(Z_{\mathbf{x^\prime}} = 1, C, Y)  &= 
    P(Z_{\mathbf{x}} = 1, Z_{\mathbf{x'}} = 0, C, Y) + P(Z_{\mathbf{x}} = 1, Z_{\mathbf{x'}} = 1, C, Y)\\
    &- P(Z_{\mathbf{x}} = 1, Z_{\mathbf{x'}} = 1, C, Y) - P(Z_{\mathbf{x}} = 0, Z_{\mathbf{x'}} = 1, C, Y)\\
    &= P(Z_{\mathbf{x}} = 1, Z_{\mathbf{x'}} = 0, C, Y) - P(Z_{\mathbf{x}} = 0, Z_{\mathbf{x'}} = 1, C, Y)
\end{align*}

And since probabilities are non-negative, we obtain the lower bound
\[
\max \begin{bmatrix}
    0\\
    P(Z_{\mathbf{x}} = 1, C, Y) - P(Z_{\mathbf{x^\prime}} = 1, C, Y) 
\end{bmatrix} \leq P(Z_{\mathbf{x}} = 1, Z_{\mathbf{x'}} = 0, C, Y)
\]
Next, the $PNS$ is obtained by marginalizing out $C$ and $Y$, giving a lower bound of
\begin{align*}
    &\sum_{C, Y}\max\begin{bmatrix}
                        0\\
                        P(Z_{\mathbf{x}} = 1, C, Y) - P(Z_{\mathbf{x^\prime}} = 1, C, Y)
                    \end{bmatrix} \leq P(Z_{\mathbf{x}} = 1, Z_{\mathbf{x^\prime}} = 0)
\end{align*}
And the upper bound is given as 
\begin{align*}
    & P(Z_{\mathbf{x}} = 1, Z_{\mathbf{x^\prime}} = 0) \leq \sum_{C, Y}\min \begin{bmatrix}
        P(Z_{\mathbf{x}} = 1, C, Y)\\
        P(Z_{\mathbf{x^\prime}} = 0, C, Y)
    \end{bmatrix}
\intertext{Since $Z_{\mathbf{x}} \independent X$, an application of consistency allows the above bounds to be re-written as}
    &\sum_{C, Y}P(C, Y)\max\begin{bmatrix}
                                0\\
                                P(Z = 1 \mid X = 1, C, Y) - P(Z = 1 \mid X = 0, C, Y)
                            \end{bmatrix} \leq P(Z_{\mathbf{x}} = 1, Z_{\mathbf{x^\prime}} = 0)\\
    &P(Z_{\mathbf{x}} = 1, Z_{\mathbf{x^\prime}} = 0) \leq \sum_{C, Y} P(C, Y)\min
    \begin{bmatrix}
        P(Z = 1 \mid X = 1, C, Y)\\
        P(Z = 0 \mid X = 0, C, Y)
    \end{bmatrix}
\end{align*}
Exploiting the independence of $C$ and $Y$, the lower bound is written as
 \begin{align*}
    \sum_{C}P(C) \Delta_C \leq &P(Z_{\mathbf{x}} = 1, Z_{\mathbf{x^\prime}} = 0)\\
    \intertext{Where}
    \Delta_C = P(Y)\max\{0, P(Z = 1 \mid X = 1, C, Y)& - P(Z = 1 \mid X = 0, C, Y)\}\\ 
\end{align*}   
Next, the minimum operator in the upper bound can be re-written as
\begin{align*}
    &\min
    \begin{bmatrix}
        P(Z = 1 \mid X = 1, C, Y)\\
        P(Z = 0 \mid X = 0, C, Y)
    \end{bmatrix}\\
    &= P(Z = 1 \mid X = 1, C, Y) 
    - \max\begin{bmatrix}
          0\\
          P(Z = 1 \mid X = 1, C, Y) - P(Z = 0 \mid X = 0, C, Y)
          \end{bmatrix}
\end{align*}
Consequently, the upper bound is expressed as
\begin{align*}
   &P(Z_{\mathbf{x}} = 1, Z_{\mathbf{x^\prime}} = 0) \leq P(Z = 1\mid X = 1) - \sum_C P(C)\Gamma_C\\
   \intertext{Where}
   &\Gamma_C = P(Y)\max \{0, P(Z = 1 \mid X = 1, C, Y) - P(Z = 0 \mid X = 0, C, Y) \}
\end{align*}
This concludes the proof of Theorem 4. 


\section{Proof of Lemma 5}

The  bounds on PNS in Equation 2 are given as
\begin{equation}\label{eq:pns-dawid-bounds}
    \Delta \leq PNS \leq P(Z = 1 \mid X = 1) - \Gamma
\end{equation}
Where
\begin{align*}
    \Delta &= \sum_c \mathbb{P}(C = c)\max \{0, \mathbb{P}(Z = 1 \mid X = 1, C = c) - \mathbb{P}(Z = 1 \mid X = 0, C = c)\} \\
    \Gamma &= \sum_c \mathbb{P}(C = c)\max \{0, \mathbb{P}(Z = 1 \mid X = 1, C = c)
     - \mathbb{P}(Z = 0 \mid X = 0, C = c)\} 
\end{align*}


And the bounds in Lemma 5 are given as
    \begin{equation}\label{eq:trident-bounds}
        \sum_{C}P(C)\Delta_C \leq PNS \leq P(Z = 1 \mid X = 1) - \sum_{C}P(C)\Gamma_C
    \end{equation}
Where
\begin{align*}
    \Delta_C &= \sum_y \mathbb{P}(Y = y)\max \{0, \mathbb{P}(Z = 1 \mid X = 1, Y = y, C) - \mathbb{P}(Z = 1 \mid X = 0, Y = y, C)\} \\
    \Gamma_C &= \sum_y \mathbb{P}(Y = y)\max \{0, \mathbb{P}(Z = 1 \mid X = 1, Y = y, C) - \mathbb{P}(Z = 0 \mid X = 0, Y = y, C)\} 
\end{align*}

Starting with the lower bound, note that both lower bounds consist of an identical weighted sum $P(C)$, hence understanding the difference of these bounds comes down to examining $\max \{0, \mathbb{P}(Z = 1 \mid X = 1, C = c) - \mathbb{P}(Z = 1 \mid X = 0, C = c)\}$ versus $\sum_y \mathbb{P}(Y = y)\max \{0, \mathbb{P}(Z = 1 \mid X = 1, Y = y, C) - \mathbb{P}(Z = 1 \mid X = 0, Y = y, C)\}$. First, note that
\begin{align*}
&\mathbb{P}(Z = 1 \mid X = 1, C = c) - \mathbb{P}(Z = 1 \mid X = 0, C = c) =\\ &\sum_y P(Y = y)\Big(\mathbb{P}(Z = 1 \mid X = 1, Y = y, C) - \mathbb{P}(Z = 1 \mid X = 0, Y = y, C) \Big)
\end{align*}

Consequently, $\max \{0, \mathbb{P}(Z = 1 \mid X = 1, C = c) - \mathbb{P}(Z = 1 \mid X = 0, C = c)\}$ can be written as
\begin{align*}
    &\max \{0, \mathbb{P}(Z = 1 \mid X = 1, C = c) - \mathbb{P}(Z = 1 \mid X = 0, C = c)\}\\
    &= \max \Bigg\{0, \sum_y P(Y = y)\Big(\mathbb{P}(Z = 1 \mid X = 1, Y = y, C) - \mathbb{P}(Z = 1 \mid X = 0, Y = y, C) \Big)\Bigg\}
\end{align*}

And $\sum_y \mathbb{P}(Y = y)\max \{0, \mathbb{P}(Z = 1 \mid X = 1, Y = y, C) - \mathbb{P}(Z = 1 \mid X = 0, Y = y, C)\}$ is written as 
\begin{align*}
    \sum_y \max \{0, \mathbb{P}(Y = y) \Big(\mathbb{P}(Z = 1 \mid X = 1, Y = y, C) - \mathbb{P}(Z = 1 \mid X = 0, Y = y, C)\Big)\}
\end{align*}
Since the maximum of a sum is less than or equal to the sum of maximums, the lower bound in Equation \ref{eq:trident-bounds} will be greater than or equal to the lower bound in Equation \ref{eq:pns-dawid-bounds}. And when for any $C$, if for some values of $Y$, $\mathbb{P}(Z = 1 \mid X = 1, Y = y, C)$ is greater than $\mathbb{P}(Z = 1 \mid X = 0, Y = y, C)$, and form some values $\mathbb{P}(Z = 1 \mid X = 1, Y = y, C)$ is less than $\mathbb{P}(Z = 1 \mid X = 0, Y = y, C)$, than the lower bound in Equation \ref{eq:trident-bounds} will be greater than the lower bound in \ref{eq:pns-dawid-bounds}. 

A similar approach can be utilized for the upper bound as well, thereby completing the proof.

\section{Proof of Theorem 6}

\begin{lemma}\label{RREF-y-c}
    Let $X$ and $Z$ be binary random variables, and let $C$ and $Y$ be discrete random variables taking values in $\{0, \dots, M\}$ and $\{0, \dots , N\}$ respectively. Let $\delta^C_X$ represent the link between the treatment assignment mechaism between the $P^E$ and $P^T$ as follows
    \[
    P^E(X = 1\mid C) = P^T(X = 1) + \delta^C_X
    \]
    For notational ease, we introduce the following terms. Let $P^T(Z = 1 \mid X = j, C = i)$ be denoted by $p^T{1ji}$ and let $P^E(Z = 1 \mid Y = j, C = i)$ be denoted as $p^E_{1ji}$. Given distributions $P^T(Z, X, C)$ and $P^E(Z, Y, C)$ obeying the following contraints
    \begin{align*}
        p^T_{10i} &= \sum_{j = 0}^N P(Z = 1\mid X = 0, Y = j, C = i)p_{y_j}\\
        p^T_{11i} &= \sum_{j = 0}^N P(Z = 1\mid X = 1, Y = j, C = i)p_{y_j}\\
        p^E_{10i} &= P(Z = 1\mid X = 0, Y = 0, C = i)(1 - p_x - \delta^i_X)\\
        &\hspace{0.2in} + P(Z = 1\mid X = 1, Y = 0, C = i)(p_x + \delta^i_X)\\
        \vdots\\
        p^E_{1Ni} &= P(Z = 1\mid X = 0, Y = N, C = i)(1 - p_x - \delta^i_X)\\
        &\hspace{0.2in} + P(Z = 1\mid X = 1, Y = N, C = i)(p_x + \delta^i_X)\\
    \end{align*}
    Then this system of equations can be expressed in terms of free parameters $P(Z = 1 \mid X = 1, Y = i, C)$ for $i \in \{1, \dots, N\}$ and all $C$ as
    {\small
    \begin{align*}
    \mathbb{P}(Z = 1 \mid X = 0, Y = 0, C) &=  \frac{p_x + \delta^C_X}{1 - p_x - \delta^C_X}\sum_{n = 1}^N\frac{p_{y_n}}{p_{y_0}}\mathbb{P}(Z = 1 \mid X = 1, Y = n, C) + \frac{p^E_{10C}p_{y_0} - p^T_{11C}(p_x +\delta^C_X)}{(1 - p_x - \delta^C_X)p_{y_0}}\\
    \mathbb{P}(Z = 1 \mid X = 1, Y = 0, C)&= \frac{p^T_{11C}}{p_{y_0}} - \sum_{n = 1}^N\frac{p_{y_n}}{p_{y_0}}\mathbb{P}(Z = 1 \mid X = 1, Y = n, C)\\
    \mathbb{P}(Z = 1 \mid X = 0, Y = 1, C)&= \frac{p^E_{11C}}{1 - p_x - \delta^C_X} - \frac{p_x + \delta^C_X}{1 - p_x - \delta^C_X}\mathbb{P}(Z = 1 \mid X = 1, Y = 1, C)\\
    \mathbb{P}(Z = 1 \mid X = 0, Y = 2, C)&= \frac{p^E_{12C}}{1 - p_x - \delta^C_X} - \frac{p_x + \delta^C_X}{1 - p_x - \delta^C_X}\mathbb{P}(Z = 1 \mid X = 1, Y = 2, C)\\
    \vdots\\
    \mathbb{P}(Z = 1 \mid X = 0, Y = N, C)&= \frac{p^E_{1N}}{1 - p_x - \delta^C_X} - \frac{p_x + \delta^C_X}{1 - p_x - \delta^C_X}\mathbb{P}(Z = 1 \mid X = 1, Y = N, C)\\
    \end{align*}
    }
\end{lemma}

\begin{lemma}\label{lem:free-param-bounds-delta}
To ensure the solution to the system of equations in Lemma \ref{lemma:RREF-y-c} form coherent probabilities, the following bounds on the free parameters must hold for all $C$
{\small
\begin{align}\label{eq:sum-bounds}
\max\begin{bmatrix}
   \frac{p^T_{11C}(p_x + \delta^C_X) - p^E_{10C}p_{y_0}}{p_x + \delta^C_X} \\
   p^T_{11C} - p_{y_0}
\end{bmatrix} \leq \sum_{n = 1}^N y_nP^T(Z = 1 \mid X = 1, Y = n, C) 
\leq \min\begin{bmatrix}
    \frac{(1 - p_x - \delta^C_X)p_{y_0} + p^T_{11C}(p_x + \delta^C_X) - p^E_{10C}p_{y_0}}{p_x + \delta^C_X}\\
    p^T_{11C}
\end{bmatrix}
\end{align}
}

And for each $i \in \{1, \dots, N\}$, we the bounds on the following free parameters $P(Z = 1\mid X = 1, Y = i, C)$
\begin{align}\label{eq:individual-bounds}
    \max\begin{bmatrix}
        0\\
        \frac{p^E_{1iC} - (1 - p_x - \delta^C_X)}{p_x + \delta^C_X}
    \end{bmatrix}
        \leq P^T(Z = 1\mid X = 1, Y = i, C) \leq 
    \min\begin{bmatrix}
        1\\
        \frac{p^E_{1iC}}{p_x + \delta^C_X}
    \end{bmatrix}
\end{align}
\end{lemma}

\begin{lemma}
Using the solution to the system of equations in Lemma \ref{lemma:RREF-y-delta}, each of the terms in $\Delta_C$ and $\Gamma_C$ defined in Lemma XXXX are expressed in terms of the free parameters below. 
\begin{enumerate}
    \item For the term in $\Gamma$ corresponding to $Y = 0$
    \begin{align*}
        &\mathbb{P}(Z = 1 \mid X = 1, Y = 0, C) - \mathbb{P}(Z = 0 \mid X = 0, Y = 0, C)\\
        &=\frac{p^E_{10C} - (1 - p_x - \delta^C_X)}{1 - p_x - \delta^C_X} + \frac{\sum_{n = 1}^N p_{y_n}P^T(Z = 1 \mid X = 1, Y = n, C) - p^T_{11C}}{p_{y_0}}\Bigg(\frac{p_x + \delta^C_X}{1 - p_x - \delta^C_X} - 1\Bigg) 
    \end{align*}
    
\item For the terms in $\Gamma$ corresponding to $Y = i$, $i \in \{1, \dots , N\}$
    \begin{align*}
        &P(Z = 1 \mid X = 1, Y = i, C) - P(Z = 0 \mid X = 0, Y = i, C)\\
        &= P(Z = 1 \mid X = 1, Y = i, C)\Bigg(1 - \frac{p_x + \delta^C_X}{1 - p_x - \delta^C_X}\Bigg) + \frac{p^E_{11C} - (1 - p_x - \delta^C_X)}{1 - p_x - \delta^C_X}\\
    \end{align*}
\item For the term in $\Delta$ corresponding to $Y = 0$:
    \begin{align*}
        &\mathbb{P}(Z = 1 \mid X = 1, Y = 0, C) - \mathbb{P}(Z = 1 \mid X = 0, Y = 0, C)\\
        &= \frac{p^T_{11C} - p^E_{10C}p_{y_0} - \sum_{n = 1}^N p_{y_n}P^T(Z = 1\mid X = 1, Y = n, C)}{(1 - p_x - \delta^C_X)p_{y_0}}
    \end{align*}
\item For the term in $\Delta$ corresponding to $Y = i$, $i \in \{1, \dots , N\}$
    \begin{align*}
        &\mathbb{P}(Z = 1 \mid X = 1, Y = i, C) - \mathbb{P}(Z = 1 \mid X = 0, Y = i, C)\\
        &=\frac{P^T(Z = 1 \mid X = 1, Y = i, C) - p^E_{1iC}}{1 - p_x - \delta^C_X}
    \end{align*}
\end{enumerate}
\end{lemma}

% \begin{proof}
%     Using the system of equations obtained in Lemma \ref{lemma:RREF-y-delta}, each term in $\Gamma$ can be expressed using these free parameters. 
% \begin{enumerate}
%     \item $\max \{0, \mathbb{P}(Z = 1 \mid X = 1, Y = 0) - \mathbb{P}(Z = 0 \mid X = 0, Y = 0)\}$
%     \begin{equation}\label{eq:Gamma-y0-1}
%         P^T(Z = 1 \mid X = 1, Y = 0) &= \frac{p^T_{11}}{p_{y_0}} - \sum_{n = 1}^N\frac{p_{y_n}}{p_{y_0}}P^T(Z = 1 \mid X = 1, Y = n)
%     \end{equation}
%     \begin{align}\label{eq:Gamma-y0-2}
%         &P^T(Z = 0 \mid X = 0, Y = 0) = 1 -\\
%         &\Bigg(\frac{p_x + \delta_X}{1 - p_x - \delta_X}\sum_{n = 1}^N\frac{p_{y_n}}{p_{y_0}}P^T(Z = 1 \mid X = 1, Y = n) + \frac{p^E_{10}p_{y_0} - p^T_{11}(p_x + \delta_X)}{(1 - p_x - \delta_X)p_{y_0}}\Bigg)
%     \end{align}
%     Subtracting these two and following a similar calculation as Lemma XXXX, this simplifies to
%     \begin{align*}
%     \frac{p^E_{10} - (1 - p_x - \delta_X)}{1 - p_x - \delta_X} + \frac{\sum_{n = 1}^N p_{y_n}P^T(Z = 1 \mid X = 1, Y = n) - p^T_{11}}{p_{y_0}}\Bigg(\frac{p_x + \delta_X}{1 - p_x - \delta_X} - 1\Bigg) 
%     \end{align*}


%     \item $\max\{0, P(Z = 1 \mid X = 1, Y = i) - P(Z = 0 \mid X = 0, Y = i)\}$: The probability $P(Z = 0 \mid X = 0, Y = i)$ for $i \in \{1, \dots ,N\}$ can be expressed in terms of the free parameters as
%     \begin{align*}
%         &P(Z = 0 \mid X = 0, Y = i) = 1 -\Bigg( \frac{p^E_{1i}}{1 - p_x - \delta_X} - \frac{p_x + \delta_X}{1 - p_x - \delta_X}P^T(Z = 1 \mid X = 1, Y = i)\Bigg)\\
%         &\implies P(Z = 1 \mid X = 1, Y = i) - P(Z = 0 \mid X = 0, Y = i) \\
%         &= P^T(Z = 1 \mid X = 1, Y = i) - 1 + \frac{p^E_{1i}}{1 - p_x - \delta_X} - \frac{p_x + \delta_X}{1 - p_x - \delta_X}P(Z = 1 \mid X = 1, Y = i)\\
%         &= P(Z = 1 \mid X = 1, Y = i)\Bigg(1 - \frac{p_x + \delta_X}{1 - p_x - \delta_X}\Bigg) + \frac{p^E_{11} - (1 - p_x - \delta_X)}{1 - p_x - \delta_X}
%     \end{align*}
% \end{enumerate}
%     This concludes the proof for the terms in $\Gamma$. Next, enumerating the calculations for the terms in $\Delta$.
%     \begin{enumerate}
%         \item $\mathbb{P}(Z = 1 \mid X = 1, Y = 0) - \mathbb{P}(Z = 1 \mid X = 0, Y = 0)$
%         \begin{align*}
%         &= \frac{p^T_{11}}{p_{y_0}} - \sum_{n = 1}^N\frac{p_{y_n}}{p_{y_0}}P^T(Z = 1 \mid X = 1, Y = n)\\
%         & - \Bigg(\frac{p_x + \delta_X}{1 - p_x - \delta_X}\sum_{n = 1}^N\frac{p_{y_n}}{p_{y_0}}\mathbb{P}(Z = 1 \mid X = 1, Y = n)
%         + \frac{p^E_{10}p_{y_0} - p^T_{11}(p_x + \delta_X)}{(1 - p_x - \delta_X))p_{y_0}}\Bigg)\\
%         &= \frac{p^T_{11} - p^E_{10}p_{y_0} - \sum_{n = 1}^N p_{y_n}P^T(Z = 1\mid X = 1, Y = n)}{(1 - p_x - \delta_X)p_{y_0}}
%     \end{align*}
%     \item $\max\{0, \mathbb{P}(Z = 1 \mid X = 1, Y = i) - \mathbb{P}(Z = 1 \mid X = 0, Y = i)\}$ for $i \in \{1, \dots, N\}$
%     \begin{align*}
%         &P^T(Z = 1 \mid X = 0, Y = i) = \frac{p^E_{1i}}{1 - p_x - \delta_X} - \frac{p_x + \delta_X}{1 - p_x - \delta_X}P^T(Z = 1 \mid X = 1, Y = i)\\
%         &\implies P^T(Z = 1 \mid X = 1, Y = i) - P^T(Z = 1 \mid X = 0, Y = i)\\
%         &= P^T(Z = 1 \mid X = 1, Y = i) - \frac{p^E_{1i}}{1 - p_x - \delta_X} + \frac{p_x + \delta_X}{1 - p_x - \delta_X}P^T(Z = 1 \mid X = 1, Y = i)\\
%         &= \frac{P^T(Z = 1 \mid X = 1, Y = i) - p^E_{1i}}{1 - p_x - \delta_X}
%     \end{align*}
%     \end{enumerate}
%     This concludes the proof of the Lemma.
% \end{proof}

\section{Proofs For Lemmas}\label{sec:lemma-proofs}

% \begin{lemma}
% Let $X$ and $Z$ be binary random variables, and let $Y$ be a discrete random variable taking on values in $0, \dots ,N$. Let $X$, $Y$ and $Z$ obey the causal structure in \ref{v-structure}. Then, given marginals $P(Z, X)$ and $P(Z, Y)$, the conditional distributions $P(Z \mid X, Y)$ can be expressed in terms of free parameters $P(Z = 1 \mid X = 1, Y = i)$ for $i \in \{1, \dots, N\}$ as

% {\small
% \begin{align*}
% \mathbb{P}(Z = 1 \mid X = 0, Y = 0) &=  \frac{p_x}{1 - p_x}\sum_{n = 1}^N\frac{p_{y_n}}{p_{y_0}}\mathbb{P}(Z = 1 \mid X = 1, Y = n) + \frac{p^\prime_{10}p_{y_0} - p_{11}p_x}{(1 - p_x)p_{y_0}}\\
% \mathbb{P}(Z = 1 \mid X = 1, Y = 0)&= \frac{p_{11}}{p_{y_0}} - \sum_{n = 1}^N\frac{p_{y_n}}{p_{y_0}}\mathbb{P}(Z = 1 \mid X = 1, Y = n)\\
% \mathbb{P}(Z = 1 \mid X = 0, Y = 1)&= \frac{p^\prime_{11}}{1 - p_x} - \frac{p_x}{1 - p_x}\mathbb{P}(Z = 1 \mid X = 1, Y = 1)\\
% \mathbb{P}(Z = 1 \mid X = 0, Y = 2)&= \frac{p^\prime_{12}}{1 - p_x} - \frac{p_x}{1 - p_x}\mathbb{P}(Z = 1 \mid X = 1, Y = 2)\\
% \vdots\\
% \mathbb{P}(Z = 1 \mid X = 0, Y = N)&= \frac{p^\prime_{1N}}{1 - p_x} - \frac{p_x}{1 - p_x}\mathbb{P}(Z = 1 \mid X = 1, Y = N)\\
% \end{align*}
% }

% Where $P(X = 1)$ is denoted as $p_x$ , $P(Y = n)$ is denoted as $p_{y_n}$, $P(Z = 1 \mid X = 1)$ is denoted as $p_{11}$, $P(Z = 1 \mid X = 0)$ is denoted as $p_{10}$, and $P(Z = 1 \mid Y = n)$ is denoted as $p^\prime_{1n}$ for $n \in \{0, \dots, N\}$.
% \end{lemma}

\textbf{Proof for Lemma \ref{lemma:RREF-y}:} This lemma is proved using mathematical induction performed on the the Reduced Row Echelon Form (RREF) of the matrix representation of the system of equations that in Equation X that impose constraints on $P(Z \mid X , Y)$ using $P(Z, X)$ and $P(Z, Y)$. 

Using the invariances defined in Section X, we obtain the following equations for $P(Z = 1 \mid X, Y)$ in terms of $P(Z, X)$ and $P(Z, Y)$. For ease of notation, we introduce the following terms. $P(X = 1)$ is denoted as $p_x$ , $P(Y = n)$ is denoted as $p_{y_n}$, $P(Z = 1 \mid X = 1)$ is denoted as $p_{11}$, $P(Z = 1 \mid X = 0)$ is denoted as $p_{10}$, and $P(Z = 1 \mid Y = n)$ is denoted as $p^\prime_{1n}$ for $n \in \{0, \dots, N\}$.

\begin{align*}
    p_{10} &= \sum_{i = 0}^N P(Z = 1\mid X = 0, Y = n)p_{y_n}\\
    p_{11} &= \sum_{n = 0}^N P(Z = 1\mid X = 1, Y = n)p_{y_n}\\
    p^\prime_{10} &= P(Z = 1\mid X = 0, Y = 0)(1 - p_x) + P(Z = 1\mid X = 1, Y = 0)p_x\\
    \vdots\\
    p^\prime_{1N} &= P(Z = 1\mid X = 0, Y = N)(1 - p_x) + P(Z = 1\mid X = 1, Y = N)p_x\\
\end{align*}

The above equations can be represented in matrix form $A\mathbf{x} = b$ as
{\scriptsize
\begin{align*}
A &= \begin{bmatrix}
    p_{y_0} & 0 & p_{y_1} & 0 & \dots & p_{y_{N - 1}} & 0 & p_{y_N} & 0\\
    0 & p_{y_0} & 0 & p_{y_1} & \dots & 0 & p_{y_{N - 1}}& 0 & p_{y_N}\\
    1 - p_{x} & p_{x} & 0 & 0 & \dots & 0 & 0 & 0 & 0\\
    0 & 0 & 1 - p_x & p_x & \dots & 0 & 0 & 0 & 0\\
    \vdots & \ddots & & & & & & & \vdots\\
    0 & 0 & \dots & 0 & 0 & 1 - p_x & p_x & 0 & 0\\
    0 & 0 & \dots & 0 & & 0 & 0 & 1 - p_x & p_x\\
\end{bmatrix}\\
b &= \begin{bmatrix}
    p_{10}\\
    p_{11}\\
    p^\prime_{10}\\
    p^\prime_{11}\\
    p^\prime_{12}
    \vdots\\
    p^\prime_{1(N - 1)}\\
    p^\prime_{1N}\\
\end{bmatrix}
\hspace{0.5in}\mathbf{x} 
= \begin{bmatrix}
P(Z = 1 \mid X = 0, Y = 0)\\    
P(Z = 1 \mid X = 1, Y = 0)\\
P(Z = 1 \mid X = 0, Y = 1)\\    
P(Z = 1 \mid X = 1, Y = 1)\\
\vdots\\
P(Z = 1 \mid X = 0, Y = N)\\    
P(Z = 1 \mid X = 1, Y = N)\\
\end{bmatrix}
\end{align*}
}
Next, denote the augmented matrix $A | b$ as 
\begin{align*}
    \begin{bmatrix}[ccccccccc|c]
    p_{y_0} & 0 & p_{y_1} & 0 & \dots & p_{y_{N - 1}} & 0 & p_{y_N} & 0 & p_{10}\\
    0 & p_{y_0} & 0 & p_{y_1} & \dots & 0 & p_{y_{N - 1}}& 0 & p_{y_N} & p_{11}\\
    1 - p_x & p_x & 0 & 0 & \dots & 0 & 0 & 0 & 0 & p^\prime_{10}\\
    0 & 0 & 1 - p_x & p_x & \dots & 0 & 0 & 0 & 0 & p^\prime_{11}\\
    \vdots & \ddots & & & & & & & \vdots & \vdots \\
    0 & 0 & \dots & 0 & 0 & 1 - p_x & p_x & 0 & 0 & p^\prime_{1(N - 1)}\\
    0 & 0 & \dots & 0 & & 0 & 0 & 1 - p_x & p_x & p^\prime_{1N}\\
    \end{bmatrix}
\end{align*}

The augmented matrix $A | b$ when expressed in RREF will express the system of equations in terms of basic variables and free parameters. Then, this can be compared to the system of equations presented in the Lemma to complete the proof.  

First, we utilize mathematical induction to provide a general form for the RREF of $A|b$ for any $N$. Formally, let $P(N)$ denote the following proposition. \\
\textbf{Proposition}: Let $P(N)$ denote the proposition that when $X$ and $Z$ are binary, and $Y$ has support in $\{ 0, \dots, N\}$, then $A|b$ will be a matrix with $N + 3$ rows and $2(N + 1) + 1$ columns. The following steps when executed will put $A|b$ in RREF, where $R_i$ denotes the $i$-th row of $A|b$

\begin{enumerate}
    \item 
        \begin{align}
        R_1 &= R_1/p_{y_0}\\
        R_3 &= R_3 - (1 - p_x)R_1
        \end{align}\label{step-1}
    \item
        \begin{align}
        R_2 &= R_2/p_{y_0}\\
        R_3 &= R_3 - p_xR_2
        \end{align}\label{step-2}
    \item 
        \begin{align}
        R_3 &= R3/(-\frac{(1 - p_x)p_{y_1}}{p_{y_0}})\\
        R_1 &= R_1 - \frac{p_{y_1}}{p_{y_0}}R3\\
        R_4 &= R4 - (1 - p_x)R3
        \end{align}\label{step-3}
    \item If $N \geq 2$, then loop through the following steps for $i \in \{2, \dots, N\}$:
    \begin{align}
        R_{2 + i} = R_{2 + i}/(-\frac{p_{y_i}(1 - p_x)}{p_{y_{i - 1}}})\\
        R_{1 + i} = R_{1 + i} - \frac{p_{y_{i}}}{p_{y_{i - 1}}}R_{2 + i}\\
        R_{3 + i} = R_{3 + i} - (1 - p_x)R_{2 + i}
    \end{align}\label{step-n}
\end{enumerate}

And the corresponding matrix will evaluate to
\begin{align}\label{matrix:rref} 
    \begin{bmatrix}
    1 &  0 &  0 &  -\frac{p_xp_{y_1}}{(1 - p_x)p_{y_0}} & \dots & 0 & -\frac{p_xp_{y_{N - 1}}}{(1 - p_x)p_{y_0}} & 0 & -\frac{p_xp_{y_N}}{(1 - p_x)p_{y_0}} & \frac{p^\prime_{10}p_{y_0} - p_{11}p_x}{(1 - p_x)p_{y_0}}\\
    0 &  1 &  0 & \frac{p_{y_1}}{p_{y_0}} & \dots & 0 & \frac{p_{y_{N - 1}}}{p_{y_0}} & 0 & \frac{p_{y_N}}{p_{y_0}} & \frac{p_{11}}{p_{y_0}}\\
    0 &  0 &  1 & \frac{p_x}{1 - p_x} &  \dots & 0 & 0 & 0 &  0 & \frac{p^\prime_{11}}{1 - p_x}\\
    \vdots &&&&&&& \ddots \\
    0 &  0 &  0 & 0 & \dots & 0 & 0 & 1 & \frac{p_x}{1 - p_x} & \frac{p_{10}(1 - p_x) + p_{11}p_x - \sum_{i = 0}^{N - 1} p^\prime_{1i}p_{y_i}}{p_{y_N}(1 - p_x)}\\
    0 &  0 &  0 & 0 & \dots & 0 & 0 & 0 & 0 & \frac{\sum_{i = 0}^{N} p^\prime_{1i}p_{y_i} - p_{10}(1 - p_x) - p_{11}p_x}{p_{y_N}} 
    \end{bmatrix}
\end{align}
\newline
\textbf{Base Case}: Starting with the base case of $N = 1$, i.e. $Y$ is binary. For the case when $Y$ is binary, we can enumerate the following equations for the $P(Z, X, Y)$
{\small
\begin{align*}
    \mathbb{P}(Z = 1 \mid X = 1) &= \mathbb{P}(Z = 1 \mid X = 1, Y = 1)\mathbb{P}(Y = 1) + \mathbb{P}(Z = 1 \mid X = 1, Y = 0)\mathbb{P}(Y = 0)\\
    \mathbb{P}(Z = 1 \mid X = 0) &= \mathbb{P}(Z = 1 \mid X = 0, Y = 1)\mathbb{P}(Y = 1) + \mathbb{P}(Z = 1 \mid X = 0, Y = 0)\mathbb{P}(Y = 0)\\
    \mathbb{P}(Z = 1 \mid Y = 1) &= \mathbb{P}(Z = 1 \mid X = 0, Y = 1)\mathbb{P}(X = 0) + \mathbb{P}(Z = 1 \mid X = 1, Y = 1)\mathbb{P}(X = 1)\\
    \mathbb{P}(Z = 1 \mid Y = 0) &= \mathbb{P}(Z = 1 \mid X = 0, Y = 0)\mathbb{P}(X = 0) + \mathbb{P}(Z = 1 \mid X = 1, Y = 0)\mathbb{P}(X = 1)
\end{align*}
}
And the augmented matrix $A|b$ will be written as
\begin{align*}
A|b &= \begin{bmatrix}
    p_{y_0} & 0 & p_{y_1} & 0 & p_{10}\\
    0 & p_{y_0} & 0 & p_{y_1} & p_{11}\\
    1 - p_x & p_x & 0 & 0 & p^\prime_{10}\\
    0 & 0 & 1 - p_x & p_x & p^\prime_{11}
\end{bmatrix}
\hspace{0.25in}\mathbf{x} 
= \begin{bmatrix}
P(Z = 1 \mid X = 0, Y = 0)\\    
P(Z = 1 \mid X = 1, Y = 0)\\
P(Z = 1 \mid X = 0, Y = 1)\\    
P(Z = 1 \mid X = 1, Y = 1)\\
\end{bmatrix}
\end{align*}

Executing the row operations on $A|b$ gives the following matrix
\begin{align*}
\begin{bmatrix}
    1 & 0 & 0 & -\frac{p_xp_{y_1}}{(1 - p_x)p_{y_0}} & \frac{p^\prime_{10}p_{y_0} - p_{11}p_x}{(1 - p_x)p_{y_0}}\\
    0 & 1 & 0 & \frac{p_{y_1}}{p_{y_0}} & \frac{p_{11}}{p_{y_0}}\\
    0 & 0 & 1 & \frac{p_x}{1 - p_x} & a\\ 
    0 & 0 & 0 & 0 & b
\end{bmatrix}    
\end{align*}
Where $a$ is:
\begin{align*}
    a &= \frac{p_{10}(1 - p_x) + p_{11}p_x - p^\prime_{10}p_{y_0}}{p_{y_1}(1 - p_x)}\\
    %\implies b &= \frac{p^\prime_{11}}{1 - x}
\end{align*}

And $b$ is 
\begin{align*}
    b &= \frac{-p_{10}(1 - p_x) - p_{11}p_x + p^\prime_{10}p_{y_0} + p^\prime_{11}p_{y_1}}{p_{y_1}}\\
    %&= 0
\end{align*}
This proves that the $A|b$ for $N = 1$ satisfies $P(1)$, proving the base case. \\
\newline
\textbf{Induction Step}: Next, we prove that if $P(N - 1)$ holds, then $P(N)$ holds as well. For $P(N)$, $A|b$ will look like
{\scriptsize
\begin{align*}
\begin{bmatrix}
    p_{y_0} & 0 & p_{y_1} & 0 & \dots & p_{y_{N - 1}} & 0 & y_N & 0 & p_{10}\\
    0 & p_{y_0} & 0 & p_{y_1} & \dots & 0 & p_{y_{N - 1}}& 0 & p_{y_N} & p_{11}\\
    1 - p_x & p_x & 0 & 0 & \dots & 0 & 0 & 0 & 0 & p^\prime_{10}\\
    0 & 0 & 1 - p_x & p_x & \dots & 0 & 0 & 0 & 0 & p^\prime_{11}\\
    \vdots & \ddots & & & & & & & & \vdots \\
    0 & 0 & 0 & 0 & \dots & 1 - p_x & p_x & 0 & 0 & p^\prime_{1(N - 1)}\\
    0 & 0 & 0 & 0 & \dots & 0 & 0 & 1 - p_x & p_x & p^\prime_{1N}\\
\end{bmatrix}    
\end{align*}
}

Now, since we assume $P(N - 1)$ holds, the submatrix of $A|b$ corresponding to $P(N - 1)$ can be put into the assumed RREF form. However, since we added two extra columns to $A \mid b$ the $P(N)$ compared to $a \mid b$ for $P(N- 1)$,  all of the row operations performed on the submatrix corresponding to $P(N - 1)$ must be performed on these added columns as well. None of these row operations apply to the final row, since it is newly added and therefore not touched by RREF computations for $P(N - 1)$. 

The row operations must be applied to the newly added columns, and we calculate these now. We use $c_N$ to denote the matrix of the newly added columns, and track the results on $c_N$ of the row operations applied to $P(N - 1)$.\\
Applying the row operations in \ref{step-1} to $c_N$
\begin{align*}
    c_N = \begin{bmatrix}
        \frac{y_N}{y_0} & 0\\
        0 & y_N\\
        -\frac{(1 - x)y_N}{y_0} & 0\\
        0 & 0\\
        \vdots \\
        1 - x & x\\
    \end{bmatrix}
\end{align*}
Next, applying the operations in \ref{step-2} to $c_N$
\begin{align*}
    c_N = \begin{bmatrix}
        \frac{y_N}{y_0} & 0\\
        0 & \frac{y_N}{y_0}\\
        -\frac{(1 - x)y_N}{y_0} & -\frac{xy_N}{y_0}\\
        0 & 0\\
        \vdots \\
        1 - x & x\\
    \end{bmatrix}
\end{align*}

Next, applying the operations in \ref{step-3} to $c_N$
\begin{align*}
    c_N = \begin{bmatrix}
        0 & -\frac{xy_N}{(1 - x)y_0}\\
        0 & \frac{y_N}{y_0}\\
        \frac{y_N}{y_1} & \frac{xy_N}{(1 - x)y_1}\\
        -\frac{y_N(1 - x)}{y_1} & -\frac{xy_N}{y_1}\\
        \vdots \\
        1 - x & x\\
    \end{bmatrix}
\end{align*}

Next, applying the operations in \ref{step-n} to $c_N$ for $i = 2$, we get
\begin{align*}
    c_N = \begin{bmatrix}
        0 & -\frac{xy_N}{(1 - x)y_0}\\
        0 & \frac{y_N}{y_0}\\
        0 & 0\\
        \frac{y_N}{y_2} & \frac{xy_N}{(1 - x)y_2}\\
        -\frac{(1 - x)y_N}{y_2} & -\frac{xy_N}{y_2}\\
        0 & 0\\
        \vdots \\
        1 - x & x\\
    \end{bmatrix}
\end{align*}

As we repeat the row operations in \ref{step-n} for  $i \in \{3, \dots, N - 1\}$, $c_N$ will ultimately become
\begin{align*}
    c_N = \begin{bmatrix}
                0 & -\frac{xy_N}{(1 - x)y_0}\\
                0 & \frac{y_N}{y_0}\\
                0 & 0\\
                0 & 0\\
                \vdots \\
                0 & 0\\
                \frac{y_N}{y_{N - 1}} & \frac{xy_N}{y_{N - 1}(1 - x)}\\
                -\frac{(1 - x)y_N}{y_{N - 1}} & -\frac{xy_N}{y_{N - 1}}\\
                1 - x & x\\
    \end{bmatrix}
\end{align*}

Consequently, the matrix $A \mid b$ corresponding to $P(N)$ will contain a submatrix corresponding to the RREF in $P(N - 1)$, with the resulting $c_N$ and extra row appended. Formally, it will look like the matrix presented below. 
{\tiny
\begin{align}\label{rref}
    \begin{bmatrix}[ccccccccc|c]
    1 &  0 &  0 &  -\frac{p_xp_{y_1}}{(1 - p_x)p_{y_0}} & \dots & 0 & -\frac{p_xp_{y_{N - 1}}}{(1 - p_x)p_{y_0}} & 0 & -\frac{p_xp_{y_N}}{(1 - p_x)p_{y_0}} & \frac{p^\prime_{10}p_{y_0} - p_{11}p_x}{(1 - p_x)p_{y_0}}\\
    0 &  1 &  0 & \frac{p_{y_1}}{p_{y_0}} & \dots & 0 & \frac{p_{y_{N - 1}}}{p_{y_0}} & 0 & \frac{p_{y_N}}{p_{y_0}} & \frac{p_{11}}{p_{y_0}}\\
    0 &  0 &  1 & \frac{p_x}{1 - p_x} &  \dots & 0 & 0 & 0 &  0 & \frac{p^\prime_{11}}{1 - p_x}\\
    \vdots &&&&&&& \ddots & &\vdots\\
    0 &  0 &  0 & 0 & \dots & 1 & \frac{p_x}{1 - p_x} & \frac{p_{y_N}}{p_{y_{N - 1}}}& \frac{p_xp_{y_N}}{p_{y_{N - 1}}(1 - p_x)} & \frac{p_{10}(1 - p_x) + p_{11}p_x - \sum_{i = 0}^{N - 2} p^\prime_{1i}y_i}{y_{N - 1}(1 - x)}\\
    0 &  0 &  0 & 0 & \dots & 0 & 0 & -\frac{(1 - x)y_N}{y_{N - 1}} & -\frac{xy_N}{y_{N - 1}} & \frac{\sum_{i = 0}^{N - 1} p^\prime_{1i}y_i - p_{10}(1 - x) - p_{11}x}{y_{N - 1}}\\
    0 &  0 &  0 & 0 & \dots & 0 & 0 & 1 - x & x & p^\prime_{1N}
    \end{bmatrix}
\end{align}
}
This matrix is not in RREF yet, so we perform the following row operations to put the matrix in RREF
\begin{align*}
    R_{N + 2} = \frac{R_{N + 2}}{-\frac{(1 - p_x)p_{y_N}}{p_{y_{N - 1}}}}\\
    R_{N + 1} = R_{N + 1} - \frac{p_{y_N}}{p_{y_{N - 1}}}R_{N + 2}\\
    R_{N + 3} = R_{N + 3} - (1 - p_x)R_{N + 2}
\end{align*}

Resulting in the following matrix:
{\tiny
\begin{align}\label{matrix:induction-case-rref}
    \begin{bmatrix}[ccccccccc|c]
    1 &  0 &  0 &  -\frac{p_xp_{y_1}}{(1 - p_x)p_{y_0}} & \dots & 0 & -\frac{p_xp_{y_{N - 1}}}{(1 - p_x)p_{y_0}} & 0 & -\frac{[_xp_{y_N}}{(1 - p_x)p_{y_0}} & \frac{p^\prime_{10}p_{y_0} - p_{11}p_x}{(1 - p_x)p_{y_0}}\\
    0 &  1 &  0 & \frac{p_{y_1}}{p_{y_0}} & \dots & 0 & \frac{p_{y_{N - 1}}}{p_{y_0}} & 0 & \frac{p_{y_N}}{p_{y_0}} & \frac{p_{11}}{p_{y_0}}\\
    0 &  0 &  1 & \frac{p_x}{1 - p_x} &  \dots & 0 & 0 & 0 &  0 & \frac{p^\prime_{11}}{1 - p_x}\\
    \vdots &&&&&&& \ddots & &\vdots\\
    0 &  0 &  0 & 0 & \dots & 1 & \frac{p_x}{1 - p_x} & 0 & 0 & \frac{p^\prime_{1(N - 1)}}{1 - p_x}\\
    0 &  0 &  0 & 0 & \dots & 0 & 0 & 1 & \frac{p_x}{1 - p_x} & \frac{p_{10}(1 - p_x) + p_{11}p_x - \sum_{i = 0}^{N - 1} p^\prime_{1i}p_{y_i}}{p_{y_N}(1 - p_x)}\\
    0 &  0 &  0 & 0 & \dots & 0 & 0 & 0 & 0 & p^\prime_{1N} - \frac{p_{10}(1 - p_x) + p_{11}p_x - \sum_{i = 0}^{N - 1}p^\prime_{1i}p_{y_i}}{p_{y_N}}
    \end{bmatrix}
\end{align}
}

And by comparison, this matrix is equal to the matrix stated in our proposition. So, if $P(N - 1)$, then $P(N)$ holds, and this concludes the induction proof. 

Finally, since $P(Z, X)$ and $P(Z, Y)$ are marginalized distributions obtained from marginalizing out $Y$ and $X$ from $P(Z, X, Y)$ respectively, they must agree on $P(Z)$. This gives the identity
\[
p_{11}x + p_{10}(1 - x) - \sum_{i = 0}^N p^\prime_{1i}y_i = 0
\]
And substituting this identity into the RREF form of $A | b$, we obtain
{\tiny
\begin{align}\label{rref}
    \begin{bmatrix}[ccccccccc|c]
    1 &  0 &  0 &  -\frac{p_xp_{y_1}}{(1 - p_x)p_{y_0}} & \dots & 0 & -\frac{p_xp_{y_{N - 1}}}{(1 - p_x)p_{y_0}} & 0 & -\frac{p_xp_{y_N}}{(1 - p_x)p_{y_0}} & \frac{p^\prime_{10}p_{y_0} - p_{11}p_x}{(1 - p_x)p_{y_0}}\\
    0 &  1 &  0 & \frac{p_{y_1}}{p_{y_0}} & \dots & 0 & \frac{p_{y_{N - 1}}}{p_{y_0}} & 0 & \frac{p_{y_N}}{p_{y_0}} & \frac{p_{11}}{p_{y_0}}\\
    0 &  0 &  1 & \frac{p_x}{1 - p_x} &  \dots & 0 & 0 & 0 &  0 & \frac{p^\prime_{11}}{1 - p_x}\\
    \vdots &&&&&&& \ddots & &\vdots\\
    0 &  0 &  0 & 0 & \dots & 1 & \frac{p_x}{1 - p_x} & 0 & 0 & \frac{p^\prime_{1(N - 1)}}{1 - p_x}\\
    0 &  0 &  0 & 0 & \dots & 0 & 0 & 1 & \frac{p_x}{1 - p_x} & \frac{p^\prime_{1N}}{1 - p_x}\\
    0 &  0 &  0 & 0 & \dots & 0 & 0 & 0 & 0 & 0
    \end{bmatrix}
\end{align}
}
Expressing this matrix in the form of its corresponding equations completes the proof for this Lemma.

% \begin{lemma}
% To ensure the solution to the system of equations in Lemma \ref{lemma:RREF-y} form coherent probabilities, the following bounds on the free parameters must hold
% {\small
% \begin{align*}
% \max\begin{bmatrix}
%    \frac{p_{11}x - p^\prime_{10}y_0}{x} \\
%    p_{11} - y_0
% \end{bmatrix} \leq \sum_{n = 1}^N y_n\mathbb{P}(Z = 1 \mid X = 1, Y = n) 
% \leq \min\begin{bmatrix}
%     \frac{(1 - x)y_0 + p_{11}x - p^\prime_{10}y_0}{x}\\
%     p_{11}
% \end{bmatrix}
% \end{align*}
% }

% And for each $i \in \{1, \dots, N\}$, we the bounds on the following free parameters $P(Z = 1\mid X = 1, Y = i)$
% \begin{align*}
%     \max\begin{bmatrix}
%         0\\
%         \frac{p^\prime_{1i} - (1 - x)}{x}
%     \end{bmatrix}
%         \leq P(Z = 1\mid X = 1, Y = i) \leq 
%     \min\begin{bmatrix}
%         1\\
%         \frac{p^\prime_{1i}}{x}
%     \end{bmatrix}
% \end{align*}
% \end{lemma}
\textbf{Proof of Lemma \ref{lem:free-param-bounds}}: Using the result presented in Lemma \ref{lemma:RREF-y}, when $Y$ has support $\{0, \dots, N\}$ and we are given marginals $P(Z, X)$ and $P(Z, Y)$, we can write the system of equations using free parameters as   

{\small
\begin{align*}
\mathbb{P}(Z = 1 \mid X = 0, Y = 0) &=  \frac{x}{1 - x}\sum_{n = 1}^N\frac{y_n}{y_0}\mathbb{P}(Z = 1 \mid X = 1, Y = n) + \frac{p^\prime_{10}y_0 - p_{11}x}{(1 - x)y_0}\\
\mathbb{P}(Z = 1 \mid X = 1, Y = 0)&= \frac{p_{11}}{y_0} - \sum_{n = 1}^N\frac{y_n}{y_0}\mathbb{P}(Z = 1 \mid X = 1, Y = n)\\
\mathbb{P}(Z = 1 \mid X = 0, Y = 1)&= \frac{p^\prime_{11}}{ 1- x} - \frac{x}{1 - x}\mathbb{P}(Z = 1 \mid X = 1, Y = 1)\\
\mathbb{P}(Z = 1 \mid X = 0, Y = 2)&= \frac{p^\prime_{12}}{ 1- x} - \frac{x}{1 - x}\mathbb{P}(Z = 1 \mid X = 1, Y = 2)\\
\vdots\\
\mathbb{P}(Z = 1 \mid X = 0, Y = N)&= \frac{p^\prime_{1N}}{ 1- x} - \frac{x}{1 - x}\mathbb{P}(Z = 1 \mid X = 1, Y = N)\\
\end{align*}
}

Now, each of the basic variables in the system above must be a valid probability, i.e. between zero and one, inclusive. Employing these constraints on the free parameters gives
\begin{align*}
    0 \leq P(Z = 1 \mid X = 0, Y = 0) \leq 1\\
    \implies 0 \leq  \frac{x}{1 - x}\sum_{n = 1}^N\frac{y_n}{y_0}\mathbb{P}(Z = 1 \mid X = 1, Y = n) + \frac{p^\prime_{10}y_0 - p_{11}x}{(1 - x)y_0} \leq 1
\end{align*}

Solving for the lower bound first, we have
\begin{align*}
    0 \leq  \frac{x}{1 - x}\sum_{n = 1}^N\frac{y_n}{y_0}\mathbb{P}(Z = 1 \mid X = 1, Y = n) + \frac{p^\prime_{10}y_0 - p_{11}x}{(1 - x)y_0}\\
    \implies \frac{p_{11}x - p^\prime_{10}y_0}{x} \leq \sum_{n = 1}^N P(Z = 1\mid X = 1, Y = n)
\end{align*}
Next, with the upper bound
\begin{align*}
    \frac{x}{1 - x}\sum_{n = 1}^N\frac{y_n}{y_0}\mathbb{P}(Z = 1 \mid X = 1, Y = n) + \frac{p^\prime_{10}y_0 - p_{11}x}{(1 - x)y_0} \leq 1\\
    \implies x\sum_{n = 1}^Ny_n\mathbb{P}(Z = 1 \mid X = 1, Y = n) + p^\prime_{10}y_0 - p_{11}x \leq (1 - x)y_0\\
    \implies \sum_{n = 1}^Ny_n\mathbb{P}(Z = 1 \mid X = 1, Y = n) \leq \frac{(1 - x)y_0 + p_{11}x - p^\prime_{10}y_0}{x}
\end{align*}

Following a similar calculation for $P(Z = 1\mid X = 1, Y = 0)$, we have
\begin{align*}
    p_{11} - y_0 \leq \sum_{n = 1}^Ny_n\mathbb{P}(Z = 1 \mid X = 1, Y = n) \leq p_{11}
\end{align*}

Since all of the bounds need to hold simultaneously, we can re-express them using using maximum and minimum operators as
{\small
\begin{align*}
\max\begin{bmatrix}
   \frac{p_{11}x - p^\prime_{10}y_0}{x} \\
   p_{11} - y_0
\end{bmatrix} \leq \sum_{n = 1}^N y_n\mathbb{P}(Z = 1 \mid X = 1, Y = n) 
\leq \min\begin{bmatrix}
    \frac{(1 - x)y_0 + p_{11}x - p^\prime_{10}y_0}{x}\\
    p_{11}
\end{bmatrix}
\end{align*}
}

Next, for $i \in \{1, \dots, N\}$, we have the following constrain on the basic variables $P(Z = 1\mid X = 0, Y = i)$
\begin{align*}
    0 \leq P(Z = 1 \mid X = 0, Y = i) \leq 1\\
    0 \leq \frac{p^\prime_{11}}{ 1- x} - \frac{x}{1 - x}\mathbb{P}(Z = 1 \mid X = 1, Y = 1) \leq 1\\
    \implies \frac{p^\prime_{1i} - (1 - x)}{x} \leq P(Z = 1\mid X = 1, Y = i) \leq \frac{p^\prime_{1i}}{x} 
\end{align*}

And since the free parameters are probabilities themselves, they must be between $0$ and $1$ and hence the bounds for $P(Z = 1 \mid X = 1, Y = i)$ become
\begin{align*}
    \max\begin{bmatrix}
        0\\
        \frac{p^\prime_{1i} - (1 - x)}{x}
    \end{bmatrix}
        \leq P(Z = 1\mid X = 1, Y = i) \leq 
    \min\begin{bmatrix}
        1\\
        \frac{p^\prime_{1i}}{x}
    \end{bmatrix}
\end{align*}
% ++++\end{proof}

\begin{lemma}
    Given $P(Z, X)$ and $P(Z, Y)$, using the solution to the system of equations in Lemma \ref{lemma:RREF-y}, each of the terms in $\Delta$ and $\Gamma$ defined in Lemma \ref{lem:joint-bounds} are expressed in terms of the free parameters below. First, for $\Gamma$, each of the terms can be written as
    \begin{align*}
        &\mathbb{P}(Z = 1 \mid X = 1, Y = 0) - \mathbb{P}(Z = 0 \mid X = 0, Y = 0)\\
        &= \frac{p^\prime_{10} - (1 - p_x)}{1 - p_x} + \frac{\sum_{n = 1}^N p_{y_n}P(Z = 1 \mid X = 1, Y = n) - p_{11}}{p_{y_0}}\Bigg(\frac{p_x}{1 - p_x} - 1\Bigg)
    \end{align*}
    And for the terms in $\Gamma$ corresponding to $Y = i$, $i \in \{1, \dots , N\}$
    \begin{align*}
        &P(Z = 1 \mid X = 1, Y = i) - P(Z = 0 \mid X = 0, Y = i)\\
        &= P(Z = 1 \mid X = 1, Y = i)\Bigg(1 - \frac{p_x}{1 - p_x}\Bigg) + \frac{p^\prime_{11} - (1 - p_x)}{1 - p_x}\\
    \end{align*}
    Similarly, the terms in $\Delta$ can be expressed in terms of the free parameter as
    \begin{align*}
        &\mathbb{P}(Z = 1 \mid X = 1, Y = 0) - \mathbb{P}(Z = 1 \mid X = 0, Y = 0)\\
        &= \frac{p_{11} - p^\prime_{10}p_{y_0} - \sum_{n = 1}^N p_{y_n}\mathbb{P}(Z = 1\mid X = 1, Y = n)}{(1 - p_x)p_{y_0}}
    \end{align*}
    And for the terms in $\Delta$ corresponding to $Y = i$, $i \in \{1, \dots , N\}$
    \begin{align*}
        &\mathbb{P}(Z = 1 \mid X = 1, Y = 1) - \mathbb{P}(Z = 1 \mid X = 0, Y = 1)\\
        &=\frac{\mathbb{P}(Z = 1 \mid X = 1, Y = i) - p^\prime_{1i}}{1 - p_x}
    \end{align*}
\end{lemma}

\begin{proof}
    Using the system of equations obtained in Lemma \ref{lemma:RREF-y}, each term in $\Gamma$ can be expressed using these free parameters. Starting with
    $\max \{0, \mathbb{P}(Z = 1 \mid X = 1, Y = 0) - \mathbb{P}(Z = 0 \mid X = 0, Y = 0)\}$. First, expressing each of these terms using the free parameters, we get
    \begin{align*}
        P(Z = 1 \mid X = 1, Y = 0) &= \frac{p_{11}}{p_{y_0}} - \sum_{n = 1}^N\frac{p_{y_n}}{p_{y_0}}\mathbb{P}(Z = 1 \mid X = 1, Y = n)\\
        P(Z = 0 \mid X = 0, Y = 0) &= 1 - \Bigg(\frac{p_x}{1 - p_x}\sum_{n = 1}^N\frac{p_{y_n}}{p_{y_0}}\mathbb{P}(Z = 1 \mid X = 1, Y = n) + \frac{p^\prime_{10}p_{y_0} - p_{11}p_x}{(1 - p_x)p_{y_0}}\Bigg)
    \end{align*}
    Subtracting these two, 
    \begin{align*}
        &= \frac{p_{11}}{p_{y_0}} - \sum_{n = 1}^N\frac{p_{y_n}}{p_{y_0}}\mathbb{P}(Z = 1 \mid X = 1, Y = n) - 1\\
        &+ \frac{p_x}{1 - p_x}\sum_{n = 1}^N\frac{p_{y_n}}{p_{y_0}}\mathbb{P}(Z = 1 \mid X = 1, Y = n) + \frac{p^\prime_{10}p_{y_0} - p_{11}p_x}{(1 - p_x)p_{y_0}}\\
        &= \frac{p^\prime_{10}p_{y_0} - p_{11}p_x}{(1 - p_x)p_{y_0}} + \frac{p_{11}}{p_{y_0}} - 1 + \sum_{n = 1}^N\frac{p_{y_n}}{p_{y_0}}P(Z = 1 \mid X = 1, Y = n)\Bigg(\frac{p_x}{1 - p_x} - 1\Bigg)\\
        &= \frac{p^\prime_{10}p_{y_0} - p_{11}p_x + p_{11}(1 - p_x) - (1 - p_x)p_{y_0}}{(1 - p_x)p_{y_0}}   + \sum_{n = 1}^N\frac{p_{y_n}}{p_{y_0}}P(Z = 1 \mid X = 1, Y = n)\Bigg(\frac{p_x}{1 - p_x} - 1\Bigg)\\
        &= \frac{p^\prime_{10} - (1 - p_x)}{1 - p_x} + \frac{p_{11}}{p_{y_0}}\Big(1 - \frac{p_x}{1 - p_x}\Big)  + \sum_{n = 1}^N\frac{p_{y_n}}{p_{y_0}}P(Z = 1 \mid X = 1, Y = n)\Bigg(\frac{p_x}{1 - p_x} - 1\Bigg)\\
        &= \frac{p^\prime_{10} - (1 - p_x)}{1 - p_x} + \frac{\sum_{n = 1}^N p_{y_n}P(Z = 1 \mid X = 1, Y = n) - p_{11}}{p_{y_0}}\Bigg(\frac{p_x}{1 - p_x} - 1\Bigg) 
    \end{align*}

    Moving on to $\max\{0, P(Z = 1 \mid X = 1, Y = i) - P(Z = 0 \mid X = 0, Y = i)\}$, the probability $P(Z = 0 \mid X = 0, Y = i)$ for $i \in \{1, \dots ,N\}$ can be expressed in terms of the free parameters as
    \begin{align*}
        &P(Z = 0 \mid X = 0, Y = i) = 1 -\Bigg( \frac{p^\prime_{1i}}{1 - p_x} - \frac{p_x}{1 - p_x}\mathbb{P}(Z = 1 \mid X = 1, Y = i)\Bigg)\\
        &\implies P(Z = 1 \mid X = 1, Y = i) - P(Z = 0 \mid X = 0, Y = i) \\
        &= P(Z = 1 \mid X = 1, Y = i) - 1 + \frac{p^\prime_{1i}}{1 - p_x} - \frac{p_x}{1 - p_x}\mathbb{P}(Z = 1 \mid X = 1, Y = i)\\
        &= P(Z = 1 \mid X = 1, Y = i)\Bigg(1 - \frac{p_x}{1 - p_x}\Bigg) + \frac{p^\prime_{11} - (1 - p_x)}{1 - p_x}
    \end{align*}
    This concludes the proof for the terms in $\Gamma$. Following a similar approach for the terms in $\Delta$, first consider
    \begin{align*}
        &\mathbb{P}(Z = 1 \mid X = 1, Y = 0) - \mathbb{P}(Z = 1 \mid X = 0, Y = 0)\\
        &= \frac{p_{11}}{p_{y_0}} - \sum_{n = 1}^N\frac{p_{y_n}}{p_{y_0}}\mathbb{P}(Z = 1 \mid X = 1, Y = n) - \Bigg(\frac{p_x}{1 - p_x}\sum_{n = 1}^N\frac{p_{y_n}}{p_{y_0}}\mathbb{P}(Z = 1 \mid X = 1, Y = n)\\
        &+ \frac{p^\prime_{10}p_{y_0} - p_{11}p_x}{(1 - p_x)p_{y_0}}\Bigg)\\
        &= \frac{p_{11} - p^\prime_{10}p_{y_0} - \sum_{n = 1}^N p_{y_n}\mathbb{P}(Z = 1\mid X = 1, Y = n)}{(1 - p_x)p_{y_0}}
    \end{align*}

    And for the terms of the form $\max\{0, \mathbb{P}(Z = 1 \mid X = 1, Y = i) - \mathbb{P}(Z = 1 \mid X = 0, Y = i)\}$ for $i \in \{1, \dots, N\}$
    \begin{align*}
        &\mathbb{P}(Z = 1 \mid X = 0, Y = i) = \frac{p^\prime_{1i}}{1 - p_x} - \frac{p_x}{1 - p_x}\mathbb{P}(Z = 1 \mid X = 1, Y = i)\\
        &\implies \mathbb{P}(Z = 1 \mid X = 1, Y = i) - \mathbb{P}(Z = 1 \mid X = 0, Y = i) =\\
        &\mathbb{P}(Z = 1 \mid X = 1, Y = i) - \frac{p^\prime_{1i}}{1 - p_x} + \frac{p_x}{1 - p_x}\mathbb{P}(Z = 1 \mid X = 1, Y = i)\\
        &= \frac{\mathbb{P}(Z = 1 \mid X = 1, Y = i) - p^\prime_{1i}}{1 - p_x}
    \end{align*}
    This concludes the proof of the Lemma.
\end{proof}

\begin{lemma}
    The following implications hold:
    \begin{equation*}
     p^\prime_{10} < p_x \implies \frac{p_{11}p_x - p^\prime_{10}p_{y_0}}{p_x} > p_{11} - p_{y_0}   
    \end{equation*}
    \begin{equation*}
     p^\prime_{10} \geq p_x \implies \frac{p_{11}p_x - p^\prime_{10}p_{y_0}}{p_x} \leq p_{11} - p_{y_0}   
    \end{equation*}
    \begin{equation*}
        p^\prime_{10} < 1 - p_x \implies p_{11} < \frac{(1 - p_x)p_{y_0} + p_{11}p_x - p^\prime_{10}p_{y_0}}{p_x}
    \end{equation*}
    \begin{equation*}
        p^\prime_{10} \geq 1 - p_x \implies p_{11} \geq \frac{(1 - p_x)p_{y_0} + p_{11}p_x - p^\prime_{10}p_{y_0}}{p_x}
    \end{equation*}
\end{lemma}

\begin{proof}
Each of these is proved using a proof by contra-positive. Starting with $p^\prime_{10} < p_x \implies \frac{p_{11}p_x - p^\prime_{10}p_{y_0}}{p_x} > p_{11} - p_{y_0}$, the contra-positive of this statement is
    \[
    \frac{p_{11}p_x - p^\prime_{10}p_{y_0}}{p_x} \leq p_{11} - p_{y_0} \implies p^\prime_{10} \geq p_x 
    \]
    To see this holds, note that
    \begin{align*}
        \frac{p_{11}p_x - p^\prime_{10}p_{y_0}}{p_x} \leq p_{11} - p_{y_0}\\
        \implies -\frac{p^\prime_{10}p_{y_0}}{p_x} \leq  - p_{y_0}\\
        \implies p^\prime_{10} \leq p_x
    \end{align*}
This proves $p^\prime_{10} < p_x \implies \frac{p_{11}p_x - p^\prime_{10}p_{y_0}}{p_x} > p_{11} - p_{y_0}$.\\
Next, for $p^\prime_{10} \geq p_x \implies \frac{p_{11}p_x - p^\prime_{10}p_{y_0}}{p_x} \leq p_{11} - p_{y_0}$, following a similar proof strategy, the contra-positive can be written as
\[
\frac{p_{11}p_x - p^\prime_{10}p_{y_0}}{p_x} > p_{11} - p_{y_0} \implies p^\prime_{10} < p_x
\]
To see this holds, note that
\begin{align*}
    \frac{p_{11}p_x - p^\prime_{10}p_{y_0}}{p_x} > p_{11} - p_{y_0}\\
    \implies -\frac{p^\prime_{10}p_{y_0}}{p_x} > - p_{y_0}\\
    \implies p^\prime_{10} < p_x
\end{align*}
This proves $p^\prime_{10} \geq p_x \implies \frac{p_{11}p_x - p^\prime_{10}p_{y_0}}{p_x} \leq p_{11} - p_{y_0}$.\\
Next, for $p^\prime_{10} < 1 - p_x \implies p_{11} < \frac{(1 - p_x)p_{y_0} + p_{11}p_x - p^\prime_{10}p_{y_0}}{p_x}$, the contra-positive is written as
\[
p_{11} \geq \frac{(1 - p_x)p_{y_0} + p_{11}p_x - p^\prime_{10}p_{y_0}}{p_x}  \implies p^\prime_{10} \geq 1 - p_x
\]
To see this holds, note that
\begin{align*}
    &p_{11} \geq \frac{(1 - p_x)p_{y_0} + p_{11}p_x - p^\prime_{10}p_{y_0}}{p_x}\\
    &\implies 0 \geq (1 - p_x)p_{y_0} - p^\prime_{10}p_{y_0}\\
    &\implies  p^\prime_{10} \geq 1 - p_x
\end{align*}
This proves $p^\prime_{10} < 1 - p_x \implies p_{11} < \frac{(1 - p_x)p_{y_0} + p_{11}p_x - p^\prime_{10}p_{y_0}}{p_x}$.\\
Next, for $p^\prime_{10} \geq 1 - p_x \implies p_{11} \geq \frac{(1 - p_x)p_{y_0} + p_{11}p_x - p^\prime_{10}p_{y_0}}{p_x}$ the contra-positive is written as
\[
p_{11} < \frac{(1 - p_x)p_{y_0} + p_{11}p_x - p^\prime_{10}p_{y_0}}{p_x}  \implies p^\prime_{10} < 1 - p_x
\]
To see this holds, note that
\begin{align*}
    &p_{11} < \frac{(1 - p_x)p_{y_0} + p_{11}p_x - p^\prime_{10}p_{y_0}}{p_x}\\
    &\implies 0 < (1 - p_x)p_{y_0} - p^\prime_{10}p_{y_0}
    &\implies p^\prime_{10} < 1 - p_x
\end{align*}

This concludes the proof.
\end{proof}

\begin{lemma}
For $i \in \{1, \dots, N\}$, when $p^\prime_{1i} > 1 - p_x \implies \frac{p^\prime_{11} - (1 - p_x)}{p_x} > 0$. When $p^\prime_{1i} < p_x \implies \frac{p^\prime_{11}}{p_x} < 1$    
\end{lemma}
\begin{proof}
The proof follows from properties of probability.     
\end{proof}

\begin{lemma}
    Assume $p_x > 1 - p_x$. The function $\max \{0, \mathbb{P}(Z = 1 \mid X = 1, Y = 0) - \mathbb{P}(Z = 0 \mid X = 0, Y = 0)\} \geq 0$ when
    \begin{align*}
            \sum_{n = 1}^N p_{y_n}P(Z = 1 \mid X = 1, Y = n) \geq \frac{p_{y_0}((1 - p_x) - p^\prime_{10})}{p_x - (1 - p_x)} + p_{11}
    \end{align*}
\end{lemma}

\begin{proof}
    From the result of Lemma \ref{}, $\mathbb{P}(Z = 1 \mid X = 1, Y = 0) - \mathbb{P}(Z = 0 \mid X = 0, Y = 0)$ can be expressed in terms of the free parameter as
    \begin{align*}
        \frac{p^\prime_{10} - (1 - p_x)}{1 - p_x} + \frac{\sum_{n = 1}^N p_{y_n}P(Z = 1 \mid X = 1, Y = n) - p_{11}}{p_{y_0}}\Bigg(\frac{p_x}{1 - p_x} - 1\Bigg)
    \end{align*}
    Now, we use a proof by contra-positive to first show that
    \begin{align*}
        &\frac{p^\prime_{10} - (1 - p_x)}{1 - p_x} + \frac{\sum_{n = 1}^N p_{y_n}P(Z = 1 \mid X = 1, Y = n) - p_{11}}{p_{y_0}}\Bigg(\frac{p_x}{1 - p_x} - 1\Bigg) < 0\\
        &\implies \sum_{n = 1}^N p_{y_n}P(Z = 1 \mid X = 1, Y = n) < \frac{p_{y_0}((1 - p_x) - p^\prime_{10})}{p_x - (1 - p_x)} + p_{11}
    \end{align*}
    To see this, note that
    \begin{align*}
        &\frac{p^\prime_{10} - (1 - p_x)}{1 - p_x} + \frac{\sum_{n = 1}^N p_{y_n}P(Z = 1 \mid X = 1, Y = n) - p_{11}}{p_{y_0}}\Bigg(\frac{p_x}{1 - p_x} - 1\Bigg) < 0\\
        &\implies p_{y_0}\frac{p^\prime_{10} - (1 - p_x)}{p_{y_0}(1 - p_x)} + \frac{\sum_{n = 1}^N p_{y_n}P(Z = 1 \mid X = 1, Y = n) - p_{11}}{p_{y_0}}\Bigg(\frac{p_x - (1 - p_x)}{1 - p_x} \Bigg) < 0\\
        &\implies p_{y_0}(p^\prime_{10} - (1 - p_x)) + (\sum_{n = 1}^N p_{y_n}P(Z = 1 \mid X = 1, Y = n) - p_{11})\Bigg(p_x - (1 - p_x)\Bigg) < 0\\
        &\implies \sum_{n = 1}^N p_{y_n}P(Z = 1 \mid X = 1, Y = n) < \frac{p_{y_0}((1 - p_x) - p^\prime_{10})}{p_x - (1 - p_x)} + p_{11}\\
    \end{align*}
    This concludes the proof.
\end{proof}

\begin{lemma}
    Assume $p_x > 1 - p_x$. The function $\max \{0, \mathbb{P}(Z = 1 \mid X = 1, Y = i) - \mathbb{P}(Z = 0 \mid X = 0, Y = i)\} \geq 0$ for $i \in \{1, \dots, N\}$ when
    \begin{align*}
            P(Z = 1 \mid X = 1, Y = i) \leq \frac{p^\prime_{1i} - (1 - p_x)}{p_x - (1 - p_x)}    
    \end{align*}
\end{lemma}

\begin{proof}
From the result of Lemma \ref{}, $\mathbb{P}(Z = 1 \mid X = 1, Y = i) - \mathbb{P}(Z = 0 \mid X = 0, Y = i)\}$ can be expressed in terms of the free parameter as 
\[
P(Z = 1 \mid X = 1, Y = i)\Bigg(1 - \frac{p_x}{1 - p_x}\Bigg) + \frac{p^\prime_{11} - (1 - p_x)}{1 - p_x}
\]
Following a proof by contra-positive, we write the contra-positive as
\begin{align*}
&P(Z = 1 \mid X = 1, Y = i)\Bigg(1 - \frac{p_x}{1 - p_x}\Bigg) + \frac{p^\prime_{11} - (1 - p_x)}{1 - p_x} < 0\\
&\implies P(Z = 1 \mid X = 1, Y = i) > \frac{p^\prime_{1i} - (1 - p_x)}{p_x - (1 - p_x)}     
\end{align*}
To see this, note that
\begin{align*}
    &P(Z = 1 \mid X = 1, Y = i)\Bigg(1 - \frac{p_x}{1 - p_x}\Bigg) + \frac{p^\prime_{11} - (1 - p_x)}{1 - p_x} < 0\\
    &\implies P(Z = 1 \mid X = 1, Y = i)\Bigg(\frac{(1 - p_x) - p_x}{1 - p_x}\Bigg)  < \frac{(1 - p_x) - p^\prime_{11}}{1 - p_x}\\
    &\implies P(Z = 1 \mid X = 1, Y = i)\Bigg((1 - p_x) - p_x\Bigg)  < (1 - p_x) - p^\prime_{11}\\
    &\implies P(Z = 1 \mid X = 1, Y = i)  >  \frac{p^\prime_{11} - (1 - p_x)}{p_x - (1 - p_x)}
\end{align*}

This concludes the proof.
\end{proof}

\begin{lemma}
    Assume $p_x < 1 - p_x$. The function $\max \{0, \mathbb{P}(Z = 1 \mid X = 1, Y = 0) - \mathbb{P}(Z = 0 \mid X = 0, Y = 0)\} \geq 0$ when
    \begin{align*}
            \sum_{n = 1}^N p_{y_n}P(Z = 1 \mid X = 1, Y = n) \leq \frac{p_{y_0}( p^\prime_{10} - (1 - p_x))}{(1 - p_x) - p_x} + p_{11}   
    \end{align*}
\end{lemma}
\begin{proof}
From the result of Lemma \ref{}, $\mathbb{P}(Z = 1 \mid X = 1, Y = 0) - \mathbb{P}(Z = 0 \mid X = 0, Y = 0)$ can be expressed in terms of the free parameter as
\begin{align*}
        \frac{p^\prime_{10} - (1 - p_x)}{1 - p_x} + \frac{\sum_{n = 1}^N p_{y_n}P(Z = 1 \mid X = 1, Y = n) - p_{11}}{p_{y_0}}\Bigg(\frac{p_x}{1 - p_x} - 1\Bigg)
\end{align*}
Following a proof by contra-positive, we write the contra-positive as
\begin{align*}
    &\frac{p^\prime_{10} - (1 - p_x)}{1 - p_x} + \frac{\sum_{n = 1}^N p_{y_n}P(Z = 1 \mid X = 1, Y = n) - p_{11}}{p_{y_0}}\Bigg(\frac{p_x}{1 - p_x} - 1\Bigg) < 0\\
    &\implies \sum_{n = 1}^N p_{y_n}P(Z = 1 \mid X = 1, Y = n) > \frac{p_{y_0}( p^\prime_{10} - (1 - p_x))}{(1 - p_x) - p_x} + p_{11}   
\end{align*}
To see this, note that
\begin{align*}
    &\frac{p^\prime_{10} - (1 - p_x)}{1 - p_x} + \frac{\sum_{n = 1}^N p_{y_n}P(Z = 1 \mid X = 1, Y = n) - p_{11}}{p_{y_0}}\Bigg(\frac{p_x}{1 - p_x} - 1\Bigg) < 0\\
    &\implies -\frac{p^\prime_{10} - (1 - p_x)}{1 - p_x} + \frac{\sum_{n = 1}^N p_{y_n}P(Z = 1 \mid X = 1, Y = n) - p_{11}}{p_{y_0}}\Bigg(1 - \frac{p_x}{1 - p_x}\Bigg) > 0\\
    &\implies -p_{y_0}\frac{p^\prime_{10} - (1 - p_x)}{p_{y_0}(1 - p_x)} + \frac{\sum_{n = 1}^N p_{y_n}P(Z = 1 \mid X = 1, Y = n) - p_{11}}{p_{y_0}}\Bigg(\frac{(1 - p_x) - p_x}{1 - p_x}\Bigg) > 0\\
    &\implies \frac{\sum_{n = 1}^N p_{y_n}P(Z = 1 \mid X = 1, Y = n) - p_{11}}{p_{y_0}}\Bigg(\frac{(1 - p_x) - p_x}{1 - p_x}\Bigg) > p_{y_0}\frac{p^\prime_{10} - (1 - p_x)}{p_{y_0}(1 - p_x)}\\
    &\implies \sum_{n = 1}^N p_{y_n}P(Z = 1 \mid X = 1, Y = n) > \frac{p_{y_0}(p^\prime_{10} - (1 - p_x))}{(1 - p_x) - p_x} + p_{11}
\end{align*}

This concludes the proof.
\end{proof}

\begin{lemma}
    Assume $p_x < 1 - p_x$. The functions $\max \{0, \mathbb{P}(Z = 1 \mid X = 1, Y = i) - \mathbb{P}(Z = 0 \mid X = 0, Y = i)\} \geq 0$ for $i \in \{1, \dots, N\}$ when
    \begin{align*}
            P(Z = 1 \mid X = 1, Y = i) \geq \frac{(1 - p_x) - p^\prime_{1i}}{(1 - p_x) - p_x}    
    \end{align*}
\end{lemma}

\begin{proof}
From the result of Lemma \ref{}, $\mathbb{P}(Z = 1 \mid X = 1, Y = i) - \mathbb{P}(Z = 0 \mid X = 0, Y = i)\}$ can be expressed in terms of the free parameter as 
\[
P(Z = 1 \mid X = 1, Y = i)\Bigg(1 - \frac{p_x}{1 - p_x}\Bigg) + \frac{p^\prime_{11} - (1 - p_x)}{1 - p_x}
\]
Following a proof by contra-positive, we can write the contra-positive as
\begin{align*}
    &P(Z = 1 \mid X = 1, Y = i)\Bigg(1 - \frac{p_x}{1 - p_x}\Bigg) + \frac{p^\prime_{11} - (1 - p_x)}{1 - p_x} < 0\\
    &\implies P(Z = 1 \mid X = 1, Y = i) < \frac{(1 - p_x) - p^\prime_{1i}}{(1 - p_x) - p_x}
\end{align*}

To see this, note that
\begin{align*}
    &P(Z = 1 \mid X = 1, Y = i)\Bigg(1 - \frac{p_x}{1 - p_x}\Bigg) + \frac{p^\prime_{11} - (1 - p_x)}{1 - p_x} < 0\\
    &\implies P(Z = 1 \mid X = 1, Y = i)\Bigg(1 - \frac{p_x}{1 - p_x}\Bigg) < \frac{(1 - p_x) - p^\prime_{11}}{1 - p_x}\\
    &\implies P(Z = 1 \mid X = 1, Y = i)\Bigg(\frac{(1 - p_x) - p_x}{1 - p_x}\Bigg) < \frac{(1 - p_x) - p^\prime_{11}}{1 - p_x}\\
    &\implies P(Z = 1 \mid X = 1, Y = i)< \frac{(1 - p_x) - p^\prime_{11}}{(1 - p_x) - p_x}
\end{align*}
This concludes the proof.
\end{proof}

\begin{lemma}
    Assume $p_x > 1 - p_x$. If $p^\prime_{10} \geq p_x$, then 
    \[
    p_{11} - y_0 \geq \frac{p_{y_0}((1 - p_x) - p^\prime_{10})}{p_x - (1 - p_x)} + p_{11}
    \]
\end{lemma}
\begin{proof}
    Following a proof by contra-positive, the contra-positive is given as
    \begin{align*}
        p_{11} - y_0 < \frac{p_{y_0}((1 - p_x) - p^\prime_{10})}{p_x - (1 - p_x)} + p_{11} \implies p^\prime_{10} < p_x
    \end{align*}
    To see this, note that
    \begin{align*}
        &p_{11} - p_{y_0} < \frac{p_{y_0}((1 - p_x) - p^\prime_{10})}{p_x - (1 - p_x)} + p_{11}\\
        &\implies - 1 < \frac{((1 - p_x) - p^\prime_{10})}{p_x - (1 - p_x)}\\
        &\implies  p_x  >  p^\prime_{10}
    \end{align*}
    This concludes the proof.
\end{proof}

\begin{lemma}
    Assume $p_x > 1 - p_x$. If $p^\prime_{10} < p_x$, then 
    \[
    \frac{p_{11}p_x - p^\prime_{10}p_{y_0}}{p_x} < \frac{p_{y_0}((1 - p_x) - p^\prime_{10})}{p_x - (1 - p_x)} + p_{11}
    \]
\end{lemma}

\begin{proof}
    Following a proof by contra-positive, the contra-positive is given as
    \[
    \frac{p_{11}p_x - p^\prime_{10}p_{y_0}}{p_x} \geq \frac{p_{y_0}((1 - p_x) - p^\prime_{10})}{p_x - (1 - p_x)} + p_{11} \implies p^\prime_{10} \geq p_x
    \]
    To see this, note that
    \begin{align*}
        &\frac{p_{11}p_x - p^\prime_{10}p_{y_0}}{p_x} \geq \frac{p_{y_0}((1 - p_x) - p^\prime_{10})}{p_x - (1 - p_x)} + p_{11}\\
        &\implies \frac{- p^\prime_{10}}{p_x} \geq \frac{((1 - p_x) - p^\prime_{10})}{p_x - (1 - p_x)}\\
        &\implies - p^\prime_{10}p_x + p^\prime_{10}(1 - p_x) \geq (1 - p_x)p_x - p^\prime_{10}p_x\\
        &\implies p^\prime_{10} \geq p_x
    \end{align*}
    This concludes the proof.
\end{proof}

\begin{lemma}
    Assume $p_x > 1 - p_x$. If $p^\prime_{1i} \geq p_x$ for $i \in \{1, \dots , N\}$, then 
    \begin{align*}
            1 \leq \frac{p^\prime_{1i} - (1 - p_x)}{p_x - (1 - p_x)}    
    \end{align*}
\end{lemma}

\begin{proof}
    A similar proof by contra-positive can be carried out to see this. 
\end{proof}

\begin{lemma}
    Assume $p_x > 1 - p_x$. If $p^\prime_{1i} < x$ for $i \in \{1, \dots , N\}$, then 
    \begin{align*}
            \frac{p^\prime_{11}}{p_x} > \frac{p^\prime_{1i} - (1 - p_x)}{p_x - (1 - p_x)}    
    \end{align*}
\end{lemma}

\begin{proof}
    Following a proof by contra-positive, the contra-positive is given as
    \[
    \frac{p^\prime_{11}}{p_x} \leq \frac{p^\prime_{1i} - (1 - p_x)}{p_x - (1 - p_x)} \implies p^\prime_{1i} \geq x
    \]
    To see this, note that
    \begin{align*}
        &\frac{p^\prime_{11}}{p_x} \leq \frac{p^\prime_{1i} - (1 - p_x)}{p_x - (1 - p_x)}\\
        &\implies p^\prime_{11}p_x - p^\prime_{11}(1 - p_x) \leq p^\prime_{1i}p_x - p_x(1 - p_x)\\
        &\implies p^\prime_{11} \geq p_x
    \end{align*}
    This concludes the proof.
\end{proof}

%%%%%%%%%%%%%%%%%%%%%%%%%%%%%%%%%%%%%%%%%%%%%%%%%%%%%%%%%
\begin{lemma}
    Assume $p_x < 1 - p_x$. If $p^\prime_{10} \geq 1 - p_x$, then 
    \[
     \frac{(1 - p_x)p_{y_0} + p_{11}p_x - p^\prime_{10}p_{y_0}}{p_x} \leq \frac{p_{y_0}( p^\prime_{10} - (1 - p_x))}{(1 - p_x) - p_x} + p_{11}   
    \]
\end{lemma}
\begin{proof}
    Following a proof by contra-positive, the contra-positive is given as
    \begin{align*}
    \frac{(1 - p_x)p_{y_0} + p_{11}p_x - p^\prime_{10}p_{y_0}}{p_x} > \frac{p_{y_0}( p^\prime_{10} - (1 - p_x))}{(1 - p_x) - p_x} + p_{11}  \implies p^\prime_{10} < 1 - p_x
    \end{align*}
    To see this, note that
    \begin{align*}
        &\frac{(1 - p_x)p_{y_0} + p_{11}p_x - p^\prime_{10}p_{y_0}}{p_x} > \frac{p_{y_0}( p^\prime_{10} - (1 - p_x))}{(1 - p_x) - p_x} + p_{11}\\
        &\implies \frac{(1 - p_x) - p^\prime_{10}}{p_x} > \frac{p^\prime_{10} - (1 - p_x)}{(1 - p_x) - p_x} \\
        &\implies (1 - p_x)((1 - p_x) - p_x) - p^\prime_{10}((1 - p_x) - p_x) > p^\prime_{10}p_x - (1 - p_x)p_x \\
        &\implies (1 - p_x)(1 - p_x) - p^\prime_{10}(1 - p_x) > 0  \\
        &\implies  (1 - p_x) > p^\prime_{10} 
    \end{align*}
    This concludes the proof.
\end{proof}

\begin{lemma}
    Assume $p_x < 1 - p_x$. If $p^\prime_{10} < 1 - p_x$, then 
    \[
    p_{11} > \frac{p_{y_0}( p^\prime_{10} - (1 - p_x))}{(1 - p_x) - p_x} + p_{11}
    \]
\end{lemma}

\begin{proof}
    Following a proof by contra-positive, the contra-positive is given as
    \[
    p_{11} \leq \frac{p_{y_0}( p^\prime_{10} - (1 - p_x))}{(1 - p_x) - p_x} + p_{11} \implies p^\prime_{10} \geq 1 - p_x
    \]
    To see this, note that
    \begin{align*}
        & p_{11} \leq \frac{p_{y_0}( p^\prime_{10} - (1 - p_x))}{(1 - p_x) - p_x} + p_{11}\\
        &\implies 0 \leq \frac{p_{y_0}( p^\prime_{10} - (1 - p_x))}{(1 - p_x) - p_x}\\
        &\implies p^\prime_{10} \geq 1 - p_x
    \end{align*}
    This concludes the proof.
\end{proof}

\begin{lemma}
    Assume $p_x < 1 - p_x$. If $p^\prime_{1i} \geq 1 - p_x$ for $i \in \{1, \dots , N\}$, then 
    \begin{align*}
            \frac{p^\prime_{1i} - (1 - p_x)}{p_x} \geq \frac{(1 - p_x) - p^\prime_{1i}}{(1 - p_x) - p_x}    
    \end{align*}
\end{lemma}

\begin{proof}
    Following a proof by contra-positive, the contra-positive can be written as
    \[
    \frac{p^\prime_{1i} - (1 - p_x)}{p_x} < \frac{(1 - p_x) - p^\prime_{1i}}{(1 - p_x) - p_x} \implies p^\prime_{1i} < 1 - p_x
    \]
    To see this, note that
    \begin{align*}
        &\frac{p^\prime_{1i} - (1 - p_x)}{p_x} < \frac{(1 - p_x) - p^\prime_{1i}}{(1 - p_x) - p_x}\\
        &\implies p^\prime_{1i}(1 - p_x) - (1 - p_x)(1 - p_x) < 0\\
        &\implies p^\prime_{1i}(1 - p_x) < 1 - p_x
    \end{align*}
    This concludes the proof.
\end{proof}

\begin{lemma}
    Assume $p_x < 1 - p_x$. If $p^\prime_{1i} < 1 - p_x$ for $i \in \{1, \dots , N\}$, then 
    \begin{align*}
            0 < \frac{(1 - p_x) - p^\prime_{1i}}{(1 - p_x) - p_x}       
    \end{align*}
\end{lemma}

\begin{proof}
    A similar proof by contradiction can be followed to prove the Lemma. 
\end{proof}

\begin{lemma}
    Let $X$, $Z$ and $Y$ be binary random variables obeying the causal structure in \ref{fig:causal-graph}. Then, if the following conditions hold,
    \begin{align*}
        x &> 1 - x\\
        p^\prime_{11} &\geq x\\
        p^\prime_{10} &\geq x\\
    \end{align*}
    Then $\implies \Phi_X > 0$.
\end{lemma}

\begin{proof}
    Since $P(Z, X)$ and $P(Z, Y)$ are marginals of $P(Z , X, Y)$, the following holds
    \[
    p_{11}x + p_{10}(1 - x) = p^\prime_{11}y_1 + p^\prime_{10}y_0
    \]
    Since $x > 1 - x$
    \begin{align*}
        \implies p_{11}x + p_{10}x > p^\prime_{11}y_1 + p^\prime_{10}y_0\\
        \intertext{Since $p^\prime_{11} \geq x$ and $p^\prime_{11} \geq x$}
        \implies p_{11}x + p_{10}x > xy_1 + xy_0\\
        \implies p_{11}x + p_{10}x > x \implies p_{11} + p_{10} > 1\\
        \implies \Phi_X > 0
    \end{align*}
\end{proof}

\begin{lemma}
    Let $X$, $Z$ and $Y$ be binary random variables obeying the causal structure in \ref{fig:causal-graph}. Then, if the following conditions hold,
    \begin{align*}
        1 - x &> x\\
        p^\prime_{11} &\geq 1 - x\\
        p^\prime_{10} &\geq 1 - x\\
    \end{align*}
    Then $\implies \Phi_X > 0$.
\end{lemma}

\begin{proof}
    Since $P(Z, X)$ and $P(Z, Y)$ are marginals of $P(Z , X, Y)$, the following holds
    \[
    p_{11}x + p_{10}(1 - x) = p^\prime_{11}y_1 + p^\prime_{10}y_0
    \]
    Since $x > 1 - x$
    \begin{align*}
        \implies p_{11}(1 - x) + p_{10}(1 - x) > p^\prime_{11}y_1 + p^\prime_{10}y_0\\
        \intertext{Since $p^\prime_{11} \geq 1 - x$ and $p^\prime_{11} \geq 1 - x$}
        \implies p_{11}(1 - x) + p_{10}(1 - x) > (1 - x)y_1 + (1 - x)y_0\\
        \implies p_{11}(1 - x) + p_{10}(1 - x) > 1 - x\\
        \implies \Phi_X > 0
    \end{align*}
\end{proof}

\begin{lemma}
    Let $X$, $Z$ and $Y$ be binary random variables obeying the causal structure in \ref{fig:causal-graph}. Then, if the following conditions hold,
    \begin{align*}
        x &> 1 - x\\
        p^\prime_{11} &\leq 1 - x\\
        p^\prime_{10} &\leq 1 - x\\
    \end{align*}
    Then $\implies \Phi_X < 0$.
\end{lemma}

\begin{proof}
    Since $P(Z, X)$ and $P(Z, Y)$ are marginals of $P(Z , X, Y)$, the following holds
    \[
    p_{11}x + p_{10}(1 - x) = p^\prime_{11}y_1 + p^\prime_{10}y_0
    \]
    Since $p^\prime_{11} \leq 1 - x$ and $p^\prime_{11} \leq 1 - x$
    \begin{align*}
        \implies p_{11}x + p_{10}(1 - x) \leq (1 - x)y_1 + (1 - x)y_0\\
        \intertext{Since $1 - x < x$}
        \implies p_{11}(1 - x) + p_{10}(1 - x) < (1 - x)y_1 + (1 - x)y_0\\
        \implies p_{11} + p_{10} < 1 \implies \Phi_X < 0
    \end{align*}
\end{proof}

\begin{lemma}
    Let $X$, $Z$ and $Y$ be binary random variables obeying the causal structure in \ref{fig:causal-graph}. Then, if the following conditions hold,
    \begin{align*}
        1 - x &> x\\
        p^\prime_{11} &\leq x\\
        p^\prime_{10} &\leq x\\
        \implies& \Phi_X < 0
    \end{align*}
\end{lemma}

\begin{proof}
    A similar proof as above can be followed to obtain the result of this Lemma. 
\end{proof}

\begin{lemma}\label{lem:a-leq-b}
    Assume $x > 1 - x$. Denote $\Phi_X = p_{11} + p_{10} - 1$, and denote $a$ and $b$ as 
    \begin{align*}
            a &= \frac{y_0((1 - x) - p^\prime_{10})}{y_1(x - (1 - x))} + \frac{p_{11}}{y_1}\\
            b &= \frac{p^\prime_{11} - (1 - x)}{x - (1 - x)}    
    \end{align*}
    Then, $\Phi_X \geq 0 \implies a \leq b$
\end{lemma}
\begin{proof}
We utilize a proof of contrapositive, where the contrapositive of the above statement is
\[
a > b \implies \Phi_X < 0
\]
\begin{align*}
    \implies \frac{y_0((1 - x) - p^\prime_{10})}{y_1(x - (1 - x))} + \frac{p_{11}}{y_1} &> \frac{p^\prime_{11} - (1 - x)}{x - (1 - x)}\\
    \implies \frac{y_0((1 - x) - p^\prime_{10})}{y_1(x - (1 - x))} + \frac{p_{11}(x - (1 - x))}{y_1(x - (1 - x))} &> \frac{p^\prime_{11}y_1 - y_1(1 - x)}{y_1(x - (1 - x))}\\
    \implies y_0((1 - x) - p^\prime_{10}) + p_{11}(x - (1 - x)) &> p^\prime_{11}y_1 - y_1(1 - x)\\
    \implies (1 - x) + p_{11}(x - (1 - x)) &> p^\prime_{11}y_1 + p^\prime_{10}y_0 \\
    \implies 0 > \Phi_X 
\end{align*}
\end{proof}
\begin{lemma}\label{lem:a-geq-b}
    Assume $x > 1 - x$. Denote $\Phi_X = p_{11} + p_{10} - 1$, and denote $a$ and $b$ as 
    \begin{align*}
            a &= \frac{y_0((1 - x) - p^\prime_{10})}{y_1(x - (1 - x))} + \frac{p_{11}}{y_1}\\
            b &= \frac{p^\prime_{11} - (1 - x)}{x - (1 - x)}    
    \end{align*}
    Then, $\Phi_X < 0 \implies a > b$
\end{lemma}
\begin{proof}
The contrapositive has been shown to hold from the Lemma above, hence the Lemma holds. 

\end{proof}

\textbf{Proof for Lemma \ref{lemma:RREF-y-delta}:} This lemma is proved in two steps, first using mathematical induction performed on the the Reduced Row Echelon Form (RREF) of the matrix representation of the system of equations that Equation XXXX, then, simplifying the final RREF based on properties of probability distributions. 

First, the equations for invariances provided in Eq. XXX are given as 

\begin{align*}
        p^T_{10} &= \sum_{j = 0}^N P^T(Z = 1\mid X = 0, Y = j)p_{y_j}\\
        p^T_{11} &= \sum_{j = 0}^N P^T(Z = 1\mid X = 1, Y = j)p_{y_j}\\
        p^E_{10} &= P^T(Z = 1\mid X = 0, Y = 0)(1 - p_x - \delta^i_X)\\
        &\hspace{0.2in} + P^T(Z = 1\mid X = 1, Y = 0)(p_x + \delta^i_X)\\
        \vdots\\
        p^E_{1N} &= P^T(Z = 1\mid X = 0, Y = N)(1 - p_x - \delta^i_X)\\
        &\hspace{0.2in} + P^T(Z = 1\mid X = 1, Y = N)(p_x + \delta^i_X)\\
\end{align*}

The above equations can be represented in matrix form $A\mathbf{x} = b$ as
{\scriptsize
\begin{align*}
A &= \begin{bmatrix}
    p_{y_0} & 0 & p_{y_1} & 0 & \dots & p_{y_{N - 1}} & 0 & p_{y_N} & 0\\
    0 & p_{y_0} & 0 & p_{y_1} & \dots & 0 & p_{y_{N - 1}}& 0 & p_{y_N}\\
    1 - p_{x} - \delta_X & p_{x} + \delta_X & 0 & 0 & \dots & 0 & 0 & 0 & 0\\
    0 & 0 & 1 - p_x - \delta_X & p_x + \delta_X & \dots & 0 & 0 & 0 & 0\\
    \vdots & \ddots & & & & & & & \vdots\\
    0 & 0 & \dots & 0 & 0 & 1 - p_x - \delta_X & p_x + \delta_X & 0 & 0\\
    0 & 0 & \dots & 0 & & 0 & 0 & 1 - p_x - \delta_X & p_x + \delta_X\\
\end{bmatrix}\\
b &= \begin{bmatrix}
    p^T_{10}\\
    p^T_{11}\\
    p^E_{10}\\
    p^E_{11}\\
    p^E_{12}
    \vdots\\
    p^E_{1(N - 1)}\\
    p^E_{1N}\\
\end{bmatrix}
\hspace{1in}\mathbf{x} 
= \begin{bmatrix}
P^T(Z = 1 \mid X = 0, Y = 0)\\    
P^T(Z = 1 \mid X = 1, Y = 0)\\
P^T(Z = 1 \mid X = 0, Y = 1)\\    
P^T(Z = 1 \mid X = 1, Y = 1)\\
\vdots\\
P^T(Z = 1 \mid X = 0, Y = N)\\    
P^T(Z = 1 \mid X = 1, Y = N)\\
\end{bmatrix}
\end{align*}
}
Next, denote the augmented matrix $A | b$ as 
{\small
\begin{align*}
    \begin{bmatrix}[ccccccccc|c]
    p_{y_0} & 0 & p_{y_1} & 0 & \dots & p_{y_{N - 1}} & 0 & p_{y_N} & 0 & p_{10}\\
    0 & p_{y_0} & 0 & p_{y_1} & \dots & 0 & p_{y_{N - 1}}& 0 & p_{y_N} & p_{11}\\
    1 - p_x - \delta_X & p_x + \delta_X & 0 & 0 & \dots & 0 & 0 & 0 & 0 & p^E_{10}\\
    0 & 0 & 1 - p_x - \delta_X & p_x + \delta_X & \dots & 0 & 0 & 0 & 0 & p^E_{11}\\
    \vdots & \ddots & & & & & & & \vdots & \vdots \\
    0 & 0 & \dots & 0 & 0 & 1 - p_x - \delta_X & p_x + \delta_X & 0 & 0 & p^E_{1(N - 1)}\\
    0 & 0 & \dots & 0 & & 0 & 0 & 1 - p_x - \delta_X & p_x + \delta_X & p^E_{1N}\\
    \end{bmatrix}
\end{align*}
}
First, we utilize mathematical induction to provide a general form for the RREF of $A|b$ for any $N$. Formally, let $P(N)$ denote the following proposition. \\
\textbf{Proposition}: Let $P(N)$ denote the proposition that the support of $Y$ has a cardinality of $N + 1$, then $A|b$ will be a matrix with $N + 3$ rows and $2(N + 1) + 1$ columns. The following steps when executed will put $A|b$ in RREF, where $R_i$ denotes the $i$-th row of $A|b$

\begin{enumerate}
    \item 
        \begin{align}
        R_1 &= R_1/p_{y_0}\\
        R_3 &= R_3 - (1 - p_x - \delta_X)R_1
        \end{align}\label{step-1}
    \item
        \begin{align}
        R_2 &= R_2/p_{y_0}\\
        R_3 &= R_3 - (p_x + \delta_X)R_2
        \end{align}\label{step-2}
    \item 
        \begin{align}
        R_3 &= R3/(-\frac{(1 - p_x - \delta_X)p_{y_1}}{p_{y_0}})\\
        R_1 &= R_1 - \frac{p_{y_1}}{p_{y_0}}R3\\
        R_4 &= R4 - (1 - p_x - \delta_X)R3
        \end{align}\label{step-3}
    \item If $N \geq 2$, then loop through the following steps for $i \in \{2, \dots, N\}$:
    \begin{align}
        R_{2 + i} = R_{2 + i}/(-\frac{p_{y_i}(1 - p_x - \delta_X)}{p_{y_{i - 1}}})\\
        R_{1 + i} = R_{1 + i} - \frac{p_{y_{i}}}{p_{y_{i - 1}}}R_{2 + i}\\
        R_{3 + i} = R_{3 + i} - (1 - p_x - \delta_X)R_{2 + i}
    \end{align}\label{step-n}
\end{enumerate}

And the corresponding matrix will evaluate to
{\small
\begin{align}\label{matrix:rref-delta-x} 
    \begin{bmatrix}
    1 &  0 &  0 &  -\frac{(p_x + \delta_X) p_{y_1}}{(1 - p_x - \delta_X)p_{y_0}} & \dots & 0 & -\frac{(p_x + \delta_X)p_{y_{N - 1}}}{(1 - p_x - \delta_X)p_{y_0}} & 0 & -\frac{(p_x + \delta_X)p_{y_N}}{(1 - p_x - \delta_X)p_{y_0}} & \frac{p^E_{10}p_{y_0} - p^T_{11}(p_x + \delta_X)}{(1 - p_x - \delta_X)p_{y_0}}\\
    0 &  1 &  0 & \frac{p_{y_1}}{p_{y_0}} & \dots & 0 & \frac{p_{y_{N - 1}}}{p_{y_0}} & 0 & \frac{p_{y_N}}{p_{y_0}} & \frac{p^T_{11}}{p_{y_0}}\\
    0 &  0 &  1 & \frac{p_x + \delta_X}{1 - p_x - \delta_X} &  \dots & 0 & 0 & 0 &  0 & \frac{p^E_{11}}{1 - p_x - \delta_X}\\
    \vdots &&&&&&& \ddots \\
    0 &  0 &  0 & 0 & \dots & 0 & 0 & 1 & \frac{p_x + \delta_X}{1 - p_x - \delta_X} & \frac{p^T_{10}(1 - p_x - \delta_X) + p^T_{11}(p_x + \delta_X) - \sum_{i = 0}^{N - 1} p^E_{1i}p_{y_i}}{p_{y_N}(1 - p_x - \delta_X)}\\
    0 &  0 &  0 & 0 & \dots & 0 & 0 & 0 & 0 & \frac{\sum_{i = 0}^{N} p^E_{1i}p_{y_i} - p^T_{10}(1 - p_x - \delta_X) - p^T_{11}(p_x + \delta_X)}{p_{y_N}} 
    \end{bmatrix}
\end{align}
}
An identical proof used in Lemma \ref{lemma:RREF-y} can be applied to prove this induction. Next, to complete this proof for this lemma, we prove the following identities. 
\[\frac{\sum_{j = 0}^{N} p^E_{1j}p_{y_j} - p^T_{10}(1 - p_x - \delta_X) - p^T_{11}(p_x + \delta_X)}{p_{y_N}} = 0\]

To prove this, note that
\[  p^T_{10}(1 - p_x - \delta_X) &= \sum_{j = 0}^N P^T(Z = 1\mid X = 0, Y = j)p_{y_j}(1 - p_x - \delta_X)\]
Along with
\[
p^T_{11}(p_x + \delta_X) = \sum_{j = 0}^N P^T(Z = 1\mid X = 1, Y = j)p_{y_j}(p_x + \delta^i_X)
\]
Consequently, 
\begin{align*}
    &p^T_{10}(1 - p_x - \delta^0_X) + p^T_{11}(p_x + \delta^i_X) = \\
    & \sum_{j = 0}^N p_{y_j}\Bigg(P^T(Z = 1\mid X = 0, Y = j)(1 - p_x - \delta^0_X) + P^T(Z = 1\mid X = 1, Y = j)(p_x + \delta^i_X)\Bigg)\\
    &= \sum_{j = 0}^N p_{y_j}\Bigg(P^E(Z = 1\mid X = 0, Y = j)P^E(X = 0) + P^E(Z = 1\mid X = 1, Y = j)P^E(X = 1)\Big)\\
    &= \sum_{j = 0}^N p_{y_j}p^E_{1j}
\end{align*}

And this will be subtracted from $\sum_{j = 0}^N p_{y_j}p^E_{1ji}$, hence it equals $0$. 
\[
\frac{p^T_{10i}(1 - p_x- \delta^i_X) + p^T_{11i}(p_x + \delta^i_X) - \sum_{j = 0}^{N - 1} p^E_{1ji}p_{y_j}}{p_{y_N}(1 - p_x - \delta^i_X)} = 
\]

Following a similar approach as before, this will simplify to
\begin{align*}
    \frac{\sum_{j = 0}^N p_{y_j}p^E_{1j} - \sum_{j = 0}^{N - 1} p_{y_j}p^E_{1j}}{p_{y_N}(1 - p_x - \delta^i_X)} = \frac{p^E_{1N}}{1 - p_x - \delta^i_X}
\end{align*}
This concludes the proof of the Lemma.


\begin{lemma}\label{RREF-y-c}
    Let $X$ and $Z$ be binary random variables, and let $C$ and $Y$ be discrete random variables taking values in $\{0, \dots, M\}$ and $\{0, \dots , N\}$ respectively. Let $\delta^C_X$ represent the link between the treatment assignment mechaism between the $P^E$ and $P^T$ as follows
    \[
    P^E(X = 1\mid C) = P^T(X = 1) + \delta^C_X
    \]
    For notational ease, we introduce the following terms. Let $P^T(Z = 1 \mid X = j, C = i)$ be denoted by $p^T{1ji}$ and let $P^E(Z = 1 \mid Y = j, C = i)$ be denoted as $p^E_{1ji}$. Given distributions $P^T(Z, X, C)$ and $P^E(Z, Y, C)$ obeying the following contraints
    \begin{align*}
        p^T_{10i} &= \sum_{j = 0}^N P(Z = 1\mid X = 0, Y = j, C = i)p_{y_j}\\
        p^T_{11i} &= \sum_{j = 0}^N P(Z = 1\mid X = 1, Y = j, C = i)p_{y_j}\\
        p^E_{10i} &= P(Z = 1\mid X = 0, Y = 0, C = i)(1 - p_x - \delta^i_X)\\
        &\hspace{0.2in} + P(Z = 1\mid X = 1, Y = 0, C = i)(p_x + \delta^i_X)\\
        \vdots\\
        p^E_{1Ni} &= P(Z = 1\mid X = 0, Y = N, C = i)(1 - p_x - \delta^i_X)\\
        &\hspace{0.2in} + P(Z = 1\mid X = 1, Y = N, C = i)(p_x + \delta^i_X)\\
    \end{align*}
    Then this system of equations can be expressed in terms of free parameters $P(Z = 1 \mid X = 1, Y = i, C)$ for $i \in \{1, \dots, N\}$ and all $C$ as
    {\small
    \begin{align*}
    \mathbb{P}(Z = 1 \mid X = 0, Y = 0, C) &=  \frac{p_x + \delta^C_X}{1 - p_x - \delta^C_X}\sum_{n = 1}^N\frac{p_{y_n}}{p_{y_0}}\mathbb{P}(Z = 1 \mid X = 1, Y = n) + \frac{p^E_{10C}p_{y_0} - p^T_{11C}(p_x +\delta^C_X)}{(1 - p_x - \delta^C_X)p_{y_0}}\\
    \mathbb{P}(Z = 1 \mid X = 1, Y = 0, C)&= \frac{p^T_{11C}}{p_{y_0}} - \sum_{n = 1}^N\frac{p_{y_n}}{p_{y_0}}\mathbb{P}(Z = 1 \mid X = 1, Y = n, C)\\
    \mathbb{P}(Z = 1 \mid X = 0, Y = 1, C)&= \frac{p^E_{11C}}{1 - p_x - \delta^C_X} - \frac{p_x + \delta^C_X}{1 - p_x - \delta^C_X}\mathbb{P}(Z = 1 \mid X = 1, Y = 1, C)\\
    \mathbb{P}(Z = 1 \mid X = 0, Y = 2, C)&= \frac{p^E_{12C}}{1 - p_x - \delta^C_X} - \frac{p_x + \delta^C_X}{1 - p_x - \delta^C_X}\mathbb{P}(Z = 1 \mid X = 1, Y = 2, C)\\
    \vdots\\
    \mathbb{P}(Z = 1 \mid X = 0, Y = N, C)&= \frac{p^E_{1N}}{1 - p_x - \delta^C_X} - \frac{p_x + \delta^C_X}{1 - p_x - \delta^C_X}\mathbb{P}(Z = 1 \mid X = 1, Y = N, C)\\
    \end{align*}
    }
\end{lemma}

\begin{proof}
The proof for this Lemma follows two major steps, the first being a proof by double mathematical induction to represent the Reduced Row Echelon Form (RREF) for the system of equations for arbitrary dimensionality of $Y$ and $C$. The second part of the proof applies properties of probability distributions to express the system of equations in the form given in the Lemma.     

We start start with the proof by double mathematical induction, and state the proposition we prove. 

\textbf{Proposition}: Let $P(m, n)$ denote the proposition that given the system of equations corresponding to the constraints provided in Lemma, represented in matrix form $A_{m, n}\mathbf{x}_{m ,n } = \mathbf{b}_{m , n}$ provided below.
{\scriptsize
\begin{align*}
A_{m, n} &= \begin{bmatrix}
            A_{0, n} & [\mathbf{0}] & \dots & [\mathbf{0}]\\
            [\mathbf{0}] & A_{1, n} & \dots & [\mathbf{0}]\\
            [\mathbf{0}] & [\mathbf{0}] & \ddots & [\mathbf{0}]\\
            [\mathbf{0}] & [\mathbf{0}] & \dots & A_{m, n}
            \end{bmatrix}
\hspace{0.2in} b_{m, n} = \begin{bmatrix}
                            b_{0, n}\\
                            \vdots\\
                            b_{m, n}
                          \end{bmatrix}
\hspace{0.2in} \mathbf{x}_{m , n} = \begin{bmatrix}
                                    \mathbf{x}_{0, n}\\
                                    \vdots\\
                                    \mathbf{x}_{m, n}
                                    \end{bmatrix}
\intertext{Where $A_{i, n}$, $b_{i, n}$ and $\mathbf{x}_{i, n}$ will be of the form}
A_{i, n} &= \begin{bmatrix}
    p_{y_0} & 0 & p_{y_1} & 0 & \dots & p_{y_{N - 1}} & 0 & p_{y_N} & 0\\
    0 & p_{y_0} & 0 & p_{y_1} & \dots & 0 & p_{y_{N - 1}}& 0 & p_{y_N}\\
    1 - p_{x} - \delta^i_X & p_{x} + \delta^i_X & 0 & 0 & \dots & 0 & 0 & 0 & 0\\
    0 & 0 & 1 - p_x - \delta^i_X & p_x + \delta^i_X & \dots & 0 & 0 & 0 & 0\\
    \vdots & \ddots & & & & & & & \vdots\\
    0 & 0 & \dots & 0 & 0 & 1 - p_x - \delta^i_X & p_x + \delta^i_X & 0 & 0\\
    0 & 0 & \dots & 0 & & 0 & 0 & 1 - p_x - \delta^i_X & p_x - \delta^i_X\\
\end{bmatrix}\\
b_{i, n} &= \begin{bmatrix}
             p^T_{10i}\\
             p^T_{11i}\\
             p^E_{10i}\\
             p^E_{11i}\\
             p^E_{12i}
             \vdots\\
             p^E_{1(n - 1)i}\\
             p^E_{1ni}\\
            \end{bmatrix}
\hspace{1in} \mathbf{x}_{i, n} = \begin{bmatrix}
                                P(Z = 1 \mid X = 0, Y = 0, C = i)\\    
                                P(Z = 1 \mid X = 1, Y = 0, C = i)\\
                                P(Z = 1 \mid X = 0, Y = 1, C = i)\\    
                                P(Z = 1 \mid X = 1, Y = 1, C = i)\\
                                \vdots\\
                                P(Z = 1 \mid X = 0, Y = N, C = i)\\    
                                P(Z = 1 \mid X = 1, Y = N, C = i)\\
                                \end{bmatrix}
\end{align*}
}
Given this system of equations, the RREF of the augmented matrix ${A \mid b}_{m, n}$ corresponding to this system of equations will be of the form
\begin{align*}
    {A \mid b}^R_{m, n} = \begin{bmatrix}
                        A^R_{0, n} & [\mathbf{0}] & [\mathbf{0}] & b^R_{0, n} \\
                        [\mathbf{0}] & A^R_{1, n} & [\mathbf{0}] & b^R_{1, n}\\
                        [\mathbf{0}] & [\mathbf{0}] & \ddots & \vdots \\
                        [\mathbf{0}] & \dots & A^R_{m, n} & b^R_{m, n} \\
                        0 & \dots & 0 & \frac{\sum_{j = 0}^{N} p^E_{1j0}p_{y_j} - p^T_{10}(1 - p_x - \delta^0_X) - p^T_{110}(p_x + \delta^0_X)}{p_{y_N}}\\
                        \vdots & \dots & 0 & \vdots\\
                        0 & \dots & 0 & \frac{\sum_{j = 0}^{N} p^E_{1j0}p_{y_j} - p^T_{10}(1 - p_x - \delta^0_X) - p^T_{110}(p_x + \delta^0_X)}{p_{y_N}}\\
                \end{bmatrix}
\end{align*}
Where $A^R_{i, n}$ and $b^R_{i, n}$ will be of the form
\begin{align*}
    \label{matrix:rref-with-covariates} 
    A^R_{i, n} = \begin{bmatrix}
    1 &  0 &  0 &  -\frac{(p_x + \delta^i_X)p_{y_1}}{(1 - p_x - \delta^i_X)p_{y_0}} & \dots & 0 & -\frac{(p_x + \delta^i_X) p_{y_{N - 1}}}{(1 - p_x - \delta^i_X)p_{y_0}} & 0 & -\frac{(p_x + \delta^i_X)p_{y_N}}{(1 - p_x- \delta^i_X)p_{y_0}}\\
    0 &  1 &  0 & \frac{p_{y_1}}{p_{y_0}} & \dots & 0 & \frac{p_{y_{N - 1}}}{p_{y_0}} & 0 & \frac{p_{y_N}}{p_{y_0}}\\
    0 &  0 &  1 & \frac{p_x + \delta^i_X}{1 - p_x - \delta^i_X} &  \dots & 0 & 0 & 0 &  0\\
    \vdots &&&&&&& \ddots\\
    0 &  0 &  0 & 0 & \dots & 0 & 0 & 1 & \frac{p_x + \delta^i_X}{1 - p_x - \delta^i_X} \\
    \end{bmatrix}
\end{align*}

And $b^R_{i, n}$ will be of the form
\begin{align*}
\begin{bmatrix}
    \frac{p^E_{10i}p_{y_0} - p^T_{11i}p_x}{(1 - p_x - \delta^i_X)p_{y_0}}\\
    \frac{p^T_{11i}}{p_{y_0}}\\
    %\frac{p^E_{11i}}{1 - p_x - \delta^i_X}\\
    \vdots\\
    \frac{p^T_{10i}(1 - p_x- \delta^i_X) + p^T_{11i}(p_x + \delta^i_X) - \sum_{j = 0}^{N - 1} p^E_{1ji}p_{y_j}}{p_{y_N}(1 - p_x - \delta^i_X)}
    % \frac{\sum_{j = 0}^{N} p^E_{1ji}p_{y_j} - p_{10}(1 - p_x - \delta^i_X) - p^T_{11i}(p_x + \delta^i_X)}{p_{y_N}} 
\end{bmatrix}    
\end{align*}

To prove $P(m, n)$ using double mathematical induction, we first prove the base case with $m = n = 1$.\\
\newline
\textbf{Base Case}: Using a symbolic solver to put the matrix in RREF, we obtain the RREF form of $A \mid b$ as
{\scriptsize
\begin{align*}
\begin{bmatrix}
1 &  0 &  0 &  -\frac{p_{y_1}(\delta^0_X + p_x)}{p_{y_0}(1 - p_x - \delta^0_X)} &  0 &  0 &  0 & 0 & \frac{p^E_{100}p_{y_0} - p^T_{110}(\delta^0_X + p_x)}{p_{y_0}(1 - p_x - \delta^0_X)}\\
0 &  1 &  0 & \frac{p_{y_1}}{p_{y_0}} &  0 &  0 &  0 & 0 & \frac{p^T_{110}}{p_{y_0}}\\
0 &  0 &  1 & \frac{\delta^0_X + x}{1 - x - \delta^0_X} &  0 &  0 &  0 & 0 & \frac{p^T_{100}(1 - p_x - \delta^0_X) + p^T_{110}(\delta^0_X + x) - p^E_{100}p_{y_0}}{p_{y_1}(1 - p_x - \delta^0_X)} \\
0 &  0 &  0 & 0 &  1 &  0 &  0 &  -\frac{p_{y_1}(\delta^1_X + x)}{p_{y_0}(1 - p_x - \delta^1_X)} & \frac{p^E_{101}p_{y_0} - p^T_{111}(\delta^1_X + p_x)}{p_{y_0}(1 - p_x - \delta^1_X)}\\
0 &  0 &  0 & 0 &  0 &  1 &  0 & \frac{p_{y_1}}{p_{y_0}} & \frac{p^T_{111}}{p_{y_0}} \\
0 &  0 &  0 & 0 &  0 &  0 &  1 & \frac{p_x + \delta^1_X}{1 - x - \delta^1_X} &  \frac{p^T_{101}(1 - p_x - \delta^1_X) + p^T_{111}(\delta^1_X + x) - p^E_{101}p_{y_0}}{p_{y_1}(1 - p_x - \delta^1_X)}\\
0 &  0 &  0 & 0 &  0 &  0 &  0 & 0 & \frac{p^E_{110}p_{y_1} + p^E_{100}p_{y_0} - p_{100}(1 - p_x - \delta^0_X) - p_{110}(\delta^0_X + p_x)}{p_{y_1}} \\
0 &  0 &  0 & 0 &  0 &  0 &  0 & 0 &  \frac{p^E_{111}p_{y_1} + p^E_{101}p_{y_0} - p^T_{101}(1 - p_x - \delta^1_X) - p_{111}(\delta^1_X + p_x)}{p_{y_1}}
\end{bmatrix}
\end{align*}
}
And by comparison, this matches the base case. Hence the base case holds.\\ 
\newline
\textbf{Induction Step I}: Here we prove that if $P(1, n - 1)$ holds, then $P(1, n)$ holds as well. For $P(1, n)$, $A|b$ will look like

\begin{align*}
{A\mid b}_{1, n} &= \begin{bmatrix}
                    A_{0, n} & [\mathbf{0}] & b_{0, n} \\
                    [\mathbf{0}] & A_{1, n} & b_{1, n}
            \end{bmatrix}
\end{align*}

Since $A_{0, n}$ and $A_{1, n}$ are non-overlapping diagional sub-matrices of ${A \mid b}_{1, n}$, a similar proof to Lemma X for each level of of $C$ can be applied, i.e. for each pair $A_{0, n}$, $b_{0,n}$ and $A_{1, n}$, $b_{1,n}$ to put each of them in their RREF matrix separately. Then the last rows correspoding to the RREF of $A_{0, n}$, $b_{0,n}$ and $A_{1, n}$, $b_{1,n}$ can be shuffled as needed to put ${A \mid b}_{1, n}$ in RREF, proving the first step of the induction.\\
\newline
\textbf{Induction Step II:} Next, we must prove that for all $n \geq 1$, $P(m, n)$ is true then $P(m + 1, n)$ is true. For $P(m + 1, n)$, the system of equations is represented in matrix form as
{\scriptsize
\begin{align*}
A_{m, n} &= \begin{bmatrix}
            A_{0, n} & [\mathbf{0}] & \dots & [\mathbf{0}] & [\mathbf{0}]\\
            [\mathbf{0}] & A_{1, n} & \dots & [\mathbf{0}] & [\mathbf{0}]\\
            [\mathbf{0}] & [\mathbf{0}] & \ddots & [\mathbf{0}] &  [\mathbf{0}]\\
            [\mathbf{0}] & [\mathbf{0}] & \dots & A_{m, n} & [\mathbf{0}]\\
            [\mathbf{0}] & [\mathbf{0}] & \dots & [\mathbf{0}] & A_{m + 1, n}
            \end{bmatrix}
\hspace{0.2in} b_{m, n} = \begin{bmatrix}
                            b_{0, n}\\
                            \vdots\\
                            b_{m, n}\\
                            b_{m + 1, n}
                          \end{bmatrix}
\hspace{0.2in} \mathbf{x}_{m , n} = \begin{bmatrix}
                                    \mathbf{x}_{0, n}\\
                                    \vdots\\
                                    \mathbf{x}_{m, n}\\
                                    \mathbf{x}_{m + 1, n}
                                    \end{bmatrix}
\intertext{Where $A_{i, n}$, $b_{i, n}$ and $\mathbf{x}_{i, n}$ will be of the form}
A_{i, n} &= \begin{bmatrix}
    p_{y_0} & 0 & p_{y_1} & 0 & \dots & p_{y_{N - 1}} & 0 & p_{y_N} & 0\\
    0 & p_{y_0} & 0 & p_{y_1} & \dots & 0 & p_{y_{N - 1}}& 0 & p_{y_N}\\
    1 - p_{x} - \delta^i_X & p_{x} + \delta^i_X & 0 & 0 & \dots & 0 & 0 & 0 & 0\\
    0 & 0 & 1 - p_x - \delta^i_X & p_x + \delta^i_X & \dots & 0 & 0 & 0 & 0\\
    \vdots & \ddots & & & & & & & \vdots\\
    0 & 0 & \dots & 0 & 0 & 1 - p_x - \delta^i_X & p_x + \delta^i_X & 0 & 0\\
    0 & 0 & \dots & 0 & & 0 & 0 & 1 - p_x - \delta^i_X & p_x - \delta^i_X\\
\end{bmatrix}\\
b_{i, n} &= \begin{bmatrix}
             p^T_{10i}\\
             p^T_{11i}\\
             p^E_{10i}\\
             p^E_{11i}\\
             p^E_{12i}
             \vdots\\
             p^E_{1(n - 1)i}\\
             p^E_{1ni}\\
            \end{bmatrix}
\hspace{1in} \mathbf{x}_{i, n} = \begin{bmatrix}
                                P(Z = 1 \mid X = 0, Y = 0, C = i)\\    
                                P(Z = 1 \mid X = 1, Y = 0, C = i)\\
                                P(Z = 1 \mid X = 0, Y = 1, C = i)\\    
                                P(Z = 1 \mid X = 1, Y = 1, C = i)\\
                                \vdots\\
                                P(Z = 1 \mid X = 0, Y = N, C = i)\\    
                                P(Z = 1 \mid X = 1, Y = N, C = i)\\
                                \end{bmatrix}
\end{align*}
}
Since we assume $P(m, n)$ is true, the submatrix corresponding to ${A \mid b}_{m, n}$ in ${A \mid b}_{m + 1, n}$ is non-overlapping with $A_{m + 1, n}$ and $b_{m + 1, n}$, and can be put into RREF form, presented below.
\begin{align*}
    {A \mid b}_{m + 1, n} = \begin{bmatrix}
                        A^R_{0, n} & [\mathbf{0}] & \dots & [\mathbf{0}] & [\mathbf{0}]&  b^R_{0, n} \\
                        [\mathbf{0}] & A^R_{1, n} & \dots & [\mathbf{0}] & [\mathbf{0}] & b^R_{1, n}\\
                        [\mathbf{0}] & [\mathbf{0}] & \ddots & [\mathbf{0}] & [\mathbf{0}] & \vdots \\
                        [\mathbf{0}] & [\mathbf{0}] & \dots & A^R_{m, n} & [\mathbf{0}] & b^R_{m, n} \\
                        0 & \dots & 0 & 0 & [\mathbf{0}] & \frac{\sum_{j = 0}^{N} p^E_{1j0}p_{y_j} - p^T_{10}(1 - p_x - \delta^0_X) - p^T_{110}(p_x + \delta^0_X)}{p_{y_N}}\\
                        \vdots & \dots & 0 & 0 & [\mathbf{0}] & \vdots\\
                        0 & \dots & 0 & 0 & [\mathbf{0}] &\frac{\sum_{j = 0}^{N} p^E_{1j0}p_{y_j} - p^T_{10}(1 - p_x - \delta^0_X) - p^T_{110}(p_x + \delta^0_X)}{p_{y_N}}\\
                        0 & \dots & 0 & 0 & A_{m + 1, n} & b_{m + 1, n}
                \end{bmatrix}
\end{align*}
Now, putting $A_{m+ 1, n}$ and $b_{m + 1, n}$ in RREF form using a similar approach to Lemma X, and shuffling all the rows that only have $0$ in every entry except the last gives us the RREF as stated and proved $P(m + 1, n)$. This concludes the proof of the double induction. 

Next, to complete this proof, we prove the following identities conclude the proof. 
\[\frac{\sum_{j = 0}^{N} p^E_{1ji}p_{y_j} - p^T_{10i}(1 - p_x - \delta^i_X) - p^T_{11i}(p_x + \delta^i_X)}{p_{y_N}} = 0\]

To prove this, note that
\[  p^T_{10i}(1 - p_x - \delta^0_X) &= \sum_{j = 0}^N P(Z = 1\mid X = 0, Y = j, C = i)p_{y_j}(1 - p_x - \delta^0_X)\]
Along with
\[
p^T_{11i}(p_x + \delta^i_X) = \sum_{j = 0}^N P(Z = 1\mid X = 1, Y = j, C = i)p_{y_j}(p_x + \delta^i_X)
\]

Consequently, 
{\small
\begin{align*}
    &p^T_{10i}(1 - p_x - \delta^0_X) + p^T_{11i}(p_x + \delta^i_X) = \\
    & \sum_{j = 0}^N p_{y_j}\Bigg(P(Z = 1\mid X = 0, Y = j, C = i)(1 - p_x - \delta^0_X) + P(Z = 1\mid X = 1, Y = j, C = i)(p_x + \delta^i_X)\Big)\\
    &= \sum_{j = 0}^N p_{y_j}\Bigg(P(Z = 1\mid X = 0, Y = j, C = i)P^E(X = 0 \mid C = i)\\
    &\hspace{0.4in} + P(Z = 1\mid X = 1, Y = j, C = i)P^E(X = 1 \mid C = i)\Big)\\
    &= \sum_{j = 0}^N p_{y_j}p^E_{1ji}
\end{align*}
}
And this will be subtracted from $\sum_{j = 0}^N p_{y_j}p^E_{1ji}$, hence it equals $0$. 
\[
\frac{p^T_{10i}(1 - p_x- \delta^i_X) + p^T_{11i}(p_x + \delta^i_X) - \sum_{j = 0}^{N - 1} p^E_{1ji}p_{y_j}}{p_{y_N}(1 - p_x - \delta^i_X)} = 
\]

Following a similar approach as before, this will simplify to
\begin{align*}
    \frac{\sum_{j = 0}^N p_{y_j}p^E_{1ji} - \sum_{j = 0}^{N - 1} p_{y_j}p^E_{1ji}}{p_{y_N}(1 - p_x - \delta^i_X)} = \frac{p^E_{1Ni}}{1 - p_x - \delta^i_X}
\end{align*}
This concludes the proof of the Lemma.
\end{proof}
\textbf{Proof of Lemma \ref{lem:free-param-bounds-delta}}: Using the result presented in Lemma \ref{lemma:RREF-y-delta}, when $Y$ has support $\{0, \dots, N\}$ and we are given marginals $P(Z, X)$ and $P(Z, Y)$, we can write the system of equations using free parameters as   

{\small
\begin{align*}
P^T(Z = 1 \mid X = 0, Y = 0) &=  \frac{p_x + \delta_X}{1 - p_x - \delta_X}\sum_{n = 1}^N\frac{p_{y_n}}{p_{y_0}}P^T(Z = 1 \mid X = 1, Y = n) + \frac{p^E_{10}p_{y_0} - p^T_{11}(p_x + \delta_X)}{(1 - p_x - \delta_X)p_{y_0}}\\
P^T(Z = 1 \mid X = 1, Y = 0)&= \frac{p^T_{11}}{p_{y_0}} - \sum_{n = 1}^N\frac{p_{y_n}}{p_{y_0}}P^T(Z = 1 \mid X = 1, Y = n)\\
P^T(Z = 1 \mid X = 0, Y = 1)&= \frac{p^E_{11}}{1 - p_x - \delta_X} - \frac{p_x + \deltaXX}{1 - p_x - \delta_X}P^T(Z = 1 \mid X = 1, Y = 1)\\
P^T(Z = 1 \mid X = 0, Y = 2)&= \frac{p^E_{12}}{1 - p_x - \delta_X} - \frac{p_x + \delta_X}{1 - p_x - \delta_X}P^T(Z = 1 \mid X = 1, Y = 2)\\
\vdots\\
P^T(Z = 1 \mid X = 0, Y = N)&= \frac{p^E_{1N}}{1 - p_x - \delta_X} - \frac{p_x + \delta_X}{1 - p_x - \delta_X}P^T(Z = 1 \mid X = 1, Y = N)\\
\end{align*}
}

Now, each of the basic variables in the system above must be a valid probability, i.e. between zero and one, inclusive. Employing these constraints on the free parameters gives
\begin{align*}
    0 &\leq P^T(Z = 1 \mid X = 0, Y = 0) \leq 1\\
    \implies 0 \leq  \frac{p_x + \delta_X}{1 - p_x - \delta_X}\sum_{n = 1}^N&\frac{p_{y_n}}{p_{y_0}}P^T(Z = 1 \mid X = 1, Y = n) + \frac{p^E_{10}p_{y_0} - p^T_{11}(p_x + \delta_X)}{(1 - p_x - \delta_X)p_{y_0}} \leq 1
\end{align*}
Solving for the lower bound first, we have
\begin{align*}
    0 &\leq  \frac{p_x + \delta_X}{1 - p_x - \delta_X}\sum_{n = 1}^N\frac{p_{y_n}}{p_{y_0}}P^T(Z = 1 \mid X = 1, Y = n) + \frac{p^E_{10}p_{y_0} - p^T_{11}(p_x + \delta_X)}{(1 - p_x - \delta_X)p_{y_0}}\\
    &\implies \frac{p^T_{11}(p_x + \delta_X) - p^E_{10}p_{y_0}}{p_x + \delta_X} \leq \sum_{n = 1}^N P(Z = 1\mid X = 1, Y = n)
\end{align*}
Next, with the upper bound
\begin{align*}
    &\frac{p_x + \delta_X}{1 - p_x - \delta_X}\sum_{n = 1}^N\frac{p_{y_n}}{p_{y_0}}P^T(Z = 1 \mid X = 1, Y = n) + \frac{p^E_{10}p_{y_0} - p^T_{11}(p_x + \delta_X)}{(1 - p_x - \delta_X)p_{y_0}} \leq 1\\
    &\implies (p_x + \delta_X)\sum_{n = 1}^N p_{y_n}P^T(Z = 1 \mid X = 1, Y = n) + p^E_{10}p_{y_0} - p^T_{11}(p_x + \delta_X) \leq (1 - p_x - \delta_X)p_{y_0}\\
    &\implies \sum_{n = 1}^N p_{y_n}P^T(Z = 1 \mid X = 1, Y = n) \leq \frac{(1 - p_x - \delta_X)p_{y_0} + p^T_{11}(p_x + \delta_X) - p^E_{10}p_{y_0}}{p_x + \delta_X}\\
\end{align*}

Following a similar calculation for $P^T(Z = 1\mid X = 1, Y = 0)$, we have
\begin{align*}
    p^T_{11} - p_{y_0} \leq \sum_{n = 1}^Ny_n P^T(Z = 1 \mid X = 1, Y = n) \leq p^T_{11}
\end{align*}

Since all of the bounds need to hold simultaneously, we can re-express them using using maximum and minimum operators as
{\small
\begin{align*}
\max\begin{bmatrix}
   \frac{p^T_{11}(p_x + \delta_X) - p^E_{10}p_{y_0}}{p_x} \\
   p^T_{11} - p_{y_0}
\end{bmatrix} \leq \sum_{n = 1}^N y_n\mathbb{P}(Z = 1 \mid X = 1, Y = n) 
\leq \min\begin{bmatrix}
    \frac{(1 - p_x - \delta_X)p_{y_0} + p^T_{11}(p_x + \delta_X) - p^E_{10}p_{y_0}}{p_x + \delta_X}\\
    p^T_{11}
\end{bmatrix}
\end{align*}
}
Next, for $i \in \{1, \dots, N\}$, we have the following constraints on the basic variables $P(Z = 1\mid X = 0, Y = i)$
\begin{align*}
    0 &\leq P^T(Z = 1 \mid X = 0, Y = i) \leq 1\\
    0 &\leq \frac{p^E_{11}}{ 1- p_x - \delta_X} - \frac{p_x + \delta_X}{1 - p_x - \delta_X}P^T(Z = 1 \mid X = 1, Y = i) \leq 1\\
    \implies &\frac{p^E_{1i} - (1 - p_x - \delta_X)}{p_x + \delta_X} \leq P^T(Z = 1\mid X = 1, Y = i) \leq \frac{p^E_{1i}}{p_x + \delta_X} 
\end{align*}

And since the free parameters are probabilities themselves, they must be between $0$ and $1$ and hence the bounds for $P(Z = 1 \mid X = 1, Y = i)$ become
\begin{align*}
    \max\begin{bmatrix}
        0\\
        \frac{p^E_{1i} - (1 - p_x - \delta_X)}{p_x + \delta_X}
    \end{bmatrix}
        \leq P(Z = 1\mid X = 1, Y = i) \leq 
    \min\begin{bmatrix}
        1\\
        \frac{p^E_{1i}}{p_x + \delta_X} 
    \end{bmatrix}
\end{align*}
This concludes the proof for the lemma.

\section{Bounds For The Causal Marginal Problem}

Problem Setup: Random variables $X$, $Y$ and $Z$ are arranged in the following graph structure

\input{tikz_figures/causal_graph_structure}

From the joint distribution $P(Z, X, Y)$ obeying the causal graph structure above, we observe marginals $P(Z, X)$ and $P(Z, Y)$, and we are interested in combining these marginals to tighten our bounds on counterfactual quantities. Specifically, we can obtain bounds on counterfactuals just using $P(Z, X)$, however, we would like to tighten these bounds by adding in information from $P(Z, Y)$ as well. The Probabilities of Causation for $X \rightarrow Z$ will be used as the running example throughout, which is defined as follows:
\begin{equation*}
    PNS \equiv P(Z_{\mathbf{x}} = 1, Z_{\mathbf{x^\prime}}  = 0)
\end{equation*}
Where $\mathbf{x}$ and $\mathbf{x^\prime}$ denote the setting of $X$ to $1$ and $0$ respectively. \\
Now, bounds on the PNS under the above causal graph when we have access to the joint $P(Z, X, Y)$ are given in \cite{dawid2017probability} as 
\begin{align*}
    \Delta \leq PNS \leq \mathbb{P}(Z = 1 \mid X = 1) - \Gamma
\end{align*}

Where
\begin{equation*}
    \Delta = \sum_y \mathbb{P}(Y = y)\max \{0, \mathbb{P}(Z = 1 \mid X = 1, Y = y) - \mathbb{P}(Z = 1 \mid X = 0, Y = y)\} 
\end{equation*}

And $\Gamma$ is 
\begin{align*}
    \Gamma = \sum_y \mathbb{P}(Y = y)\max \{0, \mathbb{P}(Z = 1 \mid X = 1, Y = y) - \mathbb{P}(Z = 0 \mid X = 0, Y = y)\} 
\end{align*}
These bounds are a function of $P(Z, X, Y)$, and since we only have marginals $P(Z, X)$ and $P(Z, Y)$, we must modify these bounds before they can be used.
Specifically, the two marginals $P(Z, X)$ and $P(Z, Y)$ are consistent with many possible joint distributions over $Z$, $X$ and $Y$, and so we must use the above bounds in the most conservative way otherwise we risk giving erroneous answers. We demonstrate this in a toy example where there are two possible joint distributions over $Z$, $X$ and $Y$ that are compatible with the observed marginals. These joint are denoted as $P_1(Z, X, Y)$ and $P_2(Z, X, Y)$. By the properties of the max operator, the expression for $\Delta$ can be written as 
\begin{align*}
    \max\begin{bmatrix}0 \\
            P(Z = 1 \mid X = 1) - P(Z= 1 \mid X = 0) \\
        \mathbb{P}(Z = 1 \mid X = 1, Y = 0) - \mathbb{P}(Z = 1 \mid X = 0, Y = 0)
        \\\mathbb{P}(Z = 1 \mid X = 1, Y = 1) - \mathbb{P}(Z = 1 \mid X = 0, Y = 1)\end{bmatrix} \leq PNS
\end{align*}

The above bound can be computed for $P_1(Z, X, Y)$ and $P_2(Z, X, Y)$. Each of these distributions will imply the following lower bound on PNS:

% Suppose the following two tuples of $P(Z = 1 \mid X, Y)$ are both compatible with the observed marginals, and these two tuples are denoted as $<P_1(Z = 1\mid X = 0, Y = 0), P_1(Z = 1\mid X = 1, Y = 0), P_1(Z = 1\mid X = 0, Y = 1), P_1(Z = 1\mid X = 1, Y = 1) >$ and $<P_2(Z = 1\mid X = 0, Y = 0), P_2(Z = 1\mid X = 1, Y = 0), P_2(Z = 1\mid X = 0, Y = 1), P_2(Z = 1\mid X = 1, Y = 1)>$. 
\begin{align*}
    \max\begin{bmatrix}0 \\
            P(Z = 1 \mid X = 1) - P(Z= 1 \mid X = 0) \\
        P_1(Z = 1 \mid X = 1, Y = 0) - P_1(Z = 1 \mid X = 0, Y = 0)
        \\P_1(Z = 1 \mid X = 1, Y = 1) - P_1(Z = 1 \mid X = 0, Y = 1)\end{bmatrix} \leq PNS
\end{align*}

And similarly, 
\begin{align*}
    \max\begin{bmatrix}0 \\
            P(Z = 1 \mid X = 1) - P(Z= 1 \mid X = 0) \\
        P_2(Z = 1 \mid X = 1, Y = 0) - P_2(Z = 1 \mid X = 0, Y = 0)
        \\P_2(Z = 1 \mid X = 1, Y = 1) - P_2(Z = 1 \mid X = 0, Y = 1)\end{bmatrix} \leq PNS
\end{align*}

Now the subtlety lies in that we don't know whether the true underlying distribution that produced the marginals is $P_1$ or $P_2$, i.e. if we choose the tighter bound on PNS that arises from using $P_2$ but the true distribution that generated the marginals is $P_1$, our lower bound is more restrictive and consequently incorrect. 

To remedy this, we choose the lower bound on PNS arising from $P_1$ and $P_2$ that is smaller, since this is guaranteed to be correct, i.e. if $P_2$ produces a greater lower bound that $P_1$, the bound obtained from $P_1$ will be correct all the time - when either $P_1$ or $P_2$ is the true distribution that generated the data, whereas the bound produced by $P_2$ will only be correct when $P_2$ is the true distribution that generated the observed marginals.\\\\
This line of reasoning can be formally expressed as 
\begin{align*}
     \min_{P_i}\max\begin{bmatrix}
             0 \\
             P(Z = 1 \mid X = 1) - P(Z= 1 \mid X = 0) \\
             \mathbb{P}(Y = 0)\{ P_i(Z = 1 \mid X = 1, Y = 0) - P_i(Z = 1 \mid X = 0, Y = 0)\}\\
             \mathbb{P}(Y = 1)\{P_i(Z = 1 \mid X = 1, Y = 1) - P_i(Z = 1 \mid X = 0, Y = 1)\}
         \end{bmatrix} \leq PNS
\end{align*}

And similarly for the upper bound, since it is expressed in the form of $P(Z = 1\mid X = 1) - \Gamma$, we focus on $\Gamma$, which can be equivalently expressed as
\begin{align*}
      PNS \leq \min_{P_i}\max\begin{bmatrix}
             0 \\
             \sum_y \mathbb{P}(Y = y)\{\mathbb{P}(Z = 1 \mid X = 1, Y = y) - \mathbb{P}(Z = 0 \mid X = 0, Y = y)\} \\
             P(Y = 0)\{ P_i(Z = 1 \mid X = 1, Y = 0) - P_i(Z = 0 \mid X = 0, Y = 0)\}\\
             P(Y = 1)\{P_i(Z = 1 \mid X = 1, Y = 1) - P_i(Z = 0 \mid X = 0, Y = 1)\}
         \end{bmatrix}
\end{align*}

Now, to compute the minimum values in the above matrices, we need to enumerate the set of solutions for $P(Z, X, Y)$ which are compatible with the observed marginals, which is done in the next section. 

\section{Enumerating The Set Of Joint Distributions Compatible With Observed Marginals}

For the graph shaped in \ref{fig:causal-graph}, we can enumerate the following equations for the $P(Z, X, Y)$
\begin{align*}
    \mathbb{P}(Z = 1 \mid X = 1) &= \mathbb{P}(Z = 1 \mid X = 1, Y = 1)\mathbb{P}(Y = 1) + \mathbb{P}(Z = 1 \mid X = 1, Y = 0)\mathbb{P}(Y = 0)\\
    \mathbb{P}(Z = 1 \mid X = 0) &= \mathbb{P}(Z = 1 \mid X = 0, Y = 1)\mathbb{P}(Y = 1) + \mathbb{P}(Z = 1 \mid X = 0, Y = 0)\mathbb{P}(Y = 0)\\
    \mathbb{P}(Z = 1 \mid Y = 1) &= \mathbb{P}(Z = 1 \mid X = 0, Y = 1)\mathbb{P}(X = 0) + \mathbb{P}(Z = 1 \mid X = 1, Y = 1)\mathbb{P}(X = 1)\\
    \mathbb{P}(Z = 1 \mid Y = 0) &= \mathbb{P}(Z = 1 \mid X = 0, Y = 0)\mathbb{P}(X = 0) + \mathbb{P}(Z = 1 \mid X = 1, Y = 0)\mathbb{P}(X = 1)
\end{align*}

This represents a system of equations with $4$ unknowns and $3$ linearly independent constraints, and for notational ease we introduce the following notation. $OR(X) = \frac{P(X = 1)}{P(X = 0)}$ and same for $OR(Y)$. $P(X = 1) = x$ and $P(Y = 1) = y$, and $P(Z = 1\mid X = 1) = p_{11}$, $P(Z = 1\mid X = 0) = p_{10}$, $P(Z = 1\mid Y = 1) = p^\prime_{11}$, $P(Z = 1\mid Y = 0) = p^\prime_{10}$.
\begin{align*}
\begin{bmatrix}
    1 & 0 & 0 & -OR(X)OR(Y) & \frac{p_{10}(1 - x) - p^\prime_{11}y}{(1 - x)(1 - y)}\\
    0 & 1 & 0 & OR(Y) & \frac{p_{11}}{1 - y}\\
    0 & 0 & 1 & OR(X) & \frac{p^\prime_{11}}{ 1- x}\\
    0 & 0 & 0 & 0 & 0
\end{bmatrix}    
\end{align*}

And this can equivalently be represented in equation form using the free parameter $P(Z = 1 \mid X = 1, Y = 1)$ 
{\small
\begin{align}
    &\mathbb{P}(Z = 1 \mid X = 0, Y = 0) - OR(X)OR(Y)\mathbb{P}(Z = 1 \mid X = 1, Y = 1) =  \frac{p_{10}(1 - x) - p^\prime_{11}y}{(1 - x)(1 - y)}
\end{align}\label{p_100}
\begin{equation}
    \mathbb{P}(Z = 1 \mid X = 1, Y = 0) + OR(Y)\mathbb{P}(Z = 1 \mid X = 1, Y = 1) = \frac{p_{11}}{1 - y}
\end{equation}
\begin{equation}
    \mathbb{P}(Z = 1 \mid X = 0, Y = 1) + OR(X)\mathbb{P}(Z = 1 \mid X = 1, Y = 1) = \frac{p^\prime_{11}}{ 1- x}
\end{equation}    
}
Now we must find bounds on $\mathbb{P}(Z = 1 \mid X = 1, Y = 1)$ such that every term in this system of equations is a valid probability. This is presented in the subssections below.

\subsection{Bounds From $\mathbb{P}(Z = 1\mid X = 0, Y = 1)$}
The following requirement can be used to compute bounds 
\[
     0 \leq \mathbb{P}(Z = 1 \mid X = 0, Y = 1) \leq 1
\]

Expressing this in terms of $\mathbb{P}(Z = 1\mid X = 1, Y = 1)$ 
\[
     0 \leq \frac{p^\prime_{11}}{ 1 - x} - OR(X)\mathbb{P}(Z = 1 \mid X = 1, Y = 1) \leq 1
\]
 \begin{itemize}
     \item Starting with the lower bound: 
     \begin{align*}
     0 \leq \frac{p^\prime_{11}}{ 1 - x} - OR(X)\mathbb{P}(Z = 1 \mid X = 1, Y = 1)\\
    \implies x\mathbb{P}(Z = 1 \mid X = 1, Y = 1) \leq p^\prime_{11}\\
     \implies \mathbb{P}(Z = 1 \mid X = 1, Y = 1) \leq \frac{p^\prime_{11}}{x}\\
    \end{align*}
    This implies the following bound
    \begin{equation}
        \mathbb{P}(Z = 1 \mid X = 1, Y = 1) \leq \frac{p^\prime_{11}}{x}
    \end{equation}\label{lower-bound-p_111-1}
    \item Repeating a similar calculation for the upper bound
    \begin{align*}
     \frac{p^\prime_{11}}{ 1 - x} - OR(X)\mathbb{P}(Z = 1 \mid X = 1, Y = 1) \leq 1\\
     \implies \frac{p^\prime_{11} - (1 - x)}{x} \leq \mathbb{P}(Z = 1 \mid X = 1, Y = 1)
    \end{align*}    
    This implies the following upper bound
    \begin{equation}
        \frac{p^\prime_{11} - (1 - x)}{x} \leq \mathbb{P}(Z = 1 \mid X = 1, Y = 1)
    \end{equation}\label{upper-bound-p_111-1}
 \end{itemize}

\subsection{Bounds From $\mathbb{P}(Z = 1\mid X = 1, Y = 0)$}

Repeating the above process to obtain bounds on $P(Z = 1 \mid X = 1, Y = 0)$
\begin{equation}
    \frac{p_{11} - (1 - y)}{y} \leq \mathbb{P}(Z = 1 \mid X = 1, Y = 1)
\end{equation}\label{lower-bound-p_111-2}

And the upper bound
\begin{equation}
     \mathbb{P}(Z = 1 \mid X = 1, Y = 1) \leq \frac{p_{11}}{y}
\end{equation}\label{upper-bound-p_111-2}
    
\subsection{Bounds Obtained From Equation \ref{p_100}}

From Equation \ref{p_100}

\begin{align*}
     0 \leq \frac{p_{10}(1 - x) - p^\prime_{11}y}{(1 - x)(1 - y)} + OR(X)OR(Y)\mathbb{P}(Z = 1 \mid X = 1, Y = 1) \leq 1
\end{align*}
\begin{itemize}
    \item Starting with the lower bound, we get
    \begin{align*}
     &0 \leq \frac{p_{10}(1 - x) - p^\prime_{11}y}{(1 - x)(1 - y)} + OR(X)OR(Y)\mathbb{P}(Z = 1 \mid X = 1, Y = 1) \\
&\implies 0 \leq p_{10}(1 - x) - p^\prime_{11}y + xy\mathbb{P}(Z = 1 \mid X = 1, Y = 1)\\
     &\implies \frac{p^\prime_{11}y - p_{10}(1 - x)}{xy} \leq  \mathbb{P}(Z = 1 \mid X = 1, Y = 1)
\end{align*}

And so, the bound implied is
\begin{equation}
    \frac{p^\prime_{11}y - p_{10}(1 - x)}{xy} \leq  \mathbb{P}(Z = 1 \mid X = 1, Y = 1)
\end{equation}\label{lower-bound-p_111-3}

\item Repeating for the upper bound:
 \begin{align*}
     &\frac{p_{10}(1 - x) - p^\prime_{11}y}{(1 - x)(1 - y)} + OR(X)OR(Y)\mathbb{P}(Z = 1 \mid X = 1, Y = 1) \leq 1\\
     &\implies \mathbb{P}(Z = 1 \mid X = 1, Y = 1) \leq \frac{(1 - x)(1 - y) - p_{10}(1 - x) + p^\prime_{11}y}{xy}
 \end{align*}

 So, the bound implied is
 \begin{equation}
     \mathbb{P}(Z = 1 \mid X = 1, Y = 1) \leq \frac{(1 - x)(1 - y) - p_{10}(1 - x) + p^\prime_{11}y}{xy}
 \end{equation}\label{lower-bound-p_111-4}
\end{itemize}

So, the final bounds on $P(Z = 1 \mid X = 1, Y = 1)$ are
\begin{align}\label{p_111_bounds}
         \max\begin{bmatrix}
                0 \\
                \frac{p^\prime_{11} - (1 - x)}{x} \\
                \frac{p_{11} - (1 - y)}{y}\\   
                \frac{p^\prime_{11}y - p_{10}(1 - x)}{xy}
            \end{bmatrix}
              \leq  \mathbb{P}(Z = 1 \mid X = 1, Y = 1)
             \leq \min\begin{bmatrix}
                        1 \\
                        \frac{(1 - x)(1 - y) - p_{10}(1 - x) + p^\prime_{11}y}{xy}\\
                        \frac{p_{11}}{y}\\
                        \frac{p^\prime_{11}}{x}
                    \end{bmatrix}
\end{align}

Since there is no implicit ordering on which is the min amongst the options, as well as which one is the max amongst all the options, this reduces to a problem of checking all at the relevant extreme points.

\subsection{Implications Of Upper And Lower Bounds}\label{implications_bounds_p111}

Each of the choice of the lower bounds being the max or the min has implications on the system constraints, which we now enumerate. 

\subsubsection{The Lower Bound Is $0$}

If $0$ is the lower bound, it means that it must be greater than the rest of the terms, i.e. 
\begin{enumerate}
    \item \begin{equation}
    0 > \frac{p^\prime_{11} - (1 - x)}{x} \implies p^\prime_{11} < 1 - x 
    \end{equation}\label{lb-1-implication-1}
\item \begin{equation}
0 > \frac{p_{11} - (1 - y)}{y} \implies p_{11} < 1 - y
\end{equation}\label{lb-1-implication-2}
\item \begin{align}
0 > \frac{p^\prime_{11}y - p_{10}(1 - x)}{xy}
\implies p_{10}(1 - x) > p^\prime_{11}y \label{lb-1-implication-3}
\end{align}
\end{enumerate}


\subsubsection{The Lower Bound Is $\frac{p^\prime_{11} - (1 - x)}{x}$}

This implies the following conditions
\begin{enumerate}
    \item \begin{equation}
    \frac{p^\prime_{11} - (1 - x)}{x} > 0 \implies p^\prime_{11} > 1 - x
    \end{equation}\label{lb-2-implication-1}
    \item 
    \begin{align}
        \frac{p^\prime_{11} - (1 - x)}{x} > \frac{p_{11} - (1 - y)}{y}
        \implies p^\prime_{01}y < p_{01}x\label{lb-2-implication-2}
    \end{align}
\item 
    \begin{align}
    \frac{p^\prime_{11} - (1 - x)}{x} > \frac{p^\prime_{11}y - p_{10}(1 - x)}{xy} 
    \implies  p_{10} > y \label{lb-2-implication-3}
    \end{align}
\end{enumerate}


\subsubsection{The Lower Bound is $\frac{p_{11} - (1 - y)}{y}$}

This implies the following conditions
\begin{enumerate}
    \item 
    \begin{equation}
        \frac{p_{11} - (1 - y)}{y} > 0 \implies p_{11} > (1 - y)
    \end{equation}\label{lb-3-implication-1}
    \item 
    \begin{align}
        \frac{p_{11} - (1 - y)}{y} > \frac{p^\prime_{11} - (1 - x)}{x}
        \implies p_{01}x < p^\prime_{01}y\label{lb-3-implication-2}
    \end{align}
    \item 
    \begin{align}
        &\frac{p_{11} - (1 - y)}{y} > \frac{p^\prime_{11}y - p_{10}(1 - x)}{xy}
        \implies p^\prime_{10} > x\label{lb-3-implication-3}
    \end{align}
\end{enumerate}


\subsubsection{When The Lower Bound Is $\frac{p^\prime_{11}y - p_{10}(1 - x)}{xy}$}

The constraints here just amount to inverting the corresponding constrains above, so we get
\begin{equation}
%P(Z = 1\mid Y = 1)P(Y = 1) \geq P(Z = 1\mid X = 0)P(X = 0)   
p^\prime_{11}y > p_{10}(1 - x)
\end{equation}\label{lb-4-implication-1}

\begin{equation}
y > p_{10}\\
\end{equation}\label{lb-4-implication-2}

\begin{equation}
x > p^\prime_{10}
\end{equation}\label{lb-4-implication-3}

\subsection{When The Upper Bound is $1$}

\begin{enumerate}
\item \begin{align}
    &1 < \frac{(1 - x)(1 - y) - p_{10}(1 - x) + p^\prime_{11}y}{xy}\notag \\
    \intertext{It is worth noting that $xy - (1 - x)(1 - y) = y - (1 - x)$}
    &\implies p^\prime_{01}y < p_{00}(1 - x) \label{ub-1-implication-1}
\end{align}
\item \begin{equation}
    1 < \frac{p_{11}}{y} \implies y < p_{11}
\end{equation}\label{ub-1-implication-2}
\item \begin{equation}
            1 < \frac{p^\prime_{11}}{x} \implies x < p^\prime_{11}
        \end{equation}\label{ub-1-implication-3}
\end{enumerate}

\subsection{The Upper Bound is $\frac{p_{11}}{y}$}

\begin{enumerate}
    \item \begin{equation}
    \frac{p_{11}}{y} < 1 \implies p_{11} < y
    \end{equation}\label{ub-2-implication-1}
    \item 
    \begin{align}
        &\frac{p_{11}}{y} < \frac{(1 - x)(1 - y) - p_{10}(1 - x) + p^\prime_{11}y}{xy}
        \implies p^\prime_{10} < (1 - x)
    \end{align}\label{ub-2-implication-2}        
    \item \begin{equation}
        \frac{p_{11}}{y} < \frac{p^\prime_{11}}{x} \implies p_{11}x < p^\prime_{11}y
    \end{equation}\label{ub-2-implication-3}        
\end{enumerate}

\subsection{The Upper Bound Is $\frac{p^\prime_{11}}{x}$}
\begin{enumerate}
    \item 
    \begin{equation}
    \frac{p^\prime_{11}}{x} < 1 \implies p^\prime_{11} < x
    \end{equation}\label{ub-3-implication-1}        

    \item 
    \begin{equation}
    \frac{p^\prime_{11}}{x} < \frac{p_{11}}{y} \implies p^\prime_{11}y < p_{11}x
    \end{equation}\label{ub-3-implication-2}
    \item \begin{align}
        &\frac{p^\prime_{11}}{x} < \frac{(1 - x)(1 - y) - p_{10}(1 - x) + p^\prime_{11}y}{xy}
        \implies p_{10} < 1 - y\label{ub-3-implication-3}
    \end{align}
\end{enumerate}

\subsection{When The Upper Bound is $\frac{(1 - x)(1 - y) - p_{10}(1 - x) + p^\prime_{11}y}{xy}$}

All the relevant constraints here can be obtained by flipping the inequlaities before, and are enumerated as
\begin{align}
    p_{00}(1 - x) < p^\prime_{01}y\label{ub-4-implication-1}
\end{align}

\begin{align}
    p^\prime_{10} > (1 - x)\label{ub-4-implication-2}
\end{align}

\begin{align}
p_{10} > 1 - y \label{ub-4-implication-2}
\end{align}

\section{Deriving Bounds On PNS}

Having enumerated the space of solutions for $P(Z, X, Y)$, we can plug them into our modification of Phil Dawid's bounds in order to obtain tighter bounds on PNS. Phil Dawid's bounds are given as
\begin{align*}
    \frac{\Delta}{\mathbb{P}(Z = 1 \mid X = 1)} \leq PC \leq 1 - \frac{\Gamma}{\mathbb{P}(Z = 1 \mid X = 1)}
\end{align*}

Where
\begin{equation*}
    \Delta = \sum_y \mathbb{P}(Y = y)\max \{0, \mathbb{P}(Z = 1 \mid X = 1, Y = y) - \mathbb{P}(Z = 1 \mid X = 0, Y = y)\} 
\end{equation*}

And $\Gamma$ is 
\begin{align*}
    \Gamma = \sum_y \mathbb{P}(Y = y)\max \{0, \mathbb{P}(Z = 1 \mid X = 1, Y = y) - \mathbb{P}(Z = 0 \mid X = 0, Y = y)\} 
\end{align*}

For binary $Y$ these can be written as
\begin{align*}
    \Delta &= \mathbb{P}(Y = 0)\max \{0, \mathbb{P}(Z = 1 \mid X = 1, Y = 0) - \mathbb{P}(Z = 1 \mid X = 0, Y = 0)\}\\
    &+ \mathbb{P}(Y = 1)\max \{0, \mathbb{P}(Z = 1 \mid X = 1, Y = 1) - \mathbb{P}(Z = 1 \mid X = 0, Y = 1)\}\\
    \Gamma &= \mathbb{P}(Y = 0)\max \{0, \mathbb{P}(Z = 1 \mid X = 1, Y = 0) - \mathbb{P}(Z = 0 \mid X = 0, Y = 0)\}\\
    &+ \mathbb{P}(Y = 1)\max \{0, \mathbb{P}(Z = 1 \mid X = 1, Y = 1) - \mathbb{P}(Z = 0 \mid X = 0, Y = 1)\} 
\end{align*}


Now as seen in \cite{gresele2022causal}, we must recover the result that the lower bound can't be tightened (since the upper bound of $\lambda_X$ can't be tightened). So we start with computing $\Delta$, aka the lower bound. To solve this, we first re-expressing all of the above bounds in terms of the free parameter $P(Z = 1 \mid X = 1, Y = 1)$. 

\subsection{Re-expressing $\Delta$ in terms of $P(Z = 1 \mid X = 1, Y = 1)$}

Re-expressing all the terms in $\Delta$ in terms of $\mathbb{P}(Z = 1 \mid X = 1, Y = 1)$, using the shortened notation defined previously for ease.

\begin{enumerate}
    \item $P(Y = 0)\{\mathbf{\mathbb{P}(Z = 1 \mid X = 1, Y = 0) - \mathbb{P}(Z = 1 \mid X = 0, Y = 0)}\}$
    \begin{align*}
    &\mathbf{\mathbb{P}(Z = 1 \mid X = 1, Y = 0) - \mathbb{P}(Z = 1 \mid X = 0, Y = 0)} = \\
    &\frac{p_{11} - p^\prime_{10}(1 - y)}{(1 - x)(1 - y)} - \frac{y\mathbb{P}(Z = 1\mid X = 1, Y = 1)}{(1 - x)(1 - y)}  
\end{align*}
So, this is expressed as 
{\scriptsize
\begin{equation}
    \frac{p_{11} - p^\prime_{10}(1 - y)}{(1 - x)} - \frac{y\mathbb{P}(Z = 1\mid X = 1, Y = 1)}{(1 - x)}  
\end{equation}\label{delta-term-1}}

\item $P(Y = 1)\{\mathbb{P}(Z = 1 \mid X = 1, Y = 1) - \mathbb{P}(Z = 1 \mid X = 0, Y = 1)\}$
    \begin{align*}
        &\mathbb{P}(Z = 1 \mid X = 1, Y = 1) - \mathbb{P}(Z = 1 \mid X = 0, Y = 1) = 
        \frac{\mathbb{P}(Z = 1 \mid X = 1, Y = 1) - p^\prime_{11}}{1 - x}
    \end{align*}
    So, this is written as 
    \begin{equation}
        \frac{\mathbb{P}(Z = 1 \mid X = 1, Y = 1)y - p^\prime_{11}y}{1 - x}
    \end{equation}\label{delta-term-2}
\end{enumerate}

\subsection{Re-expressing $\Gamma$ in terms of $P(Z = 1\mid X = 1, Y = 1)$}

A similar approach to the one used above is utilized, starting with expressing everything in terms of $P(Z = 1\mid X = 1, Y = 1)$, done below. For notational convenience, we define the following
\[
\Phi_X = p_{11} + p_{10} - 1
\]

\begin{enumerate}
    \item $P(Y = 0)\{\mathbb{P}(Z = 1 \mid X = 1, Y = 0) - \mathbb{P}(Z = 0 \mid X = 0, Y = 0)\}$
    \begin{align*}
    \mathbb{P}(Z = 1 \mid X = 1, Y = 0) &= \frac{p_{11}}{1 - y} - OR(Y)\mathbb{P}(Z = 1 \mid X = 1, Y = 1)\\
    \mathbb{P}(Z = 0 \mid X = 0, Y = 0) &= 1 - \{\frac{p_{10}(1 - x) - p^\prime_{11}y}{(1 - x)(1 - y)} + \\ &OR(X)OR(Y)\mathbb{P}(Z = 1 \mid X = 1, Y = 1)\}
    \end{align*}
    Subtracting the two, we get
{\small
\begin{align*}
    & OR(Y)P(Z = 1\mid X = 1, Y = 1)(OR(X) - 1) + \frac{p_{11}}{1 - y} + \frac{p_{10}(1 - x) - p^\prime_{11}y}{(1 - x)(1 - y)} - 1\\
    &= OR(Y)P(Z = 1\mid X = 1, Y = 1)(OR(X) - 1) + \frac{p_{11}(1 - x) + p_{10}(1 - x) - p^\prime_{11}y - (1 - x)(1 - y)}{(1 - x)(1 - y)} \\
    &= OR(Y)P(Z = 1\mid X = 1, Y = 1)(OR(X) - 1) + \frac{(1 - x)\Phi_X + (1 - x)y - p^\prime_{11}y }{(1 - x)(1 - y)} \\
    &= OR(Y)P(Z = 1\mid X = 1, Y = 1)(OR(X) - 1) + \frac{\Phi_X + y}{1 - y} - \frac{p^\prime_{11}y}{(1 - x)(1 - y)}\\
\end{align*}
}

Now, this difference is multiplied by $1 - y$, so it is finally written as
\begin{align}
    &= yP(Z = 1\mid X = 1, Y = 1)(OR(X) - 1) + \Phi_X + y - \frac{p^\prime_{11}y}{1 - x}
\end{align}\label{eq:gamma-term-1}

\item $P(Y = 1)\{\mathbb{P}(Z = 1 \mid X = 1, Y = 1) - \mathbb{P}(Z = 0 \mid X = 0, Y = 1)\}$
{\small
\begin{align*}
    \mathbb{P}(Z = 0 \mid X = 0, Y = 1) &= 1 - \Bigg(\frac{p^\prime_{11}}{1 - x} - OR(X)\mathbb{P}(Z = 1 \mid X = 1, Y = 1)\Bigg)\\
    &= 1 - \frac{p^\prime_{11}}{1 - x} + OR(X)\mathbb{P}(Z = 1 \mid X = 1, Y = 1)
\end{align*}
}

And so, 
{\small
\begin{align*}
    &\mathbb{P}(Z = 1 \mid X = 1, Y = 1) - \mathbb{P}(Z = 0 \mid X = 0, Y = 1)\\
    &= P(Z = 1 \mid X = 1, Y = 1) - 1 + \frac{p^\prime_{11}}{1 - x} - OR(X)\mathbb{P}(Z = 1 \mid X = 1, Y = 1)\\
    &= P(Z = 1 \mid X = 1, Y = 1)(1 - OR(X)) + \frac{p^\prime_{11} - (1 - x)}{1 - x}\\
    % &= \frac{P(Z = 1 \mid X = 1, Y = 1)P(X = 0) - P(X = 1)\mathbb{P}(Z = 1 \mid X = 1, Y = 1)}{P(X = 0)} - 1 + \frac{\mathbb{P}(Z = 1 \mid Y = 1)}{\mathbb{P}(X = 0)} \\
    % &= \frac{-P(Z = 1 \mid X = 1, Y = 1)[P(X = 1) - P(X = 0)]}{P(X = 0)} - 1 + \frac{\mathbb{P}(Z = 1 \mid Y = 1)}{\mathbb{P}(X = 0)} \\
\end{align*}
}
Multiplying by $y$, this will be written as
\begin{equation}
    P(Z = 1 \mid X = 1, Y = 1)(1 - OR(X))y + y\frac{p^\prime_{11} - (1 - x)}{1 - x}\\
\end{equation}\label{eq:gamma-term-2}
\end{enumerate}


\subsection{Sum of the above two terms}

This is a sanity check, since we know these must add up to $p_{11} + p_{10} - 1$.
\begin{align*}
    &yP(Z = 1\mid X = 1, Y = 1)(OR(X) - 1) + \Phi_X + y - \frac{p^\prime_{11}y}{1 - x} \\
    &+  P(Z = 1 \mid X = 1, Y = 1)(1 - OR(X))y + y\frac{p^\prime_{11} - (1 - x)}{1 - x}\\
    &= \Phi_X + y - \frac{p^\prime_{11}y}{1 - x} + y\frac{p^\prime_{11} - (1 - x)}{1 - x}\\
    &= \Phi_X
\end{align*}


So, sanity check passed. 

\section{Final Proof: Causal Marginal Problem Lower Bound}

Given $P(Z, X)$ and $P(Z, Y)$, and indexing the set of joint distributions $P(Z, X, Y)$ compatible with these constraints by $P^{(i)}$, the lower bound for the causal marginal problem is obtained by solving
\begin{align*}
     \min_{P_i}\max\begin{bmatrix}
             0 \\
             P(Z = 1 \mid X = 1) - P(Z= 1 \mid X = 0) \\
             \mathbb{P}(Y = 0)\{ P_i(Z = 1 \mid X = 1, Y = 0) - P_i(Z = 1 \mid X = 0, Y = 0)\}\\
             \mathbb{P}(Y = 1)\{P_i(Z = 1 \mid X = 1, Y = 1) - P_i(Z = 1 \mid X = 0, Y = 1)\}
         \end{bmatrix} \leq PNS
\end{align*}

Now, by solving the system of linear equations from the implied consistency constraints, we see there is a single free parameter $P(Z = 1 \mid X = 1, Y = 1)$, and so the above can be re-expressed as 
\begin{align*}
     \min_{P(Z = 1 \mid X = 1, Y = 1)}\max\begin{bmatrix}
             0 \\
             P(Z = 1 \mid X = 1) - P(Z= 1 \mid X = 0) \\
             \frac{\mathbb{P}(Z = 1 \mid X = 1) - \mathbb{P}(Z = 1\mid Y = 0)\mathbb{P}(Y = 0)}{\mathbb{P}(X = 0)} - \frac{\mathbb{P}(Y = 1)\mathbb{P}(Z = 1\mid X = 1, Y = 1)}{\mathbb{P}(X = 0)}\\
             \frac{\mathbb{P}(Z = 1 \mid X = 1, Y = 1)\mathbb{P}(Y = 1) - \mathbb{P}(Z = 1 \mid Y = 1)\mathbb{P}(Y = 1)}{\mathbb{P}(X = 0)}
         \end{bmatrix} 
\end{align*}

Now, to make proofs easier, we re-write the above as
{\small
\begin{align*}
     \min_{P(Z = 1 \mid X = 1, Y = 1)}\max\begin{bmatrix}
             0 \\
             P(Z = 1 \mid X = 1) - P(Z= 1 \mid X = 0) \\
             \mathbb{P}(Z = 1 \mid X = 1) - \mathbb{P}(Z = 1 \mid X = 0) + \frac{P(Z = 1 \mid Y = 1)P(Y = 1)}{P(X = 0)} - \frac{\mathbb{P}(Y = 1)\mathbb{P}(Z = 1\mid X = 1, Y = 1)}{\mathbb{P}(X = 0)}\\
             \frac{\mathbb{P}(Z = 1 \mid X = 1, Y = 1)\mathbb{P}(Y = 1) - \mathbb{P}(Z = 1 \mid Y = 1)\mathbb{P}(Y = 1)}{\mathbb{P}(X = 0)}
         \end{bmatrix} 
\end{align*}
}
And the lower bound on $P(Z = 1 \mid X = 1, Y = 1)$ will be
\begin{align*}
         \max\begin{bmatrix}
                0 \\
                \frac{\mathbb{P}(Z = 1 \mid Y = 1) - \mathbb{P}(X = 0)}{\mathbb{P}(X = 1)} \\
                \frac{\mathbb{P}(Z = 1 \mid X = 1) - \mathbb{P}(Y = 0)}{\mathbb{P}(Y = 1)}\\   
                \frac{\mathbb{P}(Z = 1 \mid Y = 1)\mathbb{P}(Y = 1) - \mathbb{P}(Z = 1 \mid X = 0)\mathbb{P}(X = 0)}{\mathbb{P}(X = 1) \mathbb{P}(Y = 1) }
            \end{bmatrix}
              \leq  \mathbb{P}(Z = 1 \mid X = 1, Y = 1)
\end{align*}

And the upper bound on $P(Z = 1 \mid X = 1, Y = 1)$ will be
\begin{align*}
    \mathbb{P}(Z = 1 \mid X = 1, Y = 1)
             \leq \min\begin{bmatrix}
                        1 \\
                        \frac{\mathbb{P}(X = 0)\mathbb{P}(Y = 0) - \mathbb{P}(Z = 1 \mid X = 0)\mathbb{P}(X = 0) + \mathbb{P}(Z = 1 \mid Y = 1)\mathbb{P}(Y = 1)}{\mathbb{P}(X = 1)\mathbb{P}(Y = 1)}\\
                        \frac{\mathbb{P}(Z = 1 \mid X = 1)}{\mathbb{P}(Y = 1)}\\
                        \frac{\mathbb{P}(Z = 1 \mid Y = 1)}{\mathbb{P}(X = 1)}
                    \end{bmatrix}
\end{align*}

Now, the choice between $0$ and $P(Z = 1 \mid X = 1) - P(Z = 1\mid X = 0)$ is a priori decided based on $P(Z, X)$. So, the max operator must be analyzed in each of these cases, presented in the subsections below. For convenience, we use the following notation for each of the terms. $p^\prime_{11} = P(Z = 1 \mid Y = 1)$ and $p_{11} = P(Z = 1 \mid X = 1)$ and $x = P(X = 1)$ and same for $y$, with the relevant extrapolations needed for the rest of the terms.

\textbf{Claim}: $0 \geq P(Z = 1 \mid X = 1) - P(Z = 1\mid X = 0)$ doesn't restrict the range of $P(Z = 1 \mid X = 1, Y = 1)$ as it doesn't contradict any of the implied inequalities in the choice of bounds for $P(Z = 1 \mid X = 1, Y = 1)$. 

\subsection{Case I: $0 > p_{11} - p_{10}$}

We start by examining the behavior of the max operator as the value of $P(Z = 1 \mid X = 1, Y = 1)$ varies. First we notice that line 3 of the max operator is a decreasing function of $P(Z = 1\mid X = 1, Y = 1)$ and line 4 is an increasing function, which can be seen below.
\begin{align*}
     \max\begin{bmatrix}
             0 \\
             p_{11} - p_{10} \\
             p_{11} - p_{10} + \frac{p^\prime_{11}y}{1 - x} - \frac{y\mathbb{P}(Z = 1\mid X = 1, Y = 1)}{1 - x}\\
             \frac{\mathbb{P}(Z = 1 \mid X = 1, Y = 1)y - p^\prime_{11}y}{1 - x}
         \end{bmatrix} 
\end{align*}

This is analyzed piece-wise, to see where line 3 is the output, and where line 4 is the output. First we examine where line 3 would be greater than $0$.
\begin{align*}
   p_{11} - p_{10} + \frac{p^\prime_{11}y}{1 - x} - \frac{y\mathbb{P}(Z = 1\mid X = 1, Y = 1)}{1 - x} \geq 0 \\
   \implies \frac{\Big\{p_{11} - p_{10}\Big\}(1 - x)}{y} + p^\prime_{11}  \geq \mathbb{P}(Z = 1\mid X = 1, Y = 1)
\end{align*}

Now, repeating for line 4:
\begin{align*}
    \frac{\mathbb{P}(Z = 1 \mid X = 1, Y = 1)y - p^\prime_{11}y}{1 - x} \geq 0\\
    \implies P(Z = 1 \mid X = 1, Y = 1) \geq p^\prime_{11}
\end{align*}

Since $p_{11} - p_{10} \leq 0 \implies \frac{\Big\{p_{11} - p_{10}\Big\}(1 - x)}{y} + p^\prime_{11} \leq p^\prime_{11}$. So we expect the graph to look like
\begin{figure}
    \centering
    \includegraphics[width=\textwidth]{free_parameter_lower_bounds_when_p11minusp10lessthan0.pdf}%{lower_bound_graph_case_i.jpeg}
    \caption{Identifying the lower bound of PNS (y-axis) for different values of the free parameter $P(Z=1|X=1,Y=1)$ (x-axis). Whenever the lower bound of the free parameter is less than $a$ or larger than $b$, then the resulting lower bound for the PNS results into falsification +++.}
    \label{fig:enter-label}
\end{figure}


The dashed line is meant to convey that the graph may not may not have this slope, for the following reason.  If $\frac{\Big\{p_{11} - p_{10}\Big\}(1 - x)}{y} + p^\prime_{11} \geq 0$, then we will have the dashed line, and if not, we will have the flat line. 

As long as the range of $P(Z = 1\mid X = 1, Y = 1)$ allows the Y-axis to include $0$, we will not obtain any falsification. This can happen in the following scenarios:
\begin{enumerate}
    \item $\frac{\Big\{p_{11} - p_{10}\Big\}(1 - x)}{y} + p^\prime_{11} \geq 0$, and the upper bound is always less than $\frac{\Big\{p_{11} - p_{10}\Big\}(1 - x)}{y} + p^\prime_{11}$ (since otherwise the upper bound can be as low as $0$ and still include the $0$ point in the max)
    \item The lower bound for $P(Z = 1 \mid X = 1, Y = 1)$ is always $> p^\prime_{11}$ \atalanti{isn't it that max of two things?}
\end{enumerate}

Now, we check each of these in the following subsections.

\subsubsection{Case 1}
Assume $\frac{\Big\{p_{11} - p_{10}\Big\}(1 - x)}{y} + p^\prime_{11} \geq 0$, and we check whether any of the upper bounds are less than this value. 

When the upper bound is $1$, it is impossible for $1$ to be less than this value since it would require $p^\prime_{11} > 1$.

Next, we check the upper bound when it equals $\frac{p_{11}}{y}$, and use a proof by contradiction. 

\textbf{Proof}: Assume 
\begin{align*}
    \frac{\Big\{p_{11} - p_{10}\Big\}(1 - x)}{y} + p^\prime_{11} > \frac{p_{11}}{y}\\
    \implies p_{11}(1 - x) - p_{10}(1 - x) + p^\prime_{11}y > p_{11}\\
    \implies -p_{11}x - p_{10}(1 - x) + p^\prime_{11}y > 0\\
    \intertext{From the property $p^\prime_{11}y - p_{11}x - p_{10}(1 - x) = -p^\prime_{10}(1 - y)$}
    \implies -p^\prime_{10}(1 - y) > 0\\
    \implies p^\prime_{10}(1 - y) < 0
\end{align*}

This cannot happen from the properties of probability since $0 \leq p^\prime_{10} \leq 1$ and $0 \leq y \leq 1$.

% And this is a contradiction from the properties of probability. 

Next, we check the upper bound when it equals $\frac{p^\prime_{11}}{x}$, and proceed by a similar proof by contradiction.

\textbf{Proof}: Assume 
\begin{align*}
    \frac{\Big\{p_{11} - p_{10}\Big\}(1 - x)}{y} + p^\prime_{11} > \frac{p^\prime_{11}}{x}\\
    \implies p_{11}(1 - x)x - p_{10}(1 - x)x + p^\prime_{11}yx > p^\prime_{11}y\\
    \implies p_{11}(1 - x)x - p_{10}(1 - x)x > p^\prime_{11}y(1 - x)\\
    \implies x\Big\{p_{11} - p_{10}\Big\} > p^\prime_{11}y\\
    % \implies -p^\prime_{10}(1 - y) > 0
\end{align*}

Since we assume $p_{11} - p_{10} < 0$, this produces a contradiction and concludes the proof.

Finally, when the upper bound is $\frac{(1 - x)(1- y) - p_{10}(1 - x) + p^\prime_{11}y}{xy}$, we proceed by a similar proof by contradiction strategy.

\textbf{Proof}: Assume
\begin{align*}
    \frac{\Big\{p_{11} - p_{10}\Big\}(1 - x)}{y} + p^\prime_{11} > \frac{(1 - x)(1- y) - p_{10}(1 - x) + p^\prime_{11}y}{xy}\\
    \implies \Big\{p_{11} - p_{10}\Big\}(1 - x) + p^\prime_{11}y > \frac{(1 - x)(1- y) - p_{10}(1 - x) + p^\prime_{11}y}{x}\\
    \implies x\Big\{p_{11} - p_{10}\Big\}(1 - x) > (1 - x)(1- y) - p_{10}(1 - x) + p^\prime_{11}y(1 - x)\\
    \implies x\Big\{p_{11} - p_{10}\Big\} > (1- y) - p_{10} + p^\prime_{11}y\\
    \implies p_{11}x + p_{10}(1 - x) > (1 - y) + p^\prime_{11}y\\
        \implies p_{11}x + p_{10}(1 - x) - p^\prime_{11}y > (1 - y) \\
    \intertext{Using the inequality $p_{11}x + p_{10}(1 - x) - p^\prime_{11}y = p^\prime_{10}(1 - y)$}
    \implies p^\prime_{10}(1 - y) > (1 - y)
\end{align*}

And this is a contradiction from the properties of probability. 

And so, in Case 1, the upper bound will always be $\geq \frac{\Big\{p_{11} - p_{10}\Big\}(1 - x)}{y} + p^\prime_{11}$. 

\subsubsection{Case 2}

But, we still need to ensure that the lower bound isn't so high that we wander into the right side of the graph. So, we follow a similar proof by contradiction approach to demonstrate the lower bounds relation to $p^\prime_{11}$. 

First, by the properties of probability $p^\prime_{11} \geq 0$ will always hold. 

Next, when the lower bound is $\frac{p^\prime_{11} - (1 - x)}{x}$, applying a proof by contradiction strategy. 

\textbf{Proof}: Assume $\frac{p^\prime_{11} - (1 - x)}{x} > p^\prime_{11}$. This creates a contradiction since this implies $p^\prime_{11} > 1$, and so we prove the opposite.

Next, consider the case where the lower bound is $\frac{p_{11} - (1 - y)}{y}$, following a similar proof by contradiction strategy.

\textbf{Proof}: Assume $\frac{p_{11} - (1 - y)}{y} > p^\prime_{11}$. This implies 
\begin{align*}
    p_{11} > p^\prime_{11}y + (1 - y)\\
    \implies 1 - p_{01} > (p^\prime_{11}y - y) + 1\\
    \implies p_{01} < p^\prime_{01}y 
\end{align*}

This is a contradiction because of Equation \ref{lower-bound-max-constraint}, since an implication of $\frac{p_{11} - (1 - y)}{y} > p^\prime_{11}$ being the lower bound is $P(Z = 0 \mid X = 1)P(X = 1) \geq P(Z = 0 \mid Y =1)P(Y = 1)$ and this contradicts that. 


Finally, consider the case where $\frac{p^\prime_{11}y - p_{10}(1 - x)}{xy}$, following a similar proof by contradiction approach. 

\textbf{Proof}: Assume $\frac{p^\prime_{11}y - p_{10}(1 - x)}{xy} > p^\prime_{11}$, this implies
\begin{align*}
    p^\prime_{11}y - p_{10}(1 - x) > p^\prime_{11}xy\\
    p^\prime_{11}y(1 - x) > p_{10}(1 - x)\\
    p^\prime_{11}y  > p_{10}
\end{align*}

{\color{blue}
\begin{align*}
    &p^\prime_{11}y  > p_{10} \\
    \xRightarrow{p_{11}x + p_{10}(1-x) = p'_{11}y + p'_{10}(1-y) }& p_{11}x + p_{10}(1-x) - p'_{10}(1-y) > p_{10}\\
    \implies p_{11}x > p'_{10}(1-y) + p_{10}x \\
    \implies (p_{11}-p_{10})x > p'_{10}(1-y)
\end{align*}
which is a contradiction because $p_{11}-p_{10} < 0$. 
}

\subsection{Case II: $p_{11} - p_{10} > 0$}
\begin{center}
\includegraphics[scale=0.15]{IMG_B0C2239F4243-1.jpeg}    
\end{center}

The turning points in this graph are obtained as follows:
\begin{align*}
   p_{11} - p_{10} + \frac{p^\prime_{11}y}{1 - x} - \frac{y\mathbb{P}(Z = 1\mid X = 1, Y = 1)}{1 - x} \geq p_{11} - p_{10} \\ 
   \implies \frac{p^\prime_{11}y}{1 - x} - \frac{y\mathbb{P}(Z = 1\mid X = 1, Y = 1)}{1 - x} \geq 0 \implies p^\prime_{11} \geq P(Z = 1\mid X = 1, Y = 1) \\ 
\end{align*}

Now, doing a similar calculation for the other turning point
\begin{align*}
     \frac{\mathbb{P}(Z = 1 \mid X = 1, Y = 1)y - p^\prime_{11}y}{1 - x} \geq p_{11} - p_{10}\\
     \implies P(Z = 1 \mid X = 1, Y = 1) \geq \frac{\Big\{ p^\prime_{11} - p^\prime_{10}\Big\}(1 - x)}{y} + p^\prime_{11}
\end{align*}

Now, we do a similar case by case analysis for falsification. 

\subsubsection{Case 1}

We want to check whether the upper bounds can be less that $p^\prime_{11}$. 

When the upper bound is $1$, this can never be less than $p^\prime_{11}$ from the properties of probability. 

Next, when the upper bound is $\frac{p^\prime_{11}}{x}$, this will also hold since $x \leq 1$. 

Next, when the upper bound is $\frac{p_{11}}{y}$, we follow a proof by contradiction, with the proof presented below. 

\textbf{Proof}: Assume $p^\prime_{11} > \frac{p_{11}}{y}$

\begin{align*}
    \implies p^\prime_{11}y > p_{11}\\
    \implies p_{11}x + p_{10}(1 - x) - p^\prime_{10}(1 - y) > p_{11}\\
    \implies - p^\prime_{10}(1 - y) > \{p_{11} - p_{10}\}(1 - x)\\
\end{align*}
This produces a contradiction since $p_{11} - p_{10} > 0$ by assumption. 

Next, when the upper bound is $\frac{(1 - x)(1 - y) - p_{10}(1 - x) + p^\prime_{11}y}{xy}$, following a similar proof by contradiction strategy.

\textbf{Proof}: Assume $p^\prime_{11} > \frac{(1 - x)(1 - y) - p_{10}(1 - x) + p^\prime_{11}y}{xy}$

\begin{align*}
    \implies p^\prime_{11}xy > (1 - x)(1 - y) - p_{10}(1 - x) + p^\prime_{11}y\\
    \implies 0 < (1 - x)(1 - y) - p_{10}(1 - x) + p^\prime_{11}y(1 - x)\\
    \implies 0 < (1 - y) - p_{10} + p^\prime_{11}y\\
    \implies 0 < p_{00} - p^\prime_{01}y\\
    \implies p^\prime_{01}y < p_{00} 
\end{align*}

{\color{blue} 
The above proof is wrong ;) . Please double check and replace with the one I wrote here:

\begin{align*}
    \implies p^\prime_{11}xy > (1 - x)(1 - y) - p_{10}(1 - x) + p^\prime_{11}y\\
    \implies 0 > (1 - x)(1 - y) - p_{10}(1 - x) + p^\prime_{11}y(1 - x)\\
    \implies 0 > (1 - y) - p_{10} + p^\prime_{11}y\\
    \implies p_{10} > (1-y) + p^\prime_{11}y\\
    %  \xRightarrow{p_{11}x + p_{10}(1-x) = p'_{11}y + p'_{10}(1-y) }& p_{11}x + p_{10}(1-x) - p'_{10}(1-y) > p_{10}\\
    % \implies p_{10} > (1-y) + p_{11} x + p_{10}(1-x) - p'_{10}(1-y)\\
    \implies 0> (1-y) + p_{11}x - p_{10} x - p'_{10}(1-y)\\
    \implies p'_{10}(1-y) > (1-y) + x(p_{11}-p_{10})\\
    \implies (p'_{10}-1)> x \frac{p_{11}-p_{10}}{1-y}
\end{align*}
which is a contradiction because $x \frac{p_{11}-p_{10}}{1-y}$ is a positive quantity and $p'_{10}-1$ is a negative one, since $p'_{10}$ is a probability. 
}

% {\color{red} This doesn't produce the contradiction we hope for.}

\subsubsection{Case 2}

We check whether the lower bounds can be greater than $\frac{\Big\{ p^\prime_{11} - p^\prime_{10}\Big\}(1 - x)}{y} + p^\prime_{11}$. 

\begin{itemize}
    \item Lower Bound Of $0$: This produces a contradiction since $p_{11} - p_{10}$ is positive, and $p^\prime_{11}$ is also positive, and so a sum of two positive quantities cannot be negative. 
    \item Lower Bound of $\frac{p^\prime_{11} - (1 - x)}{x}$: This follows a proof by contradiction.
    \begin{align*}
        \frac{\Big\{ p_{11} - p_{10}\Big\}(1 - x)}{y} + p^\prime_{11} < \frac{p^\prime_{11} - (1 - x)}{x}]\\
        \implies x\{p_{11} - p_{10}\}(1 - x) + p^\prime_{11}xy < p^\prime_{11}y - y(1 - x)\\
        \implies x\{p_{11} - p_{10}\}(1 - x) < p^\prime_{11}y(1 - x) - y(1 - x)\\
        \implies x\{p_{11} - p_{10}\} < p^\prime_{11}y - y\\
        \implies x\{p_{11} - p_{10}\} < -yp^\prime_{01}\\
    \end{align*}
    This produces a contradiction since $p_{11} - p_{10} > 0$
    \item Lower Bound Of $\frac{p_{11} - (1 - y)}{y}$: Following a similar proof by contradiction:
    \begin{align*}
        \frac{\Big\{ p_{11} - p_{10}\Big\}(1 - x)}{y} + p^\prime_{11} < \frac{p_{11} - (1 - y)}{y}\\
        \implies \Big\{ p_{11} - p_{10}\Big\}(1 - x) + p^\prime_{11}y < p_{11} - (1 - y)\\
        \implies -p_{10}(1 - x) - p_{11}x + p^\prime_{11}y < -(1 - y)\\
        \xRightarrow{p_{11}x + p_{10}(1-x) = p'_{11}y + p'_{10}(1-y) } -p^\prime_{10}(1 - y) < -(1 - y)
        \implies p^\prime_{10} > 1
    \end{align*}
    This is a contradiction from the properties of probability.
    \item When the lower bound is $\frac{p^\prime_{11}y - p_{10}(1 - x)}{xy}$. Following a similar proof by contradiction
    \begin{align*}
        \frac{\Big\{ p_{11} - p_{10}\Big\}(1 - x)}{y} + p^\prime_{11} < \frac{p^\prime_{11}y - p_{10}(1 - x)}{xy}\\
        \implies \Big\{ p_{11} - p_{10}\Big\}(1 - x) + p^\prime_{11}y < \frac{p^\prime_{11}y - p_{10}(1 - x)}{x}\\
        \implies x\Big\{ p_{11} - p_{10}\Big\}(1 - x) + p^\prime_{11}yx < p^\prime_{11}y - p_{10}(1 - x)\\
        \implies x\Big\{ p_{11} - p_{10}\Big\}(1 - x) < p^\prime_{11}y(1 - x) - p_{10}(1 - x)\\
        \implies x\Big\{ p_{11} - p_{10}\Big\} < p^\prime_{11}y - p_{10}\\
        \implies xp_{11} + p_{10}(1 - x) - p^\prime_{11}y < 0\\
        \xRightarrow{p_{11}x + p_{10}(1-x) = p'_{11}y + p'_{10}(1-y) } p^\prime_{10}(1 - y) < 0
    \end{align*}
    This produces a contradiction as well.
    \end{itemize}

So we have shown in both cases where $0 > p_{11} - p_{10}$ and vice versa, that $0$ or $p_{11} - p_{10}$ will always be included based on the allowed range of $P(Z = 1 \mid X = 1, Y = 1)$. This concludes the proof for the lower bound. 

\section{Final Proof: Causal Marginal Problem Upper Bound}

Given $P(Z, X)$ and $P(Z, Y)$, and indexing the set of joint distributions $P(Z, X, Y)$ compatible with these constraints by $P^{(i)}$, we want to pick the most upper bound for PNS/PC. To do this, we use the following upper bound
\begin{align*}
    PNS \leq p_{11} - \Gamma
\end{align*}

Where $\Gamma$ is 
\begin{align*}
    \Gamma = \sum_y \mathbb{P}(Y = y)\max \{0, \mathbb{P}(Z = 1 \mid X = 1, Y = y) - \mathbb{P}(Z = 0 \mid X = 0, Y = y)\} 
\end{align*}

Since we want to pick the highest upper bound, we want to pick the smallest value of $\Gamma$ since it is subtracted from $P(Z = 1\mid X = 1)$. So this is equivalent to
\[
\min_{P^{(i)}} \Gamma
\]

Now, based on Equations \ref{eq:gamma-term-1} and \ref{eq:gamma-term-2}, we can rewrite the above as 
{\scriptsize
\begin{align*}
         \min_{P_i}\max\begin{bmatrix}
             0 \\
             p_{11} + p_{10} - 1\\
             \mathbb{P}(Y = 0)\{\mathbb{P}(Z = 1 \mid X = 1, Y = 0) - \mathbb{P}(Z = 0 \mid X = 0, Y = 0)\}\\
             \mathbb{P}(Y = 1)\{\mathbb{P}(Z = 1 \mid X = 1, Y = 1) - \mathbb{P}(Z = 0 \mid X = 0, Y = 1)\}
         \end{bmatrix}
\end{align*}
}

Which from Equations \ref{eq:gamma-term-1} and \ref{eq:gamma-term-2} is equal to
\begin{align*}\label{gamma}
         \min_{P_i}\max\begin{bmatrix}
             0 \\
             p_{10} + p_{11} - 1\\
             yP(Z = 1\mid X = 1, Y = 1)(OR(X) - 1) + \Phi_X + y - \frac{p^\prime_{11}y}{1 - x}\\
             P(Z = 1 \mid X = 1, Y = 1)(1 - OR(X))y + y\frac{p^\prime_{11} - (1 - x)}{1 - x} \\
         \end{bmatrix}
\end{align*}

Now, this is analyzed on a case by case basis, and for begin with analyzing the situation where $p_{11} + p_{10} - 1 < 0$

\subsection{Case I: $p_{11} + p_{10} - 1 < 0$}

As we can see from above, depending on whether $OR(X) - 1$ is positive or negative, line 3 and line 4 in the above matrix will be increasing or decreasing functions of $P(Z = 1 \mid X = 1, Y = 1)$.

Assuming $x > 1 - x$, line 3 is an increasing function of $P(Z = 1 \mid X = 1, Y = 1)$ and line 4 is a decreasing function of this. Since falsification happens when line 3 and line 4 of the matrix are greater than 0, we first check the values of $P(Z = 1 \mid X = 1, Y = 1)$ for which this happens. 
\begin{itemize}
    \item When $yP(Z = 1\mid X = 1, Y = 1)(OR(X) - 1) + \Phi_X + y - \frac{p^\prime_{11}y}{1 - x} \geq 0$:
    \begin{equation}
        \implies P(Z = 1 \mid X = 1, Y = 1) \geq \frac{p^\prime_{11}y - (1 - x)(\Phi_X + y)}{y(x - (1 - x))}\\
    \end{equation}\label{val:turning-point-a}

    We denote this value as 
    \begin{equation}\label{b}
        b =\frac{p^\prime_{11}y - (1 - x)(\Phi_X + y)}{y(x - (1 - x))} 
    \end{equation}
    
    \item When $P(Z = 1 \mid X = 1, Y = 1)(1 - OR(X))y + y\frac{p^\prime_{11} - (1 - x)}{1 - x} \geq 0$
    \begin{equation}
        \implies \frac{p^\prime_{11} - (1 - x)}{x - (1 - x)} \geq P(Z = 1 \mid X = 1, Y = 1)
    \end{equation}\label{val:turning-point-b}

    We denote this value as
    \begin{equation}\label{a}
        a = \frac{p^\prime_{11} - (1 - x)}{x - (1 - x)}
    \end{equation}.
\end{itemize}

\subsection{Case By Case Upper Bound Calculation}

Each of these sections considers a different case where the values of $p^\prime_{11}$, $p^\prime_{10}$ are picked relative to $x$ and $1 - x$.

\subsubsection{Case I}

This case assumes the following
\begin{align}
    \Phi_X < 0\\
    1 - x < x\\
    1 - x < p^\prime_{11} < x\\
    p^\prime_{10} < 1 - x < x
\end{align}

The first two have been assumed in a larger context, and the last two are made for this specific case for this section. 

These conditions, based on the implications in subsection \ref{implications_bounds_p111}, limit the choice of bounds on $P(Z = 1 \mid X = 1, Y = 1)$ from (\ref{p_111_bounds}) to 
\[
\max \begin{bmatrix}
    \frac{p^\prime_{11} - (1 - x)}{x}\\
    \frac{p^\prime_{11}y - p_{10}(1 - x)}{xy}
\end{bmatrix} \leq P(Z = 1 \mid X = 1, Y = 1) \leq 
\min \begin{bmatrix}
   \frac{p_{11}}{y}\\
   \frac{p^\prime_{11}}{x}
\end{bmatrix}
\]

Now, we know falsification will happen when either lower bound is greater than \ref{b}, or the upper bound is less than \ref{a}. So we examine each choice of upper and lower bound, and see whether they can be less than \ref{a} or \ref{b}. 
\begin{enumerate}
    \item $\frac{p^\prime_{11} - (1 - x)}{x} $: This will be less than \ref{a}, i.e. $\frac{p^\prime_{11} - (1 - x)}{x}  < \frac{p^\prime_{11} - (1 - x)}{2x - 1}$ since the denominator is smaller on the right hand side. Since this is less than $(a)$, it will also be less than \ref{b}.
    \item $\frac{p^\prime_{11}y - p_{10}(1 - x)}{xy}$: This will always be less than \ref{b}, which we prove below. Assume
    \[
    \frac{p^\prime_{11}y - p_{10}(1 - x)}{xy} > \frac{p^\prime_{11}y - (1 - x)(p_{11} + p_{10} - 1) - y(1 - x)}{y(x - (1 - x))}
    \]

    Checking the right hand side of the implication
    \begin{align*}
        &\implies p^\prime_{11}y(x - (1 - x)) - p_{10}(1 - x)(x - (1 - x)) > p^\prime_{11}xy - x(1 - x)(p_{11} + p_{10} - 1) -xy(1 - x)\\
        &\implies -p^\prime_{11}y - p_{10}(x - (1 - x)) >  - x(p_{11} + p_{10} - 1) -xy\\
        &\implies -p^\prime_{11}y + p_{10}(1 - x) - p_{10}x  >  - xp_{11} - xp_{10} + x -xy\\
        &\implies -p^\prime_{11}y + p_{10}(1 - x) + xp_{11}  >  x(1 - y)\\
        &\implies p^\prime_{10}(1 - y) > x(1 - y) \implies p^\prime_{10} > x
    \end{align*}

    This is a contradiction based on the case we are in.
\end{enumerate}


And so, the lower bounds will always be less than \ref{b}, so any falsification will come from the upper bounds being less than \ref{a}, which we check below. 

\begin{enumerate}
    \item When the upper bound is $\frac{p_{11}}{y}$: Checking this against \ref{b} using a proof by contradiction, we assume
    \begin{align*}
        &\frac{p^\prime_{11}y - (1 - x)(p_{11} + p_{10} - 1) - y(1 - x)}{y(x - (1 - x))} < \frac{p_{11}}{y}\\
       &\implies p^\prime_{11}y - (1 - x)(p_{11} + p_{10} - 1) - y(1 - x) < p_{11}x - p_{11}(1 - x)\\
       &\implies p_{11}x + p_{10}(1 - x) - p^\prime_{10}(1 - y) - (1 - x)(p_{11} + p_{10} - 1) - y(1 - x) < p_{11}x - p_{11}(1 - x)\\
       &\implies p_{10}(1 - x) + p_{11}(1 - x) - p^\prime_{10}(1 - y) - (1 - x)(p_{11} + p_{10} - 1) - y(1 - x) < 0\\
       &\implies - p^\prime_{10}(1 - y) + (1 - x) - y(1 - x) < 0\\
       &\implies - p^\prime_{10}(1 - y) + (1 - x)(1 - y) < 0\\
       &\implies - p^\prime_{10} + (1 - x) < 0\\
    \end{align*}
    This is a contradiction, and so $\frac{p^\prime_{11}y - (1 - x)(p_{11} + p_{10} - 1) - y(1 - x)}{y(x - (1 - x))} \geq \frac{p_{11}}{y}$. Similarly, checking $\frac{p_{11}}{y}$ against \ref{a}

    \begin{align*}
    \frac{p_{11}}{y} < \frac{p^\prime_{11} - (1 - x)}{x - (1 - x)}
    \implies p_{11}x - p_{11}(1 - x) < p^\prime_{11}y - y(1 - x)\\
    \implies p_{11}x - p_{11}(1 - x) < p_{11}x + p_{10}(1 - x) - p^\prime_{10}(1 - y) - y(1 - x)\\
    \implies - p_{11}(1 - x) < p_{10}(1 - x) - p^\prime_{10}(1 - y) - y(1 - x)\\
    \implies p^\prime_{10}(1 - y)  < p_{10}(1 - x) + p_{11}(1 - x)  - y(1 - x)\\
    \implies p^\prime_{10}(1 - y)  < (1 - x)(p_{10} + p_{11}  - (1 - (1 - y)))\\
    \implies p^\prime_{10}(1 - y)  < (1 - x)(p_{10} + p_{11}  - 1) + (1 - x)(1 - y)\\
    \implies \frac{(1 - y)(p^\prime_{10} - (1 - x))}{1 - x}  < \Phi_X\\
    \end{align*}

    So, when $\frac{(1 - y)(p^\prime_{10} - (1 - x))}{1 - x}  < \Phi_X$, $\frac{p_{11}}{y}$ will be less than \ref{a} and we can get falsification. 
    
    \item When the upper bound is $\frac{p^\prime_{11}}{x}$: Checking this against the first turning point, since the graphical argument above is reliant on this.
    \begin{align*}
    \frac{p^\prime_{11}}{x} < \frac{p^\prime_{11} - (1 - x)}{x - (1 - x)}
    \implies p^\prime_{11}x - p^\prime_{11}(1 - x) < p^\prime_{11}x - x(1 - x)\\
    \implies p^\prime_{11} > x
    \end{align*}
    This is a contradiction because of the case we are in, and so $\frac{p^\prime_{11}}{x} \geq \frac{p^\prime_{11} - (1 - x)}{x - (1 - x)}$
\end{enumerate}

Putting this all together, any falsification will come from the upper bounds being less than \ref{a}. The only upper bound capable of being less than \ref{a} is $\frac{p_{11}}{y}$. This gives us the first needed condition for falsification 
\[\frac{p_{11}}{y} > \frac{p^\prime_{11}}{x} \implies p_{11}x > p^\prime_{11}y\]


Next, we examine the pairing with each of the lower bounds. 
\begin{enumerate}
    \item When the lower bound is $\frac{p^\prime_{11} - (1 - x)}{x - (1 - x)}$: As proved before, this will always be less than \ref{a}, so in this case we only check when $\frac{p_{11}}{y}$ is less than (a). We have solved this before and the condition is $\frac{(1 - y)(p^\prime_{10} - (1 - x))}{1 - x}  < \Phi_X$. Then $\frac{p_{11}}{y}$ is substituted into $P(Z = 1 \mid X = 1, Y = 1)(1 - OR(X))y + y\frac{p^\prime_{11} - (1 - x)}{1 - x}$. And this equals
    \begin{align*}
    &p_{11}(1 - OR(X)) + y\frac{p^\prime_{11} - (1 - x)}{1 - x}\\
    &= p_{11} - \frac{p_{11}x}{1 - x} + y\frac{p^\prime_{11} - (1 - x)}{1 - x}\\
    &= p_{11} + \frac{p^\prime_{11}y - y(1 - x) - p_{11}x}{1 - x}\\
    &= p_{11} + \frac{p_{10}(1 - x) - p^\prime_{10}(1 - y) - y(1 - x) }{1 - x}\\
    &= \frac{p_{11}(1 - x) + p_{10}(1 - x) - p^\prime_{10}(1 - y) - (1 - (1 - y))(1 - x) }{1 - x}\\
    &= \Phi_X + \frac{ - p^\prime_{10}(1 - y) + (1 - y)(1 - x) }{1 - x}\\
    &= \Phi_X - \frac{(1 - y)(p^\prime_{10}(1 - y) - (1 - x)}{1 - x}\\
    \end{align*}
    This will be the output of $\Gamma$.
    \item When the lower bound is $\frac{p^\prime_{11}y - p_{10}(1 - x)}{xy}$: Since the upper bound is the same, the falsification calculation is the same. Since the lower bound is always less than the upper bound, we have the same calculation and same condition for falsification. 
\end{enumerate}

% for the final piece, we want to check whether $\frac{p_{11}}{y}$ will be less than or greater than the first turning point. 
% \begin{align*}
%     \frac{p_{11}}{y} < \frac{p^\prime_{11} - (1 - x)}{x - (1 - x)}
%     \implies p_{11}x - p_{11}(1 - x) < p^\prime_{11}y - y(1 - x)\\
%     \implies p_{11}x - p_{11}(1 - x) < p_{11}x + p_{10}(1 - x) - p^\prime_{10}(1 - y) - y(1 - x)\\
%     \implies - p_{11}(1 - x) < p_{10}(1 - x) - p^\prime_{10}(1 - y) - y(1 - x)\\
%     \implies p^\prime_{10}(1 - y)  < p_{10}(1 - x) + p_{11}(1 - x)  - y(1 - x)\\
%     \implies p^\prime_{10}(1 - y)  < (1 - x)(p_{10} + p_{11}  - (1 - (1 - y)))\\
%     \implies p^\prime_{10}(1 - y)  < (1 - x)(p_{10} + p_{11}  - 1) + (1 - x)(1 - y)\\
%     \implies \frac{(1 - y)(p^\prime_{10} - (1 - x))}{1 - x}  < p_{10} + p_{11}  - 1\\
% \end{align*}

Putting this all together, in Case I, when the following conditions hold:
\begin{align*}
    &p_{11}x > p^\prime_{11}y\\
    &\frac{(1 - y)(p^\prime_{10} - (1 - x))}{1 - x}  < \Phi_X
\end{align*}
% So, when $\frac{(1 - y)(p^\prime_{10} - (1 - x))}{1 - x}  > p_{10} + p_{11}  - 1 \implies \frac{p_{11}}{y} \geq \frac{p^\prime_{11} - (1 - x)}{x - (1 - x)}$, and we don't get any falsification. 

We will get falsification, where $\Gamma$ is calculated as
\[ \Gamma = \Phi_X - \frac{(1 - y)(p^\prime_{10} - (1 - x))}{1 - x} \]

Now, subtracting this from $p_{11}$, we have
\begin{align*}
 p_{11} - \Gamma &= p_{11} - (p_{11} + p_{10} - 1) + \frac{(1 - y)(p^\prime_{10} - (1 - x))}{1 - x}\\
 p_{11} - \Gamma &= p_{00} - \frac{(1 - y)((1 - x) - p^\prime_{10})}{1 - x}
\end{align*}

\subsubsection{Case II}

This case assumes the following
\begin{align}
    \Phi_X < 0\\
    1 - x < x\\
    1 - x < p^\prime_{11} < x\\
    1 - x < p^\prime_{10} < x
\end{align}

These conditions limit the choice of bounds on $P(Z = 1 \mid X = 1, Y = 1)$ from (\ref{p_111_bounds}) to 
\[max
\begin{bmatrix}
    \frac{p^\prime_{11} - (1 - x)}{x}\\
    \frac{p^\prime_{11}y - p_{10}(1 - x)}{xy}
\end{bmatrix} \leq P(Z = 1 \mid X = 1, Y = 1) \leq 
min\begin{bmatrix}
   \frac{p^\prime_{11}}{x}\\
   \frac{(1 - x)(1 - y) - p_{10}(1 - x) + p^\prime_{11}y}{xy}
\end{bmatrix}
\]

Now, we check whether the lower bounds are greater than (b) and if the upper bounds are less than (a).
\begin{enumerate}
    \item First, $\frac{p^\prime_{11} - (1 - x)}{x} < \frac{p^\prime_{11} - (1 - x)}{2x - 1}$ since the denominator is smaller on the right hand side. This lower bound is less than (a), and will consequently be less than (b). 
    \item Checking the lower bound of $\frac{p^\prime_{11}y - p_{10}(1 - x)}{xy}$ against (b), using a proof by contradiction. Assume,
    \[ \frac{p^\prime_{11}y - p_{10}(1 - x)}{xy} > 
        \frac{p^\prime_{11}y - (1 - x)(p_{11} + p_{10} - 1) - y(1 - x)}{y(x - (1 - x))}
    \]

Checking the right hand side of the implication
\begin{align*}
    &\implies p^\prime_{11}y(x - (1 - x)) - p_{10}(1 - x)(x - (1 - x)) > p^\prime_{11}xy - x(1 - x)(p_{11} + p_{10} - 1) -xy(1 - x)\\
    &\implies -p^\prime_{11}y - p_{10}(x - (1 - x)) >  - x(p_{11} + p_{10} - 1) -xy\\
    &\implies -p^\prime_{11}y + p_{10}(1 - x) - p_{10}x  >  - xp_{11} - xp_{10} + x -xy\\
    &\implies -p^\prime_{11}y + p_{10}(1 - x) + xp_{11}  >  x(1 - y)\\
    &\implies p^\prime_{10}(1 - y) > x(1 - y) \implies p^\prime_{10} > x
\end{align*}

This is a contradiction based on the case we are in. So,
    \[
        \frac{p^\prime_{11}y - p_{10}(1 - x)}{xy} \leq 
        \frac{p^\prime_{11}y - (1 - x)(p_{11} + p_{10} - 1) - y(1 - x)}{y(x - (1 - x))}
    \]
    % $ > \frac{p^\prime_{11} - (1 - x)}{2x - 1}$
    % \begin{align*}
    % &\implies p^\prime_{11}y(x - (1 - x)) - p_{10}(1 - x)(x - (1 - x)) > p^\prime_{11}xy - xy(1 - x)\\
    % &\implies -p^\prime_{11}y - p_{10}x + p_{10}(1 - x) > -xy\\
    % &\implies p_{10}(1 - x) - p^\prime_{11}y> (p_{10} - y)x
    % \end{align*}
    % This doesn't inherently create a contradiction since both of these are negative quantities.
\end{enumerate}

Checking the upper bounds now. 

\begin{enumerate}
    \item When the upper bound is $\frac{p^\prime_{11}}{x}$: Checking this against the (a).
    \begin{align*}
    \frac{p^\prime_{11}}{x} < \frac{p^\prime_{11} - (1 - x)}{x - (1 - x)}
    \implies p^\prime_{11}x - p^\prime_{11}(1 - x) < p^\prime_{11}x - x(1 - x)\\
    \implies p^\prime_{11} > x
    \end{align*}
    This is a contradiction because of the case we are in. So
    \[
    \frac{p^\prime_{11}}{x} \geq \frac{p^\prime_{11} - (1 - x)}{x - (1 - x)}
    \]
    \item When the upper bound is $\frac{(1 - x)(1 - y) - p_{10}(1 - x) + p^\prime_{11}y}{xy}$: Assume
    \[
    \frac{(1 - x)(1 - y) - p_{10}(1 - x) + p^\prime_{11}y}{xy} < \frac{p^\prime_{11} - (1 - x)}{x - (1 - x)}
    \]
    \begin{align*}
      &\implies (1 - x)(1 - y)(x - (1 - x)) - p_{10}(1 - x)(x - (1 - x)) + p^\prime_{11}y(x - (1 - x)) < p^\prime_{11}xy - xy(1 - x)\\
      &\implies (1 - x)(1 - y)(x - (1 - x)) - p_{10}(1 - x)(x - (1 - x)) -p^\prime_{11}y(1 - x) < - xy(1 - x)\\
      &\implies (1 - y)(x - (1 - x)) - p_{10}(x - (1 - x)) -p^\prime_{11}y < - xy\\
      &\implies x - xy - (1 - y)(1 - x) - p_{10}(x - (1 - x)) -p^\prime_{11}y < - xy\\
      &\implies x - (1 - y)(1 - x) - p_{10}(x - (1 - x)) -p^\prime_{11}y < 0\\
      &\implies x - p_{10}x - (1 - y)(1 - x) + p_{10}(1 - x) -p^\prime_{11}y < 0\\
      &\implies x - p_{10}x - (1 - y)(1 - x) + p^\prime_{10}(1 - y) - p_{11}x < 0\\
      &\implies x(1 - p_{10} - p_{11}) - (1 - y)(1 - x) + p^\prime_{10}(1 - y)  < 0\\
      &\implies  (1 - y)(p^\prime_{10} - (1 - x))  < x(p_{11} + p_{10} - 1)\\
    \end{align*}
    This creates a contradiction since the LHS is positive but the RHS is negative.

    So, no falsification in this case. So,

    \[
    \frac{(1 - x)(1 - y) - p_{10}(1 - x) + p^\prime_{11}y}{xy} \geq \frac{p^\prime_{11} - (1 - x)}{x - (1 - x)}
    \]
\end{enumerate}


Since the lower bounds are less than (b), and upper bounds are greater than (a), so $\Gamma = 0$. 

\subsubsection{Case III} 

This case assumes the following conditions
\begin{align}
    \Phi_X < 0\\
    1 - x < x\\
    1 - x < p^\prime_{11} < x\\
    1 - x < x < p^\prime_{10}
\end{align}

These conditions limit the choice of bounds on $P(Z = 1 \mid X = 1, Y = 1)$ from (\ref{p_111_bounds}) to 
\[\max
\begin{bmatrix}
    \frac{p^\prime_{11} - (1 - x)}{x}\\
    \frac{p_{11} - (1 - y)}{y}
\end{bmatrix} \leq P(Z = 1 \mid X = 1, Y = 1) \leq 
\min\begin{bmatrix}
   \frac{p^\prime_{11}}{x}\\
   \frac{(1 - x)(1 - y) - p_{10}(1 - x) + p^\prime_{11}y}{xy}
\end{bmatrix}
\]

Following the usual approach, we start with checking the lower bounds against \ref{b}.

\begin{enumerate}
\item The lower bound of $\frac{p^\prime_{11} - (1 - x)}{x}$ will be less than \ref{a}, and so less than \ref{b}. 
\item Checking $\frac{p_{11} - (1 - y)}{y}$: Checking whether
    $\frac{p_{11} - (1 - y)}{y} \geq \frac{p^\prime_{11}y - (1 - x)(p_{11} + p_{10} - 1) - y(1 - x)}{y(x - (1 - x))}$. Assume
    {\small
    \begin{align*}
        &\frac{p_{11} - (1 - y)}{y} < \frac{p^\prime_{11}y - (1 - x)(p_{11} + p_{10} - 1) - y(1 - x)}{y(x - (1 - x))}\\
        &\implies p_{11} - (1 - y) < \frac{p^\prime_{11}y - (1 - x)(p_{11} + p_{10} - 1) - y(1 - x)}{(x - (1 - x))}\\
        &\implies p_{11}x - p_{11}(1 - x) - (1 - y)(x - (1 - x)) < p^\prime_{11}y - (1 - x)(p_{11} + p_{10} - 1) - y(1 - x)\\
        &\implies p^\prime_{10}(1 - y) - p_{10}(1 - x) - p_{11}(1 - x) - (1 - y)x + (1 - y)(1 - x) < - (1 - x)(p_{11} + p_{10} - 1) - y(1 - x)\\
        &\implies p^\prime_{10}(1 - y) -(1 - x)(p_{10} + p_{11} - 1) - (1 - y)x  - y(1 - x) < - (1 - x)(p_{11} + p_{10} - 1) - y(1 - x)\\
        &\implies p^\prime_{10} < x\\
    \end{align*}
    }
    This contradicts the assumptions of this case, so we expect $\frac{p_{11} - (1 - y)}{y} \geq \frac{p^\prime_{11}y - (1 - x)(p_{11} + p_{10} - 1) - y(1 - x)}{y(x - (1 - x))}$ to hold. And we will come back to this for falsification calculations. 
\end{enumerate}

Now, we check the upper bounds against \ref{a}.
\begin{enumerate}
    \item Upper bound is $\frac{p^\prime_{11}}{x}$: 
    \begin{align*}
        \frac{p^\prime_{11}}{x} < \frac{p^\prime_{11} - (1 - x)}{x - (1 - x)}
        \implies p^\prime_{11}x - p^\prime_{11}(1 - x) < p^\prime_{11}x - x(1 - x)\\
        \implies p^\prime_{11} > x
    \end{align*}
    This is a contradiction because of the case we are in. So
    \[
    \frac{p^\prime_{11}}{x} \geq \frac{p^\prime_{11} - (1 - x)}{x - (1 - x)}
    \]
    \item Upper bound is $\frac{(1 - x)(1 - y) - p_{10}(1 - x) + p^\prime_{11}y}{xy}$. Assume 
    \[
    \frac{(1 - x)(1 - y) - p_{10}(1 - x) + p^\prime_{11}y}{xy} < \frac{p^\prime_{11} - (1 - x)}{x - (1 - x)}
    \]
    \begin{align*}
        \implies (1 - y)(p^\prime_{10} - (1 - x)) < x\Phi_X
    \end{align*}
    This is a contradiction since the RHS is negative, but the LHS in positive.
\end{enumerate}

Now, the first condition that must be satisfied is $\frac{p_{11} - (1 - y)}{y}$ is the lower bound, which requires the following condition to hold
\[
p_{01}x < p^\prime_{01}y
\]

Then, we substitute the lower bound into the increasing function of $P(Z = 1\mid X = 1, Y = 1)$
\begin{align*}
    &\frac{(1 - x)(p_{10} + p_{11} - 1) - p^\prime_{11}y + P(Z = 1\mid X = 1, Y = 1)y(x - (1 - x)) + (1 - x)y}{1 - x}\\
    &= \frac{(1 - x)(p_{10} + p_{11} - 1) - p^\prime_{11}y + (p_{11} - (1 - y))(x - (1 - x)) + (1 - x)y}{1 - x}\\
    &= \frac{(1 - x)(p_{10} + p_{11} - 1) + p^\prime_{10}(1 - y) - p_{10}(1 - x) - (p_{11} - (1 - y))(1 - x) + (1 - x)y}{1 - x}\\
    &= \frac{(1 - x)(p_{10} + p_{11} - 1) + p^\prime_{10}(1 - y) -(1 - x)(p_{10} + p_{11} - 1) - x(1 - y)}{1 - x}\\
    &= \frac{p^\prime_{10}(1 - y) - x(1 - y)}{1 - x} = \frac{(1 - y)(p^\prime_{10} - x)}{1 - x}
\end{align*}

So in this case, when $p_{01}x < p^\prime_{01}y$ holds, we get falsification with $\Gamma$ evaluating to
\[
\Gamma = \frac{(1 - y)(p^\prime_{10} - x)}{1 - x}
\]

And so the upper bound for PNS will be
\[
p_{11} - \Gamma = p_{11} - \frac{(1 - y)(p^\prime_{10} - x)}{1 - x}
\] 
\subsubsection{Case IV}

We assume the following conditions
\begin{align}
    \Phi_X < 0\\
    1 - x < x\\
    p^\prime_{11} <1 - x  < x\\
    p^\prime_{10} < 1 - x < x
\end{align}

These constraints imply the following lower and upper bounds on $P(Z = 1 \mid X = 1, Y = 1)$ from (\ref{p_111_bounds}) to
\begin{align*}
    \max\begin{bmatrix}
        0 \\
        \frac{p^\prime_{11}y - p_{10}(1 - x)}{xy}
    \end{bmatrix} \leq P(Z = 1\mid X = 1, Y = 1) \leq 
    \min\begin{bmatrix}
        \frac{p_{11}}{y}\\
        \frac{p^\prime_{11}}{x}
    \end{bmatrix}
\end{align*}

Here, since \ref{a} will always be negative, we only need to check whether the lower bounds will be greater than \ref{b}. 
\begin{enumerate}
    \item Lower bound is $\frac{p^\prime_{11}y - p_{10}(1 - x)}{xy}$: Assume 
    \[
        \frac{p^\prime_{11}y - p_{10}(1 - x)}{xy} > \frac{p^\prime_{11}y - (1 - x)(\Phi_X + y)}{y(x - (1 - x))}
    \]
    \begin{align*}
        &\implies p^\prime_{11}yx - p^\prime_{11}y(1 - x) - p_{10}x(1 - x) + p_{10}(1 - x)^2 > p^\prime_{11}xy - x(1 - x)\Phi_X - xy(1 - x)\\
        &\implies - p^\prime_{11}y - p_{10}x + p_{10}(1 - x) >  - x\Phi_X - xy\\
        &\implies p^\prime_{10}(1 - y) - p_{10}x - p_{11}x + xy >  - x\Phi_X\\
        &\implies p^\prime_{10}(1 - y) -x(p_{10} + p_{11} - 1) - (1 - y)x >  - x\Phi_X\\
        &\implies p^\prime_{10}(1 - y) - (1 - y)x >  0\\
    \end{align*}
    This is a contradiction since this implies $p^\prime_{10} > x$, and so by contradiction
    \[
    \frac{p^\prime_{11}y - p_{10}(1 - x)}{xy} \leq \frac{p^\prime_{11}y - (1 - x)(\Phi_X + y)}{y(x - (1 - x))}
    \]
    \item Lower bound is $0$: It requires this condition to hold
    \[
    \frac{y(p^\prime_{11} - (1 - x))}{1 - x} < \Phi_X
    \]
    The lower bound $0$ will be greater than (b). 
\end{enumerate}

Consequently, when $0$ is the lower bound, which requires the following condition to hold 
\[
p_{10}(1 - x) > p^\prime_{11}y
\]

Then $\Gamma$ will evaluate to
\[
\Phi_X - \frac{y(p^\prime_{11} - (1 - x))}{1 - x}
\]

And the upper bound on PNS will be
\begin{align*}
p_{11} - \Gamma &= p_{11} - \Phi_X + \frac{y(p^\prime_{11} - (1 - x))}{1 - x}\\
&= p_{00} - \frac{y((1 - x) - p^\prime_{11})}{1 - x}
\end{align*}
\subsubsection{Case V}
We assume the following conditions
\begin{align}
    \Phi_X < 0\\
    1 - x < x\\
    p^\prime_{11} <1 - x  < x\\
    1 - x < p^\prime_{10} < x
\end{align}

These constraints imply the following lower bounds on $P(Z = 1 \mid X = 1, Y = 1)$ from (\ref{p_111_bounds}). Only the lower bound is checked against \ref{b} since \ref{a} will be negative in this case. 
\begin{align*}
    \max\begin{bmatrix}
        0 \\
        \frac{p^\prime_{11}y - p_{10}(1 - x)}{xy}
    \end{bmatrix} \leq P(Z = 1\mid X = 1, Y = 1) 
\end{align*}

The same argument as before will apply for $\frac{p^\prime_{11}y - p_{10}(1 - x)}{xy}$ being less than \ref{b}. 

The same condition holds on $0$ as well, so we get the requirement
\[
p_{10}(1 - x) > p^\prime_{11}y
\]

Then, $\Gamma$ will evaluate to
\[
\Phi_X - \frac{y(p^\prime_{11} - (1 - x))}{1 - x}
\]

And so, the upper bound on the PNS 
\begin{align*}
p_{11} - \Gamma &= p_{11} - \Phi_X + \frac{y(p^\prime_{11} - (1 - x))}{1 - x}\\
&= p_{00} - \frac{y((1 - x) - p^\prime_{11})}{1 - x}    
\end{align*}


\subsubsection{Case VI}
We assume the following conditions
\begin{align}
    \Phi_X < 0\\
    1 - x < x\\
    p^\prime_{11} <1 - x  < x\\
    1 - x < x < p^\prime_{10}
\end{align}

Similar to the previous case, only the lower bound needs to be checked. These constraints imply the following lower bounds on $P(Z = 1 \mid X = 1, Y = 1)$ from (\ref{p_111_bounds}) as
\begin{align*}
    max\begin{bmatrix}
        0 \\
        \frac{p_{11} - (1 - y)}{y}
    \end{bmatrix} \leq P(Z = 1\mid X = 1, Y = 1) 
\end{align*}

Now, we check whether each of these lower bounds can be greater than \ref{b}. 
\begin{enumerate}
    \item When lower bound is $\frac{p_{11} - (1 - y)}{y}$: We provide a proof by contradiction. Assume
    \[
        \frac{p_{11} - (1 - y)}{y} < \frac{p^\prime_{11}y - (1 - x)(\Phi_X + y)}{y(x - (1 - x))}
    \]
    \begin{align*}
        &\implies p_{11}x - p_{11}(1 - x) - (1 - y)x + (1 - y)(1 - x) < p^\prime_{11}y - (1 - x)(\Phi_X + y)\\
        &\implies p^\prime_{10}(1 - y) - p_{10}(1 - x) - p_{11}(1 - x) - (1 - y)x + (1 - x) - y(1 - x) < -(1 - x)\Phi_X - (1 - x)y\\
        &\implies p^\prime_{10}(1 - y) - (1 - x)\Phi_X - (1 - y)x  < -(1 - x)\Phi_X \\
        &\implies p^\prime_{10}(1 - y)  - (1 - y)x  < 0\\
        &\implies p^\prime_{10} - x < 0
    \end{align*}
    This is a contradiction since we assume $p^\prime_{10} > x$. So, this lower bound is capable of falsifying.

    \item When the lower bound is $0$: If the following condition holds as before, we get falsification:
    \[
    \frac{y(p^\prime_{11} - (1 - x))}{1 - x} < \Phi_X
    \]
\end{enumerate}

So, the falsification will be as follows. 

When $p_{11} > 1 - y$, $\frac{p_{11} - (1 - y)}{y}$ will be the lower bound, and $\Gamma$ will be evaluating by inserting this lower bound into $yP(Z = 1\mid X = 1, Y = 1)(OR(X) - 1) + \Phi_X + y - \frac{p^\prime_{11}y}{1 - x}$. And $\Gamma$ will evaluate to
\[
\Gamma = \frac{(1 - y)(p^\prime_{10} - x)}{1 - x}
\]

And therefore the upper bound on PNS will be
\begin{align*}
    p_{11} - \Gamma = p_{11} - \frac{(1 - y)(p^\prime_{10} - x)}{1 - x}
\end{align*}

Next, when $p_{11} < 1 - y$, $0$ will be the lower bound, and $\Gamma$ will evaluate to 
\[
\Gamma = \Phi_X - \frac{y(p^\prime_{11} - (1 - x))}{1 - x}
\]

And the upper bound on PNS will be
\begin{align*}
    p_{11} - \Gamma = p_{00} - \frac{y((1 - x) - p^\prime_{11})}{1 - x}
\end{align*}

\subsubsection{Case VII: Atalanti}
We assume the following conditions
\begin{align}
    \Phi_X < 0\\
    1 - x < x\\
    1 - x  < x < p^\prime_{11}\\
    p^\prime_{10} < 1 - x < x
\end{align}

These constraints imply based on (\ref{p_111_bounds}) and the implications on Subsection \ref{implications_bounds_p111}, the following lower and upper bounds on $P(Z = 1 \mid X = 1, Y = 1)$: 
\begin{align*}
    \max\begin{bmatrix}
        \frac{p^\prime_{11}-(1-x)}{x} \\
        \frac{p^\prime_{11}y-p_{10}(1-x)}{xy}
    \end{bmatrix} \leq P(Z = 1\mid X = 1, Y = 1) \leq 
    \min\begin{bmatrix}
        1\\
        \frac{p_{11}}{y}
    \end{bmatrix}
\end{align*}
Now we will check if each of the possible lower bounds are greater than $b =\frac{(1 - x)(p^\prime_{11}y - \Phi_X - y)}{y(x - (1 - x))}$ (\ref{b}).
\begin{enumerate}
    \item \[\frac{p^\prime_{11}-(1-x)}{x} > \frac{(1 - x)(p^\prime_{11}y - \Phi_X - y)}{y(x - (1 - x))} \]. This is a contradiction because we see that $\frac{p^\prime_{11}-(1-x)}{x}< \frac{p^\prime_{11}-(1-x)}{x - (1-x) } = a $. Which implies that $\frac{p^\prime_{11}-(1-x)}{x}< b$.  
    \item \[\frac{p^\prime_{11}y-p_{10}(1-x)}{xy} > \frac{(1 - x)(p^\prime_{11}y - \Phi_X - y)}{y(x - (1 - x))} \]. Checking the right hand side of the implication
\begin{align*}
    &\implies p^\prime_{11}y(x - (1 - x)) - p_{10}(1 - x)(x - (1 - x)) > p^\prime_{11}xy - x(1 - x)(p_{11} + p_{10} - 1) -xy(1 - x)\\
    &\implies -p^\prime_{11}y - p_{10}(x - (1 - x)) >  - x(p_{11} + p_{10} - 1) -xy\\
    &\implies -p^\prime_{11}y + p_{10}(1 - x) - p_{10}x  >  - xp_{11} - xp_{10} + x -xy\\
    &\implies -p^\prime_{11}y + p_{10}(1 - x) + xp_{11}  >  x(1 - y)\\
    &\implies p^\prime_{10}(1 - y) > x(1 - y) \implies p^\prime_{10} > x
\end{align*}
This leads to a contradiction of our case assumption $p^\prime_{10} < x$.
\end{enumerate}

Now we will check if each of the possible upper bounds are less than $a = \frac{p^\prime_{11} - (1 - x)}{x - (1 - x)}$ (\ref{a}). 
NOTE: Unsure whether the argument for $1$ holds since \ref{a} doesn't need to be a probability. 
\begin{enumerate}
    \item \begin{align*}
        1 > \frac{p^\prime_{11} - (1 - x)}{x - (1 - x)}\\
        \implies x - (1 - x) > p^\prime_{11} - (1 - x)\\
        \implies x > p^\prime_{11}
            \end{align*}
        This is a contradiction based on our assumption, so $1$ is capable of falsifying. 
    \item Checking if $\frac{p_{11}}{y} < \frac{p^\prime_{11} - (1 - x)}{x - (1 - x)}$.
    \begin{align*}
    \frac{p_{11}}{y} < \frac{p^\prime_{11} - (1 - x)}{x - (1 - x)}
    \implies p_{11}x - p_{11}(1 - x) < p^\prime_{11}y - y(1 - x)\\
    \implies p_{11}x - p_{11}(1 - x) < p_{11}x + p_{10}(1 - x) - p^\prime_{10}(1 - y) - y(1 - x)\\
    \implies - p_{11}(1 - x) < p_{10}(1 - x) - p^\prime_{10}(1 - y) - y(1 - x)\\
    \implies p^\prime_{10}(1 - y)  < p_{10}(1 - x) + p_{11}(1 - x)  - y(1 - x)\\
    \implies p^\prime_{10}(1 - y)  < (1 - x)(p_{10} + p_{11}  - (1 - (1 - y)))\\
    \implies p^\prime_{10}(1 - y)  < (1 - x)(p_{10} + p_{11}  - 1) + (1 - x)(1 - y)\\
    \implies \frac{(1 - y)(p^\prime_{10} - (1 - x))}{1 - x}  < \Phi_X\\
    \end{align*}
    So, when $\frac{(1 - y)(p^\prime_{10} - (1 - x))}{1 - x}  < \Phi_X$, $\frac{p_{11}}{y}$ will be less than $a$ and we can get falsification.
\end{enumerate}
%Since $a$ is a probability, $1$ cannot be an upper bound of $P(Z = 1\mid X = 1, Y = 1)$. 

% So we only need to check if $\frac{p_{11}}{y} < \frac{p^\prime_{11} - (1 - x)}{x - (1 - x)}$.
%     \begin{align*}
%     \frac{p_{11}}{y} < \frac{p^\prime_{11} - (1 - x)}{x - (1 - x)}
%     \implies p_{11}x - p_{11}(1 - x) < p^\prime_{11}y - y(1 - x)\\
%     \implies p_{11}x - p_{11}(1 - x) < p_{11}x + p_{10}(1 - x) - p^\prime_{10}(1 - y) - y(1 - x)\\
%     \implies - p_{11}(1 - x) < p_{10}(1 - x) - p^\prime_{10}(1 - y) - y(1 - x)\\
%     \implies p^\prime_{10}(1 - y)  < p_{10}(1 - x) + p_{11}(1 - x)  - y(1 - x)\\
%     \implies p^\prime_{10}(1 - y)  < (1 - x)(p_{10} + p_{11}  - (1 - (1 - y)))\\
%     \implies p^\prime_{10}(1 - y)  < (1 - x)(p_{10} + p_{11}  - 1) + (1 - x)(1 - y)\\
%     \implies \frac{(1 - y)(p^\prime_{10} - (1 - x))}{1 - x}  < \Phi_X\\
%     \end{align*}
%     So, when $\frac{(1 - y)(p^\prime_{10} - (1 - x))}{1 - x}  < \Phi_X$, $\frac{p_{11}}{y}$ will be less than $a$ and we can get falsification.

Now, for each of these settings, we evaluate $\Gamma$ and PNS.
\begin{enumerate}
    \item Upper bound is $1$:
    \begin{align*}
        \Gamma &= (1 - OR(X))y + y\frac{p^\prime_{11} - (1 - x)}{1 - x}\\
        &= y - \frac{xy}{1 - x} + \frac{yp^\prime_{11} - y(1 - x)}{1 - x}\\
        &= \frac{y(p^\prime_{11} - x)}{1 - x}
    \end{align*}
    And the PNS upper bound will be
    \begin{align*}
        p_{11} - \Gamma &= p_{11} - \Gamma\\
        \implies  &= p_{11} - \frac{y(p^\prime_{11} - x)}{1 - x}
    \end{align*}
    \item Upper bound is $\frac{p_{11}}{y}$: Then
    \begin{align*}
        \Gamma &= p_{11}(1 - OR(X)) + y\frac{p^\prime_{11} - (1 - x)}{1 - x}\\
        &= p_{11} + \frac{p^\prime_{11}y - p_{11}x - y(1 - x)}{1 - x}\\
        &= p_{11} + \frac{p_{10}(1 - x) - p^\prime_{10}(1 - y) - y(1 - x)}{1 - x}\\
        &= p_{11} + \frac{p_{10}(1 - x) - p^\prime_{10}(1 - y) - (1 - (1 - y))(1 - x)}{1 - x}\\
        &= p_{11} + p_{10} - 1 + \frac{ - p^\prime_{10}(1 - y) + (1 - y)(1 - x)}{1 - x}\\
        &= \Phi_X - \frac{(1 - y)(p^\prime_{10} - (1 - x))}{1 - x}
    \end{align*}
    And the upper bound on PNS will evaluate to
    \begin{align*}
        p_{11} - \Gamma = p_{00} - \frac{(1 - y)((1 - x) - p^\prime_{10})}{1 - x}
    \end{align*}
\end{enumerate}

\subsubsection{Case VIII: Atalanti}
We assume the following conditions
\begin{align}
    p_{11} + p_{10} - 1 < 0\\
    1 - x < x\\
    1 - x  < x < p^\prime_{11}\\
    1 - x < p^\prime_{10} < x
\end{align}

These constraints imply based on (\ref{p_111_bounds}) and the implications on Subsection \ref{implications_bounds_p111}, the following lower and upper bounds on $P(Z = 1 \mid X = 1, Y = 1)$: 
\begin{align*}
    \max\begin{bmatrix}
        \frac{p^\prime_{11}-(1-x)}{x} \\
        \frac{p^\prime_{11}y-p_{10}(1-x)}{xy}
    \end{bmatrix} \leq P(Z = 1\mid X = 1, Y = 1) \leq 
    \min\begin{bmatrix}
        1\\
        \frac{(1-x)(1-y) - p_{10}(1-x) + p^\prime_{11}y}{xy}
    \end{bmatrix}
\end{align*}
Now we will check if each of the possible lower bounds are greater than $b =\frac{p^\prime_{11}y - (1 - x)(\Phi_X + y)}{y(x - (1 - x))}$ (\ref{b}).
\begin{enumerate}
    \item \[\frac{p^\prime_{11}-(1-x)}{x} > \frac{p^\prime_{11}y -(1 - x)(\Phi_X + y)}{y(x - (1 - x))} \]. This is a contradiction because we see that $\frac{p^\prime_{11}-(1-x)}{x}< \frac{p^\prime_{11}-(1-x)}{x - (1-x)}= a $. Which implies that $\frac{p^\prime_{11}-(1-x)}{x}< b$.  
    \item \[\frac{p^\prime_{11}y-p_{10}(1-x)}{xy} > \frac{p^\prime_{11}y -(1 - x)(\Phi_X + y)}{y(x - (1 - x))} \]. Checking the right hand side of the implication
\begin{align*}
    &\implies p^\prime_{11}y(x - (1 - x)) - p_{10}(1 - x)(x - (1 - x)) > p^\prime_{11}xy - x(1 - x)(p_{11} + p_{10} - 1) -xy(1 - x)\\
    &\implies -p^\prime_{11}y - p_{10}(x - (1 - x)) >  - x(p_{11} + p_{10} - 1) -xy\\
    &\implies -p^\prime_{11}y + p_{10}(1 - x) - p_{10}x  >  - xp_{11} - xp_{10} + x -xy\\
    &\implies -p^\prime_{11}y + p_{10}(1 - x) + xp_{11}  >  x(1 - y)\\
    &\implies p^\prime_{10}(1 - y) > x(1 - y) \implies p^\prime_{10} > x
\end{align*}
This leads to a contradiction of our case assumption $p^\prime_{10} < x$.\end{enumerate}
Next, we  check if each of the possible upper bounds are less than $a = \frac{p^\prime_{11} - (1 - x)}{x - (1 - x)}$ (\ref{a}). 
\begin{enumerate}
    \item 
    \[
        \frac{p^\prime_{11} - (1 - x)}{x - (1 - x)} < 1
    \]
    \begin{align*}
        \implies p^\prime_{11} < x
    \end{align*}
    This is a contradiction, and so $1 \leq (a)$.
    \item Checking 
    \[
    \frac{(1-x)(1-y) - p_{10}(1-x) + p^\prime_{11}y}{xy} < \frac{p^\prime_{11} - (1 - x)}{x - (1 - x)}
    \]
    
    \begin{align*}
    \implies (1 - y)(p^\prime_{10} - (1 - x)) < x\Phi_X
    \end{align*}
    This is a contradiction since the RHS is negative, but the LHS in positive.
\end{enumerate}

So, when $1 < \frac{(1-x)(1-y) - p_{10}(1-x) + p^\prime_{11}y}{xy}$, then $\Gamma$ will be evaluated by subsititung $1$ as the value for $P(Z = 1 \mid X = 1, Y = 1)$ into $P(Z = 1 \mid X = 1, Y = 1)(1 - OR(X))y + y\frac{p^\prime_{11} - (1 - x)}{1 - x}$, to get
\begin{align*}
    \Gamma &= (1 - OR(X))y + y\frac{p^\prime_{11} - (1 - x)}{1 - x}\\
    &= \frac{y(p^\prime_{11} - x)}{1 - x}
\end{align*}

And the upper bound on PNS will be
\begin{align*}
    p_{11} - \Gamma = p_{11} - \frac{y(p^\prime_{11} - x)}{1 - x}
\end{align*}

\subsubsection{Case IX: Atalanti}
We assume the following conditions
\begin{align}
    \Phi_X < 0\\
    1 - x < x\\
    1 - x  < x < p^\prime_{11}\\
    1 - x < x < p^\prime_{10}
\end{align}

These constraints imply based on (\ref{p_111_bounds}) and the implications on Subsection \ref{implications_bounds_p111}, the following lower and upper bounds on $P(Z = 1 \mid X = 1, Y = 1)$: 
\begin{align*}
    \max\begin{bmatrix}
        \frac{p^\prime_{11}-(1-x)}{x} \\
        \frac{p_{11}-(1-y)}{y}
    \end{bmatrix} \leq P(Z = 1\mid X = 1, Y = 1) \leq 
    \min\begin{bmatrix}
        1\\
        \frac{(1-x)(1-y) - p_{10}(1-x) + p^\prime_{11}y}{xy}
    \end{bmatrix}
\end{align*}
Now we will check if each of the possible lower bounds are greater than $b =\frac{p^\prime_{11}y - (1 - x)(\Phi_X + y)}{y(x - (1 - x))}$ (\ref{b}).
\begin{enumerate}
    \item \[\frac{p^\prime_{11}-(1-x)}{x} > \frac{p^\prime_{11}y - (1 - x)(\Phi_X + y)}{y(x - (1 - x))} \]. This is a contradiction because we see that $\frac{p^\prime_{11}-(1-x)}{x}< \frac{p^\prime_{11}-(1-x)}{x - (1-x)}= a $. Which implies that $\frac{p^\prime_{11}-(1-x)}{x}< b$.  
    \item \begin{align*}&\frac{p_{11}-(1-y)}{y} > \frac{p^\prime_{11}y -(1 - x)(\Phi_X + y)}{y(x - (1 - x))}\\ 
    &\implies (p_{11}-(1-y))(x - (1 - x)) > p^\prime_{11}y -(1 - x)(\Phi_X + y)\\
    &\implies p_{11}x - p_{11}(1 - x) - (1 - y)x + (1 - y)(1 - x) > p^\prime_{11}y - (1 - x)(\Phi_X + y)\\
    &\implies p^\prime_{10}(1 - y) - p_{10}(1 - x) - p_{11}(1 - x) - (1 - y)x + (1 - x) - y(1 - x) > -(1 - x)\Phi_X - (1 - x)y\\
    &\implies p^\prime_{10}(1 - y) - (1 - x)\Phi_X - (1 - y)x  > -(1 - x)\Phi_X \\
    &\implies p^\prime_{10}(1 - y)  - (1 - y)x  > 0\\
    &\implies p^\prime_{10} - x > 0
    \end{align*}
    Which agrees with our assumption $p^\prime_{10} > x$. So, this lower bound is capable of falsifying, since the opposite of this inequality would create a contradiction. So,
    \[
        \frac{p_{11}-(1-y)}{y} \geq \frac{p^\prime_{11}y -(1 - x)(\Phi_X + y)}{y(x - (1 - x))}
    \]
\end{enumerate}
Now we will check if each of the possible upper bounds are less than $a = \frac{p^\prime_{11} - (1 - x)}{x - (1 - x)}$ (\ref{a}). 
\begin{enumerate}
    \item 
    \[
        \frac{p^\prime_{11} - (1 - x)}{x - (1 - x)} < 1
    \]
    \begin{align*}
        \implies p^\prime_{11} < x
    \end{align*}
    This is a contradiction, and so $1 \leq (a)$.
    \item  
    \[\frac{(1-x)(1-y) - p_{10}(1-x) + p^\prime_{11}y}{xy} < \frac{p^\prime_{11} - (1 - x)}{x - (1 - x)}
    \]
    \begin{align*}
        \implies (1 - y)(p^\prime_{10} - (1 - x)) < x\Phi_X
    \end{align*}
    This is a contradiction since the RHS is negative, but the LHS in positive.
\end{enumerate}

So, when $1$ is the upper bound, the upper bound on PNS will be
\begin{align*}
    p_{11} - \Gamma = p_{11} - \frac{y(p^\prime_{11} - x)}{1 - x}
\end{align*}

And when $\frac{p_{11} - (1- y)}{y}$ is the lower bound, $\Gamma$ will evaluate to
\begin{align*}
    \Gamma &= (p_{11} - (1 - y))(OR(X) - 1) + \Phi_X + y - \frac{p^\prime_{11}y}{1 - x} \\
    &= \frac{(1 - y)(p^\prime_{10} - x)}{1 - x} 
\end{align*}

And the upper bound on PNS will be
\[
p_{11} - \Gamma = p_{11} - \frac{(1 - y)(p^\prime_{10} - x)}{1 - x} 
\]
\subsection{When $1 - x > x$}

Here, since the $OR(X)$ will be less than $1$, we need to recompute the turning points, which we do now. 
\begin{align*}
&yP(Z = 1\mid X = 1, Y = 1)(OR(X) - 1) + \Phi_X + y - \frac{p^\prime_{11}y}{1 - x} \geq 0\\    
&\implies \Phi_X + y - \frac{p^\prime_{11}y}{1 - x} \geq yP(Z = 1\mid X = 1, Y = 1)(OR(X) - 1)\\
&\implies \frac{(1 - x)(\Phi_X + y) - p^\prime_{11}y}{1 - x} \geq \frac{yP(Z = 1\mid X = 1, Y = 1)((1 - x) - x)}{1 - x}\\
&\implies \frac{(1 - x)(\Phi_X + y) - p^\prime_{11}y}{y((1 - x) - x)} \geq P(Z = 1\mid X = 1, Y = 1)
\end{align*}

 We denote as (a). Next,            

\begin{align*}
    &P(Z = 1 \mid X = 1, Y = 1)(1 - OR(X))y + y\frac{p^\prime_{11} - (1 - x)}{1 - x} \geq 0\\
    &\implies P(Z = 1 \mid X = 1, Y = 1)(1 - OR(X)) + \frac{p^\prime_{11} - (1 - x)}{1 - x} \geq 0\\
    &\implies P(Z = 1 \mid X = 1, Y = 1)(1 - OR(X)) \geq \frac{(1 - x) - p^\prime_{11}}{1 - x}\\
    &\implies P(Z = 1 \mid X = 1, Y = 1) \geq \frac{(1 - x) - p^\prime_{11}}{(1 - x) - x}\\
\end{align*}
             
And we denote this as (b). Now, we enumerate cases in a similar fashion as before. 


\subsubsection{Case I}

This case assumes the following
\begin{align}
    \Phi_X < 0\\
    x < 1 - x\\
    x < p^\prime_{11} < 1 - x\\
    p^\prime_{10} < x <  1- x
\end{align}

Here, the chosen bounds will be
\begin{align*}
    \max \begin{bmatrix}
        0\\
        \frac{p^\prime_{11}y - p_{10}(1 - x)}{xy}
    \end{bmatrix} \leq PNS \leq 
    \min \begin{bmatrix}
    1 \\
    \frac{p_{11}}{y}
    \end{bmatrix}
\end{align*}

Now, we check the upper and lower bounds against (a) and (b). 
\begin{enumerate}
    \item Lower bound is $0$: $0$ will be less than (b) since we assume $p^\prime_{11} < 1 - x$. 
    \item Lower bound is $\frac{p^\prime_{11}y - p_{10}(1 - x)}{xy}$: This will be less than (b) when the following condition holds:
    \[
    \Phi_X < \frac{(1 - y)(p^\prime_{10} - x)}{x}
    \]
\end{enumerate}

Next, checking the upper bounds
\begin{enumerate}
    \item Upper bound of $1$: Checking this against (a), using a proof by contradiction. Assume
    \[
    \frac{(1 - x)(\Phi_X + y) - p^\prime_{11}y}{y((1 - x) - x)} > 1
    \]
    \begin{align*}
        (1 - x)(\Phi_X + y) - p^\prime_{11}y > y((1 - x) - x)\\
        \implies (1 - x)(\Phi_X + y) - p^\prime_{11}y > y(1 - x) - xy\\
        \implies (1 - x)y + (1 - x)\Phi_X - p^\prime_{11}y > y(1 - x) - xy\\
        \implies (1 - x)\Phi_X  > y(p^\prime_{11} - x)\\
    \end{align*}
    This is a contradiction since LHS is negative and RHS is positive. 
    \item Upper bound is $\frac{p_{11}}{y}$: Following proof by contradiction, assume
    \[
    \frac{p_{11}}{y} < \frac{(1 - x)(\Phi_X + y) - p^\prime_{11}y}{y((1 - x) - x)}
    \]
    \begin{align*}
        \implies p_{11}(1 - x) - p_{11}x < (1 - x)\Phi_X + y(1 - x) - p^\prime_{11}y\\
        \implies (1 - x)\Phi_X - p^\prime_{10}(1 - y) < (1 - x)\Phi_X - (1 - y)(1 - x)\\
        \implies 0 < (1 - y)(p^\prime_{10} - (1 - x))
    \end{align*}
    This is a contradiction based on our assumptions.
\end{enumerate}
So, when $\frac{p^\prime_{11}y - p_{10}(1 - x)}{xy}$ is the lower bound, i.e. $p^\prime_{11}y > p_{10}(1 - x)$ and $\Phi_X > \frac{(1 - y)(p^\prime_{10} - x)}{x}$, we compute $\Gamma$ by inserting this lower bound into increasing function $P(Z = 1 \mid X = 1, Y = 1)(1 - OR(X))y + y\frac{p^\prime_{11} - (1 - x)}{1 - x}$. 
\begin{align*}
    \Gamma &=\frac{p^\prime_{11}y - p_{10}(1 - x)}{x}(1 - OR(X)) + y\frac{p^\prime_{11} - (1 - x)}{1 - x} \\
    \Gamma &= \Phi_X - \frac{(1 - y)(p^\prime_{10} - x)}{x}
\end{align*}

And the upper bound on PNS is computed as
\begin{align*}
    p_{11} - \Gamma &= p_{11} - \Phi_X + \frac{(1 - y)(p^\prime_{10} - x)}{x}\\
    &= p_{00} - \frac{(1 - y)(x - p^\prime_{10})}{x}\\
\end{align*}
\subsubsection{Case II}

\begin{align}
    p_{10} + p_{10} - 1 < 0\\
    x < 1 - x\\
    x < p^\prime_{11} < 1 - x\\
    x < p^\prime_{10} <  1- x
\end{align}

Here, the chosen bounds will be
\begin{align*}
    \max \begin{bmatrix}
        0\\
        \frac{p_{11} - (1 - y)}{y}
    \end{bmatrix} \leq PNS \leq 
    \min \begin{bmatrix}
    1 \\
    \frac{p_{11}}{y}
    \end{bmatrix}
\end{align*}

Checking whether the lower bounds will be greater than (b) first. 
\begin{enumerate}
    \item Lower bound of $0$: $0$ will be less than (b) since $p^\prime_{11} < 1 - x$.
    \item Lower bound of $\frac{p_{11} - (1 - y)}{y}$: Following a proof by contradiction, assume
    \[
    \frac{p_{11} - (1 - y)}{y} > \frac{(1 - x) - p^\prime_{11}}{(1 - x) - x}
    \]
    \begin{align*}
        \implies (1 - x)\Phi_X > (1 - y)(p^\prime_{10} - x)
    \end{align*}
    Contradiction because LHS is negative and RHS is positive
\end{enumerate}

Now, for the upper bound $1$ will not be less than (a) using the same argument as above. Similarly, $\frac{p_{11}}{y}$ will not be less than (a) either.

So no falsification will be observed in this case. 

\subsubsection{Case III}

\begin{align}
    \Phi_X < 0\\
    x < 1 - x\\
    x < p^\prime_{11} < 1 - x\\
    x <  1- x < p^\prime_{10}
\end{align}

Here, the chosen bounds will be
\begin{align*}
    \max \begin{bmatrix}
        0\\
        \frac{p_{11} - (1 - y)}{y}
    \end{bmatrix} \leq PNS \leq 
    \min \begin{bmatrix}
    1 \\
    \frac{(1 - x)(1 - y) - p_{10}(1 - x) + p^\prime_{11}y}{xy}
    \end{bmatrix}
\end{align*}

Checking whether the lower bounds will be greater than (b). 
\begin{enumerate}
    \item Lower bound on $0$: Using arguments before, this will be less than (b).
    \item Lower bound of $\frac{p_{11} - (1 - y)}{y}$: This generates a contradiction as before.
\end{enumerate}

So, neither of the lower bounds are capable of falsifying. Next, we move on to the upper bounds.

\begin{enumerate}
    \item Upper bound of $1$: Using the argument from Case I, we know this will be greater than (a).
    \item: Upper bound of $\frac{(1 - x)(1 - y) - p_{10}(1 - x) + p^\prime_{11}y}{xy}$: Following a proof by contradiction: Assume
    \[
    \frac{(1 - x)(\Phi_X + y) - p^\prime_{11}y}{y((1 - x) - x)} < \frac{(1 - x)(1 - y) - p_{10}(1 - x) + p^\prime_{11}y}{xy}
    \]
    \begin{align*}
        &\implies \frac{(1 - x)(\Phi_X + y) - p^\prime_{11}y}{(1 - x) - x} < \frac{(1 - x)(1 - y) - p_{10}(1 - x) + p^\prime_{11}y}{x}\\
        &\implies (1 - y)(p^\prime_{10} - (1 - x)) < 0
    \end{align*}
    This is a contradiction, so 
    \[
    \frac{(1 - x)(\Phi_X + y) - p^\prime_{11}y}{y((1 - x) - x)} \geq \frac{(1 - x)(1 - y) - p_{10}(1 - x) + p^\prime_{11}y}{xy}
    \]
\end{enumerate}

Now, this will create a contradiction. So when this is the upper bound, i.e. this condition holds
\begin{align*}
    p^\prime_{01}y > p_{00}(1 - x)    
\end{align*}
Then we can insert $\frac{(1 - x)(1 - y) - p_{10}(1 - x) + p^\prime_{11}y}{xy}$ into $P(Z = 1 \mid X = 1, Y = 1)y(OR(X) - 1) + \Phi_X + y - \frac{p^\prime_{11}y}{1 - x}$. to evaluate $\Gamma$ as 
\[
\Gamma = \frac{(1 - y)(p^\prime_{10} - (1 - x))}{x}
\]

And this gives the following upper bound on PNS as
\begin{align*}
    p_{11} - \Gamma = p_{11} - \frac{(1 - y)(p^\prime_{10} - (1 - x))}{x}
\end{align*}
\subsubsection{Case IV: Atalanti}

\begin{align}
    \Phi_X < 0\\
    x < 1 - x\\
    p^\prime_{11} < x <  1 - x\\
    x <  1- x < p^\prime_{10}
\end{align}
These constraints imply based on (\ref{p_111_bounds}) and the implications on Subsection \ref{implications_bounds_p111}, the following lower and upper bounds on $P(Z = 1 \mid X = 1, Y = 1)$: 
\begin{align*}
    max\begin{bmatrix}
        0\\
        \frac{p_{11}-(1-y)}{y}
    \end{bmatrix} \leq P(Z = 1\mid X = 1, Y = 1) \leq 
    min\begin{bmatrix}
        \frac{p^\prime_{11}}{x}\\
        \frac{(1-x)(1-y) - p_{10}(1-x) + p^\prime_{11}y}{xy}
    \end{bmatrix}
\end{align*}

Now we will check if each of the possible lower bounds are greater than $b =\frac{(1 - x) - p^\prime_{11}}{(1 - x) - x}$.
\begin{enumerate}
    \item $0 < b$ holds since $1 - x > p^\prime_{11}$ by assumption. 
    \item 
    \begin{align*}
        &\frac{p_{11}-(1-y)}{y} > \frac{(1 - x) - p^\prime_{11}}{(1 - x) - x}\\ 
        &\implies \Phi_X > \frac{(1 - y)(p^\prime_{10} - x)}{1 - x}
    \end{align*}
    This is contradiction since LHS is negative but RHS is positive.
\end{enumerate}
Now we will check if each of the possible upper bounds are less than $a = \frac{p^\prime_{11} - (1 - x)}{x - (1 - x)}$. 
\begin{enumerate}
    \item Upper bound is $\frac{p^\prime_{11}}{x}$: 
    \begin{align*}
        \frac{p^\prime_{11}}{x} < \frac{(1 - x)(\Phi_X + y) - p^\prime_{11}y}{y((1 - x) - x)}\\
        \implies \frac{y(p^\prime_{11} - x)}{x} < \Phi_X
    \end{align*}
    So, when the above holds, the upper bound will be capable of falsifying. 
    \item $\frac{(1-x)(1-y) - p_{10}(1-x) + p^\prime_{11}y}{xy} < \frac{(1 - x)(\Phi_X + y) - p^\prime_{11}y}{y((1 - x) - x)}$.
    \begin{align*}
        \implies 0 < (1 - y)(p^\prime_{10} - (1 - x))
    \end{align*}
    This bound is capable of falsifying as well. 
\end{enumerate}

So now, $\Gamma$ will be evaluated for different values of upper bounds. When the upper bound is $\frac{p^\prime_{11}}{x}$, $\Gamma$ is evaluated as
\begin{align*}
    \Gamma &= \frac{p^\prime_{11}y}{x}(OR(X) - 1) + \Phi_X + y - \frac{p^\prime_{11}y}{1 - x}\\
    &= \Phi_X - \frac{y(p^\prime_{11} - x)}{x}\\
\end{align*}

And the upper bound on PNS is evaluated as
\begin{align*}
    p_{11} - \Gamma &= p_{11} - \Phi_X + \frac{y(p^\prime_{11} - x)}{x}\\
    p_{11} - \Gamma &= p_{00} - \frac{y(p^\prime_{11} - x)}{x}\\
\end{align*}
When the upper bound is $\frac{(1-x)(1-y) - p_{10}(1-x) + p^\prime_{11}y}{xy}$, $\Gamma$ is evaluated as
\[
\Gamma = \frac{(1 - y)(p^\prime_{10} - (1 - x))}{x}
\]

And this gives the following upper bound on PNS as
\begin{align*}
    p_{11} - \Gamma = p_{11} - \frac{(1 - y)(p^\prime_{10} - (1 - x))}{x}
\end{align*}

\subsubsection{Case V: Atalanti}

\begin{align}
    \Phi_X < 0\\
    x < 1 - x\\
    p^\prime_{11} < x <  1 - x\\
    x < p^\prime_{10} < 1- x 
\end{align}
These constraints imply based on (\ref{p_111_bounds}) and the implications on Subsection \ref{implications_bounds_p111}, the following lower and upper bounds on $P(Z = 1 \mid X = 1, Y = 1)$: 
\begin{align*}
    \max\begin{bmatrix}
        0\\
        \frac{p_{11}-(1-y)}{y}
    \end{bmatrix} \leq P(Z = 1\mid X = 1, Y = 1) \leq 
    \min\begin{bmatrix}
    \frac{p_{11}}{y}\\
        \frac{p^\prime_{11}}{x}
    \end{bmatrix}
\end{align*}
Now we will check if each of the possible lower bounds are greater than $b$.
\begin{enumerate}
    \item $0 < b$ holds since $1 - x > p^\prime_{11}$ by assumption. 
    \item Lower bound is $\frac{p_{11} - (1 - y)}{y}$:
    \begin{align*}
        &\frac{p_{11}-(1-y)}{y} > \frac{(1 - x) - p^\prime_{11}}{(1 - x) - x}\\ 
        &\implies \Phi_X > \frac{(1 - y)(p^\prime_{10} - x)}{1 - x}
    \end{align*}
    This is contradiction since LHS is negative but RHS is positive.
\end{enumerate}

Now we will check if each of the possible upper bounds are less than $a$. 
\begin{enumerate}
    \item Upper bound is $\frac{p_{11}}{y}$: 
    Following proof by contradiction, assume
    \[
    \frac{p_{11}}{y} < \frac{(1 - x)(\Phi_X + y) - p^\prime_{11}y}{y((1 - x) - x)}
    \]
    \begin{align*}
        \implies p_{11}(1 - x) - p_{11}x < (1 - x)\Phi_X + y(1 - x) - p^\prime_{11}y\\
        \implies (1 - x)\Phi_X - p^\prime_{10}(1 - y) < (1 - x)\Phi_X - (1 - y)(1 - x)\\
        \implies 0 < (1 - y)(p^\prime_{10} - (1 - x))
    \end{align*}
    This is a contradiction.
    \item Upper bound is $\frac{p^\prime_{11}}{x}$: 
    \begin{align*}
        \frac{p^\prime_{11}}{x} < \frac{(1 - x)(\Phi_X + y) - p^\prime_{11}y}{y((1 - x) - x)}\\
        \implies \frac{y(p^\prime_{11} - x)}{x} < \Phi_X
    \end{align*}
    So, when the above holds, the upper bound will be capable of falsifying.
\end{enumerate}

When the upper bound is $\frac{p^\prime_{11}}{x}$, $\Gamma$ will evaluate to
\[
    \Gamma = \Phi_X - \frac{y(p^\prime_{11} - x)}{x}
\]

And the upper bound on PNS is evaluated as
\begin{align*}
    p_{11} - \Gamma &= p_{11} - \Phi_X + \frac{y(p^\prime_{11} - x)}{x}\\
    p_{11} - \Gamma &= p_{00} - \frac{y(p^\prime_{11} - x)}{x}\\
\end{align*}

\subsubsection{Case VI: Atalanti}

\begin{align}
    \Phi_X < 0\\
    x < 1 - x\\
    p^\prime_{11} < x <  1 - x\\
    p^\prime_{10} < x < 1- x 
\end{align}

These constraints imply based on (\ref{p_111_bounds}) and the implications on Subsection \ref{implications_bounds_p111}, the following lower and upper bounds on $P(Z = 1 \mid X = 1, Y = 1)$: 
\begin{align*}
    max\begin{bmatrix}
        0\\
        \frac{p^\prime_{11}y-p_{10}(1-x)}{xy}
    \end{bmatrix} \leq P(Z = 1\mid X = 1, Y = 1) \leq 
    min\begin{bmatrix}
    \frac{p_{11}}{y}\\
        \frac{p^\prime_{11}}{x}
    \end{bmatrix}
\end{align*}

Now we will check if each of the possible lower bounds are greater than $b$.
\begin{enumerate}
    \item $0 < b$ holds since $1 - x > p^\prime_{11}$ by assumption. 
    \item 
    \[\frac{p^\prime_{11}y-p_{10}(1-x)}{xy} > \frac{(1 - x) - p^\prime_{11}}{(1 - x) - x}\]
\begin{align*}
    \implies x\Phi_X > (1 - y)(p^\prime_{10} - x)
\end{align*}
When this condition holds, this lower bound can falsify. 
\end{enumerate}

Now we will check if each of the possible upper bounds are less than $a$. 
\begin{enumerate}
    \item Upper bound is $\frac{p_{11}}{y}$: 
    Following proof by contradiction, assume
    \[
    \frac{p_{11}}{y} < \frac{(1 - x)(\Phi_X + y) - p^\prime_{11}y}{y((1 - x) - x)}
    \]
    \begin{align*}
        \implies p_{11}(1 - x) - p_{11}x < (1 - x)\Phi_X + y(1 - x) - p^\prime_{11}y\\
        \implies (1 - x)\Phi_X - p^\prime_{10}(1 - y) < (1 - x)\Phi_X - (1 - y)(1 - x)\\
        \implies 0 < (1 - y)(p^\prime_{10} - (1 - x))
    \end{align*}
    This is a contradiction.
    \item Upper bound is $\frac{p^\prime_{11}}{x}$: 
    \begin{align*}
        \frac{p^\prime_{11}}{x} < \frac{(1 - x)(\Phi_X + y) - p^\prime_{11}y}{y((1 - x) - x)}\\
        \implies \frac{y(p^\prime_{11} - x)}{x} < \Phi_X
    \end{align*}
    So, when the above holds, the upper bound will be capable of falsifying.
\end{enumerate}

So, when $\frac{p^\prime_{11}y - p_{10}(1 - x)}{xy}$ is the lower bound, i.e. $p^\prime_{11}y > p_{10}(1 - x)$ and $\Phi_X > \frac{(1 - y)(p^\prime_{10} - x)}{x}$, we compute $\Gamma$ by inserting this lower bound into increasing function $P(Z = 1 \mid X = 1, Y = 1)(1 - OR(X))y + y\frac{p^\prime_{11} - (1 - x)}{1 - x}$. 
\begin{align*}
    \Gamma &=\frac{p^\prime_{11}y - p_{10}(1 - x)}{x}(1 - OR(X)) + y\frac{p^\prime_{11} - (1 - x)}{1 - x} \\
    \Gamma &= \Phi_X - \frac{(1 - y)(p^\prime_{10} - x)}{x}
\end{align*}

And the upper bound on PNS is computed as
\begin{align*}
    p_{11} - \Gamma &= p_{11} - \Phi_X + \frac{(1 - y)(p^\prime_{10} - x)}{x}\\
    &= p_{00} - \frac{(1 - y)(x - p^\prime_{10})}{x}\\
\end{align*}

And when $\frac{p^\prime_{11}}{x}$ is the upper bound, $\Gamma$ will evaluate to
\[
    \Gamma = \Phi_X - \frac{y(p^\prime_{11} - x)}{x}
\]

And the upper bound on PNS is evaluated as
\begin{align*}
    p_{11} - \Gamma &= p_{11} - \Phi_X + \frac{y(p^\prime_{11} - x)}{x}\\
    p_{11} - \Gamma &= p_{00} - \frac{y(p^\prime_{11} - x)}{x}\\
\end{align*}

\subsubsection{Case VII}

\begin{align}
    \Phi_X < 0\\
    x < 1 - x\\
    x <  1 - x < p^\prime_{11}\\
    p^\prime_{10} < x < 1- x 
\end{align}

These constraints imply based on (\ref{p_111_bounds}) and the implications on Subsection \ref{implications_bounds_p111}, the following lower and upper bounds on $P(Z = 1 \mid X = 1, Y = 1)$: 
\begin{align*}
    \max\begin{bmatrix}
        \frac{p^\prime_{11} - (1 - x)}{x}\\
        \frac{p^\prime_{11}y-p_{10}(1-x)}{xy}
    \end{bmatrix} \leq P(Z = 1\mid X = 1, Y = 1) \leq 
    min\begin{bmatrix}
    1\\
    \frac{p_{11}}{y}
    \end{bmatrix}
\end{align*}
Now we will check if each of the possible lower bounds are greater than $b$.
\begin{enumerate}
    \item $\frac{p^\prime_{11} - (1 - x)}{x} < \frac{(1 - x) - p^\prime_{11}}{(1 - x) - x}$. This is a contradiction since the LHS is positive based on our assumptions while the RHS is negative. 
    \item Assume
    \[
    \frac{p^\prime_{11}y-p_{10}(1-x)}{xy} > \frac{(1 - x) - p^\prime_{11}}{(1 - x) - x}
    \]. 
    \begin{align*}
        \implies \Phi_X > \frac{(1 - y)(p^\prime_{10} - x)}{x}
    \end{align*}
    So, when this holds, this lower bound is capable of falsification. 
\end{enumerate}
Now we will check if each of the possible upper bounds are less than $a$. 
\begin{enumerate}
    \item Following proof by contradiction, assume
    \[
    \frac{p_{11}}{y} < \frac{(1 - x)(\Phi_X + y) - p^\prime_{11}y}{y((1 - x) - x)}
    \]
    \begin{align*}
        \implies p_{11}(1 - x) - p_{11}x < (1 - x)\Phi_X + y(1 - x) - p^\prime_{11}y\\
        \implies (1 - x)\Phi_X - p^\prime_{10}(1 - y) < (1 - x)\Phi_X - (1 - y)(1 - x)\\
        \implies 0 < (1 - y)(p^\prime_{10} - (1 - x))
    \end{align*}
    This is a contradiction.
    \item Upper bound is $1$: Assume 
    \[
    1 < \frac{(1 - x)(\Phi_X + y) - p^\prime_{11}y}{y((1 - x) - x)}
    \]
    \begin{align*}
        \implies (1 - x)(\Phi_X + y) > (1 - x)y - xy + p^\prime_{11}y\\
        \implies (1 - x)\Phi_X > y(p^\prime_{11} - x)
    \end{align*}
    This is a contradiction since LHS is negative but RHS is positive. 
\end{enumerate}

So, when the lower bound is $\frac{p^\prime_{11} - (1 - x)}{x}$, $\Gamma$ will evaluate to
\begin{align*}
    \Gamma &= \frac{p^\prime_{11}y - y(1 - x)}{x}(1 - OR(X)) + \frac{p^\prime_{11}y - y(1 - x)}{1 - x}\\
    &= \frac{y(p^\prime_{11} - (1 - x))}{x}
\end{align*}

And so the upper bound on PNS will be
\begin{align*}
p_{11} - \Gamma =  p_{11} - \frac{y(p^\prime_{11} - (1 - x))}{x}
\end{align*}

Next, when the lower bound is $\frac{p^\prime_{11}y-p_{10}(1-x)}{xy}$, $\Gamma$ is computed by inserting this lower bound into increasing function $P(Z = 1 \mid X = 1, Y = 1)(1 - OR(X))y + y\frac{p^\prime_{11} - (1 - x)}{1 - x}$. 
\begin{align*}
    \Gamma &=\frac{p^\prime_{11}y - p_{10}(1 - x)}{x}(1 - OR(X)) + y\frac{p^\prime_{11} - (1 - x)}{1 - x} \\
    \Gamma &= \Phi_X - \frac{(1 - y)(p^\prime_{10} - x)}{x}
\end{align*}

And the upper bound on PNS is computed as
\begin{align*}
    p_{11} - \Gamma &= p_{11} - \Phi_X + \frac{(1 - y)(p^\prime_{10} - x)}{x}\\
    &= p_{00} - \frac{(1 - y)(x - p^\prime_{10})}{x}\\
\end{align*}

\subsubsection{Case VIII}

\begin{align}
    \Phi_X < 0\\
    x < 1 - x\\
    x <  1 - x < p^\prime_{11}\\
    x < p^\prime_{10} < 1- x 
\end{align}

These constraints imply based on (\ref{p_111_bounds}) and the implications on Subsection \ref{implications_bounds_p111}, the following lower and upper bounds on $P(Z = 1 \mid X = 1, Y = 1)$: 
\begin{align*}
    max\begin{bmatrix}
        \frac{p^\prime_{11} - (1 - x)}{x}\\
        \frac{p_{11} - (1 - y)}{y}
    \end{bmatrix} \leq P(Z = 1\mid X = 1, Y = 1) \leq 
    min\begin{bmatrix}
    1\\
    \frac{p_{11}}{y}
    \end{bmatrix}
\end{align*}

The same arguments as the previous case are utilized for the upper bounds, and consequently they cannot falsify. The same argument for $\frac{p^\prime_{11} - (1 - x)}{x}$ is used, and this can falsify. 

When the lower bound is $\frac{p_{11} - (1 - y)}{y}$:
    \begin{align*}
        &\frac{p_{11}-(1-y)}{y} > \frac{(1 - x) - p^\prime_{11}}{(1 - x) - x}\\ 
        &\implies \Phi_X > \frac{(1 - y)(p^\prime_{10} - x)}{1 - x}
    \end{align*}
    This is contradiction since LHS is negative but RHS is positive.

So, when the lower bound is $\frac{p^\prime_{11} - (1 - x)}{x}$, $\Gamma$ will evaluate to
\begin{align*}
    \Gamma &= \frac{p^\prime_{11}y - y(1 - x)}{x}(1 - OR(X)) + \frac{p^\prime_{11}y - y(1 - x)}{1 - x}\\
    &= \frac{y(p^\prime_{11} - (1 - x))}{x}
\end{align*}

And so the upper bound on PNS will be
\begin{align*}
p_{11} - \Gamma =  p_{11} - \frac{y(p^\prime_{11} - (1 - x))}{x}
\end{align*}

\subsubsection{Case IX}

\begin{align}
    \Phi_X < 0\\
    x < 1 - x\\
    x <  1 - x < p^\prime_{11}\\
    x < 1- x < p^\prime_{10}
\end{align}

These constraints imply based on (\ref{p_111_bounds}) and the implications on Subsection \ref{implications_bounds_p111}, the following lower and upper bounds on $P(Z = 1 \mid X = 1, Y = 1)$: 
\begin{align*}
    \max\begin{bmatrix}
        \frac{p^\prime_{11} - (1 - x)}{x}\\
        \frac{p_{11} - (1 - y)}{y}
    \end{bmatrix} \leq P(Z = 1\mid X = 1, Y = 1) \leq 
    \min\begin{bmatrix}
    1\\
    \frac{(1-x)(1-y) - p_{10}(1-x) + p^\prime_{11}y}{xy}
    \end{bmatrix}
\end{align*}

The same arguments from the above case are used for the lower bounds, with the conclusion that $\frac{p^\prime_{11} - (1 - x)}{x}$ is capable of inducing falsification. 

Following the same argument as before for $1$, it is incapable of falsifying. $\frac{(1-x)(1-y) - p_{10}(1-x) + p^\prime_{11}y}{xy}$ is capable of falsifying. 

So, when the lower bound is $\frac{p^\prime_{11} - (1 - x)}{x}$, $\Gamma$ will evaluate to
\begin{align*}
    \Gamma &= \frac{p^\prime_{11}y - y(1 - x)}{x}(1 - OR(X)) + \frac{p^\prime_{11}y - y(1 - x)}{1 - x}\\
    &= \frac{y(p^\prime_{11} - (1 - x))}{x}
\end{align*}

And so the upper bound on PNS will be
\begin{align*}
p_{11} - \Gamma =  p_{11} - \frac{y(p^\prime_{11} - (1 - x))}{x}
\end{align*}

When the upper bound is $\frac{(1-x)(1-y) - p_{10}(1-x) + p^\prime_{11}y}{xy}$, $\Gamma$ is evaluated as
\[
\Gamma = \frac{(1 - y)(p^\prime_{10} - (1 - x))}{x}
\]

And this gives the following upper bound on PNS as
\begin{align*}
    p_{11} - \Gamma = p_{11} - \frac{(1 - y)(p^\prime_{10} - (1 - x))}{x}
\end{align*}

\subsection{Case II: $\Phi_X \geq 0$}

The usual breakdown around $x > 1- x$ or not will happen. Assuming $x > 1 - x$, falsification will happen when line 3 and line 4 of the matrix are greater than 0, we first check the values of $P(Z = 1 \mid X = 1, Y = 1)$ for which this happens. 
\begin{itemize}
    \item When $yP(Z = 1\mid X = 1, Y = 1)(OR(X) - 1) + \Phi_X + y - \frac{p^\prime_{11}y}{1 - x} \geq \Phi_X$:
    \begin{equation}
        \implies P(Z = 1 \mid X = 1, Y = 1) \geq \frac{p^\prime_{11} - (1 - x)}{x - (1 - x)}\\
    \end{equation}\label{val:turning-point-a}

    We denote this value as 
    \begin{equation}\
        b =\frac{p^\prime_{11} - (1 - x)}{x - (1 - x)}
    \end{equation}
    
    \item When $P(Z = 1 \mid X = 1, Y = 1)(1 - OR(X))y + y\frac{p^\prime_{11} - (1 - x)}{1 - x} \geq \Phi_X$
    \begin{equation}
        \implies \frac{p^\prime_{11}y - (1 - x)(\Phi_X + y)}{y(x - (1 - x))} \geq P(Z = 1 \mid X = 1, Y = 1)
    \end{equation}\label{val:turning-point-b}

    We denote this value as
    \begin{equation}
        a = \frac{p^\prime_{11}y - (1 - x)(\Phi_X + y)}{y(x - (1 - x))}
    \end{equation}.
\end{itemize}

\subsection{Case By Case Upper Bound Calculation}

Each of these sections considers a different case where the values of $p^\prime_{11}$, $p^\prime_{10}$ are picked relative to $x$ and $1 - x$.

\subsubsection{Case I}

This case assumes the following
\begin{align}
    \Phi_X \geq 0\\
    1 - x < x\\
    1 - x < p^\prime_{11} < x\\
    p^\prime_{10} < 1 - x < x
\end{align}

The first two have been assumed in a larger context, and the last two are made for this specific case for this section. 

These conditions, based on the implications in subsection \ref{implications_bounds_p111}, limit the choice of bounds on $P(Z = 1 \mid X = 1, Y = 1)$ from (\ref{p_111_bounds}) to 
\[
\max \begin{bmatrix}
    \frac{p^\prime_{11} - (1 - x)}{x}\\
    \frac{p^\prime_{11}y - p_{10}(1 - x)}{xy}
\end{bmatrix} \leq P(Z = 1 \mid X = 1, Y = 1) \leq 
\min \begin{bmatrix}
   \frac{p_{11}}{y}\\
   \frac{p^\prime_{11}}{x}
\end{bmatrix}
\]

Now, we know falsification will happen when either lower bound is greater than (b), or the upper bound is less than \ref{a}. So we examine each choice of upper and lower bound, and see whether they can be less than \ref{a} or \ref{b}. 
\begin{enumerate}
    \item $\frac{p^\prime_{11} - (1 - x)}{x} $: This will be less than (b), i.e. $\frac{p^\prime_{11} - (1 - x)}{x}  < \frac{p^\prime_{11} - (1 - x)}{2x - 1}$ since the denominator is smaller on the right hand side. 
    \item $\frac{p^\prime_{11}y - p_{10}(1 - x)}{xy}$: Assume
    \[
    \frac{p^\prime_{11}y - p_{10}(1 - x)}{xy} > \frac{p^\prime_{11} - (1 - x)}{x - (1 - x)}
    \]
    
    \begin{align*}
        &\implies \Phi_X < \frac{(1 - y)(p^\prime_{10} - x)}{x}
    \end{align*}
    This is a contradiction since RHS is negative and LHS in positive. 
\end{enumerate}


And so, the lower bounds will always be less than (b), so any falsification will come from the upper bounds being less than (a), which we check below. 

\begin{enumerate}
    \item When the upper bound is $\frac{p_{11}}{y}$: Checking this against (a) using a proof by contradiction, we assume
    \begin{align*}
        &\frac{p^\prime_{11}y - (1 - x)(p_{11} + p_{10} - 1) - y(1 - x)}{y(x - (1 - x))} < \frac{p_{11}}{y}\\
       &\implies p^\prime_{11}y - (1 - x)(p_{11} + p_{10} - 1) - y(1 - x) < p_{11}x - p_{11}(1 - x)\\
       &\implies p_{11}x + p_{10}(1 - x) - p^\prime_{10}(1 - y) - (1 - x)(p_{11} + p_{10} - 1) - y(1 - x) < p_{11}x - p_{11}(1 - x)\\
       &\implies p_{10}(1 - x) + p_{11}(1 - x) - p^\prime_{10}(1 - y) - (1 - x)(p_{11} + p_{10} - 1) - y(1 - x) < 0\\
       &\implies - p^\prime_{10}(1 - y) + (1 - x) - y(1 - x) < 0\\
       &\implies - p^\prime_{10}(1 - y) + (1 - x)(1 - y) < 0\\
       &\implies - p^\prime_{10} + (1 - x) < 0\\
    \end{align*}
    This is a contradiction, and so $\frac{p^\prime_{11}y - (1 - x)(p_{11} + p_{10} - 1) - y(1 - x)}{y(x - (1 - x))} \geq \frac{p_{11}}{y}$ and this bound is capable of falsifying.
    
    \item Upper bound is $\frac{p^\prime_{11}}{x}$: 
    \begin{align*}
        \frac{p^\prime_{11}}{x} < \frac{p^\prime_{11}y - (1 - x)(\Phi_X + y)}{y(x - (1 - x))}\\
        \implies \Phi_X < \frac{y(p^\prime_{11} - x)}{x}
    \end{align*}
    This is a contradiction, so this bound cannot falsify. 
\end{enumerate}

Falsification will happen when $\frac{p_{11}}{y}$ is the upper bound, which requires the following condition to hold
\[\frac{p_{11}}{y} < \frac{p^\prime_{11}}{x} \implies p_{11}x < p^\prime_{11}y\]


Putting this all together, in Case I, when the following condition holds:
\begin{align*}
    &p_{11}x < p^\prime_{11}y
\end{align*}

We will get falsification, where $\Gamma$ is calculated as
\[ \Gamma = \Phi_X - \frac{(1 - y)(p^\prime_{10} - (1 - x))}{1 - x} \]

Now, subtracting this from $p_{11}$, we have
\begin{align*}
 p_{11} - \Gamma &= p_{11} - (p_{11} + p_{10} - 1) + \frac{(1 - y)(p^\prime_{10} - (1 - x))}{1 - x}\\
 p_{11} - \Gamma &= p_{00} - \frac{(1 - y)((1 - x) - p^\prime_{10})}{1 - x}
\end{align*}

\subsubsection{Case II}

This case assumes the following
\begin{align}
    \Phi_X < 0\\
    1 - x < x\\
    1 - x < p^\prime_{11} < x\\
    1 - x < p^\prime_{10} < x
\end{align}

These conditions limit the choice of bounds on $P(Z = 1 \mid X = 1, Y = 1)$ from (\ref{p_111_bounds}) to 
\[
\max\begin{bmatrix}
    \frac{p^\prime_{11} - (1 - x)}{x}\\
    \frac{p^\prime_{11}y - p_{10}(1 - x)}{xy}
\end{bmatrix} \leq P(Z = 1 \mid X = 1, Y = 1) \leq 
\min\begin{bmatrix}
   \frac{p^\prime_{11}}{x}\\
   \frac{(1 - x)(1 - y) - p_{10}(1 - x) + p^\prime_{11}y}{xy}
\end{bmatrix}
\]

Now, we check whether the lower bounds are greater than (b) and if the upper bounds are less than (a).
\begin{enumerate}
     \item First, $\frac{p^\prime_{11} - (1 - x)}{x} < \frac{p^\prime_{11} - (1 - x)}{x - (1 - x)}$ since the denominator is smaller on the right hand side. This lower bound is less than (b).
     \item Checking the lower bound of $\frac{p^\prime_{11}y - p_{10}(1 - x)}{xy}$ against (b), using a proof by contradiction. Assume,
     \[ \frac{p^\prime_{11}y - p_{10}(1 - x)}{xy} > 
         \frac{p^\prime_{11} - (1 - x)}{x - (1 - x)}
     \]
     \begin{align*}
         (1 - y)(p^\prime_{10} - x) > x\Phi_X
     \end{align*}
    This is a contradiction since the RHS is positive but he LHS is negative. 
\end{enumerate}

Checking the upper bounds now. 

\begin{enumerate}
     \item When the upper bound is $\frac{p^\prime_{11}}{x}$: Checking this against the (a).
    \begin{align*}
        \frac{p^\prime_{11}}{x} < \frac{ p^\prime_{11}y - (1 - x)(\Phi_X + y)}{y(x - (1 - x))}\\
        \implies  \Phi_X < \frac{y(p^\prime_{11} - x)}{x}
    \end{align*}
     This is a contradiction because of the case we are in. 
     \item When the upper bound is $\frac{(1 - x)(1 - y) - p_{10}(1 - x) + p^\prime_{11}y}{xy}$: Assume
     \[
     \frac{(1 - x)(1 - y) - p_{10}(1 - x) + p^\prime_{11}y}{xy} < \frac{ p^\prime_{11}y - (1 - x)(\Phi_X + y)}{y(x - (1 - x))}\\
     \]
     \begin{align*}
       &\implies (1 - y)(p^\prime_{10} - (1 - x)) < 0
     \end{align*}
     This creates a contradiction since the LHS is positive but the RHS is 0.
\end{enumerate}


 Since the lower bounds are less than (b), and upper bounds are greater than (a), so $\Gamma = \Phi_X$. 

\subsubsection{Case III} 

This case assumes the following conditions
\begin{align}
    \Phi_X \geq 0\\
    1 - x < x\\
    1 - x < p^\prime_{11} < x\\
    1 - x < x < p^\prime_{10}
\end{align}

These conditions limit the choice of bounds on $P(Z = 1 \mid X = 1, Y = 1)$ from (\ref{p_111_bounds}) to 
\[\max
\begin{bmatrix}
    \frac{p^\prime_{11} - (1 - x)}{x}\\
    \frac{p_{11} - (1 - y)}{y}
\end{bmatrix} \leq P(Z = 1 \mid X = 1, Y = 1) \leq 
\min\begin{bmatrix}
   \frac{p^\prime_{11}}{x}\\
   \frac{(1 - x)(1 - y) - p_{10}(1 - x) + p^\prime_{11}y}{xy}
\end{bmatrix}
\]

Following the usual approach, we start with checking the lower bounds against \ref{b}.

\begin{enumerate}
    \item First, $\frac{p^\prime_{11} - (1 - x)}{x} < \frac{p^\prime_{11} - (1 - x)}{x - (1 - x)}$ since the denominator is smaller on the right hand side. This lower bound is less than (b).
    \item Checking $\frac{p_{11} - (1 - y)}{y}$: Assume
    \[
        \frac{p_{11} - (1 - y)}{y} > \frac{p^\prime_{11} - (1 - x)}{x - (1 - x)}
    \]
    \begin{align*}
        \implies \frac{(1 - y)(p^\prime_{10} - x)}{1 - x} < \Phi_X
    \end{align*}
    So, when this condition holds this lower bound will be greater than (b). 
\end{enumerate}

Now, we check the upper bounds against (a).
\begin{enumerate}
     \item When the upper bound is $\frac{p^\prime_{11}}{x}$: Checking this against the (a).
    \begin{align*}
        \frac{p^\prime_{11}}{x} < \frac{ p^\prime_{11}y - (1 - x)(\Phi_X + y)}{y(x - (1 - x))}\\
        \implies  \Phi_X < \frac{y(p^\prime_{11} - x)}{x}
    \end{align*}
     This is a contradiction because of the case we are in. 
     \item When the upper bound is $\frac{(1 - x)(1 - y) - p_{10}(1 - x) + p^\prime_{11}y}{xy}$: Assume
     \[
     \frac{(1 - x)(1 - y) - p_{10}(1 - x) + p^\prime_{11}y}{xy} < \frac{ p^\prime_{11}y - (1 - x)(\Phi_X + y)}{y(x - (1 - x))}\\
     \]
     \begin{align*}
       &\implies (1 - y)(p^\prime_{10} - (1 - x)) < 0
     \end{align*}
     This creates a contradiction since the LHS is positive but the RHS is 0.
\end{enumerate}

Now, the first condition that must be satisfied is $\frac{p_{11} - (1 - y)}{y}$ is the lower bound, which requires the following condition to hold
\[
 p_{01}x < p^\prime_{01}y
\]

Then, we substitute the lower bound into the increasing function of $P(Z = 1\mid X = 1, Y = 1)$
\begin{align*}
    &\frac{(1 - x)(p_{10} + p_{11} - 1) - p^\prime_{11}y + P(Z = 1\mid X = 1, Y = 1)y(x - (1 - x)) + (1 - x)y}{1 - x}\\
    &= \frac{(1 - x)(p_{10} + p_{11} - 1) - p^\prime_{11}y + (p_{11} - (1 - y))(x - (1 - x)) + (1 - x)y}{1 - x}\\
    &= \frac{(1 - x)(p_{10} + p_{11} - 1) + p^\prime_{10}(1 - y) - p_{10}(1 - x) - (p_{11} - (1 - y))(1 - x) + (1 - x)y}{1 - x}\\
    &= \frac{(1 - x)(p_{10} + p_{11} - 1) + p^\prime_{10}(1 - y) -(1 - x)(p_{10} + p_{11} - 1) - x(1 - y)}{1 - x}\\
    &= \frac{p^\prime_{10}(1 - y) - x(1 - y)}{1 - x} = \frac{(1 - y)(p^\prime_{10} - x)}{1 - x}
\end{align*}

So in this case, when $p_{01}x < p^\prime_{01}y$ holds, we get falsification with $\Gamma$ evaluating to
\[
\Gamma = \frac{(1 - y)(p^\prime_{10} - x)}{1 - x}
\]

And so the upper bound for PNS will be
\[
p_{11} - \Gamma = p_{11} - \frac{(1 - y)(p^\prime_{10} - x)}{1 - x}
\] 

\subsubsection{Case IV}

We assume the following conditions
\begin{align}
    \Phi_X \geq 0\\
    1 - x < x\\
    p^\prime_{11} <1 - x  < x\\
    p^\prime_{10} < 1 - x < x
\end{align}

These constraints imply the following lower and upper bounds on $P(Z = 1 \mid X = 1, Y = 1)$ from (\ref{p_111_bounds}) to
\begin{align*}
    \max\begin{bmatrix}
        0 \\
        \frac{p^\prime_{11}y - p_{10}(1 - x)}{xy}
    \end{bmatrix} \leq P(Z = 1\mid X = 1, Y = 1) \leq 
    \min\begin{bmatrix}
        \frac{p_{11}}{y}\\
        \frac{p^\prime_{11}}{x}
    \end{bmatrix}
\end{align*}

Here, since (b) will always be negative, we expect both lower bounds to falsify.
\begin{enumerate}
    \item Lower bound is $0$: Since the numerator in (b) is negative, $0$ will be greater. 
     \item Lower bound is $\frac{p^\prime_{11}y - p_{10}(1 - x)}{xy}$: Assume
     \[
        \frac{p^\prime_{11}y - p_{10}(1 - x)}{xy} > \frac{p^\prime_{11} - (1 - x)}{x - (1 - x)}
     \]
     \begin{align*}
         \implies (1 - y)(p^\prime_{10} - x) > x\Phi_X
     \end{align*}
     This is a contradiction. 
 \end{enumerate}

Consequently, when $0$ is the lower bound, which requires the following condition to hold 
\[
p_{10}(1 - x) > p^\prime_{11}y
\]

Then $\Gamma$ will evaluate to
\[
\Phi_X - \frac{y(p^\prime_{11} - (1 - x))}{1 - x}
\]

And the upper bound on PNS will be
\begin{align*}
p_{11} - \Gamma &= p_{11} - \Phi_X + \frac{y(p^\prime_{11} - (1 - x))}{1 - x}\\
&= p_{00} - \frac{y((1 - x) - p^\prime_{11})}{1 - x}
\end{align*}

\subsubsection{Case V}
We assume the following conditions
\begin{align}
    \Phi_X \geq 0\\
    1 - x < x\\
    p^\prime_{11} <1 - x  < x\\
    1 - x < p^\prime_{10} < x
\end{align}

These constraints imply the following lower bounds on $P(Z = 1 \mid X = 1, Y = 1)$ from (\ref{p_111_bounds}). Only the lower bound is checked against \ref{b} since \ref{a} will be negative in this case. 
\begin{align*}
    \max\begin{bmatrix}
        0 \\
        \frac{p^\prime_{11}y - p_{10}(1 - x)}{xy}
    \end{bmatrix} \leq P(Z = 1\mid X = 1, Y = 1) 
\end{align*}

$0$ will be greater than (b) since (b) is negative, and the same argument as above will apply to $\frac{p^\prime_{11}y - p_{10}(1 - x)}{xy}$. 

Then, $\Gamma$ will evaluate to
Then $\Gamma$ will evaluate to
\[
\Phi_X - \frac{y(p^\prime_{11} - (1 - x))}{1 - x}
\]

And the upper bound on PNS will be
\begin{align*}
p_{11} - \Gamma &= p_{11} - \Phi_X + \frac{y(p^\prime_{11} - (1 - x))}{1 - x}\\
&= p_{00} - \frac{y((1 - x) - p^\prime_{11})}{1 - x}
\end{align*}

\subsubsection{Case VI}
We assume the following conditions
\begin{align}
    \Phi_X \geq 0\\
    1 - x < x\\
    p^\prime_{11} <1 - x  < x\\
    1 - x < x < p^\prime_{10}
\end{align}

Similar to the previous case, only the lower bound needs to be checked. These constraints imply the following lower bounds on $P(Z = 1 \mid X = 1, Y = 1)$ from (\ref{p_111_bounds}) as
\begin{align*}
    max\begin{bmatrix}
        0 \\
        \frac{p_{11} - (1 - y)}{y}
    \end{bmatrix} \leq P(Z = 1\mid X = 1, Y = 1) 
\end{align*}

Now, we check whether each of these lower bounds can be greater than \ref{b}. 
\begin{enumerate}
    \item Lower bound is $0$ - the same argument as the previous case holds.
    \item Lower bound is $\frac{p_{11} - (1 - y)}{y}$: Assume
    \[
        \frac{p_{11} - (1 - y)}{y} > \frac{p^\prime_{11} - (1 - x)}{x - (1 - x)}
    \]
    \begin{align*}
        \implies \frac{(1 - y)(p^\prime_{10} - x)}{1 - x} < \Phi_X
    \end{align*}
    So, when this condition holds this lower bound will be greater than (b). 
\end{enumerate}

So, the falsification will be as follows. 

When $p_{11} > 1 - y$, $\frac{p_{11} - (1 - y)}{y}$ will be the lower bound, and $\Gamma$ will be evaluating by inserting this lower bound into $yP(Z = 1\mid X = 1, Y = 1)(OR(X) - 1) + \Phi_X + y - \frac{p^\prime_{11}y}{1 - x}$. And $\Gamma$ will evaluate to
\[
\Gamma = \frac{(1 - y)(p^\prime_{10} - x)}{1 - x}
\]

And therefore the upper bound on PNS will be
\begin{align*}
    p_{11} - \Gamma = p_{11} - \frac{(1 - y)(p^\prime_{10} - x)}{1 - x}
\end{align*}

Next, when $p_{11} < 1 - y$, $0$ will be the lower bound, and $\Gamma$ will evaluate to 
\[
\Gamma = \Phi_X - \frac{y(p^\prime_{11} - (1 - x))}{1 - x}
\]

And the upper bound on PNS will be
\begin{align*}
    p_{11} - \Gamma = p_{00} - \frac{y((1 - x) - p^\prime_{11})}{1 - x}
\end{align*}

\subsubsection{Case VII}
We assume the following conditions
\begin{align}
    \Phi_X \geq 0\\
    1 - x < x\\
    1 - x  < x < p^\prime_{11}\\
    p^\prime_{10} < 1 - x < x
\end{align}

These constraints imply based on (\ref{p_111_bounds}) and the implications on Subsection \ref{implications_bounds_p111}, the following lower and upper bounds on $P(Z = 1 \mid X = 1, Y = 1)$: 
\begin{align*}
    \max\begin{bmatrix}
        \frac{p^\prime_{11}-(1-x)}{x} \\
        \frac{p^\prime_{11}y-p_{10}(1-x)}{xy}
    \end{bmatrix} \leq P(Z = 1\mid X = 1, Y = 1) \leq 
    \min\begin{bmatrix}
        1\\
        \frac{p_{11}}{y}
    \end{bmatrix}
\end{align*}
Now we will check if each of the possible lower bounds are greater than (b).
\begin{enumerate}
     \item First, $\frac{p^\prime_{11} - (1 - x)}{x} < \frac{p^\prime_{11} - (1 - x)}{x - (1 - x)}$ since the denominator is smaller on the right hand side. This lower bound is less than (b).
    \item Lower bound is $\frac{p^\prime_{11}y - p_{10}(1 - x)}{xy}$: Assume
     \[
        \frac{p^\prime_{11}y - p_{10}(1 - x)}{xy} > \frac{p^\prime_{11} - (1 - x)}{x - (1 - x)}
     \]
     \begin{align*}
         \implies (1 - y)(p^\prime_{10} - x) > x\Phi_X
     \end{align*}
     This is a contradiction. 
\end{enumerate}

Now we will check if each of the possible upper bounds are less than (a). 
\begin{enumerate}
    \item When the upper bound is $\frac{p_{11}}{y}$: Checking this against (a) using a proof by contradiction, we assume
    \begin{align*}
        &\frac{p^\prime_{11}y - (1 - x)(p_{11} + p_{10} - 1) - y(1 - x)}{y(x - (1 - x))} < \frac{p_{11}}{y}\\
       &\implies p^\prime_{11}y - (1 - x)(p_{11} + p_{10} - 1) - y(1 - x) < p_{11}x - p_{11}(1 - x)\\
       &\implies p_{11}x + p_{10}(1 - x) - p^\prime_{10}(1 - y) - (1 - x)(p_{11} + p_{10} - 1) - y(1 - x) < p_{11}x - p_{11}(1 - x)\\
       &\implies p_{10}(1 - x) + p_{11}(1 - x) - p^\prime_{10}(1 - y) - (1 - x)(p_{11} + p_{10} - 1) - y(1 - x) < 0\\
       &\implies - p^\prime_{10}(1 - y) + (1 - x) - y(1 - x) < 0\\
       &\implies - p^\prime_{10}(1 - y) + (1 - x)(1 - y) < 0\\
       &\implies - p^\prime_{10} + (1 - x) < 0\\
    \end{align*}
    This is a contradiction, and so $\frac{p^\prime_{11}y - (1 - x)(p_{11} + p_{10} - 1) - y(1 - x)}{y(x - (1 - x))} \geq \frac{p_{11}}{y}$ and this bound is capable of falsifying.
    \item Upper bound is $1$: 
    \[
    \frac{p^\prime_{11}y - (1 - x)(p_{11} + p_{10} - 1) - y(1 - x)}{y(x - (1 - x))} > 1
    \]
    \begin{align*}
        \implies \frac{y(p^\prime_{11} - x)}{1 - x} > \Phi_X
    \end{align*}
\end{enumerate}

Now, for each of these settings, we evaluate $\Gamma$ and PNS.
\begin{enumerate}
    \item Upper bound is $1$:
    \begin{align*}
        \Gamma &= (1 - OR(X))y + y\frac{p^\prime_{11} - (1 - x)}{1 - x}\\
        &= y - \frac{xy}{1 - x} + \frac{yp^\prime_{11} - y(1 - x)}{1 - x}\\
        &= \frac{y(p^\prime_{11} - x)}{1 - x}
    \end{align*}
    And the PNS upper bound will be
    \begin{align*}
        p_{11} - \Gamma &= p_{11} - \Gamma\\
        \implies  &= p_{11} - \frac{y(p^\prime_{11} - x)}{1 - x}
    \end{align*}
    \item Upper bound is $\frac{p_{11}}{y}$: Then
    \begin{align*}
        \Gamma &= p_{11}(1 - OR(X)) + y\frac{p^\prime_{11} - (1 - x)}{1 - x}\\
        &= p_{11} + \frac{p^\prime_{11}y - p_{11}x - y(1 - x)}{1 - x}\\
        &= p_{11} + \frac{p_{10}(1 - x) - p^\prime_{10}(1 - y) - y(1 - x)}{1 - x}\\
        &= p_{11} + \frac{p_{10}(1 - x) - p^\prime_{10}(1 - y) - (1 - (1 - y))(1 - x)}{1 - x}\\
        &= p_{11} + p_{10} - 1 + \frac{ - p^\prime_{10}(1 - y) + (1 - y)(1 - x)}{1 - x}\\
        &= \Phi_X - \frac{(1 - y)(p^\prime_{10} - (1 - x))}{1 - x}
    \end{align*}
    And the upper bound on PNS will evaluate to
    \begin{align*}
        p_{11} - \Gamma = p_{00} - \frac{(1 - y)((1 - x) - p^\prime_{10})}{1 - x}
    \end{align*}
\end{enumerate}

\subsubsection{Case VIII}
We assume the following conditions
\begin{align}
    \Phi_X \geq 0\\
    1 - x < x\\
    1 - x  < x < p^\prime_{11}\\
    1 - x < p^\prime_{10} < x
\end{align}

These constraints imply based on (\ref{p_111_bounds}) and the implications on Subsection \ref{implications_bounds_p111}, the following lower and upper bounds on $P(Z = 1 \mid X = 1, Y = 1)$: 
\begin{align*}
    \max\begin{bmatrix}
        \frac{p^\prime_{11}-(1-x)}{x} \\
        \frac{p^\prime_{11}y-p_{10}(1-x)}{xy}
    \end{bmatrix} \leq P(Z = 1\mid X = 1, Y = 1) \leq 
    \min\begin{bmatrix}
        1\\
        \frac{(1-x)(1-y) - p_{10}(1-x) + p^\prime_{11}y}{xy}
    \end{bmatrix}
\end{align*}

Now we will check if each of the possible lower bounds are greater than (b).
\begin{enumerate}
    \item First, $\frac{p^\prime_{11} - (1 - x)}{x} < \frac{p^\prime_{11} - (1 - x)}{x - (1 - x)}$ since the denominator is smaller on the right hand side. This lower bound is less than (b).
    \item Lower bound is $\frac{p^\prime_{11}y - p_{10}(1 - x)}{xy}$: Assume
     \[
        \frac{p^\prime_{11}y - p_{10}(1 - x)}{xy} > \frac{p^\prime_{11} - (1 - x)}{x - (1 - x)}
     \]
     \begin{align*}
         \implies (1 - y)(p^\prime_{10} - x) > x\Phi_X
     \end{align*}
     This is a contradiction. 
\end{enumerate} 

Now, checking the upper bounds.
\begin{enumerate}
    \item Upper bound is $1$: 
    \[
    \frac{p^\prime_{11}y - (1 - x)(p_{11} + p_{10} - 1) - y(1 - x)}{y(x - (1 - x))} > 1
    \]
    \begin{align*}
        \implies \frac{y(p^\prime_{11} - x)}{1 - x} > \Phi_X
    \end{align*}
    So, when this holds we will get falsification. 
    \item When the upper bound is $\frac{(1 - x)(1 - y) - p_{10}(1 - x) + p^\prime_{11}y}{xy}$: Assume
     \[
     \frac{(1 - x)(1 - y) - p_{10}(1 - x) + p^\prime_{11}y}{xy} < \frac{ p^\prime_{11}y - (1 - x)(\Phi_X + y)}{y(x - (1 - x))}\\
     \]
     \begin{align*}
       &\implies (1 - y)(p^\prime_{10} - (1 - x)) < 0
     \end{align*}
     This creates a contradiction since the LHS is positive but the RHS is 0.
\end{enumerate}
So, when $1 < \frac{(1-x)(1-y) - p_{10}(1-x) + p^\prime_{11}y}{xy}$, then $\Gamma$ will be evaluated by subsititung $1$ as the value for $P(Z = 1 \mid X = 1, Y = 1)$ into $P(Z = 1 \mid X = 1, Y = 1)(1 - OR(X))y + y\frac{p^\prime_{11} - (1 - x)}{1 - x}$, to get
\begin{align*}
    \Gamma &= (1 - OR(X))y + y\frac{p^\prime_{11} - (1 - x)}{1 - x}\\
    &= \frac{y(p^\prime_{11} - x)}{1 - x}
\end{align*}

And the upper bound on PNS will be
\begin{align*}
    p_{11} - \Gamma = p_{11} - \frac{y(p^\prime_{11} - x)}{1 - x}
\end{align*}

\subsubsection{Case IX}
We assume the following conditions
\begin{align}
    \Phi_X \geq 0\\
    1 - x < x\\
    1 - x  < x < p^\prime_{11}\\
    1 - x < x < p^\prime_{10}
\end{align}

These constraints imply based on (\ref{p_111_bounds}) and the implications on Subsection \ref{implications_bounds_p111}, the following lower and upper bounds on $P(Z = 1 \mid X = 1, Y = 1)$: 
\begin{align*}
    \max\begin{bmatrix}
        \frac{p^\prime_{11}-(1-x)}{x} \\
        \frac{p_{11}-(1-y)}{y}
    \end{bmatrix} \leq P(Z = 1\mid X = 1, Y = 1) \leq 
    \min\begin{bmatrix}
        1\\
        \frac{(1-x)(1-y) - p_{10}(1-x) + p^\prime_{11}y}{xy}
    \end{bmatrix}
\end{align*}

Now we will check if each of the possible lower bounds are greater than (b).
\begin{enumerate}
    \item First, $\frac{p^\prime_{11} - (1 - x)}{x} < \frac{p^\prime_{11} - (1 - x)}{x - (1 - x)}$ since the denominator is smaller on the right hand side. This lower bound is less than (b).
    \item Lower bound is $\frac{p_{11} - (1 - y)}{y}$: Assume
    \[
        \frac{p_{11} - (1 - y)}{y} > \frac{p^\prime_{11} - (1 - x)}{x - (1 - x)}
    \]
    \begin{align*}
        \implies \frac{(1 - y)(p^\prime_{10} - x)}{1 - x} < \Phi_X
    \end{align*}
    So, when this condition holds this lower bound will be greater than (b).     
\end{enumerate}

Now we will check if each of the possible upper bounds are less than (a).
\begin{enumerate}
    \item Upper bound is $1$: 
    \[
    \frac{p^\prime_{11}y - (1 - x)(p_{11} + p_{10} - 1) - y(1 - x)}{y(x - (1 - x))} > 1
    \]
    \begin{align*}
        \implies \frac{y(p^\prime_{11} - x)}{1 - x} > \Phi_X
    \end{align*}
    So, when this holds we will get falsification. 
    \item When the upper bound is $\frac{(1 - x)(1 - y) - p_{10}(1 - x) + p^\prime_{11}y}{xy}$: Assume
     \[
     \frac{(1 - x)(1 - y) - p_{10}(1 - x) + p^\prime_{11}y}{xy} < \frac{ p^\prime_{11}y - (1 - x)(\Phi_X + y)}{y(x - (1 - x))}\\
     \]
     \begin{align*}
       &\implies (1 - y)(p^\prime_{10} - (1 - x)) < 0
     \end{align*}
     This creates a contradiction since the LHS is positive but the RHS is 0.
\end{enumerate}

So, when $1$ is the upper bound, the upper bound on PNS will be
\begin{align*}
    p_{11} - \Gamma = p_{11} - \frac{y(p^\prime_{11} - x)}{1 - x}
\end{align*}

And when $\frac{p_{11} - (1- y)}{y}$ is the lower bound, $\Gamma$ will evaluate to
\begin{align*}
    \Gamma &= (p_{11} - (1 - y))(OR(X) - 1) + \Phi_X + y - \frac{p^\prime_{11}y}{1 - x} \\
    &= \frac{(1 - y)(p^\prime_{10} - x)}{1 - x} 
\end{align*}

And the upper bound on PNS will be
\[
p_{11} - \Gamma = p_{11} - \frac{(1 - y)(p^\prime_{10} - x)}{1 - x} 
\]

\subsection{When $1 - x > x$}

Here, since the $OR(X)$ will be less than $1$, we need to recompute the turning points, which we do now. 
\begin{align*}
&yP(Z = 1\mid X = 1, Y = 1)(OR(X) - 1) + \Phi_X + y - \frac{p^\prime_{11}y}{1 - x} \geq \Phi_X\\    
&\implies  y - \frac{p^\prime_{11}y}{1 - x} \geq yP(Z = 1\mid X = 1, Y = 1)(1 - OR(X))\\
&\implies  1 - \frac{p^\prime_{11}}{1 - x} \geq \frac{P(Z = 1\mid X = 1, Y = 1)((1 - x)- x)}{1 - x}\\
&\implies  \frac{(1 - x) - p^\prime_{11}}{1 - x} \geq \frac{P(Z = 1\mid X = 1, Y = 1)((1 - x)- x)}{1 - x}\\
&\implies  \frac{(1 - x) - p^\prime_{11}}{(1 - x)- x} \geq P(Z = 1\mid X = 1, Y = 1)\\
\end{align*}

 We denote as (a). Next,            

\begin{align*}
    &P(Z = 1 \mid X = 1, Y = 1)(1 - OR(X))y + y\frac{p^\prime_{11} - (1 - x)}{1 - x} \geq \Phi_X\\
    &\implies P(Z = 1 \mid X = 1, Y = 1)(1 - OR(X))y  \geq \Phi_X - \frac{p^\prime_{11}y - y(1 - x)}{1 - x}\\
    &\implies P(Z = 1 \mid X = 1, Y = 1)(1 - OR(X))y  \geq \frac{\Phi_X(1 - x)}{1 - x} - \frac{p^\prime_{11}y - y(1 - x)}{1 - x}\\
    &\implies P(Z = 1 \mid X = 1, Y = 1)((1 - x) - x)y  \geq \Phi_X(1 - x) - p^\prime_{11}y + y(1 - x)\\
    &\implies P(Z = 1 \mid X = 1, Y = 1)  \geq \frac{\Phi_X(1 - x) - p^\prime_{11}y + y(1 - x)}{((1 - x) - x)y}\\
    &\implies P(Z = 1 \mid X = 1, Y = 1)  \geq \frac{(1 - x)(\Phi_X + y) - p^\prime_{11}y }{((1 - x) - x)y}\\
\end{align*}
             
And we denote this as (b). Now, we enumerate cases in a similar fashion as before. 


\subsubsection{Case I}

This case assumes the following
\begin{align}
    \Phi_X \geq 0\\
    x < 1 - x\\
    x < p^\prime_{11} < 1 - x\\
    p^\prime_{10} < x <  1- x
\end{align}

Here, the chosen bounds will be
\begin{align*}
    \max \begin{bmatrix}
        0\\
        \frac{p^\prime_{11}y - p_{10}(1 - x)}{xy}
    \end{bmatrix} \leq PNS \leq 
    \min \begin{bmatrix}
    1 \\
    \frac{p_{11}}{y}
    \end{bmatrix}
\end{align*}

Now, we check the upper and lower bounds against (a) and (b). 
\begin{enumerate}
    \item Lower bound is $0$: $0$ will be less than (a) since we assume $p^\prime_{11} < 1 - x$. 
    \item Lower bound is $\frac{p^\prime_{11}y - p_{10}(1 - x)}{xy}$: Assume
    \[
    \frac{p^\prime_{11}y - p_{10}(1 - x)}{xy} < \frac{(1 - x)(\Phi_X + y) - p^\prime_{11}y }{((1 - x) - x)y}
    \]
    \begin{align*}
        \implies 0 < (1 - y)(p^\prime_{10} - x)
    \end{align*}
    This is a contradiction since $p^\prime_{10} < x$. 
\end{enumerate}

Next, checking the upper bounds
\begin{enumerate}
    \item Upper bound of $1$: Checking this against (a), using a proof by contradiction. Assume
    \[
    \frac{(1 - x) - p^\prime_{11}}{(1 - x)- x} > 1
    \]
    \begin{align*}
        \implies p^\prime_{11} < x
    \end{align*}
    This is a contradiction.
    \item Upper bound is $\frac{p_{11}}{y}$: Following proof by contradiction, assume
    \[
    \frac{p_{11}}{y} < \frac{(1 - x) - p^\prime_{11}}{(1 - x)- x}
    \]
    \begin{align*}
        \implies (1 - x)\Phi_X < (1 - y)(p^\prime_{10} - (1 - x))
    \end{align*}
    This is a contradiction based on our assumptions.
\end{enumerate}
So, when $\frac{p^\prime_{11}y - p_{10}(1 - x)}{xy}$ is the lower bound, i.e. $p^\prime_{11}y > p_{10}(1 - x)$, we compute $\Gamma$ by inserting this lower bound into increasing function $P(Z = 1 \mid X = 1, Y = 1)(1 - OR(X))y + y\frac{p^\prime_{11} - (1 - x)}{1 - x}$. 
\begin{align*}
    \Gamma &=\frac{p^\prime_{11}y - p_{10}(1 - x)}{x}(1 - OR(X)) + y\frac{p^\prime_{11} - (1 - x)}{1 - x} \\
    \Gamma &= \Phi_X - \frac{(1 - y)(p^\prime_{10} - x)}{x}
\end{align*}

And the upper bound on PNS is computed as
\begin{align*}
    p_{11} - \Gamma &= p_{11} - \Phi_X + \frac{(1 - y)(p^\prime_{10} - x)}{x}\\
    &= p_{00} - \frac{(1 - y)(x - p^\prime_{10})}{x}\\
\end{align*}

\subsubsection{Case II}

\begin{align}
    \Phi_X \geq 0\\
    x < 1 - x\\
    x < p^\prime_{11} < 1 - x\\
    x < p^\prime_{10} <  1- x
\end{align}

Here, the chosen bounds will be
\begin{align*}
    \max \begin{bmatrix}
        0\\
        \frac{p_{11} - (1 - y)}{y}
    \end{bmatrix} \leq PNS \leq 
    \min \begin{bmatrix}
    1 \\
    \frac{p_{11}}{y}
    \end{bmatrix}
\end{align*}

Checking whether the lower bounds will be greater than (b) first. 
\begin{enumerate}
    \item Lower bound is $0$: $0$ will be less than (a) since we assume $p^\prime_{11} < 1 - x$. 
    \item Lower bound of $\frac{p_{11} - (1 - y)}{y}$: Following a proof by contradiction, assume
    \[
    \frac{p_{11} - (1 - y)}{y} > \frac{(1 - x)(\Phi_X + y) - p^\prime_{11}y }{((1 - x) - x)y}
    \]
    \begin{align*}
        \implies 0 > (1 - y)(p^\prime_{10} - x)
    \end{align*}
     Contradiction because $p^\prime_{10} > x$.
\end{enumerate}

Next, checking the upper bounds
\begin{enumerate}
    \item Upper bound of $1$: Checking this against (a), using a proof by contradiction. Assume
    \[
    \frac{(1 - x) - p^\prime_{11}}{(1 - x)- x} > 1
    \]
    \begin{align*}
        \implies p^\prime_{11} < x
    \end{align*}
    This is a contradiction.
    \item Upper bound is $\frac{p_{11}}{y}$: Following proof by contradiction, assume
    \[
    \frac{p_{11}}{y} < \frac{(1 - x) - p^\prime_{11}}{(1 - x)- x}
    \]
    \begin{align*}
        \implies (1 - x)\Phi_X < (1 - y)(p^\prime_{10} - (1 - x))
    \end{align*}
    This is a contradiction based on our assumptions.
\end{enumerate}

So no falsification will be observed in this case. 

\subsubsection{Case III}

\begin{align}
    \Phi_X \geq 0\\
    x < 1 - x\\
    x < p^\prime_{11} < 1 - x\\
    x <  1- x < p^\prime_{10}
\end{align}

Here, the chosen bounds will be
\begin{align*}
    \max \begin{bmatrix}
        0\\
        \frac{p_{11} - (1 - y)}{y}
    \end{bmatrix} \leq PNS \leq 
    \min \begin{bmatrix}
    1 \\
    \frac{(1 - x)(1 - y) - p_{10}(1 - x) + p^\prime_{11}y}{xy}
    \end{bmatrix}
\end{align*}

Checking whether the lower bounds will be greater than (b). 
\begin{enumerate}
    \item Lower bound on $0$: Using arguments before, this will be less than (b).
    \item Lower bound of $\frac{p_{11} - (1 - y)}{y}$: This generates a contradiction as before.
\end{enumerate}

So, neither of the lower bounds are capable of falsifying. Next, we move on to the upper bounds.

\begin{enumerate}
    \item Upper bound of $1$: Using the argument from Case II, we know this will be greater than (a).
    \item: Upper bound of $\frac{(1 - x)(1 - y) - p_{10}(1 - x) + p^\prime_{11}y}{xy}$: 
    \[
    \frac{(1 - x)(\Phi_X + y) - p^\prime_{11}y}{y((1 - x) - x)} < \frac{(1 - x) - p^\prime_{11}}{(1 - x) - x}
    \]
    \begin{align*}
        &\implies \Phi_X < \frac{(1 - y)(p^\prime_{10} - (1 - x))}{x}
    \end{align*}
    So, when the above condition holds, this can falsify.
\end{enumerate}

So when this is the upper bound, i.e. this condition holds
\begin{align*}
    p^\prime_{01}y > p_{00}(1 - x)    
\end{align*}
Then we can insert $\frac{(1 - x)(1 - y) - p_{10}(1 - x) + p^\prime_{11}y}{xy}$ into $P(Z = 1 \mid X = 1, Y = 1)y(OR(X) - 1) + \Phi_X + y - \frac{p^\prime_{11}y}{1 - x}$. to evaluate $\Gamma$ as 
\[
\Gamma = \frac{(1 - y)(p^\prime_{10} - (1 - x))}{x}
\]

And this gives the following upper bound on PNS as
\begin{align*}
    p_{11} - \Gamma = p_{11} - \frac{(1 - y)(p^\prime_{10} - (1 - x))}{x}
\end{align*}

\subsubsection{Case IV}

\begin{align}
    \Phi_X \geq 0\\
    x < 1 - x\\
    p^\prime_{11} < x <  1 - x\\
    x <  1- x < p^\prime_{10}
\end{align}
These constraints imply based on (\ref{p_111_bounds}) and the implications on Subsection \ref{implications_bounds_p111}, the following lower and upper bounds on $P(Z = 1 \mid X = 1, Y = 1)$: 
\begin{align*}
    \max\begin{bmatrix}
        0\\
        \frac{p_{11}-(1-y)}{y}
    \end{bmatrix} \leq P(Z = 1\mid X = 1, Y = 1) \leq 
    \min\begin{bmatrix}
        \frac{p^\prime_{11}}{x}\\
        \frac{(1-x)(1-y) - p_{10}(1-x) + p^\prime_{11}y}{xy}
    \end{bmatrix}
\end{align*}

Now we will check if each of the possible lower bounds are greater than (b).
\begin{enumerate}
    \item Lower bound is $0$: $0$ will be less than (a) since we assume $p^\prime_{11} < 1 - x$. 
    \item Lower bound of $\frac{p_{11} - (1 - y)}{y}$: Following a proof by contradiction, assume
    \[
    \frac{p_{11} - (1 - y)}{y} > \frac{(1 - x)(\Phi_X + y) - p^\prime_{11}y }{((1 - x) - x)y}
    \]
    \begin{align*}
        \implies 0 > (1 - y)(p^\prime_{10} - x)
    \end{align*}
     Contradiction because $p^\prime_{10} > x$.
\end{enumerate}

Now we will check if each of the possible upper bounds are less than (a). 
\begin{enumerate}
    \item Upper bound is $\frac{p^\prime_{11}}{x}$: Assume
    \[
    \frac{p^\prime_{11}}{x} > \frac{(1 - x) - p^\prime_{11}}{(1 - x) - x}
    \]
    \begin{align*}
        \implies x < p^\prime_{11}
    \end{align*}
    This is a contradiction, and so this lower bound is capable of falsifying.
    \item: Upper bound of $\frac{(1 - x)(1 - y) - p_{10}(1 - x) + p^\prime_{11}y}{xy}$: 
    \[
    \frac{(1 - x)(\Phi_X + y) - p^\prime_{11}y}{y((1 - x) - x)} < \frac{(1 - x) - p^\prime_{11}}{(1 - x) - x}
    \]
    \begin{align*}
        &\implies \Phi_X < \frac{(1 - y)(p^\prime_{10} - (1 - x))}{x}
    \end{align*}
    So, when the above condition holds, this can falsify.
\end{enumerate}

So now, $\Gamma$ will be evaluated for different values of upper bounds. When the upper bound is $\frac{p^\prime_{11}}{x}$, $\Gamma$ is evaluated as
\begin{align*}
    \Gamma &= \frac{p^\prime_{11}y}{x}(OR(X) - 1) + \Phi_X + y - \frac{p^\prime_{11}y}{1 - x}\\
    &= \Phi_X - \frac{y(p^\prime_{11} - x)}{x}\\
\end{align*}

And the upper bound on PNS is evaluated as
\begin{align*}
    p_{11} - \Gamma &= p_{11} - \Phi_X + \frac{y(p^\prime_{11} - x)}{x}\\
    p_{11} - \Gamma &= p_{00} - \frac{y(x - p^\prime_{11})}{x}\\
\end{align*}
When the upper bound is $\frac{(1-x)(1-y) - p_{10}(1-x) + p^\prime_{11}y}{xy}$, $\Gamma$ is evaluated as
\[
\Gamma = \frac{(1 - y)(p^\prime_{10} - (1 - x))}{x}
\]

And this gives the following upper bound on PNS as
\begin{align*}
    p_{11} - \Gamma = p_{11} - \frac{(1 - y)(p^\prime_{10} - (1 - x))}{x}
\end{align*}

\subsubsection{Case V: Atalanti}

\begin{align}
    \Phi_X \geq 0\\
    x < 1 - x\\
    p^\prime_{11} < x <  1 - x\\
    x < p^\prime_{10} < 1- x 
\end{align}
These constraints imply based on (\ref{p_111_bounds}) and the implications on Subsection \ref{implications_bounds_p111}, the following lower and upper bounds on $P(Z = 1 \mid X = 1, Y = 1)$: 
\begin{align*}
    \max\begin{bmatrix}
        0\\
        \frac{p_{11}-(1-y)}{y}
    \end{bmatrix} \leq P(Z = 1\mid X = 1, Y = 1) \leq 
    \min\begin{bmatrix}
    \frac{p_{11}}{y}\\
        \frac{p^\prime_{11}}{x}
    \end{bmatrix}
\end{align*}

Now we will check if each of the possible lower bounds are greater than $b$.
\begin{enumerate}
    \item Lower bound is $0$: $0$ will be less than (a) since we assume $p^\prime_{11} < 1 - x$. 
    \item Lower bound of $\frac{p_{11} - (1 - y)}{y}$: Following a proof by contradiction, assume
    \[
    \frac{p_{11} - (1 - y)}{y} > \frac{(1 - x)(\Phi_X + y) - p^\prime_{11}y }{((1 - x) - x)y}
    \]
    \begin{align*}
        \implies 0 > (1 - y)(p^\prime_{10} - x)
    \end{align*}
     Contradiction because $p^\prime_{10} > x$.
\end{enumerate}

Now we will check if each of the possible upper bounds are less than $a$. 
\begin{enumerate}
    \item Upper bound is $\frac{p_{11}}{y}$: Following proof by contradiction, assume
    \[
    \frac{p_{11}}{y} < \frac{(1 - x) - p^\prime_{11}}{(1 - x)- x}
    \]
    \begin{align*}
        \implies (1 - x)\Phi_X < (1 - y)(p^\prime_{10} - (1 - x))
    \end{align*}
    This is a contradiction based on our assumptions.
    \item Upper bound is $\frac{p^\prime_{11}}{x}$: Assume
    \[
    \frac{p^\prime_{11}}{x} > \frac{(1 - x) - p^\prime_{11}}{(1 - x) - x}
    \]
    \begin{align*}
        \implies x < p^\prime_{11}
    \end{align*}
    This is a contradiction, and so this lower bound is capable of falsifying.    
\end{enumerate}

When the upper bound is $\frac{p^\prime_{11}}{x}$, $\Gamma$ will evaluate to
\[
    \Gamma = \Phi_X - \frac{y(p^\prime_{11} - x)}{x}
\]

And the upper bound on PNS is evaluated as
\begin{align*}
    p_{11} - \Gamma &= p_{11} - \Phi_X + \frac{y(p^\prime_{11} - x)}{x}\\
    p_{11} - \Gamma &= p_{00} - \frac{y(p^\prime_{11} - x)}{x}\\
\end{align*}

\subsubsection{Case VI: Atalanti}

\begin{align}
    \Phi_X \geq 0\\
    x < 1 - x\\
    p^\prime_{11} < x <  1 - x\\
    p^\prime_{10} < x < 1- x 
\end{align}

These constraints imply based on (\ref{p_111_bounds}) and the implications on Subsection \ref{implications_bounds_p111}, the following lower and upper bounds on $P(Z = 1 \mid X = 1, Y = 1)$: 
\begin{align*}
    max\begin{bmatrix}
        0\\
        \frac{p^\prime_{11}y-p_{10}(1-x)}{xy}
    \end{bmatrix} \leq P(Z = 1\mid X = 1, Y = 1) \leq 
    min\begin{bmatrix}
    \frac{p_{11}}{y}\\
        \frac{p^\prime_{11}}{x}
    \end{bmatrix}
\end{align*}

Now we will check if each of the possible lower bounds are greater than $b$.
\begin{enumerate}
    \item $0 < b$ holds since $1 - x > p^\prime_{11}$ by assumption. 
    \item Lower bound is $\frac{p^\prime_{11}y - p_{10}(1 - x)}{xy}$: Assume
        \[
        \frac{p^\prime_{11}y - p_{10}(1 - x)}{xy} < \frac{(1 - x)(\Phi_X + y) - p^\prime_{11}y }{((1 - x) - x)y}
        \]
        \begin{align*}
            \implies 0 < (1 - y)(p^\prime_{10} - x)
        \end{align*}
        This is a contradiction since $p^\prime_{10} < x$, and so this lower bound can falsify. 
\end{enumerate}

Now we will check if each of the possible upper bounds are less than $a$. 
\begin{enumerate}
    \item Upper bound is $\frac{p_{11}}{y}$: Following proof by contradiction, assume
    \[
    \frac{p_{11}}{y} < \frac{(1 - x) - p^\prime_{11}}{(1 - x)- x}
    \]
    \begin{align*}
        \implies (1 - x)\Phi_X < (1 - y)(p^\prime_{10} - (1 - x))
    \end{align*}
    This is a contradiction based on our assumptions.
    \item Upper bound is $\frac{p^\prime_{11}}{x}$: Assume
    \[
    \frac{p^\prime_{11}}{x} > \frac{(1 - x) - p^\prime_{11}}{(1 - x) - x}
    \]
    \begin{align*}
        \implies x < p^\prime_{11}
    \end{align*}
    This is a contradiction, and so this lower bound is capable of falsifying.    
\end{enumerate}

So, when $\frac{p^\prime_{11}y - p_{10}(1 - x)}{xy}$ is the lower bound, i.e. $p^\prime_{11}y > p_{10}(1 - x)$ and $\Phi_X > \frac{(1 - y)(p^\prime_{10} - x)}{x}$, we compute $\Gamma$ by inserting this lower bound into increasing function $P(Z = 1 \mid X = 1, Y = 1)(1 - OR(X))y + y\frac{p^\prime_{11} - (1 - x)}{1 - x}$. 
\begin{align*}
    \Gamma &=\frac{p^\prime_{11}y - p_{10}(1 - x)}{x}(1 - OR(X)) + y\frac{p^\prime_{11} - (1 - x)}{1 - x} \\
    \Gamma &= \Phi_X - \frac{(1 - y)(p^\prime_{10} - x)}{x}
\end{align*}

And the upper bound on PNS is computed as
\begin{align*}
    p_{11} - \Gamma &= p_{11} - \Phi_X + \frac{(1 - y)(p^\prime_{10} - x)}{x}\\
    &= p_{00} - \frac{(1 - y)(x - p^\prime_{10})}{x}\\
\end{align*}

And when $\frac{p^\prime_{11}}{x}$ is the upper bound, $\Gamma$ will evaluate to
\[
    \Gamma = \Phi_X - \frac{y(p^\prime_{11} - x)}{x}
\]

And the upper bound on PNS is evaluated as
\begin{align*}
    p_{11} - \Gamma &= p_{11} - \Phi_X + \frac{y(p^\prime_{11} - x)}{x}\\
    p_{11} - \Gamma &= p_{00} - \frac{y(x - p^\prime_{11})}{x}\\
\end{align*}

\subsubsection{Case VII}

\begin{align}
    \Phi_X \geq 0\\
    x < 1 - x\\
    x <  1 - x < p^\prime_{11}\\
    p^\prime_{10} < x < 1- x 
\end{align}

These constraints imply based on (\ref{p_111_bounds}) and the implications on Subsection \ref{implications_bounds_p111}, the following lower and upper bounds on $P(Z = 1 \mid X = 1, Y = 1)$: 
\begin{align*}
    \max\begin{bmatrix}
        \frac{p^\prime_{11} - (1 - x)}{x}\\
        \frac{p^\prime_{11}y-p_{10}(1-x)}{xy}
    \end{bmatrix} \leq P(Z = 1\mid X = 1, Y = 1) \leq 
    min\begin{bmatrix}
    1\\
    \frac{p_{11}}{y}
    \end{bmatrix}
\end{align*}
Now we will check if each of the possible lower bounds are greater than $b$.
\begin{enumerate}
    \item $\frac{p^\prime_{11} - (1 - x)}{x} > \frac{(1 - x)(\Phi_X + y) - p^\prime_{11}y}{((1 - x) - x)y}$. This will hold when the following condition holds
    \[
    \Phi_X < \frac{y(p^\prime_{11} - (1 - x))}{x}
    \]
    \item Lower bound is $\frac{p^\prime_{11}y - p_{10}(1 - x)}{xy}$: Assume
        \[
        \frac{p^\prime_{11}y - p_{10}(1 - x)}{xy} < \frac{(1 - x)(\Phi_X + y) - p^\prime_{11}y }{((1 - x) - x)y}
        \]
        \begin{align*}
            \implies 0 < (1 - y)(p^\prime_{10} - x)
        \end{align*}
        This is a contradiction since $p^\prime_{10} < x$, and so this lower bound can falsify.
\end{enumerate}
Now we will check if each of the possible upper bounds are less than $a$. 
\begin{enumerate}
    \item Upper bound of $1$: Checking this against (a), using a proof by contradiction. Assume
    \[
    \frac{(1 - x) - p^\prime_{11}}{(1 - x)- x} > 1
    \]
    \begin{align*}
        \implies p^\prime_{11} < x
    \end{align*}
    This is a contradiction.
    \item Upper bound is $\frac{p_{11}}{y}$: Following proof by contradiction, assume
    \[
    \frac{p_{11}}{y} < \frac{(1 - x) - p^\prime_{11}}{(1 - x)- x}
    \]
    \begin{align*}
        \implies (1 - x)\Phi_X < (1 - y)(p^\prime_{10} - (1 - x))
    \end{align*}
    This is a contradiction based on our assumptions.
\end{enumerate}

So, when the lower bound is $\frac{p^\prime_{11} - (1 - x)}{x}$, $\Gamma$ will evaluate to
\begin{align*}
    \Gamma &= \frac{p^\prime_{11}y - y(1 - x)}{x}(1 - OR(X)) + \frac{p^\prime_{11}y - y(1 - x)}{1 - x}\\
    &= \frac{y(p^\prime_{11} - (1 - x))}{x}
\end{align*}

And so the upper bound on PNS will be
\begin{align*}
p_{11} - \Gamma =  p_{11} - \frac{y(p^\prime_{11} - (1 - x))}{x}
\end{align*}

Next, when the lower bound is $\frac{p^\prime_{11}y-p_{10}(1-x)}{xy}$, $\Gamma$ is computed by inserting this lower bound into increasing function $P(Z = 1 \mid X = 1, Y = 1)(1 - OR(X))y + y\frac{p^\prime_{11} - (1 - x)}{1 - x}$. 
\begin{align*}
    \Gamma &=\frac{p^\prime_{11}y - p_{10}(1 - x)}{x}(1 - OR(X)) + y\frac{p^\prime_{11} - (1 - x)}{1 - x} \\
    \Gamma &= \Phi_X - \frac{(1 - y)(p^\prime_{10} - x)}{x}
\end{align*}

And the upper bound on PNS is computed as
\begin{align*}
    p_{11} - \Gamma &= p_{11} - \Phi_X + \frac{(1 - y)(p^\prime_{10} - x)}{x}\\
    &= p_{00} - \frac{(1 - y)(x - p^\prime_{10})}{x}\\
\end{align*}

\subsubsection{Case VIII}

\begin{align}
    \Phi_X \geq 0\\
    x < 1 - x\\
    x <  1 - x < p^\prime_{11}\\
    x < p^\prime_{10} < 1- x 
\end{align}

These constraints imply based on (\ref{p_111_bounds}) and the implications on Subsection \ref{implications_bounds_p111}, the following lower and upper bounds on $P(Z = 1 \mid X = 1, Y = 1)$: 
\begin{align*}
    \max\begin{bmatrix}
        \frac{p^\prime_{11} - (1 - x)}{x}\\
        \frac{p_{11} - (1 - y)}{y}
    \end{bmatrix} \leq P(Z = 1\mid X = 1, Y = 1) \leq 
    \min\begin{bmatrix}
    1\\
    \frac{p_{11}}{y}
    \end{bmatrix}
\end{align*}

The same arguments as the previous case are utilized for the upper bounds, and consequently they cannot falsify. The same argument for $\frac{p^\prime_{11} - (1 - x)}{x}$ is used, and this can falsify. 

When the lower bound is $\frac{p_{11} - (1 - y)}{y}$, following a proof by contradiction, assume
    \[
    \frac{p_{11} - (1 - y)}{y} > \frac{(1 - x)(\Phi_X + y) - p^\prime_{11}y }{((1 - x) - x)y}
    \]
    \begin{align*}
        \implies 0 > (1 - y)(p^\prime_{10} - x)
    \end{align*}
     Contradiction because $p^\prime_{10} > x$

So, when the lower bound is $\frac{p^\prime_{11} - (1 - x)}{x}$, $\Gamma$ will evaluate to
\begin{align*}
    \Gamma &= \frac{p^\prime_{11}y - y(1 - x)}{x}(1 - OR(X)) + \frac{p^\prime_{11}y - y(1 - x)}{1 - x}\\
    &= \frac{y(p^\prime_{11} - (1 - x))}{x}
\end{align*}

And so the upper bound on PNS will be
\begin{align*}
p_{11} - \Gamma =  p_{11} - \frac{y(p^\prime_{11} - (1 - x))}{x}
\end{align*}

\subsubsection{Case IX}

\begin{align}
    \Phi_X \geq 0\\
    x < 1 - x\\
    x <  1 - x < p^\prime_{11}\\
    x < 1- x < p^\prime_{10}
\end{align}

These constraints imply based on (\ref{p_111_bounds}) and the implications on Subsection \ref{implications_bounds_p111}, the following lower and upper bounds on $P(Z = 1 \mid X = 1, Y = 1)$: 
\begin{align*}
    \max\begin{bmatrix}
        \frac{p^\prime_{11} - (1 - x)}{x}\\
        \frac{p_{11} - (1 - y)}{y}
    \end{bmatrix} \leq P(Z = 1\mid X = 1, Y = 1) \leq 
    \min\begin{bmatrix}
    1\\
    \frac{(1-x)(1-y) - p_{10}(1-x) + p^\prime_{11}y}{xy}
    \end{bmatrix}
\end{align*}

The same arguments from the above case are used for the lower bounds, with the conclusion that $\frac{p^\prime_{11} - (1 - x)}{x}$ is capable of inducing falsification. 

Following the same argument as Case VII for $1$, it is incapable of falsifying. However, $\frac{(1-x)(1-y) - p_{10}(1-x) + p^\prime_{11}y}{xy}$ is capable of falsifying. 
    When the upper bound is $\frac{(1 - x)(1 - y) - p_{10}(1 - x) + p^\prime_{11}y}{xy}$, 
    \[
    \frac{(1 - x)(\Phi_X + y) - p^\prime_{11}y}{y((1 - x) - x)} < \frac{(1 - x) - p^\prime_{11}}{(1 - x) - x}
    \]
    \begin{align*}
        &\implies \Phi_X < \frac{(1 - y)(p^\prime_{10} - (1 - x))}{x}
    \end{align*}
    So, when the above condition holds, this can falsify.
So, when the lower bound is $\frac{p^\prime_{11} - (1 - x)}{x}$, $\Gamma$ will evaluate to
\begin{align*}
    \Gamma &= \frac{p^\prime_{11}y - y(1 - x)}{x}(1 - OR(X)) + \frac{p^\prime_{11}y - y(1 - x)}{1 - x}\\
    &= \frac{y(p^\prime_{11} - (1 - x))}{x}
\end{align*}

And so the upper bound on PNS will be
\begin{align*}
p_{11} - \Gamma =  p_{11} - \frac{y(p^\prime_{11} - (1 - x))}{x}
\end{align*}

When the upper bound is $\frac{(1-x)(1-y) - p_{10}(1-x) + p^\prime_{11}y}{xy}$, $\Gamma$ is evaluated as
\[
\Gamma = \frac{(1 - y)(p^\prime_{10} - (1 - x))}{x}
\]

And this gives the following upper bound on PNS as
\begin{align*}
    p_{11} - \Gamma = p_{11} - \frac{(1 - y)(p^\prime_{10} - (1 - x))}{x}
\end{align*}

\section{Enumerating The Set Of Joint Distributions Compatible With Observed Marginals When $Y$ is Discrete And Multi-Valued}

For the graph shaped in \ref{fig:causal-graph}, we can enumerate the following equations for the $P(Z, X, Y)$
{\scriptsize
\begin{align*}
    \mathbb{P}(Z = 1 \mid X = 1) &= \mathbb{P}(Z = 1 \mid X = 1, Y = 0)\mathbb{P}(Y = 0) + \mathbb{P}(Z = 1 \mid X = 1, Y = 1)\mathbb{P}(Y = 1) + \mathbb{P}(Z = 1 \mid X = 1, Y = 2)\mathbb{P}(Y = 2)\\
    \mathbb{P}(Z = 1 \mid X = 0) &= \mathbb{P}(Z = 1 \mid X = 0, Y = 1)\mathbb{P}(Y = 1) + \mathbb{P}(Z = 1 \mid X = 0, Y = 0)\mathbb{P}(Y = 0) + \mathbb{P}(Z = 1 \mid X = 0, Y = 2)\mathbb{P}(Y = 2)\\
    \mathbb{P}(Z = 1 \mid Y = 1) &= \mathbb{P}(Z = 1 \mid X = 0, Y = 1)\mathbb{P}(X = 0) + \mathbb{P}(Z = 1 \mid X = 1, Y = 1)\mathbb{P}(X = 1)\\
    \mathbb{P}(Z = 1 \mid Y = 0) &= \mathbb{P}(Z = 1 \mid X = 0, Y = 0)\mathbb{P}(X = 0) + \mathbb{P}(Z = 1 \mid X = 1, Y = 0)\mathbb{P}(X = 1)\\
    \mathbb{P}(Z = 1 \mid Y = 2) &= \mathbb{P}(Z = 1 \mid X = 0, Y = 2)\mathbb{P}(X = 0) + \mathbb{P}(Z = 1 \mid X = 1, Y = 2)\mathbb{P}(X = 1)\\
\end{align*}
}

Putting this in RREF, we get
\begin{align*}
    \begin{bmatrix}
    1 &  0 &  0 &  -\frac{x*y_1}{(1 - x)*(1 - y_1 - y_2)} &  0 &  -\frac{x*y_2}{(1 - x)*(1 - y_1 - y_2)} & \frac{p^\prime_{10}(1 - x) - p^\prime_{11}y_1 - p^\prime_{12}y_2}{(1 - x)(1 - y_1  - y_2)}\\
    0 &  1 &  0 & \frac{y_1}{1 - y_1 - y_2} &  0 & \frac{y_2}{1 - y_1 - y_2} & \frac{p_{11}}{1 - y_1 - y_2}\\
    0 &  0 &  1 & \frac{x}{1 - x} &  0 &  0 & \frac{p^\prime_{11}}{1 - x}\\
    0 &  0 &  0 & 0 &  1 & \frac{x}{1 - x} & \frac{p^\prime_{12}}{1 - x}
    \end{bmatrix}
\end{align*}

And this can equivalently be represented in equation form using the free parameters $P(Z = 1 \mid X = 1, Y = 1)$ and $P(Z = 1 \mid X = 1, Y = 2)$ as
{\scriptsize
\begin{align}
    &\mathbb{P}(Z = 1 \mid X = 0, Y = 0) - OR(X)\frac{y_1}{1 - y_1 - y_2}\mathbb{P}(Z = 1 \mid X = 1, Y = 1) - OR(X)\frac{y_2}{1 - y_1 - y_2}\mathbb{P}(Z = 1 \mid X = 1, Y = 2)\\
    &=  \frac{p_{10}(1 - x) - p^\prime_{11}y_1 - p^\prime_{12}y_2}{(1 - x)(1 - y_1 - y_2)}
\end{align}
\begin{equation}
    \mathbb{P}(Z = 1 \mid X = 1, Y = 0) + \frac{y_1}{1 - y_1 - y_2}\mathbb{P}(Z = 1 \mid X = 1, Y = 1) + \frac{y_2}{1 - y_1 - y_2}\mathbb{P}(Z = 1 \mid X = 1, Y = 2) = \frac{p_{11}}{1 - y_1 - y_2}
\end{equation}
\begin{equation}
    \mathbb{P}(Z = 1 \mid X = 0, Y = 1) + OR(X)\mathbb{P}(Z = 1 \mid X = 1, Y = 1) = \frac{p^\prime_{11}}{ 1- x}
\end{equation}    
\begin{equation}
    \mathbb{P}(Z = 1 \mid X = 0, Y = 2) + OR(X)\mathbb{P}(Z = 1 \mid X = 1, Y = 2) = \frac{p^\prime_{12}}{ 1- x}
\end{equation}    
}
Consequently, each of the joint probabilities can be expressed in terms of the free parameters as follows:
{\scriptsize
\begin{align*}
\mathbb{P}(Z = 1 \mid X = 0, Y = 0) &=  OR(X)\frac{y_1}{1 - y_1 - y_2}\mathbb{P}(Z = 1 \mid X = 1, Y = 1)\\
&+ OR(X)\frac{y_2}{1 - y_1 - y_2}\mathbb{P}(Z = 1 \mid X = 1, Y = 2)\\
&+ \frac{p_{10}(1 - x) - p^\prime_{11}y_1 - p^\prime_{12}y_2}{(1 - x)(1 - y_1 - y_2)}\\
\mathbb{P}(Z = 1 \mid X = 1, Y = 0)&= \frac{p_{11}}{1 - y_1 - y_2}\\
& - \frac{y_1}{1 - y_1 - y_2}\mathbb{P}(Z = 1 \mid X = 1, Y = 1)\\
&- \frac{y_2}{1 - y_1 - y_2}\mathbb{P}(Z = 1 \mid X = 1, Y = 2) \\
\mathbb{P}(Z = 1 \mid X = 0, Y = 1)&= \frac{p^\prime_{11}}{ 1- x} - OR(X)\mathbb{P}(Z = 1 \mid X = 1, Y = 1)\\
\mathbb{P}(Z = 1 \mid X = 0, Y = 2)&= \frac{p^\prime_{12}}{ 1- x} - OR(X)\mathbb{P}(Z = 1 \mid X = 1, Y = 2)
\end{align*}
}
Since every variable in the equations above is a probability, these expression imply bounds on $P(Z = 1 \mid X = 1, Y = 1)$ and $p(Z = 1 \mid X = 1, Y = 2)$ to ensure all values are between $0$ and $1$.

Starting with bounds implied by $P(Z = 1\mid X = 0, Y = 1)$:
\begin{align*}
    0 \leq P(Z = 1\mid X = 0, Y = 1) &\leq 1 \implies 0 \leq \frac{p^\prime_{11}}{ 1- x} - OR(X)\mathbb{P}(Z = 1 \mid X = 1, Y = 1) \leq 1\\
    \min\begin{bmatrix}
        0\\
        \frac{p^\prime_{11} - (1 - x)}{x}
    \end{bmatrix} &\leq P(Z = 1 \mid X = 1, Y = 1) \leq 
    \max\begin{bmatrix}
        1\\
        \frac{p^\prime_{11}}{x}
    \end{bmatrix}
\end{align*}

Similarly, the bounds implied on $P(Z = 1 \mid X = 1, Y = 1)$ will be
\begin{align*}
    \min\begin{bmatrix}
        0\\
        \frac{p^\prime_{12} - (1 - x)}{x}
    \end{bmatrix} &\leq P(Z = 1 \mid X = 1, Y = 2) \leq 
    \max\begin{bmatrix}
        1\\
        \frac{p^\prime_{12}}{x}
    \end{bmatrix}
\end{align*}

Next, the remaining free parameters will imply constraints on the weighted sums of $P(Z = 1 \mid X = 1, Y = 1)$ and $P(Z = 1 \mid X = 1, Y = 2)$, which we present below. 
\begin{align*}
    0 &\leq \mathbb{P}(Z = 1 \mid X = 0, Y = 0) \leq 1\\
    \implies 0 &\leq OR(X)\frac{y_1}{1 - y_1 - y_2}\mathbb{P}(Z = 1 \mid X = 1, Y = 1)\\
&+ OR(X)\frac{y_2}{1 - y_1 - y_2}\mathbb{P}(Z = 1 \mid X = 1, Y = 2)\\
&+ \frac{p_{10}(1 - x) - p^\prime_{11}y_1 - p^\prime_{12}y_2}{(1 - x)(1 - y_1 - y_2)} \leq 1\\
&\implies \frac{p^\prime_{11}y_1 + p^\prime_{11}y_2 - p_{10}(1 - x)}{x}\\
& \leq y_1 P(Z = 1 \mid X = 1, Y = 1) + y_2 P(Z = 1 \mid X = 1, Y = 2)\\
&\leq \frac{(1 - x)(1 - y_1 - y_2) - p_{10}(1 - x) + p^\prime_{11}y_1 + p^\prime_{12}y_2}{x}
\end{align*}

Similarly, 
\begin{align*}
    &0 \leq \mathbb{P}(Z = 1 \mid X = 1, Y = 0) \leq 1\\
    &\implies 0 \leq  \frac{p_{11}}{1 - y_1 - y_2} - \frac{y_1}{1 - y_1 - y_2}\mathbb{P}(Z = 1 \mid X = 1, Y = 1) - \frac{y_2}{1 - y_1 - y_2}\mathbb{P}(Z = 1 \mid X = 1, Y = 2) \leq 1\\
    &\implies p_{11} - (1 - y_1 - y_2) \leq y_1 P(Z = 1 \mid X = 1, Y = 1) + y_2 P(Z = 1 \mid X = 1, Y = 2) \leq p_{11}
\end{align*}

Putting these together, we have the following bounds on the weighted sum:
\begin{align*}
    \max\begin{bmatrix}
        \frac{p^\prime_{11}y_1 + p^\prime_{11}y_2 - p_{10}(1 - x)}{x}\\
        p_{11} - (1 - y_1 - y_2)
    \end{bmatrix} \leq y_1 P(Z = 1 \mid X = 1, Y = 1) + y_2 P(Z = 1 \mid X = 1, Y = 2) \\\leq 
    \min\begin{bmatrix}
        \frac{(1 - x)(1 - y_1 - y_2) - p_{10}(1 - x) + p^\prime_{11}y_1 + p^\prime_{12}y_2}{x}\\
        p_{11}
    \end{bmatrix}
\end{align*}
\subsection{Evaluating $\Gamma$ And $\Delta$}
Next, we compute each of the values of the max operator.
\begin{enumerate}
    \item $\mathbb{P}(Y = 0)\{\mathbb{P}(Z = 1 \mid X = 1, Y = 0) - \mathbb{P}(Z = 0 \mid X = 0, Y = 0)\}$: This is equal to 
    {\scriptsize
    \begin{align*}
        &(1 - y_1 - y_2)(\frac{p_{11}}{1 - y_1 - y_2} - \frac{y_1}{1 - y_1 - y_2}\mathbb{P}(Z = 1 \mid X = 1, Y = 1) - \frac{y_2}{1 - y_1 - y_2}\mathbb{P}(Z = 1 \mid X = 1, Y = 2))\\
        &- (1 - y_1 - y_2)(1 - (OR(X)\frac{y_1}{1 - y_1 - y_2}\mathbb{P}(Z = 1 \mid X = 1, Y = 1)  + OR(X)\frac{y_2}{1 - y_1 - y_2}\mathbb{P}(Z = 1 \mid X = 1, Y = 2) + \frac{p_{10}(1 - x) - p^\prime_{11}y_1 - p^\prime_{12}y_2}{(1 - x)(1 - y_1 - y_2)}))\\
        &= \Phi_X + (y_1 + y_2) + (OR(X) - 1)(y_1P(Z = 1 \mid X = 1, Y = 1) + y_2P(Z = 1\mid X = 1, Y = 2)) - \frac{p^\prime_{11}y_1 + p^\prime_{12}y_2}{1 - x}
    \end{align*}
    }
    \item $\mathbb{P}(Y = 1)\{\mathbb{P}(Z = 1 \mid X = 1, Y = 1) - \mathbb{P}(Z = 0 \mid X = 0, Y = 1)\}$
    This is equal to
    \begin{align*}
        y_1P(Z = 1 \mid X = 1, Y = 1)(1 - OR(X)) + \frac{y_1p^\prime_{11} - y_1(1 - x)}{1 - x}
    \end{align*}
    \item $\mathbb{P}(Y = 2)\{\mathbb{P}(Z = 1 \mid X = 1, Y = 2) - \mathbb{P}(Z = 0 \mid X = 0, Y = 2)\}$
    This evaluates to
    \[
        y_2P(Z = 1 \mid X = 1, Y = 2)(1 - OR(X)) + \frac{y_2p^\prime_{12} - y_2(1 - x)}{1 - x}
    \]
\end{enumerate}

\section{Generalizing The Causal Marginal Problem With Observed Covariates}

Now, since the next level of generality involves dealing with observed covariates, we consider the following setting. Consider binary random variables $Z$, $X$ and $Y$, and some observed covariates $C$ arranged in the following graph. We are given access to the marginals $P(Z, X, C)$ and $P(Z, Y, C)$ and want to tighten bounds on the PNS involving $X \rightarrow C$. In this case, the benchmark will be the bounds in Section 1, given as

\begin{align*}
    \Delta \leq PNS \leq \mathbb{P}(Z = 1 \mid X = 1) - \Gamma
\end{align*}

Where
\begin{equation*}
    \Delta = \sum_y \mathbb{P}(Y = y)\max \{0, \mathbb{P}(Z = 1 \mid X = 1, Y = y) - \mathbb{P}(Z = 1 \mid X = 0, Y = y)\} 
\end{equation*}

Now, to apply a similar method as before, we must derive the bounds on PNS if we had access to $P(Z, X, Y, C)$. The derivation of these bounds is given as follows:


\input{tikz_figures/trident_graph}

Before solving the problem of dealing with covariates with arbitrary dimensionality, we start by solving a simpler case. Suppose both distributions now observe a binary covariate $C$, and we solve an analogous problem. We are given marginals $\mathbb{P}(Z, X, C)$ and $\mathbb{P}(Z, Y, C)$ and we want the conditionals $\mathbb{P}(Z = 1 \mid X, Y , C)$.

\subsection{Bounds On PNS With Access to $P(Z , X, Y, C)$}

To update bounds on PNS, we start by noting
{\small
\begin{align*}
    \max\{0, P(Z_{\mathbf{x}} = 1, C, Y) - P(Z_{\mathbf{x^\prime}} = 1, C, Y)\} \leq P(Z_{\mathbf{x}} = 1, Z_{\mathbf{x^\prime}} = 0, C, Y) \leq \min \{P(Z_{\mathbf{x}} = 1, C, Y), P(Z_{\mathbf{x^\prime}} = 0, C, Y) \}
\end{align*}
}

Now, marginalizing out $C$ and $Y$ we have
{\small
\begin{align*}
    &\sum_{C, Y}\max\{0, P(Z_{\mathbf{x}} = 1, C, Y) - P(Z_{\mathbf{x^\prime}} = 1, C, Y)\} \leq P(Z_{\mathbf{x}} = 1, Z_{\mathbf{x^\prime}} = 0) \leq \sum_{C, Y} \max \{P(Z_{\mathbf{x}} = 1, C, Y), P(Z_{\mathbf{x^\prime}} = 0, C, Y) \}\\
    &\sum_{C, Y}P(C, Y)\max\{0, P(Z = 1 \mid X = 1, C, Y) - P(Z = 1 \mid X = 0, C, Y)\} \leq P(Z_{\mathbf{x}} = 1, Z_{\mathbf{x^\prime}} = 0)\\
    &P(Z_{\mathbf{x}} = 1, Z_{\mathbf{x^\prime}} = 0) \leq \sum_{C, Y} P(C, Y)\max \{P(Z = 1 \mid X = 1, C, Y), P(Z = 0 \mid X = 0, C, Y) \}
\end{align*}
}

Exploiting the independence of $C$ and $Y$, we can write the above as 
 \begin{align*}
    &\sum_{C, Y}P(C) P(Y)\max\{0, P(Z = 1 \mid X = 1, C, Y) - P(Z = 1 \mid X = 0, C, Y)\} \leq P(Z_{\mathbf{x}} = 1, Z_{\mathbf{x^\prime}} = 0)\\
    &P(Z_{\mathbf{x}} = 1, Z_{\mathbf{x^\prime}} = 0) \leq \sum_{C, Y} P(C)P(Y)\max \{P(Z = 1 \mid X = 1, C, Y), P(Z = 0 \mid X = 0, C, Y) \}
\end{align*}   

\textcolor{red}{Need to examine the properties of these bounds? Are they tight? When are they tighter than the marginal bounds on PNS? Does adding more $C$'s help etc}


\section{Extra Stuff}
We start by proving the lower bound and express $\Delta$ in terms of the free parameter $P(Z = 1 \mid X = 1, Y = 1)$ as follows. First, in this binary case, $\Delta$ is given as 
\begin{align*}
    \Delta = &\mathbb{P}(Y = 0)\max \{0, \mathbb{P}(Z = 1 \mid X = 1, Y = 0) - \mathbb{P}(Z = 1 \mid X = 0, Y = 0)\} \\
    &+ \mathbb{P}(Y = 1)\max \{0, \mathbb{P}(Z = 1 \mid X = 1, Y = 1) - \mathbb{P}(Z = 1 \mid X = 0, Y = 1)\} 
\end{align*}

Consequently, each of the non-zero terms inside the max operator are expressed in terms of the free parameter as follows

\begin{enumerate}
    \item $\mathbb{P}(Z = 1 \mid X = 1, Y = 0) - \mathbb{P}(Z = 1 \mid X = 0, Y = 0)$
    Substituting the expression of $P(Z = 1 \mid X = 1, Y = 0)$ and $P(Z = 1 \mid X = 0, Y = 0)$ in terms of $P(Z = 1 \mid X = 1, Y = 1)$ we get
    \begin{align*}
    &\mathbb{P}(Z = 1 \mid X = 1, Y = 0) - \mathbb{P}(Z = 1 \mid X = 0, Y = 0) = \\
    &\frac{p_{11} - p^\prime_{10}y_0 - y_1\mathbb{P}(Z = 1\mid X = 1, Y = 1)}{(1 - x)y_0}  
\end{align*} 

\item $\mathbb{P}(Z = 1 \mid X = 1, Y = 1) - \mathbb{P}(Z = 1 \mid X = 0, Y = 1)$
    \begin{align*}
        &\mathbb{P}(Z = 1 \mid X = 1, Y = 1) - \mathbb{P}(Z = 1 \mid X = 0, Y = 1) = \\
        &\frac{\mathbb{P}(Z = 1 \mid X = 1, Y = 1) - p^\prime_{11}}{1 - x}
    \end{align*}
\end{enumerate}

The lower bound is obtained by computing 
\begin{align*}
    &\min_{P(Z = 1\mid X = 1, Y = 1)} \Delta(P(Z = 1 \mid X = 1, Y = 1)) = \\
    &\min_{P(Z = 1\mid X = 1, Y = 1)} \Bigg\{y_0\max\Big\{0, \frac{p_{11} - p^\prime_{10}y_0 - y_1\mathbb{P}(Z = 1\mid X = 1, Y = 1)}{(1 - x)y_0}  \Big\}\\
    + &y_1\max\Big\{0, \frac{\mathbb{P}(Z = 1 \mid X = 1, Y = 1) - p^\prime_{11}}{1 - x}\Big\}\Bigg\}
\end{align*}


Next, we identify the the values of $P(Z = 1 \mid X = 1, Y = 1)$ for which the second term of each of the max operators is larger than zero. 
\begin{enumerate}
    \item $\max\Big\{0, \frac{p_{11} - p^\prime_{10}y_0 - y_1\mathbb{P}(Z = 1\mid X = 1, Y = 1)}{(1 - x)y_0}  \Big\}$
    \begin{align*}
        &0 < \frac{p_{11} - p^\prime_{10}y_0 - y_1\mathbb{P}(Z = 1\mid X = 1, Y = 1)}{(1 - x)y_0}\\
        &\implies P(Z = 1 \mid X = 1, Y = 1) < \frac{p_{11} - p^\prime_{10}y_0}{y_1}
    \end{align*}

    \item $\max\Big\{0, \frac{\mathbb{P}(Z = 1 \mid X = 1, Y = 1) - p^\prime_{11}}{1 - x}\Big\}$
    \begin{align*}
        \frac{\mathbb{P}(Z = 1 \mid X = 1, Y = 1) - p^\prime_{11}}{1 - x} > 0\\
        \implies p^\prime_{11} < P(Z = 1 \mid X = 1, Y = 1)
    \end{align*}
\end{enumerate}

Now, we check whether both max operators can open with non-zero terms at the same time, i.e. $p^\prime_{11} < P(Z = 1 \mid X = 1, Y = 1) < \frac{p_{11} - p^\prime_{10}y_0}{y_1}$
\begin{align*}
    p^\prime_{11} &< \frac{p_{11} - p^\prime_{10}y_0}{y_1}\\
    p^\prime_{11}y_1 + p^\prime_{10}y_0 &< p_{11}\\
    \implies 0 &< p_{11} - p_{10}
\end{align*}

Therefore, both max can open when $p_{11} - p_{10} > 0$. 

First, assume $p_{11} - p_{10} \leq 0$, then $p^\prime_{11} \geq \frac{p_{11} - p^\prime_{10}y_0}{y_1}$ then both max operators cannot open with non-zero terms at the same time. So we can consider the max operator separately. 

\begin{enumerate}
    \item Does the range of $P(Z = 1\mid X = 1, Y = 1)$ always allow $\max\Big\{0, \frac{\mathbb{P}(Z = 1 \mid X = 1, Y = 1) - p^\prime_{11}}{1 - x}\Big\}$ to open as non-zero: This requires $p^\prime_{11} < P(Z = 1 \mid X = 1, Y = 1)$ to hold for all allowed values of $P(Z = 1 \mid X =1, Y = 1)$. Since we have the minimum over $P(Z = 1\mid X = 1, Y = 1)$ outside the max operator, this max operator can only open if the entire range of $P(Z = 1 \mid X = 1, Y = 1)$ allowed will always be greater than $p^\prime_{11}$. This translates to checking whether the lower bounds of $P(Z = 1 \mid X = 1, Y = 1)$ will always be greater than $p^\prime_{11}$. Using Lemma \ref{lemma:free-param-bounds}, the set of possible lower bounds on $P(Z = 1 \mid X = 1, Y = 1)$ will be
    \begin{align*}
        \max\begin{bmatrix}
            0\\
            \frac{p^\prime_{11} - (1 - x)}{x}\\
            \frac{p_{11} - y_0}{y_1}\\
            \frac{p_{11}x - p^\prime_{10}y_0}{xy_1}
        \end{bmatrix} \leq P(Z = 1 \mid X = 1, Y = 1)
    \end{align*}
    We utilize a proof by contradiction to show each of the lower bounds cannot be greater than $p^\prime_{11}$. 
    \begin{enumerate}
        \item The lower bound is $0$: Since $p^\prime_{11}$ is a probability, it cannot be less than $0$. Hence $p^\prime_{11} \geq 0$
        \item The lower bound is $\frac{p^\prime_{11} - (1 - x)}{x}$: 
        \begin{align*}
            \frac{p^\prime_{11} - (1 - x)}{x} &> p^\prime_{11}\\
            \implies p^\prime_{11} &> 1
        \end{align*}
        This is a contradiction from the properties of probability, hence 
        \[
        \frac{p^\prime_{11} - (1 - x)}{x} \leq p^\prime_{11}
        \]
        \item If the lower bound is $\frac{p_{11} - y_0}{y_1}$: Assume
        \begin{align*}
            \frac{p_{11} - y_0}{y_1} &> p^\prime_{11}\\
            \implies (1 - x)(p_{11} - p_{10}) > y_0p^\prime_{00}
        \end{align*}
        This is a contradiction since $p_{11} - p_{10} \leq 0$, hence 
        \[
            \frac{p_{11} - y_0}{y_1} \leq p^\prime_{11}
        \]
        \item The lower bound is $\frac{p_{11}x - p^\prime_{10}y_0}{xy_1}$: Assume 
        \begin{align*}
            \frac{p_{11}x - p^\prime_{10}y_0}{xy_1} &> p^\prime_{11}\\
            \implies p_{11} - p_{10} > p^\prime_{10}y_0
        \end{align*}
        And this is a contradiction as well for the same reasons as before, hence
        \[
            \frac{p_{11}x - p^\prime_{10}y_0}{xy_1} \leq p^\prime_{11}\\
        \]
    \end{enumerate}
    \item $\max\Big\{0, \frac{p_{11} - p^\prime_{10}y_0 - y_1\mathbb{P}(Z = 1\mid X = 1, Y = 1)}{(1 - x)y_0}  \Big\}$: This requires $P(Z = 1 \mid X = 1, Y = 1) < \frac{p_{11} - p^\prime_{10}y_0}{y_1}$. Following a similar argument as above, we need the upper bound on $P(Z = 1 \mid X = 1, Y = 1)$ to be less than $\frac{p_{11} - p^\prime_{10}y_0}{y_1}$. Following a proof by contradiction as before, we enumerate the choices of bounds. 
    \begin{enumerate}
        \item The upper bound is $1$: Assume
        \begin{align*}
            1 &< \frac{p_{11} - p^\prime_{10}y_0}{y_1}\\
            y_1 &< p_{11} - p_{11}x - p_{10}(1 - x) + p^\prime_{11}y_1\\
            \implies& y_1p^\prime_{01} < (1 - x)(p_{11} - p_{10})
        \end{align*}
        This is a contradiction as well, hence
        \[
        1 \geq \frac{p_{11} - p^\prime_{10}y_0}{y_1}
        \]
        \item The upper bound is $\frac{p^\prime_{11}}{x}$: Assume
        \begin{align*}
            \frac{p^\prime_{11}}{x} &< \frac{p_{11} - p^\prime_{10}y_0}{y_1}\\
            \implies& (1 - x)p^\prime_{11}y_1 < (1 - x)(p_{11} - p_{10})
        \end{align*}
        This is a contradiction, hence 
        \[
            \frac{p^\prime_{11}}{x} \geq \frac{p_{11} - p^\prime_{10}y_0}{y_1}
        \]
        \item The upper bound is $\frac{p_{11}}{y_1}$: Assume
        \begin{align*}
            \frac{p_{11}}{y_1} &< \frac{p_{11} - p^\prime_{10}y_0}{y_1}\\
            \implies & 0 < -\frac{p^\prime_{10}y_0}{y_1}
        \end{align*}
        This is a contradiction, hence
        \[
            \frac{p_{11}}{y_1} \geq \frac{p_{11} - p^\prime_{10}y_0}{y_1}
        \]
        \item The upper bound is $\frac{(1 - x)y_0 + p_{11}x - p^\prime_{10}y_0}{x}$: Assume
        \begin{align*}
            \frac{p_{11} - p^\prime_{10}y_0}{y_1} &> \frac{(1 - x)y_0 + p_{11}x - p^\prime_{10}y_0}{xy_1}\\
            p_{11} - p^\prime_{10}y_0 &> \frac{(1 - x)y_0 + p_{11}x - p^\prime_{10}y_0}{x}\\
            p_{11}x - p^\prime_{10}xy_0 &> (1 - x)y_0 + p_{11}x - p^\prime_{10}y_0\\
            - p^\prime_{10}xy_0 &> (1 - x)y_0 - p^\prime_{10}y_0\\
            p^\prime_{10}y_0(1 - x) &> (1 - x)y_0 \\
            \implies p^\prime_{10} &> 1 \\
        \end{align*}
        This is a contradiction, hence
        \[
            \frac{p_{11} - p^\prime_{10}y_0}{y_1} \leq \frac{(1 - x)y_0 + p_{11}x - p^\prime_{10}y_0}{xy_1}
        \]
    \end{enumerate}
\end{enumerate}

Since we have shown that the lower bound of $P(Z = 1\mid X = 1, Y = 1)$ is always less than $p^\prime_{11}$ and the upper bound is always greater than $\frac{p_{11} - p^\prime_{10}y_0}{y_1}$, there will always be a value of $P(Z = 1\mid X = 1, Y = 1)$ allowed such that both max operators open as $0$. 

Next, we assume that $p_{11} - p_{10} > 0$. Note that using a proof by contradiction,
\[
p_{11} - p_{10} \leq 0 \implies p^\prime_{11} < \frac{p_{11} - p^\prime_{10}y_0}{y_1}
\]
Now, we check whether the allowed ranges of $P(Z = 1 \mid X = 1, Y = 1)$ allow for the max operators to open with non-zero terms, i.e. whether the lower bound is greater than $\frac{p_{11} - p^\prime_{10}y_0}{y_1}$ or if the upper bound is less than $p^\prime_{11}$
\begin{enumerate}
    \item Checking whether the lower bound is greater than $\frac{p_{11} - p^\prime_{10}y_0}{y_1}$: We utilize a proof by contradiction, presented on a case by case basis for each lower bound.
    \begin{enumerate}
        \item The lower bound is $0$: Assume 
        \begin{align*}
            & 0 > \frac{p_{11} - p^\prime_{10}y_0}{y_1}\\
            & \implies -p^\prime_{11}y_1 > (1 - x)(p_{11} - p_{10})
        \end{align*}
        This is a contradiction since the LHS is negative and the RHS is positive, Hence
        \[
        0 \leq \frac{p_{11} - p^\prime_{10}y_0}{y_1}
        \]
        \item The lower bound is $\frac{p^\prime_{11} - (1 - x)}{x}$: Assume
            \begin{align*}
                \frac{\Big\{ p_{11} - p_{10}\Big\}(1 - x)}{y} + p^\prime_{11} < \frac{p^\prime_{11} - (1 - x)}{x}\\
                \implies x\{p_{11} - p_{10}\}(1 - x) + p^\prime_{11}xy < p^\prime_{11}y - y(1 - x)\\
                \implies x\{p_{11} - p_{10}\}(1 - x) < p^\prime_{11}y(1 - x) - y(1 - x)\\
                \implies x\{p_{11} - p_{10}\} < p^\prime_{11}y - y\\
                \implies x\{p_{11} - p_{10}\} < -yp^\prime_{01}\\
            \end{align*}
            This produces a contradiction since $p_{11} - p_{10} > 0$. Hence, 
            \[
            \frac{p^\prime_{11} - (1 - x)}{x} \leq \frac{p_{11} - p^\prime_{10}y_0}{y_1}
            \]
        \item Lower Bound Of $\frac{p_{11} - (1 - y)}{y}$: Following a similar proof by contradiction:
            \begin{align*}
                \frac{\Big\{ p_{11} - p_{10}\Big\}(1 - x)}{y} + p^\prime_{11} < \frac{p_{11} - (1 - y)}{y}\\
                \implies \Big\{ p_{11} - p_{10}\Big\}(1 - x) + p^\prime_{11}y < p_{11} - (1 - y)\\
                \implies -p_{10}(1 - x) - p_{11}x + p^\prime_{11}y < -(1 - y)\\
                \xRightarrow{p_{11}x + p_{10}(1-x) = p'_{11}y + p'_{10}(1-y) } -p^\prime_{10}(1 - y) < -(1 - y)
                \implies p^\prime_{10} > 1
            \end{align*}
            This is a contradiction from the properties of probability.
        \item When the lower bound is $\frac{p^\prime_{11}y - p_{10}(1 - x)}{xy}$. Following a similar proof by contradiction
            \begin{align*}
                \frac{\Big\{ p_{11} - p_{10}\Big\}(1 - x)}{y} + p^\prime_{11} < \frac{p^\prime_{11}y - p_{10}(1 - x)}{xy}\\
                \implies \Big\{ p_{11} - p_{10}\Big\}(1 - x) + p^\prime_{11}y < \frac{p^\prime_{11}y - p_{10}(1 - x)}{x}\\
                \implies x\Big\{ p_{11} - p_{10}\Big\}(1 - x) + p^\prime_{11}yx < p^\prime_{11}y - p_{10}(1 - x)\\
                \implies x\Big\{ p_{11} - p_{10}\Big\}(1 - x) < p^\prime_{11}y(1 - x) - p_{10}(1 - x)\\
                \implies x\Big\{ p_{11} - p_{10}\Big\} < p^\prime_{11}y - p_{10}\\
                \implies xp_{11} + p_{10}(1 - x) - p^\prime_{11}y < 0\\
                \xRightarrow{p_{11}x + p_{10}(1-x) = p'_{11}y + p'_{10}(1-y) } p^\prime_{10}(1 - y) < 0
            \end{align*}
            This produces a contradiction as well.
    \end{enumerate}
    \item Checking whether the upper bounds are less than $p^\prime_{11}$: Folloing a similar proof by contradiction on a case by case basis, we enumerate the cases below. 
    \begin{enumerate}
        \item The upper bound is $1$: This can never be less than $p^\prime_{11}$ from the properties of probability. 
        \item The upper bound is $\frac{p^\prime_{11}}{x}$: this will also hold since $x \leq 1$. 
        \item The upper bound is $\frac{p_{11}}{y}$: Assume $p^\prime_{11} > \frac{p_{11}}{y}$
            \begin{align*}
                \implies p^\prime_{11}y > p_{11}\\
                \implies p_{11}x + p_{10}(1 - x) - p^\prime_{10}(1 - y) > p_{11}\\
                \implies - p^\prime_{10}(1 - y) > \{p_{11} - p_{10}\}(1 - x)\\
            \end{align*}
        This produces a contradiction since $p_{11} - p_{10} > 0$ by assumption. 
        \item The upper bound is $\frac{(1 - x)y_0 - p_{10}(1 - x) + p^\prime_{11}y_1}{xy_1}$: Assume $p^\prime_{11} > \frac{(1 - x)y_0 - p_{10}(1 - x) + p^\prime_{11}y_1}{xy_1}$
        \begin{align*}
            \implies p^\prime_{11}xy > (1 - x)(1 - y) - p_{10}(1 - x) + p^\prime_{11}y\\
            \implies 0 > (1 - x)(1 - y) - p_{10}(1 - x) + p^\prime_{11}y(1 - x)\\
            \implies 0 > (1 - y) - p_{10} + p^\prime_{11}y\\
            \implies p_{10} > (1-y) + p^\prime_{11}y\\
            \implies 0> (1-y) + p_{11}x - p_{10} x - p'_{10}(1-y)\\
            \implies p'_{10}(1-y) > (1-y) + x(p_{11}-p_{10})\\
            \implies (p'_{10}-1)> x \frac{p_{11}-p_{10}}{1-y}
        \end{align*}
        which is a contradiction because $x \frac{p_{11}-p_{10}}{1-y}$ is a positive quantity and $p'_{10}-1$ is a negative one, since $p'_{10}$ is a probability. 
    \end{enumerate}
    A similar argument can be applied for the rest of the cases. 
\end{enumerate}

So, in this case of $p_{11} - p_{10} > 0$, we have shown that the lower bound of the free parameter is less than $\frac{p_{11} - p^\prime_{10}y_0}{y_1}$, while the upper bound is greater than $p^\prime_{11}$. This means we consider the following cases - where we denote $lb$ as lower bound of $P(Z = 1 \mid X = 1, Y = 1)$ and $ub$ as the upper bound. 
\newline
\begin{enumerate}
    \item $lb \leq p^\prime_{11}$ and $p^\prime_{11} \leq ub \leq \frac{p_{11} - p^\prime_{10}y_0}{y_1}$: In this case, the range of $P(Z = 1 \mid X = 1, Y = 1)$ allows for a value of $P(Z = 1 \mid X = 1, Y = 1)$ between $p^\prime_{11}$ and $\frac{p_{11} - p^\prime_{10}y_0}{y_1}$ where both max operators return non-zero terms and equal $p_{11} - p_{10}$. However, let's consider a value of $P(Z = 1 \mid X = 1, Y = 1) = p^\prime_{11}$. In this case, $\max\Big\{0, \frac{\mathbb{P}(Z = 1 \mid X = 1, Y = 1) - p^\prime_{11}}{1 - x}\Big\}$ will return $0$. However, $\max\Big\{0, \frac{p_{11} - p^\prime_{10}y_0 - y_1\mathbb{P}(Z = 1\mid X = 1, Y = 1)}{(1 - x)y_0}  \Big\}$ will evaluate to a non-zero term since $p^\prime_{11} < \frac{p_{11} - p^\prime_{10}y_0} {y_1}$. Evaluating $\max\Big\{0, \frac{p_{11} - p^\prime_{10}y_0 - y_1\mathbb{P}(Z = 1\mid X = 1, Y = 1)}{(1 - x)y_0}  \Big\}$ when $P(Z = 1 \mid X = 1, Y = 1) = p^\prime_{11}$, it will equal $\frac{p_{11} - p_{10}}{y_0}$, and the $y_0$ will cancel out with the $y_0$ that each max operator is multiplied by in $\Delta$. So even when only a single max operator opens, it will open at a value $\geq p_{11} - p_{10}$, and hence the final bound will always be equal to $p_{11} - p_{10}$ when $p_{11} - p_{10} > 0$. 
\end{enumerate}

Since we have shown that the range of $P(Z = 1 \mid X = 1, Y = 1)$ will always include values where $\min_{P(Z = 1 \mid X = 1, Y = 1)} \Delta(P(Z = 1 \mid X = 1, Y = 1))$ is $0$ or $p_{11} - p_{10}$ depending on $p_{11} - p_{10} > 0$ or not, we conclude the lower bound is 
\[
\max\{0, p_{11} - p_{10}\} \leq PNS
\]

% \subsection{Solving Problem With Binary Covariates}
% \begin{align*}
%     &\mathbb{P}(Z = 1 \mid X = 1, C = 0) = \\
%     &\mathbb{P}(Z = 1 \mid X = 1, Y = 1, C = 0)\mathbb{P}(Y = 1) + \mathbb{P}(Z = 1 \mid X = 1, Y = 0, C = 0)\mathbb{P}(Y = 0)\\
%     &\mathbb{P}(Z = 1 \mid X = 1, C = 1) = \\
%     &\mathbb{P}(Z = 1 \mid X = 1, Y = 1, C = 1)\mathbb{P}(Y = 1) + \mathbb{P}(Z = 1 \mid X = 1, Y = 0, C = 1)\mathbb{P}(Y = 0)\\
%     &\mathbb{P}(Z = 1 \mid X = 0, C = 0) = \\
%     &\mathbb{P}(Z = 1 \mid X = 0, Y = 1, C = 0)\mathbb{P}(Y = 1) + \mathbb{P}(Z = 1 \mid X = 0, Y = 0, C = 0)\mathbb{P}(Y = 0)\\
%     &\mathbb{P}(Z = 1 \mid X = 0, C = 1) = \\
%     &\mathbb{P}(Z = 1 \mid X = 0, Y = 1, C = 1)\mathbb{P}(Y = 1) + \mathbb{P}(Z = 1 \mid X = 0, Y = 0, C = 1)\mathbb{P}(Y = 0)\\
%     &\mathbb{P}(Z = 1 \mid Y = 1, C = 0) = \\
%     &\mathbb{P}(Z = 1 \mid X = 0, Y = 1, C = 0)\mathbb{P}(X = 0) + \mathbb{P}(Z = 1 \mid X = 1, Y = 1, C = 0)\mathbb{P}(X = 1)\\
%     &\mathbb{P}(Z = 1 \mid Y = 1, C = 1) = \\
%     &\mathbb{P}(Z = 1 \mid X = 0, Y = 1, C = 1)\mathbb{P}(X = 0) + \mathbb{P}(Z = 1 \mid X = 1, Y = 1, C = 1)\mathbb{P}(X = 1)\\
%     &\mathbb{P}(Z = 1 \mid Y = 0, C = 0) = \\
%     &\mathbb{P}(Z = 1 \mid X = 0, Y = 0, C = 0)\mathbb{P}(X = 0) + \mathbb{P}(Z = 1 \mid X = 1, Y = 0, C = 0)\mathbb{P}(X = 1)\\
%     &\mathbb{P}(Z = 1 \mid Y = 0, C = 1) = \\
%     &\mathbb{P}(Z = 1 \mid X = 0, Y = 0, C = 1)\mathbb{P}(X = 0) + \mathbb{P}(Z = 1 \mid X = 1, Y = 0, C = 1)\mathbb{P}(X = 1)
% \end{align*}

% Now, this can be written as a system of linear equations as $A\mathbf{x} = \mathbf{b}$ where 
% \begin{align*}
%     \mathbf{x} = \begin{bmatrix}
%                     \mathbb{P}(Z = 1 \mid X = 0, Y = 0, C = 0)\\
%                     \mathbb{P}(Z = 1 \mid X = 1, Y = 0, C = 0)\\
%                     \mathbb{P}(Z = 1 \mid X = 0, Y = 1, C = 0)\\
%                     \mathbb{P}(Z = 1 \mid X = 1, Y = 1, C = 0)\\
%                     \mathbb{P}(Z = 1 \mid X = 0, Y = 0, C = 1)\\
%                     \mathbb{P}(Z = 1 \mid X = 1, Y = 0, C = 1)\\
%                     \mathbb{P}(Z = 1 \mid X = 0, Y = 1, C = 1)\\
%                     \mathbb{P}(Z = 1 \mid X = 1, Y = 1, C = 1)\\
%                 \end{bmatrix}
% \end{align*}

% And $\mathbf{b}$ is 
% \begin{align*}
%     \mathbf{b} = \begin{bmatrix}
%                     \mathbb{P}(Z = 1 \mid Y = 0, C = 0)\\
%                     \mathbb{P}(Z = 1 \mid Y = 1, C = 0)\\
%                     \mathbb{P}(Z = 1 \mid X = 0, C = 0)\\
%                     \mathbb{P}(Z = 1 \mid X = 1, C = 0)\\
%                     \mathbb{P}(Z = 1 \mid Y = 0, C = 1)\\
%                     \mathbb{P}(Z = 1 \mid Y = 1, C = 1)\\
%                     \mathbb{P}(Z = 1 \mid X = 0, C = 1)\\
%                     \mathbb{P}(Z = 1 \mid X = 1, C = 1)
%                  \end{bmatrix}
% \end{align*}

% And the coefficient matrix can be written as
% {\tiny
% \begin{align*}
%     A = \begin{bmatrix}
%         P(X = 0) & P(X = 1) & 0 & 0 & 0 & 0 & 0 & 0 \\
%         0& 0& P(X = 0) & P(X = 1) & 0 & 0& 0 & 0 \\
%         P(Y = 0)& 0& P(Y = 1)& 0& 0& 0& 0& 0 \\
%         0 & P(Y = 0) & 0 & P(Y = 1) & 0 & 0 & 0 & 0 \\
%         0 & 0 & 0& 0 & P(X = 0) &  P(X = 1) & 0& 0 \\
%         0 & 0 & 0 & 0& 0 & 0 & P(X = 0) & P(X = 1) \\
%         0 & 0 & 0 & 0 & P(Y = 0) & 0 & P(Y = 1) & 0 \\
%         0 & 0 & 0 & 0 & 0 & P(Y = 0) & 0 & P(Y = 1) \\
%         \end{bmatrix}
% \end{align*}
% }
% The augmented matrix in RREF looks like
% {\tiny
% \begin{align*}
%     \begin{bmatrix}
% 1 &  0 &  0 &  -OR(X)OR(Y) &  0 &  0 &  0 & 0 &  \frac{P(Z = 1 \mid X = 0, C = 0)P(X = 0) - P(Z = 1 \mid Y = 1, C = 0)P(Y = 1)}{P(X = 0)P(Y = 0)}\\
% 0 &  1 &  0 & OR(Y) &  0 &  0 &  0 & 0 & \frac{P(Z = 1 \mid X = 1, C = 0)}{P(Y = 0)}\\
% 0 &  0 &  1 & OR(X) &  0 &  0 &  0 & 0 & \frac{P(Z = 1 \mid Y = 1, C = 0)}{P(X = 0)}\\
% 0 &  0 &  0 & 0 &  1 &  0 &  0 &  -OR(X)OR(Y) & \frac{P(Z = 1 \mid X = 0, C = 0)P(X = 0) - P(Z = 1 \mid Y = 1, C = 0)P(Y = 1)}{P(X = 0)P(Y = 0)}\\
% 0 &  0 &  0 & 0 &  0 &  1 &  0 & OR(Y) & \frac{P(Z = 1 \mid X = 1, C = 1)}{P(Y = 0)}\\
% 0 &  0 &  0 & 0 &  0 &  0 &  1 & OR(X) & \frac{P(Z = 1 \mid Y = 1, C = 1)}{P(X = 0)}\\
% 0 &  0 &  0 & 0 &  0 &  0 &  0 & 0 &  0\\
% 0 &  0 &  0 & 0 &  0 &  0 &  0 & 0 &  0\\
%     \end{bmatrix}
% \end{align*}
% }

% {\color{red} Formally write up simplification from MATLAB}
% Note this looks similar to the RREF without covariates,but every type of row is now repeated for every level of $C$. This prompts the following proof by induction to deal with covariates of arbitrary dimensionality. 

% \subsection{Mathematical Induction Proof}

% % \textbf{Proposition}: $P(n)$ For covariates $C$ with cardinality $n$,  $n \geq 2$, the RREF of the constraint matrix will be a matrix with $4n$ rows and $4n + 1$ columns, and will have have a repeating structure as seen above

% % \textbf{Proof}: For the base case of $n = 2$, we can see this holds from the above RREF matrix. Now we proceed with the induction step, i.e. we prove that if $P(n)$ holds, then $P(n + 1)$ also holds. Now onwards, $A_n$ denotes the coefficient matrix for when $C$ has cardinality of $n$, same for $\mathbf{b}_n$ and $\mathbf{x}_n$. 

% % The system of equations for when $C$ has $n+1$ levels can be written as 
% % \begin{align*}
% %     &\mathbf{x}_{n + 1} = \begin{bmatrix}
% %                             \mathbf{x}_n\\
% %                             \mathbb{P}(Z = 1 \mid X = 0, Y = 0, C = n + 1)\\
% %                             \mathbb{P}(Z = 1 \mid X = 1, Y = 0, C = n + 1)\\
% %                             \mathbb{P}(Z = 1 \mid X = 0, Y = 1, C = n + 1)\\
% %                             \mathbb{P}(Z = 1 \mid X = 1, Y = 1, C = n + 1)\\
% %                         \end{bmatrix}\\
% %     &\mathbf{b}_{n + 1} = \begin{bmatrix}
% %                             \mathbf{b}_n\\
% %                             \mathbb{P}(Z = 1 \mid Y = 0, C = n + 1)\\
% %                             \mathbb{P}(Z = 1 \mid Y = 1, C = n + 1)\\
% %                             \mathbb{P}(Z = 1 \mid X = 0, C = n + 1)\\
% %                             \mathbb{P}(Z = 1 \mid X = 1, C = n + 1)
% %                         \end{bmatrix}
% % \end{align*}

% % And similarly, $A_{n + 1}$ will look like 
% % \begin{align*}
% %     A_{n + 1} = \begin{bmatrix}
% %                     A_n & [\mathbf{0}]\\
% %                     [\mathbf{0}] & \begin{bmatrix}
% %                                     P(X = 0) & P(X = 1) & 0 & 0\\
% %                                     0& 0& P(X = 0) & P(X = 1) \\
% %                                     P(Y = 0)& 0& P(Y = 1)& 0\\
% %                                     0 & P(Y = 0) & 0 & P(Y = 1)\\
% %                                     \end{bmatrix}
% %                 \end{bmatrix}
% % \end{align*}

% % So, putting $A_{n + 1}$ requires using to put the bottom right quadrant into RREF, which we have done beffore, and so it will look like
% % \begin{align*}
% %     A_{n + 1} = \begin{bmatrix}
% %                     A_n & [\mathbf{0}]\\
% %                     [\mathbf{0}] & \begin{bmatrix}
% %                                     1 & 0 & 0 & -OR(X)OR(Y)\\
% %                                     0 & 1 & 0 & OR(Y) \\
% %                                     0 & 0 & 1 & OR(X) \\
% %                                     0 & 0 & 0 & 0\\
% %                                     \end{bmatrix}
% %                 \end{bmatrix}
% % \end{align*}

% % And $\mathbf{b}_n$ will consequently be transformed as
% % \begin{align*}
% %     \mathbf{b}_{n + 1} = \begin{bmatrix}
% %                             \mathbf{b}_n\\
% %                             \frac{P(Z = 1 \mid X = 0, C = n + 1)P(X = 0) - P(Z = 1 \mid Y = 1, C = n + 1)P(Y = 1)}{P(X = 0)P(Y = 0)}\\
% %                             \frac{P(Z = 1 \mid X = 1, C = n + 1)}{P(Y = 0)}\\
% %                             \frac{P(Z = 1 \mid Y = 1, C = n + 1)}{P(X = 0)}\\
% %                             0\\
% %                         \end{bmatrix}
% % \end{align*}

% % Which proves that $P(n + 1)$ holds as well if $P(n)$ holds.

% % {\color{red} Numair will write $P(n)$ more thoroughly later.}

\bibliography{references}
\end{document}
